# Supplementary material for: Robust Detection of Lead-Lag Relationships in Lagged Multi-Factor Models
Source: arXiv:2305.06704 source file (2023-09-19)
Supplement: Supplementary file 1 [file supplementary.tex]

% \documentclass{article}

% % Language setting
% % Replace `english' with e.g. `spanish' to change the document language
% \usepackage[english]{babel}

% % Set page size and margins
% % Replace `letterpaper' with`a4paper' for UK/EU standard size
% \usepackage[a4paper,top=2cm,bottom=2cm,left=3cm,right=3cm,marginparwidth=2cm]{geometry}
% %\renewcommand{\baselinestretch}{1.5} 

% \usepackage{setspace}
% \setstretch{1.5}

% % Useful packages
% \usepackage{amsmath}
% \usepackage{graphicx}
% \usepackage{setspace}
% \usepackage{multirow}
% \usepackage{longtable}
% %\usepackage[margin=1.5in]{geometry} 
% \usepackage[english]{babel}
% \usepackage[utf8]{inputenc}
% \usepackage{algorithm}
% \usepackage[noend]{algpseudocode}
% \usepackage{csquotes}
% \usepackage{subcaption}
% \usepackage{graphicx}
% \usepackage{tikz}
% \usepackage{lipsum}
% \usepackage{tcolorbox}
% \usepackage{tabularx}
% \usepackage{booktabs}
% \usepackage{listings}
% \usepackage{titlesec}
% \usepackage{longtable}
% \usepackage{rotating}
% \usepackage{pdflscape}
% \newlength{\RoundedBoxWidth}
% \newsavebox{\GrayRoundedBox}
% \newenvironment{GrayBox}[1][\dimexpr\textwidth-4.5ex]%
%    {\setlength{\RoundedBoxWidth}{\dimexpr#1}
%     \begin{lrbox}{\GrayRoundedBox}
%        \begin{minipage}{\RoundedBoxWidth}}%
%    {   \end{minipage}
%     \end{lrbox}
%     \begin{center}
%     \begin{tikzpicture}%
%        \draw node[draw=black,fill=black!10,rounded corners,%
%              inner sep=2ex,text width=\RoundedBoxWidth]%
%              {\usebox{\GrayRoundedBox}};
%     \end{tikzpicture}
%     \end{center}}


% \usepackage{placeins} 
% \newcolumntype{Y}{>{\raggedleft\arraybackslash}X}% raggedleft column X

% \usepackage[colorlinks=true, allcolors=blue]{hyperref}
% %\usepackage[colorlinks=true,linkcolor=red,filecolor=green,citecolor=blue]{hyperref}


% \usepackage{amsfonts}
% %\usepackage[round]{natbib}
% \usepackage[citestyle=bwl-FU]{biblatex}
% \addbibresource{./reference.bib}
% \graphicspath{ {./graphs/} }


% \newcommand{\gr}[1]{\textcolor{blue}{{{}}#1}{}}
% \newcommand{\mc}[1]{\textcolor{cyan}{{{}}#1}{}}
% \newcommand{\yl}[1]{\textcolor{red}{{{}}#1}{}}


% \newcommand{\gcomm}[1]{\marginpar{\tiny\textcolor{blue}{{{}}#1}{}}}

% % \newcommand{\MC}[1]{\marginpar{\tiny\textcolor{red}{{{}}#1}{}}}


% \newcounter{noteMCctr} \setcounter{noteMCctr}{1}
% \newcommand{\MC}[1]{\textbf{\textcolor{red}{{{MC: \#\arabic{noteMCctr}: }}#1}} \addtocounter{noteMCctr}{1}}

% \newcounter{noteYZctr} \setcounter{noteYZctr}{1}
% \newcommand{\YZ}[1]{\textbf{\textcolor{blue}{{{YZ: \#\arabic{noteYZctr}: }}#1}} \addtocounter{noteYZctr}{1}}

% %  \definecolor{colour3}{RGB}{178,55,250} % purple
% %  \newcommand{\mc}[1]{\textcolor{red}{{{}}#1}}



% %\renewcommand{\thetable}{S\arabic{table}}

% \begin{document}




% \appendix
\setcounter{page}{1}
\begin{landscape}
\section*{Supplemental material}
\subsection*{Equity data set: performance metrics for the entire grid -  rescaled to target volatility}
\label{equity_full_results}

% Table \ref{tab: equity_grid} provides performance metrics for the entire grid (rescaled to target volatility). The experiment has
% been set with the values $p = \{1,3,5,7\}$, $\delta = \{1,3,5,7\}$, and $\alpha = \{0.7,0.75,0.8,0.85\}$.

\begin{small}
\captionof{table}*{Table S1: Equity data set: performance metrics for the entire grid - rescaled to target volatility. The experiment has
been set with the values $p = \{1,3,5,7\}$, $\delta = \{1,3,5,7\}$, and $\alpha = \{0.7,0.75,0.8,0.85\}$.}
\label{tab: equity_grid}
\begin{longtable}{|p{2.9cm}p{1.2cm}p{0.1cm}p{0.1cm}p{0.5cm}p{0.5cm}p{1.4cm}p{1.2cm}p{1.6cm}p{1.7cm}p{1cm}p{1cm}p{0.5cm}p{1.2cm}p{1.4cm}p{0.9cm}p{1.5cm}|}
\toprule
\textbf{Method}       & \textbf{Strategy}   & \textbf{$p$} & \textbf{$\delta$} & \textbf{$\alpha$} & \textbf{$\beta$} & \textbf{E[Returns]} & \textbf{Volatility}  & \textbf{Downside deviation} & \textbf{Maximum drawdown} & \textbf{Sortino ratio} & \textbf{Calmar ratio} & \textbf{Hit rate} & \textbf{$\frac{\text{Avg. profit}}{\text{Avg. loss}}$} & \textbf{PnL per trade}  & \textbf{Sharpe ratio} & \textbf{P-value} \\
\midrule
KM\_Mod   & $G_\beta$ & 1 & 1     & 0.85  & 0.15 & -0.049        & 0.15 & 0.107              & -0.832        & -0.454  & -0.058 & 0.494    & 0.967                   & -1.928 & -0.324 & 0.152   \\
KM\_Med & $G_\beta$ & 1 & 1     & 0.85  & 0.15 & -0.025        & 0.15 & 0.107              & -0.761        & -0.235  & -0.033 & 0.497    & 0.981                   & -0.995 & -0.167 & 0.46    \\
SP\_Mod   & $G_\beta$ & 1 & 1     & 0.85  & 0.15 & -0.07         & 0.15 & 0.11               & -0.879        & -0.639  & -0.08  & 0.492    & 0.949                   & -2.788 & -0.468 & 0.038   \\
SP\_Med  & $G_\beta$ & 1 & 1     & 0.85  & 0.15 & -0.117        & 0.15 & 0.111              & -0.935        & -1.056  & -0.125 & 0.479    & 0.943                   & -4.656 & -0.782 & 0.001   \\
KM\_Mod   & $G_\beta$ & 1 & 3     & 0.85  & 0.15 & -0.047        & 0.15 & 0.108              & -0.765        & -0.433  & -0.061 & 0.487    & 0.999                   & -1.853 & -0.311 & 0.168   \\
KM\_Med & $G_\beta$ & 1 & 3     & 0.85  & 0.15 & -0.066        & 0.15 & 0.111              & -0.827        & -0.592  & -0.08  & 0.485    & 0.983                   & -2.609 & -0.438 & 0.051   \\
SP\_Mod   & $G_\beta$ & 1 & 3     & 0.85  & 0.15 & -0.016        & 0.15 & 0.109              & -0.658        & -0.147  & -0.024 & 0.494    & 1.005                   & -0.638 & -0.107 & 0.635   \\
SP\_Med  & $G_\beta$ & 1 & 3     & 0.85  & 0.15 & -0.033        & 0.15 & 0.109              & -0.668        & -0.301  & -0.049 & 0.494    & 0.983                   & -1.299 & -0.218 & 0.334   \\
KM\_Mod   & $G_\beta$ & 1 & 5     & 0.85  & 0.15 & 0.027         & 0.15 & 0.103              & -0.511        & 0.258   & 0.052  & 0.508    & 1.001                   & 1.052  & 0.177  & 0.434   \\
KM\_Med & $G_\beta$ & 1 & 5     & 0.85  & 0.15 & 0.004         & 0.15 & 0.107              & -0.68         & 0.038   & 0.006  & 0.5      & 1.005                   & 0.162  & 0.027  & 0.904   \\
SP\_Mod   & $G_\beta$ & 1 & 5     & 0.85  & 0.15 & 0.021         & 0.15 & 0.106              & -0.627        & 0.199   & 0.033  & 0.502    & 1.016                   & 0.831  & 0.14   & 0.537   \\
SP\_Med  & $G_\beta$ & 1 & 5     & 0.85  & 0.15 & 0.034         & 0.15 & 0.103              & -0.55         & 0.333   & 0.062  & 0.5      & 1.04                    & 1.358  & 0.228  & 0.313   \\
KM\_Mod   & $G_\beta$ & 1 & 7     & 0.85  & 0.15 & 0.086         & 0.15 & 0.101              & -0.3          & 0.852   & 0.286  & 0.513    & 1.051                   & 3.408  & 0.573  & 0.011   \\
KM\_Med & $G_\beta$ & 1 & 7     & 0.85  & 0.15 & 0.058         & 0.15 & 0.102              & -0.27         & 0.573   & 0.216  & 0.507    & 1.042                   & 2.311  & 0.388  & 0.085   \\
SP\_Mod   & $G_\beta$ & 1 & 7     & 0.85  & 0.15 & 0.038         & 0.15 & 0.105              & -0.44         & 0.365   & 0.087  & 0.504    & 1.031                   & 1.518  & 0.255  & 0.259   \\
SP\_Med  & $G_\beta$ & 1 & 7     & 0.85  & 0.15 & 0.02          & 0.15 & 0.11               & -0.441        & 0.178   & 0.045  & 0.511    & 0.981                   & 0.78   & 0.131  & 0.563   \\
KM\_Mod   & $G_\beta$ & 3 & 1     & 0.85  & 0.15 & 0             & 0.15 & 0.105              & -0.615        & -0.005  & -0.001 & 0.506    & 0.977                   & -0.019 & -0.003 & 0.989   \\
KM\_Med & $G_\beta$ & 3 & 1     & 0.85  & 0.15 & -0.004        & 0.15 & 0.107              & -0.638        & -0.035  & -0.006 & 0.503    & 0.985                   & -0.149 & -0.025 & 0.912   \\
SP\_Mod   & $G_\beta$ & 3 & 1     & 0.85  & 0.15 & -0.045        & 0.15 & 0.111              & -0.751        & -0.405  & -0.06  & 0.502    & 0.941                   & -1.782 & -0.299 & 0.185   \\
SP\_Med  & $G_\beta$ & 3 & 1     & 0.85  & 0.15 & -0.065        & 0.15 & 0.111              & -0.802        & -0.587  & -0.082 & 0.49     & 0.961                   & -2.594 & -0.436 & 0.053   \\
KM\_Mod   & $G_\beta$ & 3 & 3     & 0.85  & 0.15 & -0.023        & 0.15 & 0.105              & -0.603        & -0.221  & -0.039 & 0.491    & 1.01                    & -0.922 & -0.155 & 0.493   \\
KM\_Med & $G_\beta$ & 3 & 3     & 0.85  & 0.15 & -0.028        & 0.15 & 0.107              & -0.635        & -0.266  & -0.045 & 0.49     & 1.005                   & -1.128 & -0.189 & 0.402   \\
SP\_Mod   & $G_\beta$ & 3 & 3     & 0.85  & 0.15 & 0.003         & 0.15 & 0.108              & -0.453        & 0.031   & 0.007  & 0.497    & 1.017                   & 0.132  & 0.022  & 0.922   \\
SP\_Med  & $G_\beta$ & 3 & 3     & 0.85  & 0.15 & -0.001        & 0.15 & 0.108              & -0.515        & -0.011  & -0.002 & 0.5      & 0.999                   & -0.045 & -0.008 & 0.973   \\
KM\_Mod   & $G_\beta$ & 3 & 5     & 0.85  & 0.15 & 0.023         & 0.15 & 0.098              & -0.605        & 0.236   & 0.038  & 0.502    & 1.021                   & 0.916  & 0.154  & 0.495   \\
KM\_Med & $G_\beta$ & 3 & 5     & 0.85  & 0.15 & 0.037         & 0.15 & 0.104              & -0.472        & 0.354   & 0.078  & 0.506    & 1.018                   & 1.457  & 0.245  & 0.279   \\
SP\_Mod   & $G_\beta$ & 3 & 5     & 0.85  & 0.15 & 0.016         & 0.15 & 0.098              & -0.525        & 0.164   & 0.031  & 0.492    & 1.054                   & 0.637  & 0.107  & 0.635   \\
SP\_Med  & $G_\beta$ & 3 & 5     & 0.85  & 0.15 & 0.022         & 0.15 & 0.101              & -0.561        & 0.216   & 0.039  & 0.495    & 1.047                   & 0.861  & 0.145  & 0.522   \\
KM\_Mod   & $G_\beta$ & 3 & 7     & 0.85  & 0.15 & 0.097         & 0.15 & 0.102              & -0.222        & 0.952   & 0.438  & 0.518    & 1.044                   & 3.856  & 0.648  & 0.004   \\
KM\_Med & $G_\beta$ & 3 & 7     & 0.85  & 0.15 & 0.09          & 0.15 & 0.101              & -0.292        & 0.895   & 0.31   & 0.518    & 1.036                   & 3.587  & 0.603  & 0.007   \\
SP\_Mod   & $G_\beta$ & 3 & 7     & 0.85  & 0.15 & 0.074         & 0.15 & 0.105              & -0.42         & 0.701   & 0.175  & 0.515    & 1.027                   & 2.92   & 0.491  & 0.03    \\
SP\_Med  & $G_\beta$ & 3 & 7     & 0.85  & 0.15 & 0.051         & 0.15 & 0.108              & -0.511        & 0.473   & 0.1    & 0.514    & 1.004                   & 2.027  & 0.341  & 0.133   \\
KM\_Mod   & $G_\beta$ & 5 & 1     & 0.85  & 0.15 & -0.036        & 0.15 & 0.106              & -0.761        & -0.343  & -0.048 & 0.5      & 0.956                   & -1.446 & -0.243 & 0.283   \\
KM\_Med & $G_\beta$ & 5 & 1     & 0.85  & 0.15 & 0             & 0.15 & 0.106              & -0.74         & 0.003   & 0      & 0.501    & 0.997                   & 0.011  & 0.002  & 0.994   \\
SP\_Mod   & $G_\beta$ & 5 & 1     & 0.85  & 0.15 & -0.072        & 0.15 & 0.109              & -0.897        & -0.661  & -0.08  & 0.489    & 0.958                   & -2.859 & -0.48  & 0.034   \\
SP\_Med  & $G_\beta$ & 5 & 1     & 0.85  & 0.15 & -0.079        & 0.15 & 0.111              & -0.871        & -0.714  & -0.091 & 0.486    & 0.959                   & -3.151 & -0.529 & 0.019   \\
KM\_Mod   & $G_\beta$ & 5 & 3     & 0.85  & 0.15 & 0.007         & 0.15 & 0.103              & -0.501        & 0.067   & 0.014  & 0.496    & 1.023                   & 0.274  & 0.046  & 0.838   \\
KM\_Med & $G_\beta$ & 5 & 3     & 0.85  & 0.15 & 0.001         & 0.15 & 0.104              & -0.515        & 0.007   & 0.001  & 0.498    & 1.011                   & 0.03   & 0.005  & 0.982   \\
SP\_Mod   & $G_\beta$ & 5 & 3     & 0.85  & 0.15 & 0.02          & 0.15 & 0.104              & -0.471        & 0.193   & 0.043  & 0.493    & 1.053                   & 0.796  & 0.134  & 0.554   \\
SP\_Med  & $G_\beta$ & 5 & 3     & 0.85  & 0.15 & 0.03          & 0.15 & 0.105              & -0.489        & 0.282   & 0.061  & 0.502    & 1.028                   & 1.181  & 0.198  & 0.38    \\
KM\_Mod   & $G_\beta$ & 5 & 5     & 0.85  & 0.15 & 0.081         & 0.15 & 0.1                & -0.356        & 0.81    & 0.228  & 0.511    & 1.055                   & 3.225  & 0.542  & 0.016   \\
KM\_Med & $G_\beta$ & 5 & 5     & 0.85  & 0.15 & 0.099         & 0.15 & 0.104              & -0.271        & 0.953   & 0.365  & 0.518    & 1.048                   & 3.929  & 0.66   & 0.004   \\
SP\_Mod   & $G_\beta$ & 5 & 5     & 0.85  & 0.15 & 0.062         & 0.15 & 0.1                & -0.378        & 0.62    & 0.164  & 0.5      & 1.078                   & 2.454  & 0.412  & 0.067   \\
SP\_Med  & $G_\beta$ & 5 & 5     & 0.85  & 0.15 & 0.019         & 0.15 & 0.103              & -0.57         & 0.182   & 0.033  & 0.498    & 1.033                   & 0.742  & 0.125  & 0.581   \\
KM\_Mod   & $G_\beta$ & 5 & 7     & 0.85  & 0.15 & 0.129         & 0.15 & 0.1                & -0.155        & 1.29    & 0.834  & 0.523    & 1.062                   & 5.128  & 0.862  & 0       \\
KM\_Med & $G_\beta$ & 5 & 7     & 0.85  & 0.15 & 0.123         & 0.15 & 0.098              & -0.282        & 1.254   & 0.435  & 0.518    & 1.078                   & 4.865  & 0.817  & 0       \\
SP\_Mod   & $G_\beta$ & 5 & 7     & 0.85  & 0.15 & 0.105         & 0.15 & 0.102              & -0.227        & 1.024   & 0.462  & 0.514    & 1.073                   & 4.161  & 0.699  & 0.002   \\
SP\_Med  & $G_\beta$ & 5 & 7     & 0.85  & 0.15 & 0.059         & 0.15 & 0.105              & -0.281        & 0.563   & 0.211  & 0.51     & 1.03                    & 2.355  & 0.396  & 0.08    \\
KM\_Mod   & $G_\beta$ & 7 & 1     & 0.85  & 0.15 & -0.021        & 0.15 & 0.103              & -0.662        & -0.205  & -0.032 & 0.493    & 1.003                   & -0.841 & -0.141 & 0.532   \\
KM\_Med & $G_\beta$ & 7 & 1     & 0.85  & 0.15 & 0.004         & 0.15 & 0.105              & -0.597        & 0.04    & 0.007  & 0.496    & 1.022                   & 0.169  & 0.028  & 0.9     \\
SP\_Mod   & $G_\beta$ & 7 & 1     & 0.85  & 0.15 & -0.026        & 0.15 & 0.107              & -0.682        & -0.239  & -0.038 & 0.494    & 0.993                   & -1.018 & -0.171 & 0.449   \\
SP\_Med  & $G_\beta$ & 7 & 1     & 0.85  & 0.15 & -0.047        & 0.15 & 0.109              & -0.721        & -0.431  & -0.065 & 0.487    & 0.994                   & -1.856 & -0.312 & 0.168   \\
KM\_Mod   & $G_\beta$ & 7 & 3     & 0.85  & 0.15 & 0.054         & 0.15 & 0.102              & -0.406        & 0.53    & 0.133  & 0.504    & 1.047                   & 2.145  & 0.36   & 0.11    \\
KM\_Med & $G_\beta$ & 7 & 3     & 0.85  & 0.15 & 0.037         & 0.15 & 0.104              & -0.409        & 0.36    & 0.091  & 0.506    & 1.019                   & 1.479  & 0.248  & 0.272   \\
SP\_Mod   & $G_\beta$ & 7 & 3     & 0.85  & 0.15 & 0.042         & 0.15 & 0.104              & -0.446        & 0.403   & 0.094  & 0.5      & 1.051                   & 1.67   & 0.281  & 0.214   \\
SP\_Med  & $G_\beta$ & 7 & 3     & 0.85  & 0.15 & 0.049         & 0.15 & 0.106              & -0.382        & 0.463   & 0.128  & 0.505    & 1.04                    & 1.945  & 0.327  & 0.148   \\
KM\_Mod   & $G_\beta$ & 7 & 5     & 0.85  & 0.15 & 0.074         & 0.15 & 0.101              & -0.392        & 0.734   & 0.189  & 0.51     & 1.049                   & 2.942  & 0.494  & 0.028   \\
KM\_Med & $G_\beta$ & 7 & 5     & 0.85  & 0.15 & 0.069         & 0.15 & 0.103              & -0.457        & 0.669   & 0.151  & 0.514    & 1.028                   & 2.744  & 0.461  & 0.041   \\
SP\_Mod   & $G_\beta$ & 7 & 5     & 0.85  & 0.15 & 0.04          & 0.15 & 0.103              & -0.32         & 0.387   & 0.124  & 0.501    & 1.045                   & 1.577  & 0.265  & 0.241   \\
SP\_Med  & $G_\beta$ & 7 & 5     & 0.85  & 0.15 & 0.027         & 0.15 & 0.104              & -0.489        & 0.257   & 0.055  & 0.5      & 1.032                   & 1.063  & 0.179  & 0.429   \\
KM\_Mod   & $G_\beta$ & 7 & 7     & 0.85  & 0.15 & 0.143         & 0.15 & 0.101              & -0.213        & 1.42    & 0.672  & 0.522    & 1.085                   & 5.676  & 0.954  & 0       \\
KM\_Med & $G_\beta$ & 7 & 7     & 0.85  & 0.15 & 0.138         & 0.15 & 0.097              & -0.177        & 1.428   & 0.781  & 0.517    & 1.101                   & 5.486  & 0.922  & 0       \\
SP\_Mod   & $G_\beta$ & 7 & 7     & 0.85  & 0.15 & 0.129         & 0.15 & 0.102              & -0.162        & 1.267   & 0.798  & 0.522    & 1.07                    & 5.131  & 0.862  & 0       \\
SP\_Med  & $G_\beta$ & 7 & 7     & 0.85  & 0.15 & 0.084         & 0.15 & 0.105              & -0.256        & 0.794   & 0.327  & 0.513    & 1.051                   & 3.321  & 0.558  & 0.014   \\
KM\_Mod   & $G_\beta$ & 1 & 1     & 0.8   & 0.2  & -0.048        & 0.15 & 0.108              & -0.822        & -0.45   & -0.059 & 0.494    & 0.968                   & -1.924 & -0.323 & 0.153   \\
KM\_Med & $G_\beta$ & 1 & 1     & 0.8   & 0.2  & -0.03         & 0.15 & 0.107              & -0.739        & -0.277  & -0.04  & 0.494    & 0.987                   & -1.173 & -0.197 & 0.384   \\
SP\_Mod   & $G_\beta$ & 1 & 1     & 0.8   & 0.2  & -0.055        & 0.15 & 0.109              & -0.858        & -0.506  & -0.064 & 0.498    & 0.943                   & -2.185 & -0.367 & 0.104   \\
SP\_Med  & $G_\beta$ & 1 & 1     & 0.8   & 0.2  & -0.105        & 0.15 & 0.11               & -0.92         & -0.953  & -0.114 & 0.483    & 0.944                   & -4.17  & -0.7   & 0.002   \\
KM\_Mod   & $G_\beta$ & 1 & 3     & 0.8   & 0.2  & -0.051        & 0.15 & 0.107              & -0.748        & -0.478  & -0.068 & 0.485    & 1                       & -2.023 & -0.34  & 0.133   \\
KM\_Med & $G_\beta$ & 1 & 3     & 0.8   & 0.2  & -0.077        & 0.15 & 0.111              & -0.857        & -0.692  & -0.09  & 0.484    & 0.974                   & -3.047 & -0.512 & 0.023   \\
SP\_Mod   & $G_\beta$ & 1 & 3     & 0.8   & 0.2  & -0.031        & 0.15 & 0.11               & -0.638        & -0.28   & -0.048 & 0.496    & 0.98                    & -1.224 & -0.206 & 0.362   \\
SP\_Med  & $G_\beta$ & 1 & 3     & 0.8   & 0.2  & -0.023        & 0.15 & 0.109              & -0.697        & -0.207  & -0.032 & 0.49     & 1.012                   & -0.893 & -0.15  & 0.507   \\
KM\_Mod   & $G_\beta$ & 1 & 5     & 0.8   & 0.2  & -0.009        & 0.15 & 0.104              & -0.69         & -0.088  & -0.013 & 0.501    & 0.985                   & -0.365 & -0.061 & 0.786   \\
KM\_Med & $G_\beta$ & 1 & 5     & 0.8   & 0.2  & 0.009         & 0.15 & 0.102              & -0.649        & 0.093   & 0.014  & 0.498    & 1.02                    & 0.373  & 0.063  & 0.781   \\
SP\_Mod   & $G_\beta$ & 1 & 5     & 0.8   & 0.2  & 0.027         & 0.15 & 0.105              & -0.648        & 0.256   & 0.042  & 0.5      & 1.033                   & 1.072  & 0.18   & 0.426   \\
SP\_Med  & $G_\beta$ & 1 & 5     & 0.8   & 0.2  & 0.033         & 0.15 & 0.103              & -0.59         & 0.32    & 0.056  & 0.5      & 1.041                   & 1.303  & 0.219  & 0.333   \\
KM\_Mod   & $G_\beta$ & 1 & 7     & 0.8   & 0.2  & 0.087         & 0.15 & 0.102              & -0.301        & 0.852   & 0.288  & 0.512    & 1.058                   & 3.445  & 0.579  & 0.01    \\
KM\_Med & $G_\beta$ & 1 & 7     & 0.8   & 0.2  & 0.045         & 0.15 & 0.104              & -0.309        & 0.431   & 0.145  & 0.509    & 1.019                   & 1.774  & 0.298  & 0.187   \\
SP\_Mod   & $G_\beta$ & 1 & 7     & 0.8   & 0.2  & 0.035         & 0.15 & 0.106              & -0.38         & 0.328   & 0.092  & 0.504    & 1.027                   & 1.383  & 0.232  & 0.304   \\
SP\_Med  & $G_\beta$ & 1 & 7     & 0.8   & 0.2  & 0.03          & 0.15 & 0.11               & -0.429        & 0.276   & 0.071  & 0.51     & 0.997                   & 1.201  & 0.202  & 0.373   \\
KM\_Mod   & $G_\beta$ & 3 & 1     & 0.8   & 0.2  & -0.022        & 0.15 & 0.106              & -0.717        & -0.208  & -0.031 & 0.495    & 0.993                   & -0.879 & -0.148 & 0.514   \\
KM\_Med & $G_\beta$ & 3 & 1     & 0.8   & 0.2  & 0.008         & 0.15 & 0.108              & -0.522        & 0.076   & 0.016  & 0.5      & 1.009                   & 0.325  & 0.055  & 0.81    \\
SP\_Mod   & $G_\beta$ & 3 & 1     & 0.8   & 0.2  & -0.034        & 0.15 & 0.11               & -0.721        & -0.307  & -0.047 & 0.505    & 0.943                   & -1.344 & -0.226 & 0.317   \\
SP\_Med  & $G_\beta$ & 3 & 1     & 0.8   & 0.2  & -0.049        & 0.15 & 0.111              & -0.766        & -0.444  & -0.064 & 0.494    & 0.965                   & -1.947 & -0.327 & 0.148   \\
KM\_Mod   & $G_\beta$ & 3 & 3     & 0.8   & 0.2  & -0.016        & 0.15 & 0.103              & -0.575        & -0.15   & -0.027 & 0.493    & 1.011                   & -0.616 & -0.103 & 0.647   \\
KM\_Med & $G_\beta$ & 3 & 3     & 0.8   & 0.2  & -0.034        & 0.15 & 0.106              & -0.685        & -0.316  & -0.049 & 0.493    & 0.987                   & -1.335 & -0.224 & 0.321   \\
SP\_Mod   & $G_\beta$ & 3 & 3     & 0.8   & 0.2  & -0.019        & 0.15 & 0.108              & -0.624        & -0.175  & -0.03  & 0.496    & 0.995                   & -0.748 & -0.126 & 0.578   \\
SP\_Med  & $G_\beta$ & 3 & 3     & 0.8   & 0.2  & -0.004        & 0.15 & 0.107              & -0.597        & -0.036  & -0.006 & 0.497    & 1.008                   & -0.152 & -0.026 & 0.91    \\
KM\_Mod   & $G_\beta$ & 3 & 5     & 0.8   & 0.2  & 0.03          & 0.15 & 0.097              & -0.613        & 0.307   & 0.049  & 0.5      & 1.038                   & 1.184  & 0.199  & 0.378   \\
KM\_Med & $G_\beta$ & 3 & 5     & 0.8   & 0.2  & 0.033         & 0.15 & 0.103              & -0.503        & 0.325   & 0.066  & 0.508    & 1.007                   & 1.327  & 0.223  & 0.324   \\
SP\_Mod   & $G_\beta$ & 3 & 5     & 0.8   & 0.2  & 0.033         & 0.15 & 0.098              & -0.484        & 0.333   & 0.067  & 0.497    & 1.054                   & 1.294  & 0.217  & 0.335   \\
SP\_Med  & $G_\beta$ & 3 & 5     & 0.8   & 0.2  & 0.014         & 0.15 & 0.1                & -0.563        & 0.137   & 0.024  & 0.496    & 1.035                   & 0.542  & 0.091  & 0.687   \\
KM\_Mod   & $G_\beta$ & 3 & 7     & 0.8   & 0.2  & 0.096         & 0.15 & 0.104              & -0.233        & 0.92    & 0.412  & 0.518    & 1.042                   & 3.807  & 0.64   & 0.005   \\
KM\_Med & $G_\beta$ & 3 & 7     & 0.8   & 0.2  & 0.089         & 0.15 & 0.102              & -0.262        & 0.868   & 0.338  & 0.516    & 1.042                   & 3.515  & 0.591  & 0.009   \\
SP\_Mod   & $G_\beta$ & 3 & 7     & 0.8   & 0.2  & 0.061         & 0.15 & 0.106              & -0.359        & 0.572   & 0.169  & 0.513    & 1.021                   & 2.404  & 0.404  & 0.074   \\
SP\_Med  & $G_\beta$ & 3 & 7     & 0.8   & 0.2  & 0.048         & 0.15 & 0.109              & -0.438        & 0.442   & 0.11   & 0.513    & 1.004                   & 1.907  & 0.32   & 0.157   \\
KM\_Mod   & $G_\beta$ & 5 & 1     & 0.8   & 0.2  & -0.037        & 0.15 & 0.107              & -0.729        & -0.343  & -0.05  & 0.496    & 0.971                   & -1.458 & -0.245 & 0.279   \\
KM\_Med & $G_\beta$ & 5 & 1     & 0.8   & 0.2  & -0.003        & 0.15 & 0.107              & -0.708        & -0.032  & -0.005 & 0.497    & 1.01                    & -0.138 & -0.023 & 0.918   \\
SP\_Mod   & $G_\beta$ & 5 & 1     & 0.8   & 0.2  & -0.038        & 0.15 & 0.107              & -0.836        & -0.36   & -0.046 & 0.494    & 0.979                   & -1.525 & -0.256 & 0.258   \\
SP\_Med  & $G_\beta$ & 5 & 1     & 0.8   & 0.2  & -0.073        & 0.15 & 0.11               & -0.855        & -0.663  & -0.085 & 0.486    & 0.966                   & -2.891 & -0.486 & 0.032   \\
KM\_Mod   & $G_\beta$ & 5 & 3     & 0.8   & 0.2  & 0.002         & 0.15 & 0.101              & -0.579        & 0.017   & 0.003  & 0.499    & 1.007                   & 0.067  & 0.011  & 0.961   \\
KM\_Med & $G_\beta$ & 5 & 3     & 0.8   & 0.2  & 0.007         & 0.15 & 0.105              & -0.565        & 0.069   & 0.013  & 0.504    & 0.992                   & 0.289  & 0.048  & 0.83    \\
SP\_Mod   & $G_\beta$ & 5 & 3     & 0.8   & 0.2  & 0.023         & 0.15 & 0.104              & -0.463        & 0.219   & 0.049  & 0.5      & 1.028                   & 0.905  & 0.152  & 0.501   \\
SP\_Med  & $G_\beta$ & 5 & 3     & 0.8   & 0.2  & 0.032         & 0.15 & 0.106              & -0.524        & 0.3     & 0.06   & 0.499    & 1.042                   & 1.255  & 0.211  & 0.351   \\
KM\_Mod   & $G_\beta$ & 5 & 5     & 0.8   & 0.2  & 0.09          & 0.15 & 0.101              & -0.402        & 0.891   & 0.224  & 0.518    & 1.036                   & 3.579  & 0.601  & 0.008   \\
KM\_Med & $G_\beta$ & 5 & 5     & 0.8   & 0.2  & 0.103         & 0.15 & 0.104              & -0.325        & 0.983   & 0.315  & 0.52     & 1.042                   & 4.068  & 0.683  & 0.003   \\
SP\_Mod   & $G_\beta$ & 5 & 5     & 0.8   & 0.2  & 0.066         & 0.15 & 0.1                & -0.372        & 0.665   & 0.178  & 0.499    & 1.086                   & 2.629  & 0.442  & 0.05    \\
SP\_Med  & $G_\beta$ & 5 & 5     & 0.8   & 0.2  & 0.029         & 0.15 & 0.103              & -0.489        & 0.287   & 0.06   & 0.498    & 1.045                   & 1.169  & 0.196  & 0.384   \\
KM\_Mod   & $G_\beta$ & 5 & 7     & 0.8   & 0.2  & 0.121         & 0.15 & 0.103              & -0.211        & 1.174   & 0.573  & 0.517    & 1.08                    & 4.801  & 0.807  & 0       \\
KM\_Med & $G_\beta$ & 5 & 7     & 0.8   & 0.2  & 0.093         & 0.15 & 0.1                & -0.273        & 0.926   & 0.339  & 0.511    & 1.069                   & 3.673  & 0.617  & 0.006   \\
SP\_Mod   & $G_\beta$ & 5 & 7     & 0.8   & 0.2  & 0.094         & 0.15 & 0.103              & -0.219        & 0.913   & 0.429  & 0.515    & 1.051                   & 3.729  & 0.626  & 0.005   \\
SP\_Med  & $G_\beta$ & 5 & 7     & 0.8   & 0.2  & 0.072         & 0.15 & 0.106              & -0.326        & 0.68    & 0.222  & 0.515    & 1.029                   & 2.871  & 0.482  & 0.033   \\
KM\_Mod   & $G_\beta$ & 7 & 1     & 0.8   & 0.2  & -0.031        & 0.15 & 0.106              & -0.708        & -0.298  & -0.044 & 0.494    & 0.987                   & -1.247 & -0.209 & 0.355   \\
KM\_Med & $G_\beta$ & 7 & 1     & 0.8   & 0.2  & 0.007         & 0.15 & 0.107              & -0.586        & 0.061   & 0.011  & 0.498    & 1.015                   & 0.258  & 0.043  & 0.848   \\
SP\_Mod   & $G_\beta$ & 7 & 1     & 0.8   & 0.2  & -0.01         & 0.15 & 0.107              & -0.65         & -0.095  & -0.016 & 0.499    & 0.991                   & -0.406 & -0.068 & 0.763   \\
SP\_Med  & $G_\beta$ & 7 & 1     & 0.8   & 0.2  & -0.04         & 0.15 & 0.109              & -0.684        & -0.364  & -0.058 & 0.491    & 0.989                   & -1.57  & -0.264 & 0.243   \\
KM\_Mod   & $G_\beta$ & 7 & 3     & 0.8   & 0.2  & 0.037         & 0.15 & 0.101              & -0.455        & 0.367   & 0.082  & 0.506    & 1.021                   & 1.476  & 0.248  & 0.272   \\
KM\_Med & $G_\beta$ & 7 & 3     & 0.8   & 0.2  & 0.03          & 0.15 & 0.105              & -0.492        & 0.287   & 0.061  & 0.508    & 1.002                   & 1.191  & 0.2    & 0.376   \\
SP\_Mod   & $G_\beta$ & 7 & 3     & 0.8   & 0.2  & 0.061         & 0.15 & 0.104              & -0.345        & 0.581   & 0.176  & 0.514    & 1.017                   & 2.408  & 0.405  & 0.073   \\
SP\_Med  & $G_\beta$ & 7 & 3     & 0.8   & 0.2  & 0.047         & 0.15 & 0.106              & -0.417        & 0.443   & 0.113  & 0.501    & 1.053                   & 1.863  & 0.313  & 0.166   \\
KM\_Mod   & $G_\beta$ & 7 & 5     & 0.8   & 0.2  & 0.051         & 0.15 & 0.102              & -0.451        & 0.5     & 0.113  & 0.508    & 1.028                   & 2.03   & 0.341  & 0.131   \\
KM\_Med & $G_\beta$ & 7 & 5     & 0.8   & 0.2  & 0.045         & 0.15 & 0.105              & -0.489        & 0.43    & 0.092  & 0.513    & 1.001                   & 1.794  & 0.301  & 0.183   \\
SP\_Mod   & $G_\beta$ & 7 & 5     & 0.8   & 0.2  & 0.061         & 0.15 & 0.102              & -0.294        & 0.595   & 0.206  & 0.502    & 1.067                   & 2.408  & 0.405  & 0.072   \\
SP\_Med  & $G_\beta$ & 7 & 5     & 0.8   & 0.2  & 0.031         & 0.15 & 0.105              & -0.415        & 0.299   & 0.076  & 0.502    & 1.029                   & 1.244  & 0.209  & 0.355   \\
KM\_Mod   & $G_\beta$ & 7 & 7     & 0.8   & 0.2  & 0.117         & 0.15 & 0.103              & -0.236        & 1.137   & 0.494  & 0.516    & 1.078                   & 4.63   & 0.778  & 0.001   \\
KM\_Med & $G_\beta$ & 7 & 7     & 0.8   & 0.2  & 0.121         & 0.15 & 0.099              & -0.22         & 1.225   & 0.549  & 0.509    & 1.113                   & 4.796  & 0.806  & 0       \\
SP\_Mod   & $G_\beta$ & 7 & 7     & 0.8   & 0.2  & 0.129         & 0.15 & 0.103              & -0.206        & 1.258   & 0.628  & 0.522    & 1.069                   & 5.135  & 0.863  & 0       \\
SP\_Med  & $G_\beta$ & 7 & 7     & 0.8   & 0.2  & 0.098         & 0.15 & 0.106              & -0.271        & 0.927   & 0.363  & 0.518    & 1.046                   & 3.904  & 0.656  & 0.004   \\
KM\_Mod   & $G_\beta$ & 1 & 1     & 0.75  & 0.25 & -0.036        & 0.15 & 0.108              & -0.781        & -0.334  & -0.046 & 0.497    & 0.971                   & -1.432 & -0.241 & 0.287   \\
KM\_Med & $G_\beta$ & 1 & 1     & 0.75  & 0.25 & -0.03         & 0.15 & 0.108              & -0.743        & -0.281  & -0.041 & 0.496    & 0.981                   & -1.199 & -0.201 & 0.374   \\
SP\_Mod   & $G_\beta$ & 1 & 1     & 0.75  & 0.25 & -0.051        & 0.15 & 0.109              & -0.82         & -0.468  & -0.062 & 0.496    & 0.958                   & -2.017 & -0.339 & 0.134   \\
SP\_Med  & $G_\beta$ & 1 & 1     & 0.75  & 0.25 & -0.107        & 0.15 & 0.11               & -0.918        & -0.977  & -0.117 & 0.488    & 0.923                   & -4.247 & -0.713 & 0.002   \\
KM\_Mod   & $G_\beta$ & 1 & 3     & 0.75  & 0.25 & -0.045        & 0.15 & 0.105              & -0.737        & -0.428  & -0.061 & 0.482    & 1.022                   & -1.779 & -0.299 & 0.186   \\
KM\_Med & $G_\beta$ & 1 & 3     & 0.75  & 0.25 & -0.05         & 0.15 & 0.112              & -0.764        & -0.447  & -0.066 & 0.492    & 0.973                   & -1.992 & -0.335 & 0.137   \\
SP\_Mod   & $G_\beta$ & 1 & 3     & 0.75  & 0.25 & -0.03         & 0.15 & 0.111              & -0.655        & -0.271  & -0.046 & 0.495    & 0.986                   & -1.194 & -0.201 & 0.374   \\
SP\_Med  & $G_\beta$ & 1 & 3     & 0.75  & 0.25 & -0.026        & 0.15 & 0.108              & -0.7          & -0.243  & -0.037 & 0.495    & 0.987                   & -1.041 & -0.175 & 0.439   \\
KM\_Mod   & $G_\beta$ & 1 & 5     & 0.75  & 0.25 & 0.001         & 0.15 & 0.103              & -0.636        & 0.012   & 0.002  & 0.496    & 1.017                   & 0.05   & 0.008  & 0.971   \\
KM\_Med & $G_\beta$ & 1 & 5     & 0.75  & 0.25 & 0.009         & 0.15 & 0.102              & -0.623        & 0.088   & 0.014  & 0.497    & 1.022                   & 0.358  & 0.06   & 0.79    \\
SP\_Mod   & $G_\beta$ & 1 & 5     & 0.75  & 0.25 & 0.023         & 0.15 & 0.104              & -0.683        & 0.226   & 0.034  & 0.502    & 1.019                   & 0.931  & 0.156  & 0.489   \\
SP\_Med  & $G_\beta$ & 1 & 5     & 0.75  & 0.25 & 0.017         & 0.15 & 0.102              & -0.689        & 0.165   & 0.025  & 0.497    & 1.033                   & 0.671  & 0.113  & 0.618   \\
KM\_Mod   & $G_\beta$ & 1 & 7     & 0.75  & 0.25 & 0.085         & 0.15 & 0.102              & -0.31         & 0.834   & 0.275  & 0.515    & 1.043                   & 3.382  & 0.568  & 0.012   \\
KM\_Med & $G_\beta$ & 1 & 7     & 0.75  & 0.25 & 0.054         & 0.15 & 0.104              & -0.275        & 0.519   & 0.196  & 0.512    & 1.018                   & 2.137  & 0.359  & 0.111   \\
SP\_Mod   & $G_\beta$ & 1 & 7     & 0.75  & 0.25 & 0.053         & 0.15 & 0.107              & -0.373        & 0.497   & 0.142  & 0.51     & 1.025                   & 2.1    & 0.353  & 0.119   \\
SP\_Med  & $G_\beta$ & 1 & 7     & 0.75  & 0.25 & 0.023         & 0.15 & 0.11               & -0.47         & 0.212   & 0.049  & 0.509    & 0.994                   & 0.922  & 0.155  & 0.494   \\
KM\_Mod   & $G_\beta$ & 3 & 1     & 0.75  & 0.25 & -0.012        & 0.15 & 0.107              & -0.645        & -0.111  & -0.018 & 0.5      & 0.985                   & -0.468 & -0.079 & 0.728   \\
KM\_Med & $G_\beta$ & 3 & 1     & 0.75  & 0.25 & 0.002         & 0.15 & 0.108              & -0.597        & 0.021   & 0.004  & 0.505    & 0.983                   & 0.088  & 0.015  & 0.948   \\
SP\_Mod   & $G_\beta$ & 3 & 1     & 0.75  & 0.25 & -0.019        & 0.15 & 0.111              & -0.686        & -0.167  & -0.027 & 0.509    & 0.945                   & -0.735 & -0.123 & 0.585   \\
SP\_Med  & $G_\beta$ & 3 & 1     & 0.75  & 0.25 & -0.058        & 0.15 & 0.11               & -0.81         & -0.532  & -0.072 & 0.497    & 0.942                   & -2.32  & -0.39  & 0.085   \\
KM\_Mod   & $G_\beta$ & 3 & 3     & 0.75  & 0.25 & -0.005        & 0.15 & 0.103              & -0.537        & -0.049  & -0.009 & 0.497    & 1.008                   & -0.201 & -0.034 & 0.882   \\
KM\_Med & $G_\beta$ & 3 & 3     & 0.75  & 0.25 & -0.022        & 0.15 & 0.107              & -0.551        & -0.209  & -0.041 & 0.495    & 0.993                   & -0.89  & -0.15  & 0.508   \\
SP\_Mod   & $G_\beta$ & 3 & 3     & 0.75  & 0.25 & -0.026        & 0.15 & 0.109              & -0.664        & -0.243  & -0.04  & 0.497    & 0.982                   & -1.05  & -0.176 & 0.435   \\
SP\_Med  & $G_\beta$ & 3 & 3     & 0.75  & 0.25 & 0.008         & 0.15 & 0.106              & -0.5          & 0.079   & 0.017  & 0.501    & 1.005                   & 0.334  & 0.056  & 0.804   \\
KM\_Mod   & $G_\beta$ & 3 & 5     & 0.75  & 0.25 & 0.021         & 0.15 & 0.098              & -0.563        & 0.217   & 0.038  & 0.495    & 1.047                   & 0.848  & 0.142  & 0.528   \\
KM\_Med & $G_\beta$ & 3 & 5     & 0.75  & 0.25 & 0.049         & 0.15 & 0.1                & -0.495        & 0.487   & 0.099  & 0.503    & 1.048                   & 1.937  & 0.325  & 0.149   \\
SP\_Mod   & $G_\beta$ & 3 & 5     & 0.75  & 0.25 & 0.021         & 0.15 & 0.098              & -0.592        & 0.212   & 0.035  & 0.497    & 1.038                   & 0.829  & 0.139  & 0.537   \\
SP\_Med  & $G_\beta$ & 3 & 5     & 0.75  & 0.25 & -0.005        & 0.15 & 0.101              & -0.662        & -0.05   & -0.008 & 0.49     & 1.035                   & -0.201 & -0.034 & 0.881   \\
KM\_Mod   & $G_\beta$ & 3 & 7     & 0.75  & 0.25 & 0.107         & 0.15 & 0.101              & -0.214        & 1.057   & 0.5    & 0.52     & 1.048                   & 4.244  & 0.713  & 0.001   \\
KM\_Med & $G_\beta$ & 3 & 7     & 0.75  & 0.25 & 0.077         & 0.15 & 0.103              & -0.267        & 0.74    & 0.287  & 0.517    & 1.025                   & 3.037  & 0.51   & 0.024   \\
SP\_Mod   & $G_\beta$ & 3 & 7     & 0.75  & 0.25 & 0.047         & 0.15 & 0.106              & -0.375        & 0.441   & 0.125  & 0.506    & 1.033                   & 1.854  & 0.311  & 0.168   \\
SP\_Med  & $G_\beta$ & 3 & 7     & 0.75  & 0.25 & 0.045         & 0.15 & 0.109              & -0.432        & 0.413   & 0.104  & 0.511    & 1.009                   & 1.782  & 0.299  & 0.186   \\
KM\_Mod   & $G_\beta$ & 5 & 1     & 0.75  & 0.25 & -0.029        & 0.15 & 0.108              & -0.708        & -0.271  & -0.041 & 0.499    & 0.97                    & -1.16  & -0.195 & 0.389   \\
KM\_Med & $G_\beta$ & 5 & 1     & 0.75  & 0.25 & 0.001         & 0.15 & 0.105              & -0.604        & 0.007   & 0.001  & 0.499    & 1.004                   & 0.03   & 0.005  & 0.982   \\
SP\_Mod   & $G_\beta$ & 5 & 1     & 0.75  & 0.25 & -0.035        & 0.15 & 0.107              & -0.796        & -0.324  & -0.044 & 0.496    & 0.976                   & -1.38  & -0.232 & 0.306   \\
SP\_Med  & $G_\beta$ & 5 & 1     & 0.75  & 0.25 & -0.085        & 0.15 & 0.109              & -0.881        & -0.782  & -0.097 & 0.49     & 0.94                    & -3.391 & -0.57  & 0.012   \\
KM\_Mod   & $G_\beta$ & 5 & 3     & 0.75  & 0.25 & 0.007         & 0.15 & 0.101              & -0.55         & 0.07    & 0.013  & 0.499    & 1.014                   & 0.28   & 0.047  & 0.835   \\
KM\_Med & $G_\beta$ & 5 & 3     & 0.75  & 0.25 & 0.001         & 0.15 & 0.107              & -0.465        & 0.014   & 0.003  & 0.499    & 1.005                   & 0.058  & 0.01   & 0.966   \\
SP\_Mod   & $G_\beta$ & 5 & 3     & 0.75  & 0.25 & -0.003        & 0.15 & 0.105              & -0.557        & -0.028  & -0.005 & 0.499    & 1                       & -0.117 & -0.02  & 0.931   \\
SP\_Med  & $G_\beta$ & 5 & 3     & 0.75  & 0.25 & 0.028         & 0.15 & 0.104              & -0.558        & 0.264   & 0.049  & 0.502    & 1.025                   & 1.093  & 0.184  & 0.417   \\
KM\_Mod   & $G_\beta$ & 5 & 5     & 0.75  & 0.25 & 0.1           & 0.15 & 0.102              & -0.271        & 0.983   & 0.369  & 0.511    & 1.077                   & 3.972  & 0.667  & 0.003   \\
KM\_Med & $G_\beta$ & 5 & 5     & 0.75  & 0.25 & 0.117         & 0.15 & 0.099              & -0.313        & 1.19    & 0.375  & 0.52     & 1.063                   & 4.656  & 0.782  & 0       \\
SP\_Mod   & $G_\beta$ & 5 & 5     & 0.75  & 0.25 & 0.059         & 0.15 & 0.099              & -0.363        & 0.598   & 0.163  & 0.502    & 1.067                   & 2.353  & 0.395  & 0.079   \\
SP\_Med  & $G_\beta$ & 5 & 5     & 0.75  & 0.25 & 0.029         & 0.15 & 0.103              & -0.409        & 0.283   & 0.071  & 0.497    & 1.049                   & 1.158  & 0.195  & 0.389   \\
KM\_Mod   & $G_\beta$ & 5 & 7     & 0.75  & 0.25 & 0.109         & 0.15 & 0.103              & -0.19         & 1.056   & 0.572  & 0.516    & 1.067                   & 4.311  & 0.724  & 0.001   \\
KM\_Med & $G_\beta$ & 5 & 7     & 0.75  & 0.25 & 0.092         & 0.15 & 0.102              & -0.249        & 0.9     & 0.367  & 0.51     & 1.075                   & 3.631  & 0.61   & 0.007   \\
SP\_Mod   & $G_\beta$ & 5 & 7     & 0.75  & 0.25 & 0.112         & 0.15 & 0.102              & -0.277        & 1.098   & 0.405  & 0.514    & 1.082                   & 4.453  & 0.748  & 0.001   \\
SP\_Med  & $G_\beta$ & 5 & 7     & 0.75  & 0.25 & 0.089         & 0.15 & 0.106              & -0.428        & 0.842   & 0.208  & 0.518    & 1.035                   & 3.526  & 0.592  & 0.009   \\
KM\_Mod   & $G_\beta$ & 7 & 1     & 0.75  & 0.25 & -0.03         & 0.15 & 0.107              & -0.665        & -0.279  & -0.045 & 0.497    & 0.978                   & -1.18  & -0.198 & 0.381   \\
KM\_Med & $G_\beta$ & 7 & 1     & 0.75  & 0.25 & 0.011         & 0.15 & 0.106              & -0.601        & 0.103   & 0.018  & 0.502    & 1.004                   & 0.434  & 0.073  & 0.747   \\
SP\_Mod   & $G_\beta$ & 7 & 1     & 0.75  & 0.25 & -0.013        & 0.15 & 0.108              & -0.622        & -0.118  & -0.02  & 0.501    & 0.979                   & -0.505 & -0.085 & 0.708   \\
SP\_Med  & $G_\beta$ & 7 & 1     & 0.75  & 0.25 & -0.042        & 0.15 & 0.108              & -0.733        & -0.386  & -0.057 & 0.497    & 0.963                   & -1.659 & -0.279 & 0.218   \\
KM\_Mod   & $G_\beta$ & 7 & 3     & 0.75  & 0.25 & 0.065         & 0.15 & 0.1                & -0.414        & 0.643   & 0.156  & 0.51     & 1.035                   & 2.562  & 0.43   & 0.056   \\
KM\_Med & $G_\beta$ & 7 & 3     & 0.75  & 0.25 & 0.033         & 0.15 & 0.106              & -0.425        & 0.311   & 0.078  & 0.508    & 1.006                   & 1.311  & 0.22   & 0.33    \\
SP\_Mod   & $G_\beta$ & 7 & 3     & 0.75  & 0.25 & 0.042         & 0.15 & 0.105              & -0.453        & 0.396   & 0.092  & 0.509    & 1.014                   & 1.647  & 0.277  & 0.22    \\
SP\_Med  & $G_\beta$ & 7 & 3     & 0.75  & 0.25 & 0.046         & 0.15 & 0.105              & -0.396        & 0.441   & 0.117  & 0.502    & 1.05                    & 1.835  & 0.308  & 0.173   \\
KM\_Mod   & $G_\beta$ & 7 & 5     & 0.75  & 0.25 & 0.047         & 0.15 & 0.102              & -0.441        & 0.457   & 0.106  & 0.507    & 1.028                   & 1.852  & 0.311  & 0.168   \\
KM\_Med & $G_\beta$ & 7 & 5     & 0.75  & 0.25 & 0.046         & 0.15 & 0.105              & -0.486        & 0.434   & 0.094  & 0.508    & 1.023                   & 1.81   & 0.304  & 0.179   \\
SP\_Mod   & $G_\beta$ & 7 & 5     & 0.75  & 0.25 & 0.061         & 0.15 & 0.102              & -0.33         & 0.599   & 0.184  & 0.506    & 1.048                   & 2.416  & 0.406  & 0.072   \\
SP\_Med  & $G_\beta$ & 7 & 5     & 0.75  & 0.25 & 0.025         & 0.15 & 0.106              & -0.453        & 0.238   & 0.056  & 0.502    & 1.023                   & 0.998  & 0.168  & 0.459   \\
KM\_Mod   & $G_\beta$ & 7 & 7     & 0.75  & 0.25 & 0.126         & 0.15 & 0.103              & -0.26         & 1.222   & 0.484  & 0.521    & 1.068                   & 4.996  & 0.839  & 0       \\
KM\_Med & $G_\beta$ & 7 & 7     & 0.75  & 0.25 & 0.118         & 0.15 & 0.101              & -0.215        & 1.166   & 0.548  & 0.51     & 1.107                   & 4.672  & 0.785  & 0       \\
SP\_Mod   & $G_\beta$ & 7 & 7     & 0.75  & 0.25 & 0.127         & 0.15 & 0.103              & -0.214        & 1.237   & 0.594  & 0.516    & 1.091                   & 5.041  & 0.847  & 0       \\
SP\_Med  & $G_\beta$ & 7 & 7     & 0.75  & 0.25 & 0.104         & 0.15 & 0.105              & -0.287        & 0.988   & 0.362  & 0.519    & 1.051                   & 4.119  & 0.692  & 0.002   \\
KM\_Mod   & $G_\beta$ & 1 & 1     & 0.7   & 0.3  & -0.042        & 0.15 & 0.109              & -0.785        & -0.388  & -0.054 & 0.496    & 0.968                   & -1.68  & -0.282 & 0.211   \\
KM\_Med & $G_\beta$ & 1 & 1     & 0.7   & 0.3  & -0.029        & 0.15 & 0.108              & -0.694        & -0.267  & -0.041 & 0.494    & 0.99                    & -1.141 & -0.192 & 0.397   \\
SP\_Mod   & $G_\beta$ & 1 & 1     & 0.7   & 0.3  & -0.051        & 0.15 & 0.109              & -0.81         & -0.47   & -0.063 & 0.496    & 0.957                   & -2.03  & -0.341 & 0.132   \\
SP\_Med  & $G_\beta$ & 1 & 1     & 0.7   & 0.3  & -0.103        & 0.15 & 0.11               & -0.913        & -0.935  & -0.113 & 0.488    & 0.925                   & -4.093 & -0.688 & 0.002   \\
KM\_Mod   & $G_\beta$ & 1 & 3     & 0.7   & 0.3  & -0.054        & 0.15 & 0.106              & -0.768        & -0.507  & -0.07  & 0.487    & 0.988                   & -2.141 & -0.36  & 0.112   \\
KM\_Med & $G_\beta$ & 1 & 3     & 0.7   & 0.3  & -0.051        & 0.15 & 0.114              & -0.775        & -0.45   & -0.066 & 0.492    & 0.97                    & -2.031 & -0.341 & 0.129   \\
SP\_Mod   & $G_\beta$ & 1 & 3     & 0.7   & 0.3  & -0.029        & 0.15 & 0.111              & -0.66         & -0.264  & -0.044 & 0.494    & 0.989                   & -1.157 & -0.194 & 0.39    \\
SP\_Med  & $G_\beta$ & 1 & 3     & 0.7   & 0.3  & -0.032        & 0.15 & 0.108              & -0.734        & -0.3    & -0.044 & 0.485    & 1.02                    & -1.282 & -0.215 & 0.341   \\
KM\_Mod   & $G_\beta$ & 1 & 5     & 0.7   & 0.3  & -0.017        & 0.15 & 0.103              & -0.753        & -0.163  & -0.022 & 0.492    & 1.013                   & -0.67  & -0.112 & 0.619   \\
KM\_Med & $G_\beta$ & 1 & 5     & 0.7   & 0.3  & 0.008         & 0.15 & 0.104              & -0.642        & 0.077   & 0.012  & 0.497    & 1.021                   & 0.316  & 0.053  & 0.814   \\
SP\_Mod   & $G_\beta$ & 1 & 5     & 0.7   & 0.3  & 0.007         & 0.15 & 0.104              & -0.718        & 0.066   & 0.01   & 0.499    & 1.011                   & 0.272  & 0.046  & 0.84    \\
SP\_Med  & $G_\beta$ & 1 & 5     & 0.7   & 0.3  & 0.013         & 0.15 & 0.102              & -0.7          & 0.129   & 0.019  & 0.494    & 1.043                   & 0.522  & 0.088  & 0.698   \\
KM\_Mod   & $G_\beta$ & 1 & 7     & 0.7   & 0.3  & 0.09          & 0.15 & 0.103              & -0.284        & 0.879   & 0.318  & 0.514    & 1.052                   & 3.588  & 0.603  & 0.008   \\
KM\_Med & $G_\beta$ & 1 & 7     & 0.7   & 0.3  & 0.052         & 0.15 & 0.107              & -0.284        & 0.481   & 0.182  & 0.513    & 1.01                    & 2.05   & 0.344  & 0.128   \\
SP\_Mod   & $G_\beta$ & 1 & 7     & 0.7   & 0.3  & 0.053         & 0.15 & 0.107              & -0.367        & 0.496   & 0.145  & 0.517    & 0.996                   & 2.108  & 0.354  & 0.117   \\
SP\_Med  & $G_\beta$ & 1 & 7     & 0.7   & 0.3  & 0.038         & 0.15 & 0.11               & -0.415        & 0.343   & 0.091  & 0.51     & 1.006                   & 1.493  & 0.251  & 0.268   \\
KM\_Mod   & $G_\beta$ & 3 & 1     & 0.7   & 0.3  & -0.013        & 0.15 & 0.108              & -0.625        & -0.119  & -0.021 & 0.506    & 0.963                   & -0.511 & -0.086 & 0.704   \\
KM\_Med & $G_\beta$ & 3 & 1     & 0.7   & 0.3  & -0.01         & 0.15 & 0.108              & -0.595        & -0.094  & -0.017 & 0.503    & 0.976                   & -0.404 & -0.068 & 0.764   \\
SP\_Mod   & $G_\beta$ & 3 & 1     & 0.7   & 0.3  & -0.024        & 0.15 & 0.111              & -0.714        & -0.213  & -0.033 & 0.509    & 0.939                   & -0.941 & -0.158 & 0.484   \\
SP\_Med  & $G_\beta$ & 3 & 1     & 0.7   & 0.3  & -0.051        & 0.15 & 0.11               & -0.785        & -0.459  & -0.064 & 0.498    & 0.95                    & -2.005 & -0.337 & 0.136   \\
KM\_Mod   & $G_\beta$ & 3 & 3     & 0.7   & 0.3  & 0.01          & 0.15 & 0.102              & -0.428        & 0.096   & 0.023  & 0.5      & 1.011                   & 0.389  & 0.065  & 0.773   \\
KM\_Med & $G_\beta$ & 3 & 3     & 0.7   & 0.3  & -0.014        & 0.15 & 0.108              & -0.509        & -0.133  & -0.028 & 0.499    & 0.988                   & -0.57  & -0.096 & 0.672   \\
SP\_Mod   & $G_\beta$ & 3 & 3     & 0.7   & 0.3  & -0.023        & 0.15 & 0.109              & -0.618        & -0.211  & -0.037 & 0.494    & 0.995                   & -0.91  & -0.153 & 0.499   \\
SP\_Med  & $G_\beta$ & 3 & 3     & 0.7   & 0.3  & -0.003        & 0.15 & 0.106              & -0.592        & -0.024  & -0.004 & 0.497    & 1.008                   & -0.102 & -0.017 & 0.94    \\
KM\_Mod   & $G_\beta$ & 3 & 5     & 0.7   & 0.3  & 0.026         & 0.15 & 0.099              & -0.564        & 0.268   & 0.047  & 0.5      & 1.03                    & 1.048  & 0.176  & 0.435   \\
KM\_Med & $G_\beta$ & 3 & 5     & 0.7   & 0.3  & 0.049         & 0.15 & 0.101              & -0.502        & 0.482   & 0.097  & 0.507    & 1.032                   & 1.93   & 0.324  & 0.15    \\
SP\_Mod   & $G_\beta$ & 3 & 5     & 0.7   & 0.3  & 0.028         & 0.15 & 0.099              & -0.541        & 0.281   & 0.052  & 0.5      & 1.036                   & 1.109  & 0.186  & 0.409   \\
SP\_Med  & $G_\beta$ & 3 & 5     & 0.7   & 0.3  & 0.001         & 0.15 & 0.102              & -0.636        & 0.007   & 0.001  & 0.495    & 1.021                   & 0.029  & 0.005  & 0.983   \\
KM\_Mod   & $G_\beta$ & 3 & 7     & 0.7   & 0.3  & 0.104         & 0.15 & 0.102              & -0.221        & 1.025   & 0.473  & 0.522    & 1.038                   & 4.147  & 0.697  & 0.002   \\
KM\_Med & $G_\beta$ & 3 & 7     & 0.7   & 0.3  & 0.068         & 0.15 & 0.108              & -0.328        & 0.635   & 0.208  & 0.519    & 1.006                   & 2.712  & 0.456  & 0.044   \\
SP\_Mod   & $G_\beta$ & 3 & 7     & 0.7   & 0.3  & 0.063         & 0.15 & 0.106              & -0.34         & 0.589   & 0.184  & 0.513    & 1.025                   & 2.482  & 0.417  & 0.065   \\
SP\_Med  & $G_\beta$ & 3 & 7     & 0.7   & 0.3  & 0.048         & 0.15 & 0.11               & -0.434        & 0.44    & 0.111  & 0.513    & 1.008                   & 1.918  & 0.322  & 0.155   \\
KM\_Mod   & $G_\beta$ & 5 & 1     & 0.7   & 0.3  & -0.029        & 0.15 & 0.109              & -0.704        & -0.266  & -0.041 & 0.502    & 0.958                   & -1.15  & -0.193 & 0.393   \\
KM\_Med & $G_\beta$ & 5 & 1     & 0.7   & 0.3  & -0.007        & 0.15 & 0.106              & -0.61         & -0.066  & -0.011 & 0.504    & 0.976                   & -0.275 & -0.046 & 0.838   \\
SP\_Mod   & $G_\beta$ & 5 & 1     & 0.7   & 0.3  & -0.023        & 0.15 & 0.107              & -0.732        & -0.213  & -0.031 & 0.499    & 0.976                   & -0.907 & -0.152 & 0.501   \\
SP\_Med  & $G_\beta$ & 5 & 1     & 0.7   & 0.3  & -0.073        & 0.15 & 0.11               & -0.858        & -0.668  & -0.086 & 0.492    & 0.944                   & -2.913 & -0.489 & 0.03    \\
KM\_Mod   & $G_\beta$ & 5 & 3     & 0.7   & 0.3  & 0.01          & 0.15 & 0.1                & -0.526        & 0.096   & 0.018  & 0.501    & 1.009                   & 0.382  & 0.064  & 0.777   \\
KM\_Med & $G_\beta$ & 5 & 3     & 0.7   & 0.3  & -0.008        & 0.15 & 0.109              & -0.538        & -0.077  & -0.016 & 0.5      & 0.99                    & -0.334 & -0.056 & 0.804   \\
SP\_Mod   & $G_\beta$ & 5 & 3     & 0.7   & 0.3  & 0.007         & 0.15 & 0.105              & -0.515        & 0.07    & 0.014  & 0.497    & 1.02                    & 0.294  & 0.049  & 0.827   \\
SP\_Med  & $G_\beta$ & 5 & 3     & 0.7   & 0.3  & 0.034         & 0.15 & 0.105              & -0.527        & 0.327   & 0.065  & 0.504    & 1.026                   & 1.363  & 0.229  & 0.311   \\
KM\_Mod   & $G_\beta$ & 5 & 5     & 0.7   & 0.3  & 0.101         & 0.15 & 0.1                & -0.287        & 1.005   & 0.35   & 0.514    & 1.064                   & 3.991  & 0.671  & 0.003   \\
KM\_Med & $G_\beta$ & 5 & 5     & 0.7   & 0.3  & 0.129         & 0.15 & 0.098              & -0.273        & 1.314   & 0.473  & 0.519    & 1.083                   & 5.127  & 0.861  & 0       \\
SP\_Mod   & $G_\beta$ & 5 & 5     & 0.7   & 0.3  & 0.058         & 0.15 & 0.099              & -0.302        & 0.586   & 0.193  & 0.498    & 1.079                   & 2.313  & 0.389  & 0.084   \\
SP\_Med  & $G_\beta$ & 5 & 5     & 0.7   & 0.3  & 0.053         & 0.15 & 0.103              & -0.374        & 0.513   & 0.141  & 0.504    & 1.048                   & 2.09   & 0.351  & 0.12    \\
KM\_Mod   & $G_\beta$ & 5 & 7     & 0.7   & 0.3  & 0.102         & 0.15 & 0.103              & -0.204        & 0.981   & 0.498  & 0.518    & 1.049                   & 4.028  & 0.677  & 0.003   \\
KM\_Med & $G_\beta$ & 5 & 7     & 0.7   & 0.3  & 0.09          & 0.15 & 0.105              & -0.219        & 0.853   & 0.411  & 0.516    & 1.045                   & 3.569  & 0.6    & 0.008   \\
SP\_Mod   & $G_\beta$ & 5 & 7     & 0.7   & 0.3  & 0.098         & 0.15 & 0.103              & -0.313        & 0.946   & 0.312  & 0.517    & 1.048                   & 3.874  & 0.651  & 0.004   \\
SP\_Med  & $G_\beta$ & 5 & 7     & 0.7   & 0.3  & 0.108         & 0.15 & 0.105              & -0.288        & 1.024   & 0.375  & 0.517    & 1.062                   & 4.282  & 0.719  & 0.001   \\
KM\_Mod   & $G_\beta$ & 7 & 1     & 0.7   & 0.3  & -0.023        & 0.15 & 0.107              & -0.623        & -0.213  & -0.037 & 0.499    & 0.976                   & -0.91  & -0.153 & 0.499   \\
KM\_Med & $G_\beta$ & 7 & 1     & 0.7   & 0.3  & 0.006         & 0.15 & 0.106              & -0.543        & 0.062   & 0.012  & 0.504    & 0.992                   & 0.258  & 0.043  & 0.848   \\
SP\_Mod   & $G_\beta$ & 7 & 1     & 0.7   & 0.3  & -0.019        & 0.15 & 0.108              & -0.611        & -0.173  & -0.031 & 0.498    & 0.987                   & -0.741 & -0.125 & 0.582   \\
SP\_Med  & $G_\beta$ & 7 & 1     & 0.7   & 0.3  & -0.036        & 0.15 & 0.108              & -0.69         & -0.336  & -0.053 & 0.496    & 0.973                   & -1.446 & -0.243 & 0.283   \\
KM\_Mod   & $G_\beta$ & 7 & 3     & 0.7   & 0.3  & 0.056         & 0.15 & 0.1                & -0.416        & 0.553   & 0.134  & 0.51     & 1.025                   & 2.207  & 0.371  & 0.1     \\
KM\_Med & $G_\beta$ & 7 & 3     & 0.7   & 0.3  & 0.038         & 0.15 & 0.106              & -0.428        & 0.36    & 0.089  & 0.509    & 1.012                   & 1.51   & 0.254  & 0.262   \\
SP\_Mod   & $G_\beta$ & 7 & 3     & 0.7   & 0.3  & 0.039         & 0.15 & 0.106              & -0.447        & 0.366   & 0.087  & 0.505    & 1.028                   & 1.537  & 0.258  & 0.253   \\
SP\_Med  & $G_\beta$ & 7 & 3     & 0.7   & 0.3  & 0.056         & 0.15 & 0.104              & -0.383        & 0.533   & 0.145  & 0.501    & 1.066                   & 2.205  & 0.37   & 0.101   \\
KM\_Mod   & $G_\beta$ & 7 & 5     & 0.7   & 0.3  & 0.05          & 0.15 & 0.102              & -0.411        & 0.491   & 0.122  & 0.507    & 1.033                   & 1.989  & 0.334  & 0.139   \\
KM\_Med & $G_\beta$ & 7 & 5     & 0.7   & 0.3  & 0.066         & 0.15 & 0.104              & -0.357        & 0.633   & 0.184  & 0.505    & 1.059                   & 2.602  & 0.437  & 0.053   \\
SP\_Mod   & $G_\beta$ & 7 & 5     & 0.7   & 0.3  & 0.053         & 0.15 & 0.102              & -0.379        & 0.514   & 0.139  & 0.503    & 1.05                    & 2.087  & 0.351  & 0.12    \\
SP\_Med  & $G_\beta$ & 7 & 5     & 0.7   & 0.3  & 0.038         & 0.15 & 0.106              & -0.37         & 0.363   & 0.104  & 0.504    & 1.031                   & 1.524  & 0.256  & 0.257   \\
KM\_Mod   & $G_\beta$ & 7 & 7     & 0.7   & 0.3  & 0.117         & 0.15 & 0.104              & -0.245        & 1.127   & 0.476  & 0.521    & 1.059                   & 4.628  & 0.778  & 0.001   \\
KM\_Med & $G_\beta$ & 7 & 7     & 0.7   & 0.3  & 0.115         & 0.15 & 0.103              & -0.235        & 1.115   & 0.487  & 0.517    & 1.074                   & 4.545  & 0.764  & 0.001   \\
SP\_Mod   & $G_\beta$ & 7 & 7     & 0.7   & 0.3  & 0.137         & 0.15 & 0.102              & -0.199        & 1.346   & 0.691  & 0.523    & 1.076                   & 5.456  & 0.917  & 0       \\
SP\_Med  & $G_\beta$ & 7 & 7     & 0.7   & 0.3  & 0.115         & 0.15 & 0.105              & -0.279        & 1.099   & 0.414  & 0.52     & 1.059                   & 4.579  & 0.769  & 0.001   \\
CCF              & $G_\beta$ & 1 & 1     & 0.85  & 0.15 & -0.13         & 0.15 & 0.111              & -0.952        & -1.176  & -0.137 & 0.47     & 0.968                   & -5.165 & -0.868 & 0       \\
CCF              & $G_\beta$ & 1 & 3     & 0.85  & 0.15 & -0.048        & 0.15 & 0.108              & -0.78         & -0.441  & -0.061 & 0.489    & 0.985                   & -1.897 & -0.319 & 0.159   \\
CCF              & $G_\beta$ & 1 & 5     & 0.85  & 0.15 & 0.025         & 0.15 & 0.103              & -0.637        & 0.243   & 0.039  & 0.499    & 1.035                   & 0.997  & 0.167  & 0.459   \\
CCF              & $G_\beta$ & 1 & 7     & 0.85  & 0.15 & 0.021         & 0.15 & 0.108              & -0.576        & 0.194   & 0.036  & 0.501    & 1.02                    & 0.829  & 0.139  & 0.538   \\
CCF              & $G_\beta$ & 3 & 1     & 0.85  & 0.15 & -0.104        & 0.15 & 0.11               & -0.92         & -0.944  & -0.113 & 0.478    & 0.966                   & -4.132 & -0.694 & 0.002   \\
CCF              & $G_\beta$ & 3 & 3     & 0.85  & 0.15 & 0.001         & 0.15 & 0.104              & -0.425        & 0.005   & 0.001  & 0.5      & 0.999                   & 0.021  & 0.004  & 0.988   \\
CCF              & $G_\beta$ & 3 & 5     & 0.85  & 0.15 & 0.002         & 0.15 & 0.103              & -0.586        & 0.015   & 0.003  & 0.492    & 1.032                   & 0.063  & 0.011  & 0.963   \\
CCF              & $G_\beta$ & 3 & 7     & 0.85  & 0.15 & 0.034         & 0.15 & 0.107              & -0.467        & 0.316   & 0.072  & 0.508    & 1.011                   & 1.34   & 0.225  & 0.32    \\
CCF              & $G_\beta$ & 5 & 1     & 0.85  & 0.15 & -0.085        & 0.15 & 0.112              & -0.894        & -0.763  & -0.095 & 0.485    & 0.958                   & -3.381 & -0.568 & 0.011   \\
CCF              & $G_\beta$ & 5 & 3     & 0.85  & 0.15 & -0.003        & 0.15 & 0.107              & -0.591        & -0.028  & -0.005 & 0.502    & 0.988                   & -0.117 & -0.02  & 0.931   \\
CCF              & $G_\beta$ & 5 & 5     & 0.85  & 0.15 & 0.039         & 0.15 & 0.106              & -0.353        & 0.365   & 0.11   & 0.508    & 1.015                   & 1.541  & 0.259  & 0.253   \\
CCF              & $G_\beta$ & 5 & 7     & 0.85  & 0.15 & 0.068         & 0.15 & 0.105              & -0.518        & 0.644   & 0.13   & 0.503    & 1.072                   & 2.679  & 0.45   & 0.046   \\
CCF              & $G_\beta$ & 7 & 1     & 0.85  & 0.15 & -0.055        & 0.15 & 0.107              & -0.747        & -0.512  & -0.073 & 0.484    & 1                       & -2.165 & -0.364 & 0.108   \\
CCF              & $G_\beta$ & 7 & 3     & 0.85  & 0.15 & 0.04          & 0.15 & 0.107              & -0.35         & 0.374   & 0.114  & 0.507    & 1.019                   & 1.581  & 0.266  & 0.24    \\
CCF              & $G_\beta$ & 7 & 5     & 0.85  & 0.15 & 0.031         & 0.15 & 0.107              & -0.433        & 0.292   & 0.072  & 0.499    & 1.041                   & 1.243  & 0.209  & 0.356   \\
CCF              & $G_\beta$ & 7 & 7     & 0.85  & 0.15 & 0.079         & 0.15 & 0.105              & -0.259        & 0.757   & 0.306  & 0.505    & 1.08                    & 3.143  & 0.528  & 0.02    \\
CCF              & $G_\beta$ & 1 & 1     & 0.8   & 0.2  & -0.119        & 0.15 & 0.112              & -0.934        & -1.065  & -0.128 & 0.483    & 0.927                   & -4.734 & -0.795 & 0       \\
CCF              & $G_\beta$ & 1 & 3     & 0.8   & 0.2  & -0.029        & 0.15 & 0.109              & -0.701        & -0.268  & -0.042 & 0.498    & 0.972                   & -1.159 & -0.195 & 0.389   \\
CCF              & $G_\beta$ & 1 & 5     & 0.8   & 0.2  & 0.008         & 0.15 & 0.103              & -0.706        & 0.074   & 0.011  & 0.495    & 1.03                    & 0.305  & 0.051  & 0.821   \\
CCF              & $G_\beta$ & 1 & 7     & 0.8   & 0.2  & 0.046         & 0.15 & 0.104              & -0.541        & 0.441   & 0.085  & 0.499    & 1.062                   & 1.826  & 0.307  & 0.174   \\
CCF              & $G_\beta$ & 3 & 1     & 0.8   & 0.2  & -0.095        & 0.15 & 0.111              & -0.895        & -0.854  & -0.106 & 0.485    & 0.947                   & -3.768 & -0.633 & 0.005   \\
CCF              & $G_\beta$ & 3 & 3     & 0.8   & 0.2  & 0.013         & 0.15 & 0.105              & -0.422        & 0.128   & 0.032  & 0.506    & 0.991                   & 0.532  & 0.089  & 0.693   \\
CCF              & $G_\beta$ & 3 & 5     & 0.8   & 0.2  & -0.001        & 0.15 & 0.103              & -0.593        & -0.012  & -0.002 & 0.494    & 1.021                   & -0.051 & -0.009 & 0.97    \\
CCF              & $G_\beta$ & 3 & 7     & 0.8   & 0.2  & 0.057         & 0.15 & 0.105              & -0.452        & 0.541   & 0.126  & 0.506    & 1.046                   & 2.262  & 0.38   & 0.092   \\
CCF              & $G_\beta$ & 5 & 1     & 0.8   & 0.2  & -0.076        & 0.15 & 0.112              & -0.879        & -0.683  & -0.087 & 0.489    & 0.954                   & -3.031 & -0.509 & 0.024   \\
CCF              & $G_\beta$ & 5 & 3     & 0.8   & 0.2  & -0.001        & 0.15 & 0.108              & -0.591        & -0.013  & -0.002 & 0.506    & 0.974                   & -0.057 & -0.01  & 0.966   \\
CCF              & $G_\beta$ & 5 & 5     & 0.8   & 0.2  & 0.031         & 0.15 & 0.105              & -0.404        & 0.296   & 0.077  & 0.503    & 1.027                   & 1.238  & 0.208  & 0.358   \\
CCF              & $G_\beta$ & 5 & 7     & 0.8   & 0.2  & 0.067         & 0.15 & 0.107              & -0.506        & 0.628   & 0.132  & 0.505    & 1.063                   & 2.654  & 0.446  & 0.049   \\
CCF              & $G_\beta$ & 7 & 1     & 0.8   & 0.2  & -0.059        & 0.15 & 0.11               & -0.785        & -0.542  & -0.076 & 0.488    & 0.977                   & -2.356 & -0.396 & 0.079   \\
CCF              & $G_\beta$ & 7 & 3     & 0.8   & 0.2  & 0.043         & 0.15 & 0.106              & -0.375        & 0.402   & 0.114  & 0.51     & 1.011                   & 1.698  & 0.285  & 0.207   \\
CCF              & $G_\beta$ & 7 & 5     & 0.8   & 0.2  & 0.025         & 0.15 & 0.108              & -0.443        & 0.231   & 0.056  & 0.507    & 1.002                   & 0.99   & 0.166  & 0.463   \\
CCF              & $G_\beta$ & 7 & 7     & 0.8   & 0.2  & 0.089         & 0.15 & 0.105              & -0.29         & 0.849   & 0.306  & 0.505    & 1.091                   & 3.526  & 0.592  & 0.009   \\
CCF              & $G_\beta$ & 1 & 1     & 0.75  & 0.25 & -0.125        & 0.15 & 0.112              & -0.939        & -1.108  & -0.133 & 0.479    & 0.937                   & -4.942 & -0.83  & 0       \\
CCF              & $G_\beta$ & 1 & 3     & 0.75  & 0.25 & -0.045        & 0.15 & 0.111              & -0.756        & -0.402  & -0.059 & 0.493    & 0.976                   & -1.768 & -0.297 & 0.188   \\
CCF              & $G_\beta$ & 1 & 5     & 0.75  & 0.25 & 0.015         & 0.15 & 0.101              & -0.653        & 0.146   & 0.023  & 0.496    & 1.035                   & 0.585  & 0.098  & 0.663   \\
CCF              & $G_\beta$ & 1 & 7     & 0.75  & 0.25 & 0.064         & 0.15 & 0.104              & -0.545        & 0.615   & 0.118  & 0.5      & 1.079                   & 2.547  & 0.428  & 0.058   \\
CCF              & $G_\beta$ & 3 & 1     & 0.75  & 0.25 & -0.098        & 0.15 & 0.113              & -0.9          & -0.873  & -0.109 & 0.485    & 0.942                   & -3.902 & -0.655 & 0.004   \\
CCF              & $G_\beta$ & 3 & 3     & 0.75  & 0.25 & 0.009         & 0.15 & 0.105              & -0.444        & 0.084   & 0.02   & 0.497    & 1.024                   & 0.351  & 0.059  & 0.794   \\
CCF              & $G_\beta$ & 3 & 5     & 0.75  & 0.25 & 0.014         & 0.15 & 0.101              & -0.505        & 0.141   & 0.028  & 0.497    & 1.03                    & 0.567  & 0.095  & 0.674   \\
CCF              & $G_\beta$ & 3 & 7     & 0.75  & 0.25 & 0.074         & 0.15 & 0.105              & -0.404        & 0.706   & 0.184  & 0.509    & 1.054                   & 2.943  & 0.494  & 0.028   \\
CCF              & $G_\beta$ & 5 & 1     & 0.75  & 0.25 & -0.072        & 0.15 & 0.111              & -0.871        & -0.651  & -0.083 & 0.492    & 0.946                   & -2.872 & -0.482 & 0.032   \\
CCF              & $G_\beta$ & 5 & 3     & 0.75  & 0.25 & -0.002        & 0.15 & 0.107              & -0.65         & -0.023  & -0.004 & 0.498    & 1.005                   & -0.095 & -0.016 & 0.943   \\
CCF              & $G_\beta$ & 5 & 5     & 0.75  & 0.25 & 0.025         & 0.15 & 0.105              & -0.42         & 0.234   & 0.058  & 0.499    & 1.034                   & 0.974  & 0.164  & 0.469   \\
CCF              & $G_\beta$ & 5 & 7     & 0.75  & 0.25 & 0.071         & 0.15 & 0.106              & -0.515        & 0.669   & 0.138  & 0.504    & 1.073                   & 2.826  & 0.475  & 0.036   \\
CCF              & $G_\beta$ & 7 & 1     & 0.75  & 0.25 & -0.062        & 0.15 & 0.11               & -0.795        & -0.564  & -0.078 & 0.491    & 0.963                   & -2.472 & -0.415 & 0.066   \\
CCF              & $G_\beta$ & 7 & 3     & 0.75  & 0.25 & 0.043         & 0.15 & 0.107              & -0.378        & 0.403   & 0.114  & 0.507    & 1.023                   & 1.705  & 0.286  & 0.205   \\
CCF              & $G_\beta$ & 7 & 5     & 0.75  & 0.25 & 0.034         & 0.15 & 0.106              & -0.425        & 0.318   & 0.079  & 0.502    & 1.033                   & 1.338  & 0.225  & 0.32    \\
CCF              & $G_\beta$ & 7 & 7     & 0.75  & 0.25 & 0.089         & 0.15 & 0.105              & -0.313        & 0.85    & 0.285  & 0.499    & 1.117                   & 3.542  & 0.595  & 0.009   \\
CCF              & $G_\beta$ & 1 & 1     & 0.7   & 0.3  & -0.128        & 0.15 & 0.113              & -0.944        & -1.136  & -0.136 & 0.482    & 0.92                    & -5.095 & -0.856 & 0       \\
CCF              & $G_\beta$ & 1 & 3     & 0.7   & 0.3  & -0.043        & 0.15 & 0.111              & -0.764        & -0.385  & -0.056 & 0.492    & 0.982                   & -1.702 & -0.286 & 0.205   \\
CCF              & $G_\beta$ & 1 & 5     & 0.7   & 0.3  & 0.011         & 0.15 & 0.102              & -0.7          & 0.106   & 0.015  & 0.496    & 1.03                    & 0.43   & 0.072  & 0.749   \\
CCF              & $G_\beta$ & 1 & 7     & 0.7   & 0.3  & 0.048         & 0.15 & 0.107              & -0.566        & 0.451   & 0.085  & 0.503    & 1.049                   & 1.912  & 0.321  & 0.156   \\
CCF              & $G_\beta$ & 3 & 1     & 0.7   & 0.3  & -0.089        & 0.15 & 0.113              & -0.888        & -0.784  & -0.1   & 0.491    & 0.933                   & -3.52  & -0.591 & 0.008   \\
CCF              & $G_\beta$ & 3 & 3     & 0.7   & 0.3  & 0.005         & 0.15 & 0.106              & -0.48         & 0.051   & 0.011  & 0.495    & 1.028                   & 0.217  & 0.037  & 0.872   \\
CCF              & $G_\beta$ & 3 & 5     & 0.7   & 0.3  & 0.012         & 0.15 & 0.102              & -0.559        & 0.117   & 0.021  & 0.495    & 1.034                   & 0.474  & 0.08   & 0.725   \\
CCF              & $G_\beta$ & 3 & 7     & 0.7   & 0.3  & 0.074         & 0.15 & 0.107              & -0.369        & 0.693   & 0.201  & 0.513    & 1.038                   & 2.95   & 0.496  & 0.028   \\
CCF              & $G_\beta$ & 5 & 1     & 0.7   & 0.3  & -0.068        & 0.15 & 0.112              & -0.865        & -0.609  & -0.079 & 0.494    & 0.944                   & -2.7   & -0.454 & 0.044   \\
CCF              & $G_\beta$ & 5 & 3     & 0.7   & 0.3  & -0.006        & 0.15 & 0.108              & -0.617        & -0.058  & -0.01  & 0.497    & 1.004                   & -0.25  & -0.042 & 0.853   \\
CCF              & $G_\beta$ & 5 & 5     & 0.7   & 0.3  & 0.03          & 0.15 & 0.106              & -0.451        & 0.287   & 0.067  & 0.499    & 1.043                   & 1.205  & 0.203  & 0.37    \\
CCF              & $G_\beta$ & 5 & 7     & 0.7   & 0.3  & 0.069         & 0.15 & 0.107              & -0.433        & 0.644   & 0.159  & 0.507    & 1.056                   & 2.739  & 0.46   & 0.042   \\
CCF              & $G_\beta$ & 7 & 1     & 0.7   & 0.3  & -0.083        & 0.15 & 0.111              & -0.849        & -0.749  & -0.098 & 0.487    & 0.953                   & -3.307 & -0.556 & 0.014   \\
CCF              & $G_\beta$ & 7 & 3     & 0.7   & 0.3  & 0.037         & 0.15 & 0.107              & -0.484        & 0.342   & 0.076  & 0.506    & 1.022                   & 1.454  & 0.244  & 0.28    \\
CCF              & $G_\beta$ & 7 & 5     & 0.7   & 0.3  & 0.035         & 0.15 & 0.107              & -0.429        & 0.326   & 0.082  & 0.508    & 1.011                   & 1.391  & 0.234  & 0.302   \\
CCF              & $G_\beta$ & 7 & 7     & 0.7   & 0.3  & 0.082         & 0.15 & 0.106              & -0.313        & 0.776   & 0.263  & 0.504    & 1.086                   & 3.262  & 0.548  & 0.015  \\
\hline

KM\_Mod   & $D_\alpha$ & 1 & 1     & 0.85  & 0.15 & -0.065        & 0.15 & 0.11               & -0.827        & -0.594  & -0.079 & 0.491    & 0.957                   & -2.597 & -0.436 & 0.054   \\
KM\_Med & $D_\alpha$ & 1 & 1     & 0.85  & 0.15 & -0.069        & 0.15 & 0.111              & -0.843        & -0.626  & -0.082 & 0.49     & 0.956                   & -2.751 & -0.462 & 0.041   \\
SP\_Mod   & $D_\alpha$ & 1 & 1     & 0.85  & 0.15 & -0.065        & 0.15 & 0.109              & -0.838        & -0.598  & -0.078 & 0.492    & 0.955                   & -2.592 & -0.436 & 0.054   \\
SP\_Med  & $D_\alpha$ & 1 & 1     & 0.85  & 0.15 & -0.066        & 0.15 & 0.109              & -0.843        & -0.604  & -0.078 & 0.489    & 0.966                   & -2.615 & -0.439 & 0.052   \\
KM\_Mod   & $D_\alpha$ & 1 & 3     & 0.85  & 0.15 & -0.039        & 0.15 & 0.111              & -0.697        & -0.351  & -0.056 & 0.487    & 1.003                   & -1.547 & -0.26  & 0.25    \\
KM\_Med & $D_\alpha$ & 1 & 3     & 0.85  & 0.15 & -0.04         & 0.15 & 0.112              & -0.697        & -0.355  & -0.057 & 0.494    & 0.976                   & -1.58  & -0.265 & 0.24    \\
SP\_Mod   & $D_\alpha$ & 1 & 3     & 0.85  & 0.15 & -0.043        & 0.15 & 0.108              & -0.751        & -0.395  & -0.057 & 0.491    & 0.984                   & -1.695 & -0.285 & 0.208   \\
SP\_Med  & $D_\alpha$ & 1 & 3     & 0.85  & 0.15 & -0.03         & 0.15 & 0.107              & -0.7          & -0.28   & -0.043 & 0.488    & 1.01                    & -1.188 & -0.2   & 0.378   \\
KM\_Mod   & $D_\alpha$ & 1 & 5     & 0.85  & 0.15 & 0.013         & 0.15 & 0.104              & -0.681        & 0.129   & 0.02   & 0.498    & 1.025                   & 0.532  & 0.089  & 0.693   \\
KM\_Med & $D_\alpha$ & 1 & 5     & 0.85  & 0.15 & 0.011         & 0.15 & 0.104              & -0.708        & 0.11    & 0.016  & 0.499    & 1.017                   & 0.454  & 0.076  & 0.736   \\
SP\_Mod   & $D_\alpha$ & 1 & 5     & 0.85  & 0.15 & 0.004         & 0.15 & 0.104              & -0.732        & 0.043   & 0.006  & 0.501    & 1.002                   & 0.178  & 0.03   & 0.895   \\
SP\_Med  & $D_\alpha$ & 1 & 5     & 0.85  & 0.15 & 0.022         & 0.15 & 0.102              & -0.692        & 0.212   & 0.031  & 0.502    & 1.017                   & 0.86   & 0.145  & 0.522   \\
KM\_Mod   & $D_\alpha$ & 1 & 7     & 0.85  & 0.15 & 0.031         & 0.15 & 0.111              & -0.448        & 0.276   & 0.068  & 0.513    & 0.987                   & 1.218  & 0.205  & 0.366   \\
KM\_Med & $D_\alpha$ & 1 & 7     & 0.85  & 0.15 & 0.031         & 0.15 & 0.112              & -0.52         & 0.274   & 0.059  & 0.509    & 1.002                   & 1.222  & 0.205  & 0.365   \\
SP\_Mod   & $D_\alpha$ & 1 & 7     & 0.85  & 0.15 & 0.05          & 0.15 & 0.109              & -0.36         & 0.462   & 0.14   & 0.513    & 1.007                   & 1.995  & 0.335  & 0.139   \\
SP\_Med  & $D_\alpha$ & 1 & 7     & 0.85  & 0.15 & 0.046         & 0.15 & 0.109              & -0.388        & 0.418   & 0.117  & 0.515    & 0.997                   & 1.809  & 0.304  & 0.179   \\
KM\_Mod   & $D_\alpha$ & 3 & 1     & 0.85  & 0.15 & -0.026        & 0.15 & 0.111              & -0.611        & -0.232  & -0.042 & 0.499    & 0.974                   & -1.027 & -0.173 & 0.445   \\
KM\_Med & $D_\alpha$ & 3 & 1     & 0.85  & 0.15 & -0.034        & 0.15 & 0.113              & -0.702        & -0.298  & -0.048 & 0.5      & 0.959                   & -1.335 & -0.224 & 0.32    \\
SP\_Mod   & $D_\alpha$ & 3 & 1     & 0.85  & 0.15 & -0.021        & 0.15 & 0.11               & -0.681        & -0.192  & -0.031 & 0.501    & 0.972                   & -0.836 & -0.141 & 0.534   \\
SP\_Med  & $D_\alpha$ & 3 & 1     & 0.85  & 0.15 & -0.023        & 0.15 & 0.11               & -0.674        & -0.205  & -0.033 & 0.502    & 0.965                   & -0.893 & -0.15  & 0.507   \\
KM\_Mod   & $D_\alpha$ & 3 & 3     & 0.85  & 0.15 & -0.006        & 0.15 & 0.109              & -0.582        & -0.053  & -0.01  & 0.5      & 0.992                   & -0.229 & -0.038 & 0.865   \\
KM\_Med & $D_\alpha$ & 3 & 3     & 0.85  & 0.15 & 0.004         & 0.15 & 0.109              & -0.429        & 0.034   & 0.009  & 0.501    & 1.002                   & 0.149  & 0.025  & 0.912   \\
SP\_Mod   & $D_\alpha$ & 3 & 3     & 0.85  & 0.15 & 0.001         & 0.15 & 0.107              & -0.532        & 0.011   & 0.002  & 0.499    & 1.006                   & 0.046  & 0.008  & 0.973   \\
SP\_Med  & $D_\alpha$ & 3 & 3     & 0.85  & 0.15 & 0             & 0.15 & 0.106              & -0.545        & 0.002   & 0      & 0.499    & 1.006                   & 0.009  & 0.001  & 0.995   \\
KM\_Mod   & $D_\alpha$ & 3 & 5     & 0.85  & 0.15 & 0.004         & 0.15 & 0.102              & -0.632        & 0.039   & 0.006  & 0.495    & 1.026                   & 0.16   & 0.027  & 0.906   \\
KM\_Med & $D_\alpha$ & 3 & 5     & 0.85  & 0.15 & 0.014         & 0.15 & 0.101              & -0.53         & 0.138   & 0.026  & 0.496    & 1.033                   & 0.553  & 0.093  & 0.681   \\
SP\_Mod   & $D_\alpha$ & 3 & 5     & 0.85  & 0.15 & 0.021         & 0.15 & 0.1                & -0.504        & 0.212   & 0.042  & 0.499    & 1.029                   & 0.843  & 0.142  & 0.53    \\
SP\_Med  & $D_\alpha$ & 3 & 5     & 0.85  & 0.15 & 0.026         & 0.15 & 0.1                & -0.534        & 0.263   & 0.049  & 0.5      & 1.032                   & 1.038  & 0.174  & 0.44    \\
KM\_Mod   & $D_\alpha$ & 3 & 7     & 0.85  & 0.15 & 0.051         & 0.15 & 0.11               & -0.412        & 0.463   & 0.123  & 0.513    & 1.008                   & 2.013  & 0.338  & 0.135   \\
KM\_Med & $D_\alpha$ & 3 & 7     & 0.85  & 0.15 & 0.045         & 0.15 & 0.111              & -0.448        & 0.404   & 0.1    & 0.508    & 1.023                   & 1.774  & 0.298  & 0.188   \\
SP\_Mod   & $D_\alpha$ & 3 & 7     & 0.85  & 0.15 & 0.067         & 0.15 & 0.109              & -0.412        & 0.612   & 0.162  & 0.518    & 1.008                   & 2.644  & 0.444  & 0.05    \\
SP\_Med  & $D_\alpha$ & 3 & 7     & 0.85  & 0.15 & 0.085         & 0.15 & 0.108              & -0.408        & 0.786   & 0.209  & 0.522    & 1.015                   & 3.381  & 0.568  & 0.012   \\
KM\_Mod   & $D_\alpha$ & 5 & 1     & 0.85  & 0.15 & -0.048        & 0.15 & 0.11               & -0.76         & -0.433  & -0.063 & 0.49     & 0.981                   & -1.899 & -0.319 & 0.158   \\
KM\_Med & $D_\alpha$ & 5 & 1     & 0.85  & 0.15 & -0.03         & 0.15 & 0.111              & -0.709        & -0.271  & -0.043 & 0.504    & 0.95                    & -1.196 & -0.201 & 0.374   \\
SP\_Mod   & $D_\alpha$ & 5 & 1     & 0.85  & 0.15 & -0.053        & 0.15 & 0.108              & -0.791        & -0.487  & -0.067 & 0.494    & 0.962                   & -2.088 & -0.351 & 0.121   \\
SP\_Med  & $D_\alpha$ & 5 & 1     & 0.85  & 0.15 & -0.033        & 0.15 & 0.108              & -0.737        & -0.304  & -0.044 & 0.499    & 0.966                   & -1.301 & -0.219 & 0.334   \\
KM\_Mod   & $D_\alpha$ & 5 & 3     & 0.85  & 0.15 & 0.021         & 0.15 & 0.106              & -0.472        & 0.196   & 0.044  & 0.501    & 1.022                   & 0.824  & 0.138  & 0.54    \\
KM\_Med & $D_\alpha$ & 5 & 3     & 0.85  & 0.15 & 0.022         & 0.15 & 0.107              & -0.437        & 0.207   & 0.051  & 0.498    & 1.034                   & 0.882  & 0.148  & 0.512   \\
SP\_Mod   & $D_\alpha$ & 5 & 3     & 0.85  & 0.15 & 0.006         & 0.15 & 0.105              & -0.574        & 0.053   & 0.01   & 0.498    & 1.015                   & 0.22   & 0.037  & 0.87    \\
SP\_Med  & $D_\alpha$ & 5 & 3     & 0.85  & 0.15 & 0.015         & 0.15 & 0.104              & -0.545        & 0.14    & 0.027  & 0.502    & 1.009                   & 0.582  & 0.098  & 0.665   \\
KM\_Mod   & $D_\alpha$ & 5 & 5     & 0.85  & 0.15 & 0.043         & 0.15 & 0.104              & -0.464        & 0.416   & 0.093  & 0.499    & 1.059                   & 1.707  & 0.287  & 0.204   \\
KM\_Med & $D_\alpha$ & 5 & 5     & 0.85  & 0.15 & 0.069         & 0.15 & 0.104              & -0.307        & 0.664   & 0.225  & 0.509    & 1.049                   & 2.74   & 0.46   & 0.041   \\
SP\_Mod   & $D_\alpha$ & 5 & 5     & 0.85  & 0.15 & 0.049         & 0.15 & 0.102              & -0.427        & 0.479   & 0.115  & 0.502    & 1.054                   & 1.945  & 0.327  & 0.148   \\
SP\_Med  & $D_\alpha$ & 5 & 5     & 0.85  & 0.15 & 0.072         & 0.15 & 0.102              & -0.323        & 0.699   & 0.221  & 0.508    & 1.057                   & 2.837  & 0.477  & 0.034   \\
KM\_Mod   & $D_\alpha$ & 5 & 7     & 0.85  & 0.15 & 0.097         & 0.15 & 0.108              & -0.347        & 0.904   & 0.281  & 0.519    & 1.044                   & 3.865  & 0.649  & 0.004   \\
KM\_Med & $D_\alpha$ & 5 & 7     & 0.85  & 0.15 & 0.096         & 0.15 & 0.109              & -0.324        & 0.874   & 0.295  & 0.514    & 1.063                   & 3.791  & 0.637  & 0.005   \\
SP\_Mod   & $D_\alpha$ & 5 & 7     & 0.85  & 0.15 & 0.094         & 0.15 & 0.106              & -0.311        & 0.885   & 0.302  & 0.519    & 1.038                   & 3.729  & 0.627  & 0.006   \\
SP\_Med  & $D_\alpha$ & 5 & 7     & 0.85  & 0.15 & 0.119         & 0.15 & 0.105              & -0.309        & 1.132   & 0.386  & 0.519    & 1.07                    & 4.729  & 0.795  & 0       \\
KM\_Mod   & $D_\alpha$ & 7 & 1     & 0.85  & 0.15 & -0.021        & 0.15 & 0.111              & -0.561        & -0.189  & -0.037 & 0.5      & 0.975                   & -0.829 & -0.139 & 0.538   \\
KM\_Med & $D_\alpha$ & 7 & 1     & 0.85  & 0.15 & -0.022        & 0.15 & 0.112              & -0.542        & -0.199  & -0.041 & 0.504    & 0.958                   & -0.88  & -0.148 & 0.513   \\
SP\_Mod   & $D_\alpha$ & 7 & 1     & 0.85  & 0.15 & -0.024        & 0.15 & 0.107              & -0.659        & -0.221  & -0.036 & 0.494    & 0.994                   & -0.942 & -0.158 & 0.484   \\
SP\_Med  & $D_\alpha$ & 7 & 1     & 0.85  & 0.15 & -0.004        & 0.15 & 0.107              & -0.541        & -0.036  & -0.007 & 0.501    & 0.991                   & -0.154 & -0.026 & 0.909   \\
KM\_Mod   & $D_\alpha$ & 7 & 3     & 0.85  & 0.15 & 0.061         & 0.15 & 0.105              & -0.367        & 0.581   & 0.166  & 0.505    & 1.056                   & 2.414  & 0.406  & 0.072   \\
KM\_Med & $D_\alpha$ & 7 & 3     & 0.85  & 0.15 & 0.046         & 0.15 & 0.105              & -0.365        & 0.436   & 0.126  & 0.501    & 1.054                   & 1.822  & 0.306  & 0.175   \\
SP\_Mod   & $D_\alpha$ & 7 & 3     & 0.85  & 0.15 & 0.046         & 0.15 & 0.105              & -0.446        & 0.435   & 0.102  & 0.503    & 1.042                   & 1.809  & 0.304  & 0.178   \\
SP\_Med  & $D_\alpha$ & 7 & 3     & 0.85  & 0.15 & 0.067         & 0.15 & 0.104              & -0.385        & 0.644   & 0.173  & 0.513    & 1.031                   & 2.646  & 0.445  & 0.049   \\
KM\_Mod   & $D_\alpha$ & 7 & 5     & 0.85  & 0.15 & 0.044         & 0.15 & 0.106              & -0.347        & 0.417   & 0.127  & 0.506    & 1.031                   & 1.755  & 0.295  & 0.192   \\
KM\_Med & $D_\alpha$ & 7 & 5     & 0.85  & 0.15 & 0.051         & 0.15 & 0.107              & -0.387        & 0.477   & 0.132  & 0.508    & 1.032                   & 2.025  & 0.34   & 0.132   \\
SP\_Mod   & $D_\alpha$ & 7 & 5     & 0.85  & 0.15 & 0.041         & 0.15 & 0.106              & -0.406        & 0.391   & 0.102  & 0.512    & 1                       & 1.64   & 0.276  & 0.223   \\
SP\_Med  & $D_\alpha$ & 7 & 5     & 0.85  & 0.15 & 0.053         & 0.15 & 0.106              & -0.392        & 0.505   & 0.136  & 0.511    & 1.022                   & 2.12   & 0.356  & 0.115   \\
KM\_Mod   & $D_\alpha$ & 7 & 7     & 0.85  & 0.15 & 0.123         & 0.15 & 0.106              & -0.288        & 1.157   & 0.427  & 0.522    & 1.065                   & 4.881  & 0.82   & 0       \\
KM\_Med & $D_\alpha$ & 7 & 7     & 0.85  & 0.15 & 0.1           & 0.15 & 0.108              & -0.259        & 0.925   & 0.386  & 0.514    & 1.068                   & 3.97   & 0.667  & 0.003   \\
SP\_Mod   & $D_\alpha$ & 7 & 7     & 0.85  & 0.15 & 0.123         & 0.15 & 0.105              & -0.256        & 1.18    & 0.482  & 0.521    & 1.068                   & 4.895  & 0.822  & 0       \\
SP\_Med  & $D_\alpha$ & 7 & 7     & 0.85  & 0.15 & 0.13          & 0.15 & 0.104              & -0.215        & 1.253   & 0.604  & 0.525    & 1.059                   & 5.15   & 0.865  & 0       \\
KM\_Mod   & $D_\alpha$ & 1 & 1     & 0.8   & 0.2  & -0.064        & 0.15 & 0.11               & -0.828        & -0.577  & -0.077 & 0.487    & 0.974                   & -2.521 & -0.424 & 0.061   \\
KM\_Med & $D_\alpha$ & 1 & 1     & 0.8   & 0.2  & -0.074        & 0.15 & 0.11               & -0.859        & -0.672  & -0.086 & 0.484    & 0.973                   & -2.938 & -0.494 & 0.029   \\
SP\_Mod   & $D_\alpha$ & 1 & 1     & 0.8   & 0.2  & -0.059        & 0.15 & 0.109              & -0.837        & -0.544  & -0.071 & 0.488    & 0.978                   & -2.352 & -0.395 & 0.081   \\
SP\_Med  & $D_\alpha$ & 1 & 1     & 0.8   & 0.2  & -0.07         & 0.15 & 0.109              & -0.85         & -0.644  & -0.083 & 0.489    & 0.958                   & -2.787 & -0.468 & 0.038   \\
KM\_Mod   & $D_\alpha$ & 1 & 3     & 0.8   & 0.2  & -0.046        & 0.15 & 0.112              & -0.732        & -0.411  & -0.063 & 0.485    & 1.005                   & -1.819 & -0.306 & 0.176   \\
KM\_Med & $D_\alpha$ & 1 & 3     & 0.8   & 0.2  & -0.039        & 0.15 & 0.112              & -0.692        & -0.352  & -0.057 & 0.493    & 0.981                   & -1.559 & -0.262 & 0.246   \\
SP\_Mod   & $D_\alpha$ & 1 & 3     & 0.8   & 0.2  & -0.044        & 0.15 & 0.11               & -0.732        & -0.396  & -0.06  & 0.492    & 0.981                   & -1.73  & -0.291 & 0.198   \\
SP\_Med  & $D_\alpha$ & 1 & 3     & 0.8   & 0.2  & -0.029        & 0.15 & 0.107              & -0.711        & -0.268  & -0.04  & 0.489    & 1.011                   & -1.135 & -0.191 & 0.399   \\
KM\_Mod   & $D_\alpha$ & 1 & 5     & 0.8   & 0.2  & 0.008         & 0.15 & 0.104              & -0.644        & 0.08    & 0.013  & 0.497    & 1.022                   & 0.332  & 0.056  & 0.805   \\
KM\_Med & $D_\alpha$ & 1 & 5     & 0.8   & 0.2  & 0.014         & 0.15 & 0.104              & -0.678        & 0.13    & 0.02   & 0.494    & 1.04                    & 0.536  & 0.09   & 0.69    \\
SP\_Mod   & $D_\alpha$ & 1 & 5     & 0.8   & 0.2  & -0.004        & 0.15 & 0.104              & -0.749        & -0.039  & -0.005 & 0.498    & 1.003                   & -0.16  & -0.027 & 0.905   \\
SP\_Med  & $D_\alpha$ & 1 & 5     & 0.8   & 0.2  & 0.019         & 0.15 & 0.103              & -0.703        & 0.184   & 0.027  & 0.5      & 1.022                   & 0.753  & 0.126  & 0.576   \\
KM\_Mod   & $D_\alpha$ & 1 & 7     & 0.8   & 0.2  & 0.032         & 0.15 & 0.111              & -0.424        & 0.292   & 0.076  & 0.511    & 0.996                   & 1.279  & 0.215  & 0.342   \\
KM\_Med & $D_\alpha$ & 1 & 7     & 0.8   & 0.2  & 0.041         & 0.15 & 0.113              & -0.441        & 0.367   & 0.094  & 0.51     & 1.011                   & 1.637  & 0.275  & 0.225   \\
SP\_Mod   & $D_\alpha$ & 1 & 7     & 0.8   & 0.2  & 0.044         & 0.15 & 0.109              & -0.399        & 0.402   & 0.11   & 0.513    & 1.002                   & 1.738  & 0.292  & 0.197   \\
SP\_Med  & $D_\alpha$ & 1 & 7     & 0.8   & 0.2  & 0.047         & 0.15 & 0.109              & -0.38         & 0.429   & 0.124  & 0.514    & 1                       & 1.865  & 0.313  & 0.166   \\
KM\_Mod   & $D_\alpha$ & 3 & 1     & 0.8   & 0.2  & -0.049        & 0.15 & 0.113              & -0.723        & -0.43   & -0.067 & 0.498    & 0.951                   & -1.93  & -0.324 & 0.151   \\
KM\_Med & $D_\alpha$ & 3 & 1     & 0.8   & 0.2  & -0.034        & 0.15 & 0.113              & -0.674        & -0.301  & -0.051 & 0.496    & 0.973                   & -1.351 & -0.227 & 0.315   \\
SP\_Mod   & $D_\alpha$ & 3 & 1     & 0.8   & 0.2  & -0.031        & 0.15 & 0.11               & -0.746        & -0.279  & -0.041 & 0.495    & 0.982                   & -1.221 & -0.205 & 0.364   \\
SP\_Med  & $D_\alpha$ & 3 & 1     & 0.8   & 0.2  & -0.018        & 0.15 & 0.109              & -0.672        & -0.166  & -0.027 & 0.5      & 0.977                   & -0.723 & -0.121 & 0.591   \\
KM\_Mod   & $D_\alpha$ & 3 & 3     & 0.8   & 0.2  & -0.007        & 0.15 & 0.109              & -0.557        & -0.063  & -0.012 & 0.498    & 0.999                   & -0.27  & -0.045 & 0.841   \\
KM\_Med & $D_\alpha$ & 3 & 3     & 0.8   & 0.2  & 0.012         & 0.15 & 0.109              & -0.347        & 0.11    & 0.035  & 0.505    & 0.996                   & 0.477  & 0.08   & 0.723   \\
SP\_Mod   & $D_\alpha$ & 3 & 3     & 0.8   & 0.2  & -0.023        & 0.15 & 0.108              & -0.697        & -0.213  & -0.033 & 0.491    & 1.006                   & -0.91  & -0.153 & 0.499   \\
SP\_Med  & $D_\alpha$ & 3 & 3     & 0.8   & 0.2  & 0.007         & 0.15 & 0.106              & -0.509        & 0.063   & 0.013  & 0.498    & 1.015                   & 0.265  & 0.045  & 0.844   \\
KM\_Mod   & $D_\alpha$ & 3 & 5     & 0.8   & 0.2  & 0.019         & 0.15 & 0.101              & -0.527        & 0.184   & 0.035  & 0.498    & 1.032                   & 0.742  & 0.125  & 0.581   \\
KM\_Med & $D_\alpha$ & 3 & 5     & 0.8   & 0.2  & 0.027         & 0.15 & 0.102              & -0.484        & 0.264   & 0.056  & 0.498    & 1.041                   & 1.069  & 0.18   & 0.426   \\
SP\_Mod   & $D_\alpha$ & 3 & 5     & 0.8   & 0.2  & 0.023         & 0.15 & 0.1                & -0.545        & 0.235   & 0.043  & 0.5      & 1.03                    & 0.927  & 0.156  & 0.49    \\
SP\_Med  & $D_\alpha$ & 3 & 5     & 0.8   & 0.2  & 0.024         & 0.15 & 0.1                & -0.502        & 0.24    & 0.048  & 0.496    & 1.045                   & 0.951  & 0.16   & 0.479   \\
KM\_Mod   & $D_\alpha$ & 3 & 7     & 0.8   & 0.2  & 0.045         & 0.15 & 0.11               & -0.404        & 0.408   & 0.111  & 0.508    & 1.023                   & 1.778  & 0.299  & 0.187   \\
KM\_Med & $D_\alpha$ & 3 & 7     & 0.8   & 0.2  & 0.041         & 0.15 & 0.111              & -0.478        & 0.364   & 0.085  & 0.509    & 1.014                   & 1.607  & 0.27   & 0.233   \\
SP\_Mod   & $D_\alpha$ & 3 & 7     & 0.8   & 0.2  & 0.056         & 0.15 & 0.109              & -0.42         & 0.516   & 0.134  & 0.515    & 1.008                   & 2.235  & 0.376  & 0.097   \\
SP\_Med  & $D_\alpha$ & 3 & 7     & 0.8   & 0.2  & 0.082         & 0.15 & 0.109              & -0.387        & 0.75    & 0.211  & 0.522    & 1.012                   & 3.247  & 0.546  & 0.016   \\
KM\_Mod   & $D_\alpha$ & 5 & 1     & 0.8   & 0.2  & -0.048        & 0.15 & 0.111              & -0.751        & -0.433  & -0.064 & 0.492    & 0.974                   & -1.911 & -0.321 & 0.156   \\
KM\_Med & $D_\alpha$ & 5 & 1     & 0.8   & 0.2  & -0.046        & 0.15 & 0.112              & -0.76         & -0.415  & -0.061 & 0.498    & 0.952                   & -1.842 & -0.309 & 0.171   \\
SP\_Mod   & $D_\alpha$ & 5 & 1     & 0.8   & 0.2  & -0.039        & 0.15 & 0.108              & -0.771        & -0.358  & -0.05  & 0.492    & 0.986                   & -1.537 & -0.258 & 0.254   \\
SP\_Med  & $D_\alpha$ & 5 & 1     & 0.8   & 0.2  & -0.038        & 0.15 & 0.108              & -0.739        & -0.351  & -0.051 & 0.495    & 0.975                   & -1.497 & -0.251 & 0.266   \\
KM\_Mod   & $D_\alpha$ & 5 & 3     & 0.8   & 0.2  & 0.03          & 0.15 & 0.106              & -0.461        & 0.281   & 0.065  & 0.498    & 1.045                   & 1.183  & 0.199  & 0.379   \\
KM\_Med & $D_\alpha$ & 5 & 3     & 0.8   & 0.2  & 0.027         & 0.15 & 0.108              & -0.447        & 0.253   & 0.061  & 0.5      & 1.034                   & 1.09   & 0.183  & 0.418   \\
SP\_Mod   & $D_\alpha$ & 5 & 3     & 0.8   & 0.2  & 0.007         & 0.15 & 0.105              & -0.597        & 0.064   & 0.011  & 0.497    & 1.019                   & 0.267  & 0.045  & 0.843   \\
SP\_Med  & $D_\alpha$ & 5 & 3     & 0.8   & 0.2  & 0.018         & 0.15 & 0.105              & -0.538        & 0.172   & 0.033  & 0.503    & 1.011                   & 0.715  & 0.12   & 0.595   \\
KM\_Mod   & $D_\alpha$ & 5 & 5     & 0.8   & 0.2  & 0.05          & 0.15 & 0.105              & -0.478        & 0.474   & 0.104  & 0.501    & 1.057                   & 1.972  & 0.331  & 0.142   \\
KM\_Med & $D_\alpha$ & 5 & 5     & 0.8   & 0.2  & 0.072         & 0.15 & 0.104              & -0.316        & 0.696   & 0.229  & 0.508    & 1.059                   & 2.873  & 0.483  & 0.032   \\
SP\_Mod   & $D_\alpha$ & 5 & 5     & 0.8   & 0.2  & 0.046         & 0.15 & 0.102              & -0.396        & 0.453   & 0.117  & 0.502    & 1.051                   & 1.834  & 0.308  & 0.172   \\
SP\_Med  & $D_\alpha$ & 5 & 5     & 0.8   & 0.2  & 0.071         & 0.15 & 0.102              & -0.332        & 0.698   & 0.214  & 0.501    & 1.083                   & 2.817  & 0.473  & 0.036   \\
KM\_Mod   & $D_\alpha$ & 5 & 7     & 0.8   & 0.2  & 0.094         & 0.15 & 0.107              & -0.369        & 0.878   & 0.256  & 0.515    & 1.056                   & 3.743  & 0.629  & 0.005   \\
KM\_Med & $D_\alpha$ & 5 & 7     & 0.8   & 0.2  & 0.068         & 0.15 & 0.111              & -0.396        & 0.615   & 0.172  & 0.513    & 1.032                   & 2.698  & 0.453  & 0.045   \\
SP\_Mod   & $D_\alpha$ & 5 & 7     & 0.8   & 0.2  & 0.089         & 0.15 & 0.106              & -0.279        & 0.835   & 0.318  & 0.517    & 1.041                   & 3.524  & 0.592  & 0.009   \\
SP\_Med  & $D_\alpha$ & 5 & 7     & 0.8   & 0.2  & 0.121         & 0.15 & 0.106              & -0.338        & 1.147   & 0.359  & 0.523    & 1.058                   & 4.818  & 0.809  & 0       \\
KM\_Mod   & $D_\alpha$ & 7 & 1     & 0.8   & 0.2  & -0.03         & 0.15 & 0.111              & -0.608        & -0.267  & -0.049 & 0.496    & 0.979                   & -1.175 & -0.197 & 0.382   \\
KM\_Med & $D_\alpha$ & 7 & 1     & 0.8   & 0.2  & -0.023        & 0.15 & 0.112              & -0.578        & -0.205  & -0.04  & 0.501    & 0.969                   & -0.912 & -0.153 & 0.498   \\
SP\_Mod   & $D_\alpha$ & 7 & 1     & 0.8   & 0.2  & -0.021        & 0.15 & 0.109              & -0.674        & -0.195  & -0.031 & 0.493    & 1.001                   & -0.842 & -0.142 & 0.531   \\
SP\_Med  & $D_\alpha$ & 7 & 1     & 0.8   & 0.2  & -0.014        & 0.15 & 0.107              & -0.606        & -0.132  & -0.023 & 0.497    & 0.994                   & -0.562 & -0.094 & 0.677   \\
KM\_Mod   & $D_\alpha$ & 7 & 3     & 0.8   & 0.2  & 0.046         & 0.15 & 0.105              & -0.355        & 0.439   & 0.13   & 0.497    & 1.071                   & 1.829  & 0.307  & 0.173   \\
KM\_Med & $D_\alpha$ & 7 & 3     & 0.8   & 0.2  & 0.048         & 0.15 & 0.105              & -0.369        & 0.455   & 0.129  & 0.501    & 1.054                   & 1.89   & 0.317  & 0.159   \\
SP\_Mod   & $D_\alpha$ & 7 & 3     & 0.8   & 0.2  & 0.062         & 0.15 & 0.104              & -0.381        & 0.598   & 0.164  & 0.508    & 1.043                   & 2.48   & 0.417  & 0.065   \\
SP\_Med  & $D_\alpha$ & 7 & 3     & 0.8   & 0.2  & 0.071         & 0.15 & 0.103              & -0.353        & 0.69    & 0.201  & 0.51     & 1.048                   & 2.813  & 0.473  & 0.036   \\
KM\_Mod   & $D_\alpha$ & 7 & 5     & 0.8   & 0.2  & 0.031         & 0.15 & 0.107              & -0.358        & 0.292   & 0.087  & 0.504    & 1.023                   & 1.242  & 0.209  & 0.356   \\
KM\_Med & $D_\alpha$ & 7 & 5     & 0.8   & 0.2  & 0.038         & 0.15 & 0.107              & -0.397        & 0.355   & 0.096  & 0.502    & 1.04                    & 1.513  & 0.254  & 0.261   \\
SP\_Mod   & $D_\alpha$ & 7 & 5     & 0.8   & 0.2  & 0.051         & 0.15 & 0.105              & -0.343        & 0.486   & 0.148  & 0.511    & 1.019                   & 2.016  & 0.339  & 0.134   \\
SP\_Med  & $D_\alpha$ & 7 & 5     & 0.8   & 0.2  & 0.059         & 0.15 & 0.105              & -0.375        & 0.56    & 0.157  & 0.507    & 1.043                   & 2.334  & 0.392  & 0.083   \\
KM\_Mod   & $D_\alpha$ & 7 & 7     & 0.8   & 0.2  & 0.117         & 0.15 & 0.106              & -0.289        & 1.102   & 0.405  & 0.52     & 1.067                   & 4.648  & 0.781  & 0.001   \\
KM\_Med & $D_\alpha$ & 7 & 7     & 0.8   & 0.2  & 0.086         & 0.15 & 0.109              & -0.286        & 0.788   & 0.299  & 0.512    & 1.058                   & 3.397  & 0.571  & 0.012   \\
SP\_Mod   & $D_\alpha$ & 7 & 7     & 0.8   & 0.2  & 0.129         & 0.15 & 0.105              & -0.28         & 1.226   & 0.46   & 0.52     & 1.079                   & 5.115  & 0.859  & 0       \\
SP\_Med  & $D_\alpha$ & 7 & 7     & 0.8   & 0.2  & 0.134         & 0.15 & 0.105              & -0.217        & 1.273   & 0.617  & 0.526    & 1.06                    & 5.316  & 0.893  & 0       \\
KM\_Mod   & $D_\alpha$ & 1 & 1     & 0.75  & 0.25 & -0.065        & 0.15 & 0.11               & -0.819        & -0.592  & -0.08  & 0.492    & 0.952                   & -2.59  & -0.435 & 0.054   \\
KM\_Med & $D_\alpha$ & 1 & 1     & 0.75  & 0.25 & -0.066        & 0.15 & 0.111              & -0.861        & -0.596  & -0.077 & 0.484    & 0.981                   & -2.615 & -0.439 & 0.052   \\
SP\_Mod   & $D_\alpha$ & 1 & 1     & 0.75  & 0.25 & -0.057        & 0.15 & 0.11               & -0.815        & -0.519  & -0.07  & 0.491    & 0.966                   & -2.26  & -0.38  & 0.093   \\
SP\_Med  & $D_\alpha$ & 1 & 1     & 0.75  & 0.25 & -0.069        & 0.15 & 0.11               & -0.838        & -0.627  & -0.082 & 0.491    & 0.953                   & -2.734 & -0.459 & 0.042   \\
KM\_Mod   & $D_\alpha$ & 1 & 3     & 0.75  & 0.25 & -0.043        & 0.15 & 0.112              & -0.737        & -0.383  & -0.058 & 0.486    & 1.004                   & -1.697 & -0.285 & 0.207   \\
KM\_Med & $D_\alpha$ & 1 & 3     & 0.75  & 0.25 & -0.027        & 0.15 & 0.113              & -0.673        & -0.241  & -0.04  & 0.497    & 0.981                   & -1.078 & -0.181 & 0.423   \\
SP\_Mod   & $D_\alpha$ & 1 & 3     & 0.75  & 0.25 & -0.044        & 0.15 & 0.109              & -0.729        & -0.408  & -0.061 & 0.49     & 0.985                   & -1.762 & -0.296 & 0.19    \\
SP\_Med  & $D_\alpha$ & 1 & 3     & 0.75  & 0.25 & -0.026        & 0.15 & 0.107              & -0.693        & -0.242  & -0.038 & 0.491    & 1.005                   & -1.033 & -0.174 & 0.443   \\
KM\_Mod   & $D_\alpha$ & 1 & 5     & 0.75  & 0.25 & 0.008         & 0.15 & 0.105              & -0.671        & 0.079   & 0.012  & 0.497    & 1.023                   & 0.326  & 0.055  & 0.808   \\
KM\_Med & $D_\alpha$ & 1 & 5     & 0.75  & 0.25 & 0.007         & 0.15 & 0.104              & -0.739        & 0.065   & 0.009  & 0.494    & 1.032                   & 0.271  & 0.045  & 0.841   \\
SP\_Mod   & $D_\alpha$ & 1 & 5     & 0.75  & 0.25 & 0.002         & 0.15 & 0.103              & -0.748        & 0.017   & 0.002  & 0.497    & 1.014                   & 0.069  & 0.012  & 0.959   \\
SP\_Med  & $D_\alpha$ & 1 & 5     & 0.75  & 0.25 & 0.021         & 0.15 & 0.103              & -0.681        & 0.208   & 0.031  & 0.499    & 1.029                   & 0.85   & 0.143  & 0.527   \\
KM\_Mod   & $D_\alpha$ & 1 & 7     & 0.75  & 0.25 & 0.03          & 0.15 & 0.111              & -0.448        & 0.273   & 0.068  & 0.512    & 0.989                   & 1.206  & 0.203  & 0.371   \\
KM\_Med & $D_\alpha$ & 1 & 7     & 0.75  & 0.25 & 0.03          & 0.15 & 0.113              & -0.491        & 0.265   & 0.061  & 0.509    & 1.002                   & 1.19   & 0.2    & 0.377   \\
SP\_Mod   & $D_\alpha$ & 1 & 7     & 0.75  & 0.25 & 0.052         & 0.15 & 0.109              & -0.384        & 0.476   & 0.135  & 0.513    & 1.009                   & 2.056  & 0.345  & 0.127   \\
SP\_Med  & $D_\alpha$ & 1 & 7     & 0.75  & 0.25 & 0.039         & 0.15 & 0.109              & -0.421        & 0.358   & 0.093  & 0.507    & 1.018                   & 1.55   & 0.26   & 0.25    \\
KM\_Mod   & $D_\alpha$ & 3 & 1     & 0.75  & 0.25 & -0.047        & 0.15 & 0.112              & -0.731        & -0.418  & -0.064 & 0.499    & 0.949                   & -1.867 & -0.314 & 0.165   \\
KM\_Med & $D_\alpha$ & 3 & 1     & 0.75  & 0.25 & -0.038        & 0.15 & 0.114              & -0.694        & -0.334  & -0.055 & 0.495    & 0.973                   & -1.507 & -0.253 & 0.262   \\
SP\_Mod   & $D_\alpha$ & 3 & 1     & 0.75  & 0.25 & -0.028        & 0.15 & 0.111              & -0.739        & -0.255  & -0.038 & 0.5      & 0.966                   & -1.123 & -0.189 & 0.404   \\
SP\_Med  & $D_\alpha$ & 3 & 1     & 0.75  & 0.25 & -0.029        & 0.15 & 0.109              & -0.737        & -0.262  & -0.039 & 0.498    & 0.975                   & -1.14  & -0.192 & 0.397   \\
KM\_Mod   & $D_\alpha$ & 3 & 3     & 0.75  & 0.25 & -0.006        & 0.15 & 0.109              & -0.488        & -0.057  & -0.013 & 0.499    & 0.997                   & -0.247 & -0.041 & 0.854   \\
KM\_Med & $D_\alpha$ & 3 & 3     & 0.75  & 0.25 & 0.002         & 0.15 & 0.109              & -0.351        & 0.019   & 0.006  & 0.499    & 1.007                   & 0.083  & 0.014  & 0.951   \\
SP\_Mod   & $D_\alpha$ & 3 & 3     & 0.75  & 0.25 & -0.018        & 0.15 & 0.107              & -0.64         & -0.165  & -0.028 & 0.494    & 1.002                   & -0.701 & -0.118 & 0.603   \\
SP\_Med  & $D_\alpha$ & 3 & 3     & 0.75  & 0.25 & 0.005         & 0.15 & 0.106              & -0.502        & 0.048   & 0.01   & 0.499    & 1.009                   & 0.203  & 0.034  & 0.88    \\
KM\_Mod   & $D_\alpha$ & 3 & 5     & 0.75  & 0.25 & 0.014         & 0.15 & 0.103              & -0.541        & 0.134   & 0.025  & 0.499    & 1.022                   & 0.544  & 0.091  & 0.686   \\
KM\_Med & $D_\alpha$ & 3 & 5     & 0.75  & 0.25 & 0.02          & 0.15 & 0.104              & -0.48         & 0.192   & 0.042  & 0.5      & 1.026                   & 0.791  & 0.133  & 0.556   \\
SP\_Mod   & $D_\alpha$ & 3 & 5     & 0.75  & 0.25 & 0.014         & 0.15 & 0.1                & -0.587        & 0.143   & 0.024  & 0.497    & 1.029                   & 0.567  & 0.095  & 0.673   \\
SP\_Med  & $D_\alpha$ & 3 & 5     & 0.75  & 0.25 & 0.009         & 0.15 & 0.102              & -0.566        & 0.087   & 0.016  & 0.496    & 1.029                   & 0.353  & 0.059  & 0.793   \\
KM\_Mod   & $D_\alpha$ & 3 & 7     & 0.75  & 0.25 & 0.042         & 0.15 & 0.108              & -0.391        & 0.386   & 0.107  & 0.509    & 1.017                   & 1.663  & 0.279  & 0.217   \\
KM\_Med & $D_\alpha$ & 3 & 7     & 0.75  & 0.25 & 0.047         & 0.15 & 0.112              & -0.472        & 0.415   & 0.099  & 0.513    & 1.007                   & 1.847  & 0.31   & 0.171   \\
SP\_Mod   & $D_\alpha$ & 3 & 7     & 0.75  & 0.25 & 0.045         & 0.15 & 0.109              & -0.437        & 0.41    & 0.102  & 0.514    & 0.999                   & 1.771  & 0.297  & 0.189   \\
SP\_Med  & $D_\alpha$ & 3 & 7     & 0.75  & 0.25 & 0.074         & 0.15 & 0.11               & -0.353        & 0.673   & 0.209  & 0.517    & 1.022                   & 2.925  & 0.491  & 0.03    \\
KM\_Mod   & $D_\alpha$ & 5 & 1     & 0.75  & 0.25 & -0.041        & 0.15 & 0.111              & -0.726        & -0.37   & -0.057 & 0.495    & 0.97                    & -1.631 & -0.274 & 0.226   \\
KM\_Med & $D_\alpha$ & 5 & 1     & 0.75  & 0.25 & -0.049        & 0.15 & 0.113              & -0.751        & -0.435  & -0.065 & 0.498    & 0.949                   & -1.942 & -0.326 & 0.149   \\
SP\_Mod   & $D_\alpha$ & 5 & 1     & 0.75  & 0.25 & -0.037        & 0.15 & 0.108              & -0.742        & -0.343  & -0.05  & 0.496    & 0.97                    & -1.472 & -0.247 & 0.274   \\
SP\_Med  & $D_\alpha$ & 5 & 1     & 0.75  & 0.25 & -0.047        & 0.15 & 0.108              & -0.75         & -0.437  & -0.063 & 0.494    & 0.967                   & -1.876 & -0.315 & 0.164   \\
KM\_Mod   & $D_\alpha$ & 5 & 3     & 0.75  & 0.25 & 0.029         & 0.15 & 0.107              & -0.42         & 0.276   & 0.07   & 0.502    & 1.027                   & 1.17   & 0.197  & 0.384   \\
KM\_Med & $D_\alpha$ & 5 & 3     & 0.75  & 0.25 & 0.031         & 0.15 & 0.108              & -0.347        & 0.29    & 0.09   & 0.502    & 1.029                   & 1.241  & 0.209  & 0.356   \\
SP\_Mod   & $D_\alpha$ & 5 & 3     & 0.75  & 0.25 & 0.001         & 0.15 & 0.105              & -0.58         & 0.01    & 0.002  & 0.497    & 1.013                   & 0.04   & 0.007  & 0.976   \\
SP\_Med  & $D_\alpha$ & 5 & 3     & 0.75  & 0.25 & 0.011         & 0.15 & 0.105              & -0.554        & 0.109   & 0.021  & 0.503    & 1.003                   & 0.455  & 0.076  & 0.735   \\
KM\_Mod   & $D_\alpha$ & 5 & 5     & 0.75  & 0.25 & 0.059         & 0.15 & 0.104              & -0.419        & 0.565   & 0.141  & 0.503    & 1.061                   & 2.341  & 0.393  & 0.081   \\
KM\_Med & $D_\alpha$ & 5 & 5     & 0.75  & 0.25 & 0.059         & 0.15 & 0.105              & -0.367        & 0.567   & 0.162  & 0.506    & 1.051                   & 2.354  & 0.395  & 0.08    \\
SP\_Mod   & $D_\alpha$ & 5 & 5     & 0.75  & 0.25 & 0.049         & 0.15 & 0.102              & -0.405        & 0.478   & 0.121  & 0.502    & 1.053                   & 1.94   & 0.326  & 0.149   \\
SP\_Med  & $D_\alpha$ & 5 & 5     & 0.75  & 0.25 & 0.075         & 0.15 & 0.102              & -0.262        & 0.731   & 0.285  & 0.506    & 1.067                   & 2.966  & 0.498  & 0.027   \\
KM\_Mod   & $D_\alpha$ & 5 & 7     & 0.75  & 0.25 & 0.091         & 0.15 & 0.107              & -0.322        & 0.854   & 0.283  & 0.515    & 1.054                   & 3.617  & 0.608  & 0.007   \\
KM\_Med & $D_\alpha$ & 5 & 7     & 0.75  & 0.25 & 0.069         & 0.15 & 0.111              & -0.381        & 0.623   & 0.181  & 0.51     & 1.046                   & 2.742  & 0.461  & 0.042   \\
SP\_Mod   & $D_\alpha$ & 5 & 7     & 0.75  & 0.25 & 0.105         & 0.15 & 0.106              & -0.282        & 0.991   & 0.372  & 0.52     & 1.05                    & 4.162  & 0.699  & 0.002   \\
SP\_Med  & $D_\alpha$ & 5 & 7     & 0.75  & 0.25 & 0.12          & 0.15 & 0.106              & -0.401        & 1.133   & 0.3    & 0.518    & 1.076                   & 4.769  & 0.801  & 0       \\
KM\_Mod   & $D_\alpha$ & 7 & 1     & 0.75  & 0.25 & -0.035        & 0.15 & 0.112              & -0.63         & -0.313  & -0.055 & 0.5      & 0.959                   & -1.386 & -0.233 & 0.303   \\
KM\_Med & $D_\alpha$ & 7 & 1     & 0.75  & 0.25 & -0.022        & 0.15 & 0.113              & -0.544        & -0.195  & -0.04  & 0.501    & 0.969                   & -0.871 & -0.146 & 0.517   \\
SP\_Mod   & $D_\alpha$ & 7 & 1     & 0.75  & 0.25 & -0.02         & 0.15 & 0.109              & -0.633        & -0.187  & -0.032 & 0.497    & 0.987                   & -0.808 & -0.136 & 0.548   \\
SP\_Med  & $D_\alpha$ & 7 & 1     & 0.75  & 0.25 & -0.019        & 0.15 & 0.108              & -0.652        & -0.179  & -0.03  & 0.498    & 0.985                   & -0.765 & -0.128 & 0.57    \\
KM\_Mod   & $D_\alpha$ & 7 & 3     & 0.75  & 0.25 & 0.044         & 0.15 & 0.106              & -0.347        & 0.412   & 0.126  & 0.499    & 1.058                   & 1.734  & 0.291  & 0.197   \\
KM\_Med & $D_\alpha$ & 7 & 3     & 0.75  & 0.25 & 0.051         & 0.15 & 0.104              & -0.341        & 0.493   & 0.151  & 0.498    & 1.073                   & 2.042  & 0.343  & 0.128   \\
SP\_Mod   & $D_\alpha$ & 7 & 3     & 0.75  & 0.25 & 0.053         & 0.15 & 0.104              & -0.445        & 0.513   & 0.12   & 0.503    & 1.053                   & 2.113  & 0.355  & 0.116   \\
SP\_Med  & $D_\alpha$ & 7 & 3     & 0.75  & 0.25 & 0.062         & 0.15 & 0.104              & -0.371        & 0.598   & 0.167  & 0.508    & 1.046                   & 2.46   & 0.413  & 0.067   \\
KM\_Mod   & $D_\alpha$ & 7 & 5     & 0.75  & 0.25 & 0.026         & 0.15 & 0.107              & -0.445        & 0.239   & 0.058  & 0.502    & 1.025                   & 1.019  & 0.171  & 0.449   \\
KM\_Med & $D_\alpha$ & 7 & 5     & 0.75  & 0.25 & 0.02          & 0.15 & 0.108              & -0.411        & 0.184   & 0.048  & 0.503    & 1.012                   & 0.791  & 0.133  & 0.557   \\
SP\_Mod   & $D_\alpha$ & 7 & 5     & 0.75  & 0.25 & 0.05          & 0.15 & 0.105              & -0.422        & 0.481   & 0.119  & 0.509    & 1.026                   & 1.997  & 0.335  & 0.138   \\
SP\_Med  & $D_\alpha$ & 7 & 5     & 0.75  & 0.25 & 0.046         & 0.15 & 0.107              & -0.443        & 0.426   & 0.103  & 0.505    & 1.036                   & 1.809  & 0.304  & 0.179   \\
KM\_Mod   & $D_\alpha$ & 7 & 7     & 0.75  & 0.25 & 0.122         & 0.15 & 0.107              & -0.251        & 1.148   & 0.488  & 0.521    & 1.069                   & 4.856  & 0.816  & 0       \\
KM\_Med & $D_\alpha$ & 7 & 7     & 0.75  & 0.25 & 0.095         & 0.15 & 0.108              & -0.21         & 0.876   & 0.452  & 0.513    & 1.066                   & 3.765  & 0.632  & 0.005   \\
SP\_Mod   & $D_\alpha$ & 7 & 7     & 0.75  & 0.25 & 0.129         & 0.15 & 0.106              & -0.283        & 1.222   & 0.456  & 0.522    & 1.072                   & 5.121  & 0.86   & 0       \\
SP\_Med  & $D_\alpha$ & 7 & 7     & 0.75  & 0.25 & 0.134         & 0.15 & 0.105              & -0.227        & 1.269   & 0.59   & 0.525    & 1.065                   & 5.312  & 0.892  & 0       \\
KM\_Mod   & $D_\alpha$ & 1 & 1     & 0.7   & 0.3  & -0.062        & 0.15 & 0.109              & -0.796        & -0.567  & -0.078 & 0.488    & 0.974                   & -2.459 & -0.413 & 0.068   \\
KM\_Med & $D_\alpha$ & 1 & 1     & 0.7   & 0.3  & -0.062        & 0.15 & 0.111              & -0.842        & -0.558  & -0.073 & 0.483    & 0.99                    & -2.447 & -0.411 & 0.069   \\
SP\_Mod   & $D_\alpha$ & 1 & 1     & 0.7   & 0.3  & -0.062        & 0.15 & 0.11               & -0.832        & -0.565  & -0.075 & 0.493    & 0.955                   & -2.468 & -0.415 & 0.067   \\
SP\_Med  & $D_\alpha$ & 1 & 1     & 0.7   & 0.3  & -0.066        & 0.15 & 0.11               & -0.838        & -0.603  & -0.079 & 0.491    & 0.956                   & -2.624 & -0.441 & 0.051   \\
KM\_Mod   & $D_\alpha$ & 1 & 3     & 0.7   & 0.3  & -0.042        & 0.15 & 0.112              & -0.752        & -0.379  & -0.056 & 0.487    & 0.999                   & -1.686 & -0.283 & 0.21    \\
KM\_Med & $D_\alpha$ & 1 & 3     & 0.7   & 0.3  & -0.02         & 0.15 & 0.112              & -0.667        & -0.174  & -0.029 & 0.497    & 0.987                   & -0.775 & -0.13  & 0.564   \\
SP\_Mod   & $D_\alpha$ & 1 & 3     & 0.7   & 0.3  & -0.045        & 0.15 & 0.109              & -0.724        & -0.411  & -0.062 & 0.486    & 1                       & -1.778 & -0.299 & 0.186   \\
SP\_Med  & $D_\alpha$ & 1 & 3     & 0.7   & 0.3  & -0.014        & 0.15 & 0.107              & -0.634        & -0.126  & -0.021 & 0.494    & 1.007                   & -0.536 & -0.09  & 0.691   \\
KM\_Mod   & $D_\alpha$ & 1 & 5     & 0.7   & 0.3  & -0.002        & 0.15 & 0.105              & -0.743        & -0.015  & -0.002 & 0.494    & 1.023                   & -0.063 & -0.011 & 0.963   \\
KM\_Med & $D_\alpha$ & 1 & 5     & 0.7   & 0.3  & 0.001         & 0.15 & 0.105              & -0.738        & 0.006   & 0.001  & 0.495    & 1.02                    & 0.026  & 0.004  & 0.984   \\
SP\_Mod   & $D_\alpha$ & 1 & 5     & 0.7   & 0.3  & -0.001        & 0.15 & 0.104              & -0.75         & -0.013  & -0.002 & 0.498    & 1.005                   & -0.053 & -0.009 & 0.968   \\
SP\_Med  & $D_\alpha$ & 1 & 5     & 0.7   & 0.3  & 0.014         & 0.15 & 0.103              & -0.705        & 0.138   & 0.02   & 0.496    & 1.033                   & 0.565  & 0.095  & 0.674   \\
KM\_Mod   & $D_\alpha$ & 1 & 7     & 0.7   & 0.3  & 0.057         & 0.15 & 0.108              & -0.408        & 0.529   & 0.14   & 0.513    & 1.02                    & 2.268  & 0.381  & 0.092   \\
KM\_Med & $D_\alpha$ & 1 & 7     & 0.7   & 0.3  & 0.041         & 0.15 & 0.111              & -0.459        & 0.368   & 0.089  & 0.51     & 1.009                   & 1.623  & 0.273  & 0.228   \\
SP\_Mod   & $D_\alpha$ & 1 & 7     & 0.7   & 0.3  & 0.044         & 0.15 & 0.109              & -0.425        & 0.402   & 0.103  & 0.511    & 1.008                   & 1.741  & 0.292  & 0.196   \\
SP\_Med  & $D_\alpha$ & 1 & 7     & 0.7   & 0.3  & 0.047         & 0.15 & 0.108              & -0.399        & 0.435   & 0.118  & 0.511    & 1.015                   & 1.87   & 0.314  & 0.165   \\
KM\_Mod   & $D_\alpha$ & 3 & 1     & 0.7   & 0.3  & -0.046        & 0.15 & 0.112              & -0.718        & -0.407  & -0.064 & 0.496    & 0.962                   & -1.81  & -0.304 & 0.178   \\
KM\_Med & $D_\alpha$ & 3 & 1     & 0.7   & 0.3  & -0.053        & 0.15 & 0.114              & -0.759        & -0.462  & -0.07  & 0.494    & 0.961                   & -2.095 & -0.352 & 0.119   \\
SP\_Mod   & $D_\alpha$ & 3 & 1     & 0.7   & 0.3  & -0.034        & 0.15 & 0.11               & -0.757        & -0.307  & -0.045 & 0.499    & 0.962                   & -1.343 & -0.226 & 0.318   \\
SP\_Med  & $D_\alpha$ & 3 & 1     & 0.7   & 0.3  & -0.022        & 0.15 & 0.11               & -0.75         & -0.204  & -0.03  & 0.501    & 0.969                   & -0.887 & -0.149 & 0.51    \\
KM\_Mod   & $D_\alpha$ & 3 & 3     & 0.7   & 0.3  & 0.003         & 0.15 & 0.11               & -0.394        & 0.031   & 0.009  & 0.501    & 1                       & 0.136  & 0.023  & 0.92    \\
KM\_Med & $D_\alpha$ & 3 & 3     & 0.7   & 0.3  & 0.004         & 0.15 & 0.11               & -0.335        & 0.032   & 0.01   & 0.502    & 0.995                   & 0.139  & 0.023  & 0.918   \\
SP\_Mod   & $D_\alpha$ & 3 & 3     & 0.7   & 0.3  & -0.021        & 0.15 & 0.107              & -0.594        & -0.198  & -0.036 & 0.492    & 1.007                   & -0.841 & -0.141 & 0.532   \\
SP\_Med  & $D_\alpha$ & 3 & 3     & 0.7   & 0.3  & 0.002         & 0.15 & 0.106              & -0.536        & 0.017   & 0.003  & 0.501    & 0.997                   & 0.071  & 0.012  & 0.958   \\
KM\_Mod   & $D_\alpha$ & 3 & 5     & 0.7   & 0.3  & 0.009         & 0.15 & 0.104              & -0.558        & 0.082   & 0.015  & 0.497    & 1.024                   & 0.34   & 0.057  & 0.8     \\
KM\_Med & $D_\alpha$ & 3 & 5     & 0.7   & 0.3  & 0.034         & 0.15 & 0.104              & -0.482        & 0.327   & 0.071  & 0.503    & 1.029                   & 1.35   & 0.227  & 0.315   \\
SP\_Mod   & $D_\alpha$ & 3 & 5     & 0.7   & 0.3  & 0.017         & 0.15 & 0.101              & -0.58         & 0.165   & 0.029  & 0.501    & 1.015                   & 0.661  & 0.111  & 0.623   \\
SP\_Med  & $D_\alpha$ & 3 & 5     & 0.7   & 0.3  & 0.012         & 0.15 & 0.103              & -0.535        & 0.113   & 0.022  & 0.497    & 1.027                   & 0.459  & 0.077  & 0.733   \\
KM\_Mod   & $D_\alpha$ & 3 & 7     & 0.7   & 0.3  & 0.041         & 0.15 & 0.108              & -0.386        & 0.375   & 0.105  & 0.506    & 1.024                   & 1.614  & 0.271  & 0.231   \\
KM\_Med & $D_\alpha$ & 3 & 7     & 0.7   & 0.3  & 0.03          & 0.15 & 0.114              & -0.567        & 0.263   & 0.053  & 0.513    & 0.984                   & 1.186  & 0.199  & 0.379   \\
SP\_Mod   & $D_\alpha$ & 3 & 7     & 0.7   & 0.3  & 0.055         & 0.15 & 0.109              & -0.426        & 0.499   & 0.128  & 0.514    & 1.012                   & 2.164  & 0.364  & 0.108   \\
SP\_Med  & $D_\alpha$ & 3 & 7     & 0.7   & 0.3  & 0.066         & 0.15 & 0.11               & -0.373        & 0.601   & 0.177  & 0.517    & 1.011                   & 2.613  & 0.439  & 0.053   \\
KM\_Mod   & $D_\alpha$ & 5 & 1     & 0.7   & 0.3  & -0.048        & 0.15 & 0.111              & -0.754        & -0.429  & -0.063 & 0.49     & 0.98                    & -1.897 & -0.319 & 0.159   \\
KM\_Med & $D_\alpha$ & 5 & 1     & 0.7   & 0.3  & -0.056        & 0.15 & 0.113              & -0.771        & -0.497  & -0.073 & 0.497    & 0.943                   & -2.231 & -0.375 & 0.097   \\
SP\_Mod   & $D_\alpha$ & 5 & 1     & 0.7   & 0.3  & -0.036        & 0.15 & 0.108              & -0.721        & -0.337  & -0.051 & 0.498    & 0.965                   & -1.447 & -0.243 & 0.283   \\
SP\_Med  & $D_\alpha$ & 5 & 1     & 0.7   & 0.3  & -0.048        & 0.15 & 0.11               & -0.774        & -0.436  & -0.062 & 0.496    & 0.961                   & -1.898 & -0.319 & 0.158   \\
KM\_Mod   & $D_\alpha$ & 5 & 3     & 0.7   & 0.3  & 0.021         & 0.15 & 0.107              & -0.435        & 0.192   & 0.047  & 0.497    & 1.037                   & 0.817  & 0.137  & 0.544   \\
KM\_Med & $D_\alpha$ & 5 & 3     & 0.7   & 0.3  & 0.025         & 0.15 & 0.109              & -0.335        & 0.226   & 0.073  & 0.505    & 1.01                    & 0.976  & 0.164  & 0.468   \\
SP\_Mod   & $D_\alpha$ & 5 & 3     & 0.7   & 0.3  & 0.011         & 0.15 & 0.104              & -0.511        & 0.107   & 0.022  & 0.498    & 1.02                    & 0.442  & 0.074  & 0.743   \\
SP\_Med  & $D_\alpha$ & 5 & 3     & 0.7   & 0.3  & 0.018         & 0.15 & 0.105              & -0.532        & 0.173   & 0.034  & 0.504    & 1.007                   & 0.722  & 0.121  & 0.592   \\
KM\_Mod   & $D_\alpha$ & 5 & 5     & 0.7   & 0.3  & 0.053         & 0.15 & 0.105              & -0.387        & 0.508   & 0.137  & 0.501    & 1.062                   & 2.108  & 0.354  & 0.117   \\
KM\_Med & $D_\alpha$ & 5 & 5     & 0.7   & 0.3  & 0.068         & 0.15 & 0.104              & -0.424        & 0.655   & 0.16   & 0.508    & 1.054                   & 2.695  & 0.453  & 0.044   \\
SP\_Mod   & $D_\alpha$ & 5 & 5     & 0.7   & 0.3  & 0.048         & 0.15 & 0.103              & -0.443        & 0.471   & 0.109  & 0.501    & 1.056                   & 1.916  & 0.322  & 0.154   \\
SP\_Med  & $D_\alpha$ & 5 & 5     & 0.7   & 0.3  & 0.081         & 0.15 & 0.102              & -0.366        & 0.8     & 0.222  & 0.506    & 1.075                   & 3.231  & 0.543  & 0.016   \\
KM\_Mod   & $D_\alpha$ & 5 & 7     & 0.7   & 0.3  & 0.092         & 0.15 & 0.106              & -0.308        & 0.872   & 0.3    & 0.511    & 1.074                   & 3.669  & 0.616  & 0.006   \\
KM\_Med & $D_\alpha$ & 5 & 7     & 0.7   & 0.3  & 0.066         & 0.15 & 0.111              & -0.397        & 0.597   & 0.167  & 0.511    & 1.04                    & 2.627  & 0.441  & 0.051   \\
SP\_Mod   & $D_\alpha$ & 5 & 7     & 0.7   & 0.3  & 0.09          & 0.15 & 0.107              & -0.339        & 0.842   & 0.265  & 0.52     & 1.031                   & 3.561  & 0.598  & 0.008   \\
SP\_Med  & $D_\alpha$ & 5 & 7     & 0.7   & 0.3  & 0.136         & 0.15 & 0.105              & -0.303        & 1.288   & 0.448  & 0.524    & 1.07                    & 5.387  & 0.905  & 0       \\
KM\_Mod   & $D_\alpha$ & 7 & 1     & 0.7   & 0.3  & -0.031        & 0.15 & 0.111              & -0.608        & -0.28   & -0.051 & 0.494    & 0.986                   & -1.234 & -0.207 & 0.359   \\
KM\_Med & $D_\alpha$ & 7 & 1     & 0.7   & 0.3  & -0.033        & 0.15 & 0.114              & -0.603        & -0.293  & -0.055 & 0.501    & 0.954                   & -1.328 & -0.223 & 0.323   \\
SP\_Mod   & $D_\alpha$ & 7 & 1     & 0.7   & 0.3  & -0.025        & 0.15 & 0.109              & -0.656        & -0.225  & -0.037 & 0.497    & 0.982                   & -0.973 & -0.163 & 0.47    \\
SP\_Med  & $D_\alpha$ & 7 & 1     & 0.7   & 0.3  & -0.009        & 0.15 & 0.107              & -0.611        & -0.08   & -0.014 & 0.497    & 1.003                   & -0.34  & -0.057 & 0.8     \\
KM\_Mod   & $D_\alpha$ & 7 & 3     & 0.7   & 0.3  & 0.039         & 0.15 & 0.106              & -0.379        & 0.37    & 0.103  & 0.498    & 1.058                   & 1.555  & 0.261  & 0.247   \\
KM\_Med & $D_\alpha$ & 7 & 3     & 0.7   & 0.3  & 0.045         & 0.15 & 0.107              & -0.332        & 0.426   & 0.137  & 0.504    & 1.04                    & 1.804  & 0.303  & 0.18    \\
SP\_Mod   & $D_\alpha$ & 7 & 3     & 0.7   & 0.3  & 0.054         & 0.15 & 0.104              & -0.409        & 0.523   & 0.132  & 0.503    & 1.056                   & 2.147  & 0.361  & 0.11    \\
SP\_Med  & $D_\alpha$ & 7 & 3     & 0.7   & 0.3  & 0.064         & 0.15 & 0.103              & -0.376        & 0.62    & 0.17   & 0.507    & 1.049                   & 2.542  & 0.427  & 0.058   \\
KM\_Mod   & $D_\alpha$ & 7 & 5     & 0.7   & 0.3  & 0.031         & 0.15 & 0.108              & -0.348        & 0.285   & 0.088  & 0.501    & 1.034                   & 1.219  & 0.205  & 0.365   \\
KM\_Med & $D_\alpha$ & 7 & 5     & 0.7   & 0.3  & 0.025         & 0.15 & 0.109              & -0.395        & 0.226   & 0.062  & 0.5      & 1.029                   & 0.977  & 0.164  & 0.468   \\
SP\_Mod   & $D_\alpha$ & 7 & 5     & 0.7   & 0.3  & 0.049         & 0.15 & 0.104              & -0.398        & 0.468   & 0.122  & 0.51     & 1.02                    & 1.932  & 0.325  & 0.151   \\
SP\_Med  & $D_\alpha$ & 7 & 5     & 0.7   & 0.3  & 0.046         & 0.15 & 0.107              & -0.43         & 0.428   & 0.106  & 0.504    & 1.038                   & 1.812  & 0.304  & 0.178   \\
KM\_Mod   & $D_\alpha$ & 7 & 7     & 0.7   & 0.3  & 0.116         & 0.15 & 0.105              & -0.207        & 1.099   & 0.559  & 0.51     & 1.107                   & 4.596  & 0.772  & 0.001   \\
KM\_Med & $D_\alpha$ & 7 & 7     & 0.7   & 0.3  & 0.094         & 0.15 & 0.109              & -0.198        & 0.866   & 0.476  & 0.515    & 1.058                   & 3.741  & 0.629  & 0.005   \\
SP\_Mod   & $D_\alpha$ & 7 & 7     & 0.7   & 0.3  & 0.139         & 0.15 & 0.105              & -0.276        & 1.333   & 0.505  & 0.524    & 1.074                   & 5.532  & 0.929  & 0       \\
SP\_Med  & $D_\alpha$ & 7 & 7     & 0.7   & 0.3  & 0.142         & 0.15 & 0.104              & -0.221        & 1.367   & 0.644  & 0.527    & 1.067                   & 5.648  & 0.949  & 0       \\
CCF              & $D_\alpha$ & 1 & 1     & 0.85  & 0.15 & -0.065        & 0.15 & 0.109              & -0.857        & -0.596  & -0.076 & 0.489    & 0.967                   & -2.577 & -0.433 & 0.056   \\
CCF              & $D_\alpha$ & 1 & 3     & 0.85  & 0.15 & -0.062        & 0.15 & 0.111              & -0.811        & -0.561  & -0.077 & 0.486    & 0.982                   & -2.471 & -0.415 & 0.066   \\
CCF              & $D_\alpha$ & 1 & 5     & 0.85  & 0.15 & 0.017         & 0.15 & 0.102              & -0.705        & 0.165   & 0.024  & 0.5      & 1.021                   & 0.67   & 0.113  & 0.618   \\
CCF              & $D_\alpha$ & 1 & 7     & 0.85  & 0.15 & 0.007         & 0.15 & 0.113              & -0.578        & 0.064   & 0.013  & 0.509    & 0.973                   & 0.288  & 0.048  & 0.83    \\
CCF              & $D_\alpha$ & 3 & 1     & 0.85  & 0.15 & -0.041        & 0.15 & 0.111              & -0.771        & -0.373  & -0.054 & 0.498    & 0.959                   & -1.638 & -0.275 & 0.223   \\
CCF              & $D_\alpha$ & 3 & 3     & 0.85  & 0.15 & -0.002        & 0.15 & 0.106              & -0.573        & -0.017  & -0.003 & 0.499    & 1.004                   & -0.071 & -0.012 & 0.958   \\
CCF              & $D_\alpha$ & 3 & 5     & 0.85  & 0.15 & 0.015         & 0.15 & 0.1                & -0.564        & 0.149   & 0.026  & 0.494    & 1.042                   & 0.588  & 0.099  & 0.662   \\
CCF              & $D_\alpha$ & 3 & 7     & 0.85  & 0.15 & 0.034         & 0.15 & 0.11               & -0.449        & 0.307   & 0.076  & 0.514    & 0.986                   & 1.347  & 0.226  & 0.318   \\
CCF              & $D_\alpha$ & 5 & 1     & 0.85  & 0.15 & -0.011        & 0.15 & 0.107              & -0.7          & -0.107  & -0.016 & 0.499    & 0.991                   & -0.453 & -0.076 & 0.737   \\
CCF              & $D_\alpha$ & 5 & 3     & 0.85  & 0.15 & -0.015        & 0.15 & 0.106              & -0.643        & -0.142  & -0.023 & 0.493    & 1.009                   & -0.596 & -0.1   & 0.658   \\
CCF              & $D_\alpha$ & 5 & 5     & 0.85  & 0.15 & 0.05          & 0.15 & 0.104              & -0.351        & 0.479   & 0.142  & 0.502    & 1.054                   & 1.973  & 0.331  & 0.142   \\
CCF              & $D_\alpha$ & 5 & 7     & 0.85  & 0.15 & 0.078         & 0.15 & 0.106              & -0.517        & 0.732   & 0.15   & 0.515    & 1.036                   & 3.077  & 0.517  & 0.022   \\
CCF              & $D_\alpha$ & 7 & 1     & 0.85  & 0.15 & -0.02         & 0.15 & 0.109              & -0.622        & -0.184  & -0.032 & 0.499    & 0.981                   & -0.795 & -0.134 & 0.555   \\
CCF              & $D_\alpha$ & 7 & 3     & 0.85  & 0.15 & 0.039         & 0.15 & 0.106              & -0.394        & 0.369   & 0.099  & 0.505    & 1.029                   & 1.546  & 0.26   & 0.25    \\
CCF              & $D_\alpha$ & 7 & 5     & 0.85  & 0.15 & 0.043         & 0.15 & 0.106              & -0.327        & 0.403   & 0.13   & 0.509    & 1.018                   & 1.691  & 0.284  & 0.209   \\
CCF              & $D_\alpha$ & 7 & 7     & 0.85  & 0.15 & 0.106         & 0.15 & 0.105              & -0.254        & 1.009   & 0.418  & 0.52     & 1.048                   & 4.209  & 0.707  & 0.002   \\
CCF              & $D_\alpha$ & 1 & 1     & 0.8   & 0.2  & -0.058        & 0.15 & 0.109              & -0.85         & -0.532  & -0.068 & 0.491    & 0.967                   & -2.294 & -0.385 & 0.089   \\
CCF              & $D_\alpha$ & 1 & 3     & 0.8   & 0.2  & -0.055        & 0.15 & 0.111              & -0.771        & -0.495  & -0.071 & 0.486    & 0.988                   & -2.182 & -0.367 & 0.104   \\
CCF              & $D_\alpha$ & 1 & 5     & 0.8   & 0.2  & 0.002         & 0.15 & 0.103              & -0.742        & 0.015   & 0.002  & 0.496    & 1.018                   & 0.06   & 0.01   & 0.965   \\
CCF              & $D_\alpha$ & 1 & 7     & 0.8   & 0.2  & 0.03          & 0.15 & 0.111              & -0.577        & 0.269   & 0.052  & 0.513    & 0.983                   & 1.184  & 0.199  & 0.379   \\
CCF              & $D_\alpha$ & 3 & 1     & 0.8   & 0.2  & -0.049        & 0.15 & 0.112              & -0.791        & -0.436  & -0.061 & 0.497    & 0.955                   & -1.93  & -0.324 & 0.151   \\
CCF              & $D_\alpha$ & 3 & 3     & 0.8   & 0.2  & 0.001         & 0.15 & 0.106              & -0.548        & 0.007   & 0.001  & 0.499    & 1.006                   & 0.029  & 0.005  & 0.983   \\
CCF              & $D_\alpha$ & 3 & 5     & 0.8   & 0.2  & 0.009         & 0.15 & 0.101              & -0.607        & 0.091   & 0.015  & 0.493    & 1.039                   & 0.366  & 0.061  & 0.786   \\
CCF              & $D_\alpha$ & 3 & 7     & 0.8   & 0.2  & 0.057         & 0.15 & 0.109              & -0.402        & 0.529   & 0.143  & 0.52     & 0.991                   & 2.281  & 0.383  & 0.09    \\
CCF              & $D_\alpha$ & 5 & 1     & 0.8   & 0.2  & -0.018        & 0.15 & 0.107              & -0.724        & -0.168  & -0.025 & 0.499    & 0.981                   & -0.716 & -0.12  & 0.595   \\
CCF              & $D_\alpha$ & 5 & 3     & 0.8   & 0.2  & -0.024        & 0.15 & 0.106              & -0.681        & -0.229  & -0.036 & 0.491    & 1.007                   & -0.96  & -0.161 & 0.476   \\
CCF              & $D_\alpha$ & 5 & 5     & 0.8   & 0.2  & 0.041         & 0.15 & 0.104              & -0.45         & 0.393   & 0.09   & 0.497    & 1.062                   & 1.613  & 0.271  & 0.23    \\
CCF              & $D_\alpha$ & 5 & 7     & 0.8   & 0.2  & 0.074         & 0.15 & 0.107              & -0.472        & 0.696   & 0.157  & 0.516    & 1.025                   & 2.946  & 0.495  & 0.029   \\
CCF              & $D_\alpha$ & 7 & 1     & 0.8   & 0.2  & -0.033        & 0.15 & 0.11               & -0.717        & -0.3    & -0.046 & 0.496    & 0.977                   & -1.31  & -0.22  & 0.33    \\
CCF              & $D_\alpha$ & 7 & 3     & 0.8   & 0.2  & 0.046         & 0.15 & 0.105              & -0.417        & 0.434   & 0.11   & 0.506    & 1.031                   & 1.812  & 0.304  & 0.178   \\
CCF              & $D_\alpha$ & 7 & 5     & 0.8   & 0.2  & 0.04          & 0.15 & 0.106              & -0.404        & 0.379   & 0.1    & 0.506    & 1.023                   & 1.599  & 0.269  & 0.235   \\
CCF              & $D_\alpha$ & 7 & 7     & 0.8   & 0.2  & 0.108         & 0.15 & 0.105              & -0.254        & 1.027   & 0.425  & 0.521    & 1.047                   & 4.288  & 0.72   & 0.001   \\
CCF              & $D_\alpha$ & 1 & 1     & 0.75  & 0.25 & -0.063        & 0.15 & 0.109              & -0.871        & -0.578  & -0.073 & 0.493    & 0.952                   & -2.51  & -0.422 & 0.062   \\
CCF              & $D_\alpha$ & 1 & 3     & 0.75  & 0.25 & -0.054        & 0.15 & 0.112              & -0.769        & -0.482  & -0.07  & 0.488    & 0.983                   & -2.141 & -0.36  & 0.111   \\
CCF              & $D_\alpha$ & 1 & 5     & 0.75  & 0.25 & 0.005         & 0.15 & 0.102              & -0.698        & 0.045   & 0.007  & 0.497    & 1.018                   & 0.181  & 0.03   & 0.893   \\
CCF              & $D_\alpha$ & 1 & 7     & 0.75  & 0.25 & 0.052         & 0.15 & 0.11               & -0.442        & 0.474   & 0.117  & 0.514    & 1.005                   & 2.059  & 0.346  & 0.127   \\
CCF              & $D_\alpha$ & 3 & 1     & 0.75  & 0.25 & -0.048        & 0.15 & 0.112              & -0.797        & -0.423  & -0.06  & 0.499    & 0.947                   & -1.886 & -0.317 & 0.161   \\
CCF              & $D_\alpha$ & 3 & 3     & 0.75  & 0.25 & 0.004         & 0.15 & 0.106              & -0.546        & 0.038   & 0.007  & 0.498    & 1.012                   & 0.161  & 0.027  & 0.905   \\
CCF              & $D_\alpha$ & 3 & 5     & 0.75  & 0.25 & 0.026         & 0.15 & 0.1                & -0.505        & 0.259   & 0.051  & 0.495    & 1.051                   & 1.024  & 0.172  & 0.446   \\
CCF              & $D_\alpha$ & 3 & 7     & 0.75  & 0.25 & 0.074         & 0.15 & 0.109              & -0.349        & 0.679   & 0.211  & 0.524    & 0.994                   & 2.927  & 0.492  & 0.03    \\
CCF              & $D_\alpha$ & 5 & 1     & 0.75  & 0.25 & -0.022        & 0.15 & 0.107              & -0.723        & -0.203  & -0.03  & 0.498    & 0.98                    & -0.865 & -0.145 & 0.521   \\
CCF              & $D_\alpha$ & 5 & 3     & 0.75  & 0.25 & -0.032        & 0.15 & 0.106              & -0.69         & -0.306  & -0.047 & 0.488    & 1.01                    & -1.284 & -0.216 & 0.341   \\
CCF              & $D_\alpha$ & 5 & 5     & 0.75  & 0.25 & 0.029         & 0.15 & 0.104              & -0.544        & 0.282   & 0.054  & 0.497    & 1.051                   & 1.169  & 0.196  & 0.385   \\
CCF              & $D_\alpha$ & 5 & 7     & 0.75  & 0.25 & 0.073         & 0.15 & 0.108              & -0.47         & 0.677   & 0.155  & 0.516    & 1.026                   & 2.895  & 0.486  & 0.032   \\
CCF              & $D_\alpha$ & 7 & 1     & 0.75  & 0.25 & -0.043        & 0.15 & 0.11               & -0.766        & -0.39   & -0.056 & 0.492    & 0.978                   & -1.707 & -0.287 & 0.204   \\
CCF              & $D_\alpha$ & 7 & 3     & 0.75  & 0.25 & 0.049         & 0.15 & 0.105              & -0.419        & 0.468   & 0.117  & 0.504    & 1.046                   & 1.942  & 0.326  & 0.148   \\
CCF              & $D_\alpha$ & 7 & 5     & 0.75  & 0.25 & 0.04          & 0.15 & 0.106              & -0.439        & 0.375   & 0.091  & 0.503    & 1.036                   & 1.581  & 0.266  & 0.24    \\
CCF              & $D_\alpha$ & 7 & 7     & 0.75  & 0.25 & 0.101         & 0.15 & 0.105              & -0.288        & 0.964   & 0.352  & 0.518    & 1.05                    & 4.018  & 0.675  & 0.003   \\
CCF              & $D_\alpha$ & 1 & 1     & 0.7   & 0.3  & -0.066        & 0.15 & 0.11               & -0.875        & -0.6    & -0.075 & 0.49     & 0.961                   & -2.619 & -0.44  & 0.052   \\
CCF              & $D_\alpha$ & 1 & 3     & 0.7   & 0.3  & -0.056        & 0.15 & 0.111              & -0.785        & -0.508  & -0.072 & 0.484    & 0.994                   & -2.242 & -0.377 & 0.095   \\
CCF              & $D_\alpha$ & 1 & 5     & 0.7   & 0.3  & 0.009         & 0.15 & 0.101              & -0.71         & 0.092   & 0.013  & 0.497    & 1.025                   & 0.372  & 0.062  & 0.782   \\
CCF              & $D_\alpha$ & 1 & 7     & 0.7   & 0.3  & 0.042         & 0.15 & 0.11               & -0.423        & 0.38    & 0.099  & 0.513    & 1                       & 1.665  & 0.28   & 0.217   \\
CCF              & $D_\alpha$ & 3 & 1     & 0.7   & 0.3  & -0.04         & 0.15 & 0.112              & -0.774        & -0.354  & -0.052 & 0.501    & 0.95                    & -1.582 & -0.266 & 0.239   \\
CCF              & $D_\alpha$ & 3 & 3     & 0.7   & 0.3  & -0.012        & 0.15 & 0.106              & -0.548        & -0.11   & -0.021 & 0.496    & 1.001                   & -0.461 & -0.077 & 0.732   \\
CCF              & $D_\alpha$ & 3 & 5     & 0.7   & 0.3  & 0.018         & 0.15 & 0.101              & -0.599        & 0.18    & 0.03   & 0.494    & 1.049                   & 0.723  & 0.121  & 0.591   \\
CCF              & $D_\alpha$ & 3 & 7     & 0.7   & 0.3  & 0.073         & 0.15 & 0.109              & -0.325        & 0.675   & 0.226  & 0.525    & 0.99                    & 2.91   & 0.489  & 0.031   \\
CCF              & $D_\alpha$ & 5 & 1     & 0.7   & 0.3  & -0.013        & 0.15 & 0.107              & -0.672        & -0.117  & -0.019 & 0.501    & 0.979                   & -0.498 & -0.084 & 0.711   \\
CCF              & $D_\alpha$ & 5 & 3     & 0.7   & 0.3  & -0.019        & 0.15 & 0.106              & -0.615        & -0.182  & -0.031 & 0.492    & 1.007                   & -0.767 & -0.129 & 0.569   \\
CCF              & $D_\alpha$ & 5 & 5     & 0.7   & 0.3  & 0.046         & 0.15 & 0.104              & -0.455        & 0.439   & 0.1    & 0.497    & 1.069                   & 1.814  & 0.305  & 0.177   \\
CCF              & $D_\alpha$ & 5 & 7     & 0.7   & 0.3  & 0.071         & 0.15 & 0.107              & -0.42         & 0.662   & 0.169  & 0.516    & 1.022                   & 2.818  & 0.473  & 0.036   \\
CCF              & $D_\alpha$ & 7 & 1     & 0.7   & 0.3  & -0.058        & 0.15 & 0.111              & -0.812        & -0.519  & -0.071 & 0.491    & 0.967                   & -2.286 & -0.384 & 0.089   \\
CCF              & $D_\alpha$ & 7 & 3     & 0.7   & 0.3  & 0.045         & 0.15 & 0.105              & -0.469        & 0.428   & 0.096  & 0.505    & 1.036                   & 1.787  & 0.3    & 0.184   \\
CCF              & $D_\alpha$ & 7 & 5     & 0.7   & 0.3  & 0.031         & 0.15 & 0.107              & -0.444        & 0.289   & 0.069  & 0.499    & 1.041                   & 1.222  & 0.205  & 0.364   \\
CCF              & $D_\alpha$ & 7 & 7     & 0.7   & 0.3  & 0.088         & 0.15 & 0.106              & -0.267        & 0.824   & 0.328  & 0.517    & 1.037                   & 3.473  & 0.583  & 0.01   \\




\end{longtable}
\end{small}









\subsection*{ETF data set: performance metrics for the entire grid -  rescaled to target volatility}
\label{etf_full_results}

% Table \ref{tab: etf_grid} provides performance metrics for the entire grid (rescaled to target volatility). The experiment has
% been set with the values $p = \{1,3,5,7\}$, $\delta = \{1,3,5,7\}$, and $\alpha = \{0.75,0.85\}$.

\begin{small}
\captionof{table}*{Table S2: ETF data set: performance metrics for the entire grid - rescaled to target volatility. The experiment has
been set with the values $p = \{1,3,5,7\}$, $\delta = \{1,3,5,7\}$, and $\alpha = \{0.75,0.85\}$.}
\label{tab: etf_grid}
\begin{longtable}{|p{2.9cm}p{1.2cm}p{0.1cm}p{0.1cm}p{0.5cm}p{0.5cm}p{1.4cm}p{1.2cm}p{1.6cm}p{1.7cm}p{1cm}p{1cm}p{0.5cm}p{1.2cm}p{1.4cm}p{0.9cm}p{1.5cm}|}
\toprule
\textbf{Method}       & \textbf{Strategy}   & \textbf{$p$} & \textbf{$\delta$} & \textbf{$\alpha$} & \textbf{$\beta$} & \textbf{E[Returns]} & \textbf{Volatility}  & \textbf{Downside deviation} & \textbf{Maximum drawdown} & \textbf{Sortino ratio} & \textbf{Calmar ratio} & \textbf{Hit rate} & \textbf{$\frac{\text{Avg. profit}}{\text{Avg. loss}}$} & \textbf{PnL per trade}  & \textbf{Sharpe ratio} & \textbf{P-value} \\
\midrule
KM\_Mod   & $G_\beta$ & 1 & 1     & 0.85  & 0.15 & -0.086        & 0.15 & 0.118              & -0.733        & -0.729  & -0.117 & 0.484    & 0.956                   & -3.41  & -0.573 & 0.037   \\
KM\_Med & $G_\beta$ & 1 & 1     & 0.85  & 0.15 & -0.071        & 0.15 & 0.114              & -0.707        & -0.621  & -0.1   & 0.49     & 0.952                   & -2.817 & -0.473 & 0.087   \\
SP\_Mod    & $G_\beta$ & 1 & 1     & 0.85  & 0.15 & 0.027         & 0.15 & 0.109              & -0.474        & 0.246   & 0.057  & 0.508    & 1.001                   & 1.065  & 0.179  & 0.517   \\
SP\_Med  & $G_\beta$ & 1 & 1     & 0.85  & 0.15 & -0.003        & 0.15 & 0.118              & -0.332        & -0.024  & -0.008 & 0.503    & 0.985                   & -0.111 & -0.019 & 0.946   \\
KM\_Mod   & $G_\beta$ & 1 & 3     & 0.85  & 0.15 & -0.017        & 0.15 & 0.103              & -0.495        & -0.162  & -0.034 & 0.487    & 1.032                   & -0.666 & -0.112 & 0.686   \\
KM\_Med & $G_\beta$ & 1 & 3     & 0.85  & 0.15 & 0.036         & 0.15 & 0.104              & -0.316        & 0.347   & 0.115  & 0.504    & 1.032                   & 1.437  & 0.241  & 0.381   \\
SP\_Mod    & $G_\beta$ & 1 & 3     & 0.85  & 0.15 & -0.038        & 0.15 & 0.118              & -0.659        & -0.321  & -0.058 & 0.485    & 1.011                   & -1.506 & -0.253 & 0.357   \\
SP\_Med  & $G_\beta$ & 1 & 3     & 0.85  & 0.15 & 0.045         & 0.15 & 0.112              & -0.337        & 0.402   & 0.134  & 0.507    & 1.032                   & 1.786  & 0.3    & 0.278   \\
KM\_Mod   & $G_\beta$ & 1 & 5     & 0.85  & 0.15 & 0.026         & 0.15 & 0.107              & -0.355        & 0.246   & 0.074  & 0.502    & 1.026                   & 1.045  & 0.176  & 0.525   \\
KM\_Med & $G_\beta$ & 1 & 5     & 0.85  & 0.15 & 0.024         & 0.15 & 0.114              & -0.484        & 0.208   & 0.049  & 0.507    & 1.001                   & 0.939  & 0.158  & 0.569   \\
SP\_Mod    & $G_\beta$ & 1 & 5     & 0.85  & 0.15 & -0.002        & 0.15 & 0.111              & -0.493        & -0.022  & -0.005 & 0.503    & 0.984                   & -0.098 & -0.016 & 0.953   \\
SP\_Med  & $G_\beta$ & 1 & 5     & 0.85  & 0.15 & -0.029        & 0.15 & 0.117              & -0.489        & -0.248  & -0.059 & 0.502    & 0.955                   & -1.147 & -0.193 & 0.486   \\
KM\_Mod   & $G_\beta$ & 1 & 7     & 0.85  & 0.15 & -0.046        & 0.15 & 0.119              & -0.699        & -0.387  & -0.066 & 0.503    & 0.934                   & -1.821 & -0.306 & 0.267   \\
KM\_Med & $G_\beta$ & 1 & 7     & 0.85  & 0.15 & 0.017         & 0.15 & 0.118              & -0.417        & 0.145   & 0.041  & 0.506    & 0.999                   & 0.678  & 0.114  & 0.681   \\
SP\_Mod    & $G_\beta$ & 1 & 7     & 0.85  & 0.15 & 0.01          & 0.15 & 0.116              & -0.489        & 0.083   & 0.02   & 0.508    & 0.98                    & 0.382  & 0.064  & 0.817   \\
SP\_Med  & $G_\beta$ & 1 & 7     & 0.85  & 0.15 & -0.005        & 0.15 & 0.107              & -0.478        & -0.046  & -0.01  & 0.499    & 0.999                   & -0.197 & -0.033 & 0.905   \\
KM\_Mod   & $G_\beta$ & 3 & 1     & 0.85  & 0.15 & -0.003        & 0.15 & 0.112              & -0.415        & -0.03   & -0.008 & 0.49     & 1.038                   & -0.133 & -0.022 & 0.936   \\
KM\_Med & $G_\beta$ & 3 & 1     & 0.85  & 0.15 & -0.055        & 0.15 & 0.11               & -0.659        & -0.497  & -0.083 & 0.482    & 1.001                   & -2.176 & -0.366 & 0.187   \\
SP\_Mod    & $G_\beta$ & 3 & 1     & 0.85  & 0.15 & -0.079        & 0.15 & 0.119              & -0.743        & -0.666  & -0.107 & 0.493    & 0.93                    & -3.144 & -0.528 & 0.054   \\
SP\_Med  & $G_\beta$ & 3 & 1     & 0.85  & 0.15 & -0.008        & 0.15 & 0.119              & -0.535        & -0.067  & -0.015 & 0.486    & 1.048                   & -0.318 & -0.053 & 0.847   \\
KM\_Mod   & $G_\beta$ & 3 & 3     & 0.85  & 0.15 & 0.004         & 0.15 & 0.107              & -0.493        & 0.038   & 0.008  & 0.494    & 1.031                   & 0.162  & 0.027  & 0.922   \\
KM\_Med & $G_\beta$ & 3 & 3     & 0.85  & 0.15 & 0.05          & 0.15 & 0.109              & -0.295        & 0.462   & 0.171  & 0.509    & 1.027                   & 2.001  & 0.336  & 0.224   \\
SP\_Mod    & $G_\beta$ & 3 & 3     & 0.85  & 0.15 & 0.029         & 0.15 & 0.119              & -0.347        & 0.242   & 0.083  & 0.498    & 1.048                   & 1.144  & 0.192  & 0.49    \\
SP\_Med  & $G_\beta$ & 3 & 3     & 0.85  & 0.15 & 0.037         & 0.15 & 0.112              & -0.395        & 0.328   & 0.093  & 0.507    & 1.018                   & 1.452  & 0.244  & 0.377   \\
KM\_Mod   & $G_\beta$ & 3 & 5     & 0.85  & 0.15 & 0.015         & 0.15 & 0.106              & -0.378        & 0.139   & 0.039  & 0.495    & 1.038                   & 0.584  & 0.098  & 0.723   \\
KM\_Med & $G_\beta$ & 3 & 5     & 0.85  & 0.15 & 0.054         & 0.15 & 0.113              & -0.474        & 0.482   & 0.115  & 0.509    & 1.032                   & 2.156  & 0.362  & 0.191   \\
SP\_Mod    & $G_\beta$ & 3 & 5     & 0.85  & 0.15 & -0.068        & 0.15 & 0.116              & -0.744        & -0.581  & -0.091 & 0.496    & 0.932                   & -2.681 & -0.45  & 0.103   \\
SP\_Med  & $G_\beta$ & 3 & 5     & 0.85  & 0.15 & -0.048        & 0.15 & 0.122              & -0.631        & -0.395  & -0.076 & 0.498    & 0.948                   & -1.906 & -0.32  & 0.244   \\
KM\_Mod   & $G_\beta$ & 3 & 7     & 0.85  & 0.15 & -0.068        & 0.15 & 0.122              & -0.752        & -0.552  & -0.09  & 0.502    & 0.913                   & -2.68  & -0.45  & 0.1     \\
KM\_Med & $G_\beta$ & 3 & 7     & 0.85  & 0.15 & 0.045         & 0.15 & 0.113              & -0.374        & 0.396   & 0.12   & 0.511    & 1.014                   & 1.779  & 0.299  & 0.28    \\
SP\_Mod    & $G_\beta$ & 3 & 7     & 0.85  & 0.15 & -0.005        & 0.15 & 0.113              & -0.507        & -0.045  & -0.01  & 0.507    & 0.966                   & -0.203 & -0.034 & 0.902   \\
SP\_Med  & $G_\beta$ & 3 & 7     & 0.85  & 0.15 & -0.022        & 0.15 & 0.108              & -0.59         & -0.203  & -0.037 & 0.495    & 0.995                   & -0.867 & -0.146 & 0.599   \\
KM\_Mod   & $G_\beta$ & 5 & 1     & 0.85  & 0.15 & -0.047        & 0.15 & 0.114              & -0.665        & -0.409  & -0.07  & 0.49     & 0.982                   & -1.846 & -0.31  & 0.261   \\
KM\_Med & $G_\beta$ & 5 & 1     & 0.85  & 0.15 & -0.038        & 0.15 & 0.109              & -0.529        & -0.348  & -0.072 & 0.487    & 1.006                   & -1.506 & -0.253 & 0.361   \\
SP\_Mod    & $G_\beta$ & 5 & 1     & 0.85  & 0.15 & -0.006        & 0.15 & 0.115              & -0.443        & -0.051  & -0.013 & 0.499    & 0.996                   & -0.235 & -0.039 & 0.886   \\
SP\_Med  & $G_\beta$ & 5 & 1     & 0.85  & 0.15 & 0.014         & 0.15 & 0.116              & -0.451        & 0.119   & 0.031  & 0.491    & 1.055                   & 0.548  & 0.092  & 0.739   \\
KM\_Mod   & $G_\beta$ & 5 & 3     & 0.85  & 0.15 & 0.014         & 0.15 & 0.107              & -0.569        & 0.132   & 0.025  & 0.498    & 1.025                   & 0.558  & 0.094  & 0.735   \\
KM\_Med & $G_\beta$ & 5 & 3     & 0.85  & 0.15 & 0.062         & 0.15 & 0.109              & -0.265        & 0.571   & 0.235  & 0.512    & 1.032                   & 2.474  & 0.416  & 0.133   \\
SP\_Mod    & $G_\beta$ & 5 & 3     & 0.85  & 0.15 & 0.024         & 0.15 & 0.121              & -0.43         & 0.202   & 0.057  & 0.505    & 1.01                    & 0.97   & 0.163  & 0.558   \\
SP\_Med  & $G_\beta$ & 5 & 3     & 0.85  & 0.15 & 0.092         & 0.15 & 0.109              & -0.264        & 0.844   & 0.347  & 0.521    & 1.036                   & 3.637  & 0.611  & 0.026   \\
KM\_Mod   & $G_\beta$ & 5 & 5     & 0.85  & 0.15 & 0.038         & 0.15 & 0.103              & -0.445        & 0.366   & 0.085  & 0.496    & 1.065                   & 1.503  & 0.252  & 0.359   \\
KM\_Med & $G_\beta$ & 5 & 5     & 0.85  & 0.15 & 0.066         & 0.15 & 0.109              & -0.389        & 0.606   & 0.17   & 0.501    & 1.084                   & 2.629  & 0.442  & 0.11    \\
SP\_Mod    & $G_\beta$ & 5 & 5     & 0.85  & 0.15 & -0.092        & 0.15 & 0.113              & -0.742        & -0.817  & -0.125 & 0.491    & 0.923                   & -3.668 & -0.616 & 0.027   \\
SP\_Med  & $G_\beta$ & 5 & 5     & 0.85  & 0.15 & -0.084        & 0.15 & 0.124              & -0.745        & -0.679  & -0.113 & 0.489    & 0.939                   & -3.339 & -0.561 & 0.04    \\
KM\_Mod   & $G_\beta$ & 5 & 7     & 0.85  & 0.15 & -0.034        & 0.15 & 0.12               & -0.619        & -0.287  & -0.056 & 0.505    & 0.939                   & -1.364 & -0.229 & 0.405   \\
KM\_Med & $G_\beta$ & 5 & 7     & 0.85  & 0.15 & 0.05          & 0.15 & 0.108              & -0.329        & 0.46    & 0.151  & 0.51     & 1.023                   & 1.969  & 0.331  & 0.23    \\
SP\_Mod    & $G_\beta$ & 5 & 7     & 0.85  & 0.15 & -0.033        & 0.15 & 0.114              & -0.495        & -0.288  & -0.067 & 0.5      & 0.958                   & -1.308 & -0.22  & 0.426   \\
SP\_Med  & $G_\beta$ & 5 & 7     & 0.85  & 0.15 & 0.019         & 0.15 & 0.108              & -0.296        & 0.178   & 0.065  & 0.505    & 1.002                   & 0.767  & 0.129  & 0.641   \\
KM\_Mod   & $G_\beta$ & 7 & 1     & 0.85  & 0.15 & -0.003        & 0.15 & 0.112              & -0.497        & -0.026  & -0.006 & 0.498    & 1.004                   & -0.116 & -0.02  & 0.944   \\
KM\_Med & $G_\beta$ & 7 & 1     & 0.85  & 0.15 & -0.035        & 0.15 & 0.11               & -0.482        & -0.317  & -0.073 & 0.486    & 1.013                   & -1.387 & -0.233 & 0.4     \\
SP\_Mod    & $G_\beta$ & 7 & 1     & 0.85  & 0.15 & -0.012        & 0.15 & 0.116              & -0.549        & -0.105  & -0.022 & 0.504    & 0.969                   & -0.487 & -0.082 & 0.767   \\
SP\_Med  & $G_\beta$ & 7 & 1     & 0.85  & 0.15 & -0.018        & 0.15 & 0.115              & -0.633        & -0.153  & -0.028 & 0.481    & 1.053                   & -0.698 & -0.117 & 0.671   \\
KM\_Mod   & $G_\beta$ & 7 & 3     & 0.85  & 0.15 & -0.009        & 0.15 & 0.109              & -0.573        & -0.08   & -0.015 & 0.497    & 1.003                   & -0.345 & -0.058 & 0.834   \\
KM\_Med & $G_\beta$ & 7 & 3     & 0.85  & 0.15 & 0.039         & 0.15 & 0.11               & -0.385        & 0.355   & 0.101  & 0.51     & 1.01                    & 1.543  & 0.259  & 0.348   \\
SP\_Mod    & $G_\beta$ & 7 & 3     & 0.85  & 0.15 & 0.043         & 0.15 & 0.119              & -0.335        & 0.362   & 0.128  & 0.51     & 1.015                   & 1.707  & 0.287  & 0.304   \\
SP\_Med  & $G_\beta$ & 7 & 3     & 0.85  & 0.15 & 0.058         & 0.15 & 0.112              & -0.351        & 0.519   & 0.166  & 0.512    & 1.026                   & 2.312  & 0.388  & 0.16    \\
KM\_Mod   & $G_\beta$ & 7 & 5     & 0.85  & 0.15 & 0.059         & 0.15 & 0.104              & -0.385        & 0.567   & 0.153  & 0.501    & 1.074                   & 2.341  & 0.393  & 0.153   \\
KM\_Med & $G_\beta$ & 7 & 5     & 0.85  & 0.15 & 0.069         & 0.15 & 0.112              & -0.392        & 0.622   & 0.177  & 0.508    & 1.058                   & 2.753  & 0.462  & 0.095   \\
SP\_Mod    & $G_\beta$ & 7 & 5     & 0.85  & 0.15 & -0.067        & 0.15 & 0.112              & -0.693        & -0.596  & -0.096 & 0.488    & 0.963                   & -2.643 & -0.444 & 0.111   \\
SP\_Med  & $G_\beta$ & 7 & 5     & 0.85  & 0.15 & -0.079        & 0.15 & 0.123              & -0.718        & -0.643  & -0.11  & 0.491    & 0.939                   & -3.135 & -0.527 & 0.054   \\
KM\_Mod   & $G_\beta$ & 7 & 7     & 0.85  & 0.15 & -0.06         & 0.15 & 0.122              & -0.707        & -0.487  & -0.084 & 0.505    & 0.911                   & -2.363 & -0.397 & 0.147   \\
KM\_Med & $G_\beta$ & 7 & 7     & 0.85  & 0.15 & 0.004         & 0.15 & 0.113              & -0.436        & 0.031   & 0.008  & 0.505    & 0.984                   & 0.14   & 0.024  & 0.932   \\
SP\_Mod    & $G_\beta$ & 7 & 7     & 0.85  & 0.15 & -0.076        & 0.15 & 0.118              & -0.726        & -0.648  & -0.105 & 0.497    & 0.918                   & -3.035 & -0.51  & 0.064   \\
SP\_Med  & $G_\beta$ & 7 & 7     & 0.85  & 0.15 & -0.025        & 0.15 & 0.11               & -0.452        & -0.232  & -0.056 & 0.495    & 0.987                   & -1.01  & -0.17  & 0.54    \\
KM\_Mod   & $G_\beta$ & 1 & 1     & 0.75  & 0.25 & -0.085        & 0.15 & 0.114              & -0.741        & -0.745  & -0.114 & 0.484    & 0.96                    & -3.36  & -0.564 & 0.041   \\
KM\_Med & $G_\beta$ & 1 & 1     & 0.75  & 0.25 & -0.06         & 0.15 & 0.112              & -0.658        & -0.537  & -0.091 & 0.493    & 0.954                   & -2.383 & -0.4   & 0.149   \\
SP\_Mod    & $G_\beta$ & 1 & 1     & 0.75  & 0.25 & -0.034        & 0.15 & 0.111              & -0.564        & -0.308  & -0.061 & 0.502    & 0.95                    & -1.356 & -0.228 & 0.41    \\
SP\_Med  & $G_\beta$ & 1 & 1     & 0.75  & 0.25 & -0.031        & 0.15 & 0.117              & -0.462        & -0.261  & -0.066 & 0.493    & 0.99                    & -1.216 & -0.204 & 0.459   \\
KM\_Mod   & $G_\beta$ & 1 & 3     & 0.75  & 0.25 & -0.028        & 0.15 & 0.111              & -0.618        & -0.252  & -0.045 & 0.488    & 1.012                   & -1.106 & -0.186 & 0.501   \\
KM\_Med & $G_\beta$ & 1 & 3     & 0.75  & 0.25 & -0.023        & 0.15 & 0.11               & -0.577        & -0.212  & -0.04  & 0.495    & 0.991                   & -0.924 & -0.155 & 0.575   \\
SP\_Mod    & $G_\beta$ & 1 & 3     & 0.75  & 0.25 & -0.013        & 0.15 & 0.119              & -0.606        & -0.113  & -0.022 & 0.495    & 1.004                   & -0.535 & -0.09  & 0.745   \\
SP\_Med  & $G_\beta$ & 1 & 3     & 0.75  & 0.25 & 0.103         & 0.15 & 0.106              & -0.263        & 0.968   & 0.39   & 0.512    & 1.084                   & 4.073  & 0.684  & 0.013   \\
KM\_Mod   & $G_\beta$ & 1 & 5     & 0.75  & 0.25 & 0.06          & 0.15 & 0.102              & -0.373        & 0.586   & 0.161  & 0.502    & 1.068                   & 2.378  & 0.399  & 0.146   \\
KM\_Med & $G_\beta$ & 1 & 5     & 0.75  & 0.25 & -0.0          & 0.15 & 0.114              & -0.512        & -0.001  & -0.0   & 0.503    & 0.987                   & -0.006 & -0.001 & 0.997   \\
SP\_Mod    & $G_\beta$ & 1 & 5     & 0.75  & 0.25 & -0.002        & 0.15 & 0.109              & -0.498        & -0.018  & -0.004 & 0.498    & 1.006                   & -0.08  & -0.013 & 0.961   \\
SP\_Med  & $G_\beta$ & 1 & 5     & 0.75  & 0.25 & -0.024        & 0.15 & 0.116              & -0.608        & -0.208  & -0.04  & 0.508    & 0.939                   & -0.961 & -0.161 & 0.559   \\
KM\_Mod   & $G_\beta$ & 1 & 7     & 0.75  & 0.25 & 0.047         & 0.15 & 0.116              & -0.481        & 0.402   & 0.097  & 0.519    & 0.982                   & 1.853  & 0.311  & 0.263   \\
KM\_Med & $G_\beta$ & 1 & 7     & 0.75  & 0.25 & -0.003        & 0.15 & 0.118              & -0.484        & -0.024  & -0.006 & 0.491    & 1.031                   & -0.11  & -0.019 & 0.946   \\
SP\_Mod    & $G_\beta$ & 1 & 7     & 0.75  & 0.25 & 0.025         & 0.15 & 0.112              & -0.453        & 0.226   & 0.056  & 0.506    & 1.006                   & 1.007  & 0.169  & 0.541   \\
SP\_Med  & $G_\beta$ & 1 & 7     & 0.75  & 0.25 & 0.021         & 0.15 & 0.105              & -0.348        & 0.199   & 0.06   & 0.495    & 1.048                   & 0.828  & 0.139  & 0.614   \\
KM\_Mod   & $G_\beta$ & 3 & 1     & 0.75  & 0.25 & -0.039        & 0.15 & 0.11               & -0.531        & -0.354  & -0.073 & 0.49     & 0.992                   & -1.542 & -0.259 & 0.349   \\
KM\_Med & $G_\beta$ & 3 & 1     & 0.75  & 0.25 & -0.062        & 0.15 & 0.111              & -0.648        & -0.558  & -0.096 & 0.486    & 0.98                    & -2.461 & -0.414 & 0.135   \\
SP\_Mod    & $G_\beta$ & 3 & 1     & 0.75  & 0.25 & -0.079        & 0.15 & 0.114              & -0.753        & -0.69   & -0.105 & 0.494    & 0.93                    & -3.126 & -0.525 & 0.057   \\
SP\_Med  & $G_\beta$ & 3 & 1     & 0.75  & 0.25 & 0.021         & 0.15 & 0.112              & -0.417        & 0.183   & 0.049  & 0.498    & 1.033                   & 0.818  & 0.138  & 0.619   \\
KM\_Mod   & $G_\beta$ & 3 & 3     & 0.75  & 0.25 & 0.013         & 0.15 & 0.109              & -0.489        & 0.116   & 0.026  & 0.493    & 1.046                   & 0.505  & 0.085  & 0.759   \\
KM\_Med & $G_\beta$ & 3 & 3     & 0.75  & 0.25 & 0.005         & 0.15 & 0.108              & -0.475        & 0.042   & 0.01   & 0.498    & 1.014                   & 0.18   & 0.03   & 0.913   \\
SP\_Mod    & $G_\beta$ & 3 & 3     & 0.75  & 0.25 & -0.029        & 0.15 & 0.12               & -0.64         & -0.243  & -0.045 & 0.492    & 0.994                   & -1.151 & -0.193 & 0.482   \\
SP\_Med  & $G_\beta$ & 3 & 3     & 0.75  & 0.25 & 0.078         & 0.15 & 0.108              & -0.391        & 0.718   & 0.199  & 0.504    & 1.086                   & 3.083  & 0.518  & 0.061   \\
KM\_Mod   & $G_\beta$ & 3 & 5     & 0.75  & 0.25 & 0.003         & 0.15 & 0.103              & -0.461        & 0.028   & 0.006  & 0.492    & 1.037                   & 0.113  & 0.019  & 0.945   \\
KM\_Med & $G_\beta$ & 3 & 5     & 0.75  & 0.25 & 0.051         & 0.15 & 0.112              & -0.382        & 0.457   & 0.134  & 0.517    & 0.998                   & 2.033  & 0.341  & 0.217   \\
SP\_Mod    & $G_\beta$ & 3 & 5     & 0.75  & 0.25 & -0.037        & 0.15 & 0.112              & -0.698        & -0.329  & -0.053 & 0.493    & 0.982                   & -1.464 & -0.246 & 0.374   \\
SP\_Med  & $G_\beta$ & 3 & 5     & 0.75  & 0.25 & -0.045        & 0.15 & 0.121              & -0.727        & -0.368  & -0.061 & 0.497    & 0.957                   & -1.774 & -0.298 & 0.279   \\
KM\_Mod   & $G_\beta$ & 3 & 7     & 0.75  & 0.25 & 0.062         & 0.15 & 0.117              & -0.459        & 0.53    & 0.135  & 0.524    & 0.981                   & 2.454  & 0.412  & 0.14    \\
KM\_Med & $G_\beta$ & 3 & 7     & 0.75  & 0.25 & 0.064         & 0.15 & 0.113              & -0.397        & 0.561   & 0.16   & 0.502    & 1.075                   & 2.527  & 0.425  & 0.126   \\
SP\_Mod    & $G_\beta$ & 3 & 7     & 0.75  & 0.25 & 0.012         & 0.15 & 0.11               & -0.433        & 0.112   & 0.028  & 0.506    & 0.992                   & 0.488  & 0.082  & 0.767   \\
SP\_Med  & $G_\beta$ & 3 & 7     & 0.75  & 0.25 & -0.008        & 0.15 & 0.114              & -0.433        & -0.073  & -0.019 & 0.506    & 0.966                   & -0.333 & -0.056 & 0.84    \\
KM\_Mod   & $G_\beta$ & 5 & 1     & 0.75  & 0.25 & -0.02         & 0.15 & 0.11               & -0.544        & -0.178  & -0.036 & 0.494    & 1.0                     & -0.776 & -0.13  & 0.637   \\
KM\_Med & $G_\beta$ & 5 & 1     & 0.75  & 0.25 & -0.113        & 0.15 & 0.115              & -0.811        & -0.98   & -0.139 & 0.488    & 0.91                    & -4.473 & -0.751 & 0.006   \\
SP\_Mod    & $G_\beta$ & 5 & 1     & 0.75  & 0.25 & -0.044        & 0.15 & 0.112              & -0.659        & -0.397  & -0.067 & 0.491    & 0.981                   & -1.759 & -0.296 & 0.285   \\
SP\_Med  & $G_\beta$ & 5 & 1     & 0.75  & 0.25 & 0.027         & 0.15 & 0.112              & -0.371        & 0.239   & 0.072  & 0.502    & 1.025                   & 1.062  & 0.178  & 0.519   \\
KM\_Mod   & $G_\beta$ & 5 & 3     & 0.75  & 0.25 & 0.037         & 0.15 & 0.107              & -0.488        & 0.343   & 0.075  & 0.494    & 1.073                   & 1.462  & 0.246  & 0.375   \\
KM\_Med & $G_\beta$ & 5 & 3     & 0.75  & 0.25 & 0.034         & 0.15 & 0.109              & -0.353        & 0.308   & 0.095  & 0.511    & 0.998                   & 1.332  & 0.224  & 0.418   \\
SP\_Mod    & $G_\beta$ & 5 & 3     & 0.75  & 0.25 & 0.039         & 0.15 & 0.117              & -0.317        & 0.331   & 0.122  & 0.506    & 1.025                   & 1.535  & 0.258  & 0.354   \\
SP\_Med  & $G_\beta$ & 5 & 3     & 0.75  & 0.25 & 0.112         & 0.15 & 0.107              & -0.284        & 1.042   & 0.394  & 0.516    & 1.079                   & 4.442  & 0.746  & 0.007   \\
KM\_Mod   & $G_\beta$ & 5 & 5     & 0.75  & 0.25 & 0.027         & 0.15 & 0.103              & -0.33         & 0.258   & 0.081  & 0.5      & 1.033                   & 1.055  & 0.177  & 0.52    \\
KM\_Med & $G_\beta$ & 5 & 5     & 0.75  & 0.25 & 0.0           & 0.15 & 0.117              & -0.52         & 0.001   & 0.0    & 0.504    & 0.986                   & 0.004  & 0.001  & 0.998   \\
SP\_Mod    & $G_\beta$ & 5 & 5     & 0.75  & 0.25 & -0.019        & 0.15 & 0.104              & -0.565        & -0.18   & -0.033 & 0.493    & 1.003                   & -0.739 & -0.124 & 0.654   \\
SP\_Med  & $G_\beta$ & 5 & 5     & 0.75  & 0.25 & -0.071        & 0.15 & 0.122              & -0.782        & -0.585  & -0.091 & 0.495    & 0.933                   & -2.83  & -0.475 & 0.083   \\
KM\_Mod   & $G_\beta$ & 5 & 7     & 0.75  & 0.25 & 0.066         & 0.15 & 0.117              & -0.493        & 0.563   & 0.134  & 0.519    & 1.004                   & 2.612  & 0.439  & 0.116   \\
KM\_Med & $G_\beta$ & 5 & 7     & 0.75  & 0.25 & 0.062         & 0.15 & 0.116              & -0.348        & 0.532   & 0.178  & 0.508    & 1.051                   & 2.459  & 0.413  & 0.138   \\
SP\_Mod    & $G_\beta$ & 5 & 7     & 0.75  & 0.25 & -0.011        & 0.15 & 0.114              & -0.564        & -0.093  & -0.019 & 0.501    & 0.982                   & -0.418 & -0.07  & 0.799   \\
SP\_Med  & $G_\beta$ & 5 & 7     & 0.75  & 0.25 & 0.009         & 0.15 & 0.115              & -0.424        & 0.076   & 0.021  & 0.508    & 0.981                   & 0.347  & 0.058  & 0.833   \\
KM\_Mod   & $G_\beta$ & 7 & 1     & 0.75  & 0.25 & -0.042        & 0.15 & 0.112              & -0.643        & -0.374  & -0.065 & 0.496    & 0.966                   & -1.668 & -0.28  & 0.311   \\
KM\_Med & $G_\beta$ & 7 & 1     & 0.75  & 0.25 & -0.05         & 0.15 & 0.115              & -0.608        & -0.434  & -0.082 & 0.502    & 0.934                   & -1.975 & -0.332 & 0.229   \\
SP\_Mod    & $G_\beta$ & 7 & 1     & 0.75  & 0.25 & -0.012        & 0.15 & 0.111              & -0.542        & -0.112  & -0.023 & 0.494    & 1.009                   & -0.493 & -0.083 & 0.765   \\
SP\_Med  & $G_\beta$ & 7 & 1     & 0.75  & 0.25 & -0.01         & 0.15 & 0.112              & -0.646        & -0.091  & -0.016 & 0.491    & 1.021                   & -0.405 & -0.068 & 0.806   \\
KM\_Mod   & $G_\beta$ & 7 & 3     & 0.75  & 0.25 & -0.01         & 0.15 & 0.107              & -0.577        & -0.097  & -0.018 & 0.489    & 1.033                   & -0.41  & -0.069 & 0.803   \\
KM\_Med & $G_\beta$ & 7 & 3     & 0.75  & 0.25 & 0.002         & 0.15 & 0.109              & -0.524        & 0.021   & 0.004  & 0.506    & 0.98                    & 0.092  & 0.015  & 0.955   \\
SP\_Mod    & $G_\beta$ & 7 & 3     & 0.75  & 0.25 & -0.012        & 0.15 & 0.118              & -0.603        & -0.106  & -0.021 & 0.495    & 1.005                   & -0.495 & -0.083 & 0.763   \\
SP\_Med  & $G_\beta$ & 7 & 3     & 0.75  & 0.25 & 0.065         & 0.15 & 0.109              & -0.476        & 0.597   & 0.137  & 0.507    & 1.057                   & 2.59   & 0.435  & 0.115   \\
KM\_Mod   & $G_\beta$ & 7 & 5     & 0.75  & 0.25 & 0.033         & 0.15 & 0.105              & -0.389        & 0.309   & 0.084  & 0.498    & 1.049                   & 1.29   & 0.217  & 0.433   \\
KM\_Med & $G_\beta$ & 7 & 5     & 0.75  & 0.25 & 0.047         & 0.15 & 0.108              & -0.333        & 0.439   & 0.142  & 0.501    & 1.058                   & 1.882  & 0.316  & 0.252   \\
SP\_Mod    & $G_\beta$ & 7 & 5     & 0.75  & 0.25 & -0.007        & 0.15 & 0.105              & -0.467        & -0.064  & -0.014 & 0.498    & 0.998                   & -0.268 & -0.045 & 0.871   \\
SP\_Med  & $G_\beta$ & 7 & 5     & 0.75  & 0.25 & -0.041        & 0.15 & 0.117              & -0.722        & -0.354  & -0.057 & 0.493    & 0.974                   & -1.644 & -0.276 & 0.317   \\
KM\_Mod   & $G_\beta$ & 7 & 7     & 0.75  & 0.25 & 0.02          & 0.15 & 0.115              & -0.525        & 0.176   & 0.038  & 0.512    & 0.978                   & 0.8    & 0.134  & 0.628   \\
KM\_Med & $G_\beta$ & 7 & 7     & 0.75  & 0.25 & 0.022         & 0.15 & 0.116              & -0.465        & 0.188   & 0.047  & 0.499    & 1.034                   & 0.87   & 0.146  & 0.598   \\
SP\_Mod    & $G_\beta$ & 7 & 7     & 0.75  & 0.25 & -0.005        & 0.15 & 0.113              & -0.579        & -0.043  & -0.008 & 0.503    & 0.983                   & -0.191 & -0.032 & 0.908   \\
SP\_Med  & $G_\beta$ & 7 & 7     & 0.75  & 0.25 & 0.013         & 0.15 & 0.108              & -0.369        & 0.122   & 0.036  & 0.5      & 1.016                   & 0.527  & 0.088  & 0.749   \\
CCF              & $G_\beta$ & 1 & 1     & 0.85  & 0.15 & 0.033         & 0.15 & 0.122              & -0.45         & 0.269   & 0.073  & 0.518    & 0.969                   & 1.302  & 0.219  & 0.432   \\
CCF              & $G_\beta$ & 1 & 3     & 0.85  & 0.15 & 0.012         & 0.15 & 0.113              & -0.505        & 0.102   & 0.023  & 0.507    & 0.988                   & 0.458  & 0.077  & 0.781   \\
CCF              & $G_\beta$ & 1 & 5     & 0.85  & 0.15 & -0.013        & 0.15 & 0.117              & -0.449        & -0.109  & -0.028 & 0.498    & 0.99                    & -0.508 & -0.085 & 0.758   \\
CCF              & $G_\beta$ & 1 & 7     & 0.85  & 0.15 & -0.041        & 0.15 & 0.114              & -0.641        & -0.364  & -0.065 & 0.496    & 0.964                   & -1.642 & -0.276 & 0.319   \\
CCF              & $G_\beta$ & 3 & 1     & 0.85  & 0.15 & -0.04         & 0.15 & 0.123              & -0.592        & -0.329  & -0.068 & 0.5      & 0.95                    & -1.601 & -0.269 & 0.328   \\
CCF              & $G_\beta$ & 3 & 3     & 0.85  & 0.15 & 0.069         & 0.15 & 0.11               & -0.329        & 0.628   & 0.21   & 0.51     & 1.046                   & 2.738  & 0.46   & 0.096   \\
CCF              & $G_\beta$ & 3 & 5     & 0.85  & 0.15 & -0.049        & 0.15 & 0.116              & -0.614        & -0.425  & -0.08  & 0.488    & 0.988                   & -1.947 & -0.327 & 0.236   \\
CCF              & $G_\beta$ & 3 & 7     & 0.85  & 0.15 & -0.052        & 0.15 & 0.12               & -0.644        & -0.436  & -0.081 & 0.499    & 0.939                   & -2.077 & -0.349 & 0.205   \\
CCF              & $G_\beta$ & 5 & 1     & 0.85  & 0.15 & -0.042        & 0.15 & 0.126              & -0.666        & -0.336  & -0.063 & 0.505    & 0.929                   & -1.674 & -0.281 & 0.305   \\
CCF              & $G_\beta$ & 5 & 3     & 0.85  & 0.15 & 0.031         & 0.15 & 0.11               & -0.393        & 0.281   & 0.078  & 0.504    & 1.024                   & 1.222  & 0.205  & 0.458   \\
CCF              & $G_\beta$ & 5 & 5     & 0.85  & 0.15 & -0.009        & 0.15 & 0.114              & -0.377        & -0.078  & -0.023 & 0.493    & 1.017                   & -0.351 & -0.059 & 0.831   \\
CCF              & $G_\beta$ & 5 & 7     & 0.85  & 0.15 & -0.019        & 0.15 & 0.115              & -0.571        & -0.163  & -0.033 & 0.502    & 0.968                   & -0.743 & -0.125 & 0.652   \\
CCF              & $G_\beta$ & 7 & 1     & 0.85  & 0.15 & -0.046        & 0.15 & 0.122              & -0.573        & -0.377  & -0.08  & 0.495    & 0.963                   & -1.828 & -0.307 & 0.264   \\
CCF              & $G_\beta$ & 7 & 3     & 0.85  & 0.15 & 0.065         & 0.15 & 0.108              & -0.433        & 0.607   & 0.151  & 0.511    & 1.04                    & 2.594  & 0.436  & 0.115   \\
CCF              & $G_\beta$ & 7 & 5     & 0.85  & 0.15 & -0.017        & 0.15 & 0.109              & -0.442        & -0.157  & -0.039 & 0.492    & 1.01                    & -0.678 & -0.114 & 0.681   \\
CCF              & $G_\beta$ & 7 & 7     & 0.85  & 0.15 & -0.038        & 0.15 & 0.116              & -0.672        & -0.324  & -0.056 & 0.501    & 0.949                   & -1.49  & -0.25  & 0.365   \\
CCF              & $G_\beta$ & 1 & 1     & 0.75  & 0.25 & 0.035         & 0.15 & 0.11               & -0.312        & 0.318   & 0.112  & 0.512    & 0.997                   & 1.388  & 0.233  & 0.399   \\
CCF              & $G_\beta$ & 1 & 3     & 0.75  & 0.25 & 0.004         & 0.15 & 0.112              & -0.609        & 0.032   & 0.006  & 0.501    & 1.002                   & 0.143  & 0.024  & 0.931   \\
CCF              & $G_\beta$ & 1 & 5     & 0.75  & 0.25 & -0.002        & 0.15 & 0.116              & -0.399        & -0.019  & -0.006 & 0.505    & 0.978                   & -0.088 & -0.015 & 0.957   \\
CCF              & $G_\beta$ & 1 & 7     & 0.75  & 0.25 & 0.029         & 0.15 & 0.111              & -0.432        & 0.265   & 0.068  & 0.505    & 1.02                    & 1.164  & 0.196  & 0.479   \\
CCF              & $G_\beta$ & 3 & 1     & 0.75  & 0.25 & -0.032        & 0.15 & 0.115              & -0.536        & -0.282  & -0.06  & 0.5      & 0.96                    & -1.286 & -0.216 & 0.434   \\
CCF              & $G_\beta$ & 3 & 3     & 0.75  & 0.25 & -0.008        & 0.15 & 0.114              & -0.576        & -0.072  & -0.014 & 0.499    & 0.994                   & -0.329 & -0.055 & 0.842   \\
CCF              & $G_\beta$ & 3 & 5     & 0.75  & 0.25 & -0.026        & 0.15 & 0.113              & -0.541        & -0.228  & -0.048 & 0.49     & 1.006                   & -1.023 & -0.172 & 0.534   \\
CCF              & $G_\beta$ & 3 & 7     & 0.75  & 0.25 & -0.02         & 0.15 & 0.118              & -0.504        & -0.166  & -0.039 & 0.502    & 0.969                   & -0.778 & -0.131 & 0.636   \\
CCF              & $G_\beta$ & 5 & 1     & 0.75  & 0.25 & -0.059        & 0.15 & 0.121              & -0.705        & -0.488  & -0.084 & 0.5      & 0.93                    & -2.343 & -0.394 & 0.151   \\
CCF              & $G_\beta$ & 5 & 3     & 0.75  & 0.25 & 0.03          & 0.15 & 0.111              & -0.444        & 0.275   & 0.068  & 0.5      & 1.038                   & 1.205  & 0.202  & 0.465   \\
CCF              & $G_\beta$ & 5 & 5     & 0.75  & 0.25 & -0.047        & 0.15 & 0.115              & -0.609        & -0.404  & -0.076 & 0.5      & 0.944                   & -1.847 & -0.31  & 0.261   \\
CCF              & $G_\beta$ & 5 & 7     & 0.75  & 0.25 & 0.039         & 0.15 & 0.113              & -0.491        & 0.345   & 0.079  & 0.498    & 1.059                   & 1.546  & 0.26   & 0.348   \\
CCF              & $G_\beta$ & 7 & 1     & 0.75  & 0.25 & -0.053        & 0.15 & 0.119              & -0.663        & -0.449  & -0.08  & 0.504    & 0.922                   & -2.114 & -0.355 & 0.196   \\
CCF              & $G_\beta$ & 7 & 3     & 0.75  & 0.25 & 0.019         & 0.15 & 0.114              & -0.501        & 0.166   & 0.038  & 0.503    & 1.012                   & 0.748  & 0.126  & 0.65    \\
CCF              & $G_\beta$ & 7 & 5     & 0.75  & 0.25 & -0.069        & 0.15 & 0.118              & -0.682        & -0.59   & -0.102 & 0.492    & 0.945                   & -2.757 & -0.463 & 0.092   \\
CCF              & $G_\beta$ & 7 & 7     & 0.75  & 0.25 & -0.019        & 0.15 & 0.116              & -0.668        & -0.165  & -0.029 & 0.492    & 1.006                   & -0.76  & -0.128 & 0.644  \\
\hline 

KM\_Mod   & $D_\alpha$ & 1 & 1     & 0.85  & 0.15 & -0.133        & 0.15 & 0.115              & -0.862        & -1.158  & -0.155 & 0.466    & 0.974                   & -5.293 & -0.889 & 0.001   \\
KM\_Med & $D_\alpha$ & 1 & 1     & 0.85  & 0.15 & -0.123        & 0.15 & 0.118              & -0.832        & -1.04   & -0.148 & 0.471    & 0.963                   & -4.871 & -0.818 & 0.002   \\
SP\_Mod    & $D_\alpha$ & 1 & 1     & 0.85  & 0.15 & -0.116        & 0.15 & 0.12               & -0.849        & -0.965  & -0.137 & 0.477    & 0.947                   & -4.612 & -0.775 & 0.004   \\
SP\_Med  & $D_\alpha$ & 1 & 1     & 0.85  & 0.15 & -0.124        & 0.15 & 0.117              & -0.848        & -1.061  & -0.146 & 0.468    & 0.974                   & -4.922 & -0.827 & 0.002   \\
KM\_Mod   & $D_\alpha$ & 1 & 3     & 0.85  & 0.15 & 0.008         & 0.15 & 0.119              & -0.364        & 0.066   & 0.022  & 0.511    & 0.968                   & 0.312  & 0.052  & 0.85    \\
KM\_Med & $D_\alpha$ & 1 & 3     & 0.85  & 0.15 & 0.014         & 0.15 & 0.119              & -0.404        & 0.118   & 0.035  & 0.508    & 0.986                   & 0.561  & 0.094  & 0.734   \\
SP\_Mod    & $D_\alpha$ & 1 & 3     & 0.85  & 0.15 & 0.017         & 0.15 & 0.114              & -0.442        & 0.146   & 0.038  & 0.508    & 0.988                   & 0.662  & 0.111  & 0.688   \\
SP\_Med  & $D_\alpha$ & 1 & 3     & 0.85  & 0.15 & 0.02          & 0.15 & 0.119              & -0.405        & 0.172   & 0.051  & 0.512    & 0.975                   & 0.812  & 0.136  & 0.624   \\
KM\_Mod   & $D_\alpha$ & 1 & 5     & 0.85  & 0.15 & -0.04         & 0.15 & 0.121              & -0.648        & -0.332  & -0.062 & 0.492    & 0.981                   & -1.593 & -0.268 & 0.327   \\
KM\_Med & $D_\alpha$ & 1 & 5     & 0.85  & 0.15 & -0.054        & 0.15 & 0.114              & -0.641        & -0.469  & -0.084 & 0.49     & 0.975                   & -2.127 & -0.357 & 0.193   \\
SP\_Mod    & $D_\alpha$ & 1 & 5     & 0.85  & 0.15 & 0.013         & 0.15 & 0.118              & -0.511        & 0.107   & 0.025  & 0.507    & 0.986                   & 0.501  & 0.084  & 0.761   \\
SP\_Med  & $D_\alpha$ & 1 & 5     & 0.85  & 0.15 & 0.011         & 0.15 & 0.115              & -0.482        & 0.095   & 0.023  & 0.505    & 0.993                   & 0.434  & 0.073  & 0.793   \\
KM\_Mod   & $D_\alpha$ & 1 & 7     & 0.85  & 0.15 & 0.041         & 0.15 & 0.099              & -0.306        & 0.409   & 0.133  & 0.499    & 1.055                   & 1.61   & 0.271  & 0.32    \\
KM\_Med & $D_\alpha$ & 1 & 7     & 0.85  & 0.15 & 0.035         & 0.15 & 0.105              & -0.377        & 0.337   & 0.094  & 0.503    & 1.03                    & 1.404  & 0.236  & 0.392   \\
SP\_Mod    & $D_\alpha$ & 1 & 7     & 0.85  & 0.15 & 0.017         & 0.15 & 0.101              & -0.333        & 0.171   & 0.052  & 0.5      & 1.02                    & 0.686  & 0.115  & 0.676   \\
SP\_Med  & $D_\alpha$ & 1 & 7     & 0.85  & 0.15 & 0.035         & 0.15 & 0.104              & -0.334        & 0.334   & 0.104  & 0.507    & 1.015                   & 1.377  & 0.231  & 0.401   \\
KM\_Mod   & $D_\alpha$ & 3 & 1     & 0.85  & 0.15 & -0.125        & 0.15 & 0.115              & -0.852        & -1.086  & -0.147 & 0.481    & 0.928                   & -4.963 & -0.834 & 0.002   \\
KM\_Med & $D_\alpha$ & 3 & 1     & 0.85  & 0.15 & -0.137        & 0.15 & 0.121              & -0.868        & -1.136  & -0.158 & 0.478    & 0.922                   & -5.442 & -0.914 & 0.001   \\
SP\_Mod    & $D_\alpha$ & 3 & 1     & 0.85  & 0.15 & -0.054        & 0.15 & 0.119              & -0.729        & -0.454  & -0.074 & 0.5      & 0.935                   & -2.147 & -0.361 & 0.187   \\
SP\_Med  & $D_\alpha$ & 3 & 1     & 0.85  & 0.15 & -0.065        & 0.15 & 0.119              & -0.733        & -0.544  & -0.088 & 0.488    & 0.97                    & -2.56  & -0.43  & 0.115   \\
KM\_Mod   & $D_\alpha$ & 3 & 3     & 0.85  & 0.15 & 0.057         & 0.15 & 0.112              & -0.286        & 0.504   & 0.198  & 0.513    & 1.018                   & 2.249  & 0.378  & 0.176   \\
KM\_Med & $D_\alpha$ & 3 & 3     & 0.85  & 0.15 & 0.04          & 0.15 & 0.115              & -0.307        & 0.343   & 0.129  & 0.508    & 1.017                   & 1.571  & 0.264  & 0.345   \\
SP\_Mod    & $D_\alpha$ & 3 & 3     & 0.85  & 0.15 & -0.004        & 0.15 & 0.119              & -0.465        & -0.035  & -0.009 & 0.515    & 0.935                   & -0.166 & -0.028 & 0.92    \\
SP\_Med  & $D_\alpha$ & 3 & 3     & 0.85  & 0.15 & -0.013        & 0.15 & 0.116              & -0.495        & -0.109  & -0.026 & 0.502    & 0.979                   & -0.502 & -0.084 & 0.76    \\
KM\_Mod   & $D_\alpha$ & 3 & 5     & 0.85  & 0.15 & -0.028        & 0.15 & 0.117              & -0.622        & -0.237  & -0.045 & 0.495    & 0.984                   & -1.101 & -0.185 & 0.501   \\
KM\_Med & $D_\alpha$ & 3 & 5     & 0.85  & 0.15 & -0.031        & 0.15 & 0.114              & -0.605        & -0.271  & -0.051 & 0.498    & 0.97                    & -1.228 & -0.206 & 0.454   \\
SP\_Mod    & $D_\alpha$ & 3 & 5     & 0.85  & 0.15 & 0.029         & 0.15 & 0.11               & -0.387        & 0.262   & 0.074  & 0.506    & 1.011                   & 1.142  & 0.192  & 0.489   \\
SP\_Med  & $D_\alpha$ & 3 & 5     & 0.85  & 0.15 & 0.035         & 0.15 & 0.111              & -0.477        & 0.32    & 0.074  & 0.509    & 1.008                   & 1.404  & 0.236  & 0.396   \\
KM\_Mod   & $D_\alpha$ & 3 & 7     & 0.85  & 0.15 & 0.057         & 0.15 & 0.1                & -0.291        & 0.567   & 0.195  & 0.505    & 1.053                   & 2.247  & 0.377  & 0.163   \\
KM\_Med & $D_\alpha$ & 3 & 7     & 0.85  & 0.15 & 0.047         & 0.15 & 0.105              & -0.495        & 0.448   & 0.095  & 0.51     & 1.019                   & 1.867  & 0.314  & 0.254   \\
SP\_Mod    & $D_\alpha$ & 3 & 7     & 0.85  & 0.15 & 0.05          & 0.15 & 0.101              & -0.333        & 0.497   & 0.151  & 0.517    & 0.995                   & 2.0    & 0.336  & 0.219   \\
SP\_Med  & $D_\alpha$ & 3 & 7     & 0.85  & 0.15 & 0.052         & 0.15 & 0.104              & -0.365        & 0.499   & 0.142  & 0.509    & 1.028                   & 2.053  & 0.345  & 0.209   \\
KM\_Mod   & $D_\alpha$ & 5 & 1     & 0.85  & 0.15 & -0.113        & 0.15 & 0.117              & -0.838        & -0.97   & -0.135 & 0.48     & 0.944                   & -4.5   & -0.756 & 0.006   \\
KM\_Med & $D_\alpha$ & 5 & 1     & 0.85  & 0.15 & -0.092        & 0.15 & 0.123              & -0.771        & -0.745  & -0.119 & 0.492    & 0.92                    & -3.648 & -0.613 & 0.022   \\
SP\_Mod    & $D_\alpha$ & 5 & 1     & 0.85  & 0.15 & -0.097        & 0.15 & 0.121              & -0.781        & -0.799  & -0.124 & 0.493    & 0.911                   & -3.84  & -0.645 & 0.017   \\
SP\_Med  & $D_\alpha$ & 5 & 1     & 0.85  & 0.15 & -0.106        & 0.15 & 0.122              & -0.802        & -0.869  & -0.132 & 0.487    & 0.926                   & -4.193 & -0.704 & 0.009   \\
KM\_Mod   & $D_\alpha$ & 5 & 3     & 0.85  & 0.15 & 0.035         & 0.15 & 0.116              & -0.365        & 0.3     & 0.095  & 0.508    & 1.012                   & 1.38   & 0.232  & 0.406   \\
KM\_Med & $D_\alpha$ & 5 & 3     & 0.85  & 0.15 & -0.011        & 0.15 & 0.115              & -0.488        & -0.095  & -0.022 & 0.492    & 1.017                   & -0.435 & -0.073 & 0.791   \\
SP\_Mod    & $D_\alpha$ & 5 & 3     & 0.85  & 0.15 & 0.055         & 0.15 & 0.11               & -0.344        & 0.501   & 0.16   & 0.512    & 1.018                   & 2.186  & 0.367  & 0.186   \\
SP\_Med  & $D_\alpha$ & 5 & 3     & 0.85  & 0.15 & 0.019         & 0.15 & 0.116              & -0.407        & 0.162   & 0.046  & 0.505    & 1.002                   & 0.746  & 0.125  & 0.652   \\
KM\_Mod   & $D_\alpha$ & 5 & 5     & 0.85  & 0.15 & -0.049        & 0.15 & 0.12               & -0.644        & -0.411  & -0.076 & 0.496    & 0.957                   & -1.953 & -0.328 & 0.23    \\
KM\_Med & $D_\alpha$ & 5 & 5     & 0.85  & 0.15 & -0.057        & 0.15 & 0.116              & -0.656        & -0.491  & -0.087 & 0.493    & 0.958                   & -2.254 & -0.379 & 0.167   \\
SP\_Mod    & $D_\alpha$ & 5 & 5     & 0.85  & 0.15 & -0.006        & 0.15 & 0.106              & -0.39         & -0.053  & -0.014 & 0.498    & 1.0                     & -0.224 & -0.038 & 0.892   \\
SP\_Med  & $D_\alpha$ & 5 & 5     & 0.85  & 0.15 & -0.017        & 0.15 & 0.11               & -0.535        & -0.156  & -0.032 & 0.497    & 0.99                    & -0.682 & -0.115 & 0.678   \\
KM\_Mod   & $D_\alpha$ & 5 & 7     & 0.85  & 0.15 & 0.069         & 0.15 & 0.096              & -0.313        & 0.721   & 0.222  & 0.502    & 1.085                   & 2.753  & 0.463  & 0.085   \\
KM\_Med & $D_\alpha$ & 5 & 7     & 0.85  & 0.15 & 0.034         & 0.15 & 0.103              & -0.476        & 0.329   & 0.072  & 0.496    & 1.06                    & 1.352  & 0.227  & 0.41    \\
SP\_Mod    & $D_\alpha$ & 5 & 7     & 0.85  & 0.15 & 0.075         & 0.15 & 0.097              & -0.329        & 0.768   & 0.227  & 0.509    & 1.055                   & 2.966  & 0.498  & 0.066   \\
SP\_Med  & $D_\alpha$ & 5 & 7     & 0.85  & 0.15 & 0.083         & 0.15 & 0.1                & -0.246        & 0.838   & 0.339  & 0.506    & 1.08                    & 3.313  & 0.557  & 0.041   \\
KM\_Mod   & $D_\alpha$ & 7 & 1     & 0.85  & 0.15 & -0.038        & 0.15 & 0.112              & -0.549        & -0.338  & -0.069 & 0.492    & 0.985                   & -1.502 & -0.252 & 0.36    \\
KM\_Med & $D_\alpha$ & 7 & 1     & 0.85  & 0.15 & -0.063        & 0.15 & 0.12               & -0.661        & -0.521  & -0.095 & 0.491    & 0.957                   & -2.483 & -0.417 & 0.124   \\
SP\_Mod    & $D_\alpha$ & 7 & 1     & 0.85  & 0.15 & -0.037        & 0.15 & 0.12               & -0.613        & -0.306  & -0.06  & 0.497    & 0.965                   & -1.461 & -0.245 & 0.371   \\
SP\_Med  & $D_\alpha$ & 7 & 1     & 0.85  & 0.15 & -0.055        & 0.15 & 0.117              & -0.71         & -0.472  & -0.078 & 0.489    & 0.977                   & -2.194 & -0.369 & 0.178   \\
KM\_Mod   & $D_\alpha$ & 7 & 3     & 0.85  & 0.15 & -0.011        & 0.15 & 0.12               & -0.514        & -0.092  & -0.021 & 0.505    & 0.966                   & -0.435 & -0.073 & 0.791   \\
KM\_Med & $D_\alpha$ & 7 & 3     & 0.85  & 0.15 & 0.031         & 0.15 & 0.114              & -0.329        & 0.274   & 0.095  & 0.502    & 1.03                    & 1.239  & 0.208  & 0.456   \\
SP\_Mod    & $D_\alpha$ & 7 & 3     & 0.85  & 0.15 & -0.017        & 0.15 & 0.12               & -0.669        & -0.142  & -0.026 & 0.516    & 0.918                   & -0.68  & -0.114 & 0.679   \\
SP\_Med  & $D_\alpha$ & 7 & 3     & 0.85  & 0.15 & -0.027        & 0.15 & 0.12               & -0.631        & -0.227  & -0.043 & 0.506    & 0.944                   & -1.084 & -0.182 & 0.507   \\
KM\_Mod   & $D_\alpha$ & 7 & 5     & 0.85  & 0.15 & -0.025        & 0.15 & 0.117              & -0.592        & -0.215  & -0.042 & 0.502    & 0.961                   & -0.998 & -0.168 & 0.542   \\
KM\_Med & $D_\alpha$ & 7 & 5     & 0.85  & 0.15 & -0.006        & 0.15 & 0.112              & -0.54         & -0.05   & -0.01  & 0.5      & 0.994                   & -0.22  & -0.037 & 0.893   \\
SP\_Mod    & $D_\alpha$ & 7 & 5     & 0.85  & 0.15 & 0.075         & 0.15 & 0.1                & -0.276        & 0.748   & 0.271  & 0.513    & 1.038                   & 2.963  & 0.498  & 0.068   \\
SP\_Med  & $D_\alpha$ & 7 & 5     & 0.85  & 0.15 & 0.022         & 0.15 & 0.106              & -0.278        & 0.208   & 0.08   & 0.496    & 1.042                   & 0.878  & 0.148  & 0.595   \\
KM\_Mod   & $D_\alpha$ & 7 & 7     & 0.85  & 0.15 & 0.083         & 0.15 & 0.096              & -0.292        & 0.86    & 0.283  & 0.505    & 1.086                   & 3.28   & 0.551  & 0.039   \\
KM\_Med & $D_\alpha$ & 7 & 7     & 0.85  & 0.15 & 0.052         & 0.15 & 0.104              & -0.336        & 0.504   & 0.155  & 0.502    & 1.06                    & 2.071  & 0.348  & 0.205   \\
SP\_Mod    & $D_\alpha$ & 7 & 7     & 0.85  & 0.15 & 0.12          & 0.15 & 0.095              & -0.258        & 1.259   & 0.464  & 0.511    & 1.107                   & 4.747  & 0.797  & 0.003   \\
SP\_Med  & $D_\alpha$ & 7 & 7     & 0.85  & 0.15 & 0.08          & 0.15 & 0.103              & -0.348        & 0.779   & 0.23   & 0.51     & 1.061                   & 3.18   & 0.534  & 0.051   \\
KM\_Mod   & $D_\alpha$ & 1 & 1     & 0.75  & 0.25 & -0.09         & 0.15 & 0.118              & -0.794        & -0.76   & -0.113 & 0.48     & 0.97                    & -3.566 & -0.599 & 0.027   \\
KM\_Med & $D_\alpha$ & 1 & 1     & 0.75  & 0.25 & -0.109        & 0.15 & 0.12               & -0.806        & -0.904  & -0.135 & 0.475    & 0.967                   & -4.317 & -0.725 & 0.007   \\
SP\_Mod    & $D_\alpha$ & 1 & 1     & 0.75  & 0.25 & -0.092        & 0.15 & 0.122              & -0.758        & -0.759  & -0.122 & 0.479    & 0.968                   & -3.658 & -0.615 & 0.023   \\
SP\_Med  & $D_\alpha$ & 1 & 1     & 0.75  & 0.25 & -0.133        & 0.15 & 0.117              & -0.859        & -1.13   & -0.154 & 0.461    & 0.99                    & -5.264 & -0.884 & 0.001   \\
KM\_Mod   & $D_\alpha$ & 1 & 3     & 0.75  & 0.25 & 0.012         & 0.15 & 0.119              & -0.365        & 0.102   & 0.033  & 0.516    & 0.953                   & 0.479  & 0.081  & 0.772   \\
KM\_Med & $D_\alpha$ & 1 & 3     & 0.75  & 0.25 & 0.044         & 0.15 & 0.119              & -0.289        & 0.371   & 0.153  & 0.517    & 0.987                   & 1.75   & 0.294  & 0.293   \\
SP\_Mod    & $D_\alpha$ & 1 & 3     & 0.75  & 0.25 & 0.014         & 0.15 & 0.116              & -0.502        & 0.117   & 0.027  & 0.508    & 0.987                   & 0.539  & 0.09   & 0.744   \\
SP\_Med  & $D_\alpha$ & 1 & 3     & 0.75  & 0.25 & -0.014        & 0.15 & 0.122              & -0.588        & -0.113  & -0.023 & 0.513    & 0.932                   & -0.544 & -0.091 & 0.74    \\
KM\_Mod   & $D_\alpha$ & 1 & 5     & 0.75  & 0.25 & 0.002         & 0.15 & 0.123              & -0.471        & 0.012   & 0.003  & 0.509    & 0.966                   & 0.06   & 0.01   & 0.971   \\
KM\_Med & $D_\alpha$ & 1 & 5     & 0.75  & 0.25 & -0.034        & 0.15 & 0.111              & -0.521        & -0.31   & -0.066 & 0.487    & 1.009                   & -1.365 & -0.229 & 0.405   \\
SP\_Mod    & $D_\alpha$ & 1 & 5     & 0.75  & 0.25 & 0.014         & 0.15 & 0.12               & -0.471        & 0.115   & 0.029  & 0.506    & 0.994                   & 0.547  & 0.092  & 0.741   \\
SP\_Med  & $D_\alpha$ & 1 & 5     & 0.75  & 0.25 & 0.021         & 0.15 & 0.116              & -0.353        & 0.18    & 0.059  & 0.501    & 1.021                   & 0.832  & 0.14   & 0.615   \\
KM\_Mod   & $D_\alpha$ & 1 & 7     & 0.75  & 0.25 & -0.038        & 0.15 & 0.123              & -0.628        & -0.308  & -0.06  & 0.488    & 1.001                   & -1.5   & -0.252 & 0.355   \\
KM\_Med & $D_\alpha$ & 1 & 7     & 0.75  & 0.25 & 0.05          & 0.15 & 0.104              & -0.412        & 0.479   & 0.121  & 0.498    & 1.073                   & 1.984  & 0.333  & 0.226   \\
SP\_Mod    & $D_\alpha$ & 1 & 7     & 0.75  & 0.25 & 0.0           & 0.15 & 0.108              & -0.368        & 0.002   & 0.001  & 0.509    & 0.965                   & 0.01   & 0.002  & 0.995   \\
SP\_Med  & $D_\alpha$ & 1 & 7     & 0.75  & 0.25 & 0.054         & 0.15 & 0.107              & -0.316        & 0.508   & 0.172  & 0.507    & 1.039                   & 2.156  & 0.362  & 0.189   \\
KM\_Mod   & $D_\alpha$ & 3 & 1     & 0.75  & 0.25 & -0.117        & 0.15 & 0.119              & -0.844        & -0.99   & -0.139 & 0.473    & 0.962                   & -4.661 & -0.783 & 0.004   \\
KM\_Med & $D_\alpha$ & 3 & 1     & 0.75  & 0.25 & -0.112        & 0.15 & 0.12               & -0.836        & -0.933  & -0.134 & 0.48     & 0.945                   & -4.429 & -0.744 & 0.006   \\
SP\_Mod    & $D_\alpha$ & 3 & 1     & 0.75  & 0.25 & -0.097        & 0.15 & 0.121              & -0.799        & -0.801  & -0.121 & 0.485    & 0.937                   & -3.84  & -0.645 & 0.017   \\
SP\_Med  & $D_\alpha$ & 3 & 1     & 0.75  & 0.25 & -0.102        & 0.15 & 0.123              & -0.817        & -0.835  & -0.125 & 0.482    & 0.946                   & -4.063 & -0.683 & 0.011   \\
KM\_Mod   & $D_\alpha$ & 3 & 3     & 0.75  & 0.25 & 0.023         & 0.15 & 0.118              & -0.398        & 0.191   & 0.057  & 0.511    & 0.984                   & 0.893  & 0.15   & 0.59    \\
KM\_Med & $D_\alpha$ & 3 & 3     & 0.75  & 0.25 & 0.046         & 0.15 & 0.117              & -0.341        & 0.393   & 0.135  & 0.515    & 0.996                   & 1.824  & 0.307  & 0.273   \\
SP\_Mod    & $D_\alpha$ & 3 & 3     & 0.75  & 0.25 & 0.006         & 0.15 & 0.119              & -0.466        & 0.054   & 0.014  & 0.506    & 0.985                   & 0.254  & 0.043  & 0.878   \\
SP\_Med  & $D_\alpha$ & 3 & 3     & 0.75  & 0.25 & -0.018        & 0.15 & 0.121              & -0.513        & -0.148  & -0.035 & 0.508    & 0.947                   & -0.709 & -0.119 & 0.665   \\
KM\_Mod   & $D_\alpha$ & 3 & 5     & 0.75  & 0.25 & -0.035        & 0.15 & 0.12               & -0.559        & -0.287  & -0.062 & 0.506    & 0.934                   & -1.373 & -0.231 & 0.4     \\
KM\_Med & $D_\alpha$ & 3 & 5     & 0.75  & 0.25 & -0.014        & 0.15 & 0.11               & -0.508        & -0.128  & -0.028 & 0.491    & 1.017                   & -0.56  & -0.094 & 0.734   \\
SP\_Mod    & $D_\alpha$ & 3 & 5     & 0.75  & 0.25 & 0.009         & 0.15 & 0.112              & -0.381        & 0.077   & 0.023  & 0.5      & 1.01                    & 0.343  & 0.058  & 0.835   \\
SP\_Med  & $D_\alpha$ & 3 & 5     & 0.75  & 0.25 & -0.001        & 0.15 & 0.111              & -0.566        & -0.009  & -0.002 & 0.492    & 1.032                   & -0.041 & -0.007 & 0.98    \\
KM\_Mod   & $D_\alpha$ & 3 & 7     & 0.75  & 0.25 & 0.047         & 0.15 & 0.104              & -0.278        & 0.457   & 0.17   & 0.501    & 1.059                   & 1.879  & 0.316  & 0.246   \\
KM\_Med & $D_\alpha$ & 3 & 7     & 0.75  & 0.25 & 0.059         & 0.15 & 0.106              & -0.427        & 0.557   & 0.138  & 0.511    & 1.028                   & 2.338  & 0.393  & 0.153   \\
SP\_Mod    & $D_\alpha$ & 3 & 7     & 0.75  & 0.25 & 0.037         & 0.15 & 0.108              & -0.409        & 0.346   & 0.091  & 0.522    & 0.96                    & 1.483  & 0.249  & 0.366   \\
SP\_Med  & $D_\alpha$ & 3 & 7     & 0.75  & 0.25 & 0.051         & 0.15 & 0.106              & -0.246        & 0.478   & 0.206  & 0.502    & 1.057                   & 2.016  & 0.339  & 0.22    \\
KM\_Mod   & $D_\alpha$ & 5 & 1     & 0.75  & 0.25 & -0.107        & 0.15 & 0.12               & -0.809        & -0.893  & -0.133 & 0.487    & 0.922                   & -4.265 & -0.716 & 0.008   \\
KM\_Med & $D_\alpha$ & 5 & 1     & 0.75  & 0.25 & -0.101        & 0.15 & 0.122              & -0.805        & -0.832  & -0.126 & 0.484    & 0.942                   & -4.021 & -0.676 & 0.012   \\
SP\_Mod    & $D_\alpha$ & 5 & 1     & 0.75  & 0.25 & -0.099        & 0.15 & 0.125              & -0.796        & -0.794  & -0.125 & 0.494    & 0.904                   & -3.94  & -0.662 & 0.014   \\
SP\_Med  & $D_\alpha$ & 5 & 1     & 0.75  & 0.25 & -0.094        & 0.15 & 0.122              & -0.766        & -0.766  & -0.122 & 0.491    & 0.923                   & -3.713 & -0.624 & 0.021   \\
KM\_Mod   & $D_\alpha$ & 5 & 3     & 0.75  & 0.25 & 0.015         & 0.15 & 0.12               & -0.362        & 0.125   & 0.041  & 0.514    & 0.965                   & 0.595  & 0.1    & 0.719   \\
KM\_Med & $D_\alpha$ & 5 & 3     & 0.75  & 0.25 & 0.028         & 0.15 & 0.115              & -0.351        & 0.241   & 0.079  & 0.505    & 1.014                   & 1.097  & 0.184  & 0.508   \\
SP\_Mod    & $D_\alpha$ & 5 & 3     & 0.75  & 0.25 & 0.039         & 0.15 & 0.113              & -0.384        & 0.34    & 0.1    & 0.512    & 1.002                   & 1.529  & 0.257  & 0.354   \\
SP\_Med  & $D_\alpha$ & 5 & 3     & 0.75  & 0.25 & -0.002        & 0.15 & 0.119              & -0.523        & -0.013  & -0.003 & 0.503    & 0.986                   & -0.063 & -0.011 & 0.969   \\
KM\_Mod   & $D_\alpha$ & 5 & 5     & 0.75  & 0.25 & -0.032        & 0.15 & 0.12               & -0.543        & -0.27   & -0.06  & 0.506    & 0.935                   & -1.289 & -0.217 & 0.43    \\
KM\_Med & $D_\alpha$ & 5 & 5     & 0.75  & 0.25 & -0.048        & 0.15 & 0.111              & -0.552        & -0.434  & -0.087 & 0.488    & 0.988                   & -1.916 & -0.322 & 0.242   \\
SP\_Mod    & $D_\alpha$ & 5 & 5     & 0.75  & 0.25 & 0.016         & 0.15 & 0.109              & -0.448        & 0.146   & 0.036  & 0.501    & 1.017                   & 0.631  & 0.106  & 0.701   \\
SP\_Med  & $D_\alpha$ & 5 & 5     & 0.75  & 0.25 & -0.044        & 0.15 & 0.113              & -0.662        & -0.391  & -0.067 & 0.484    & 1.009                   & -1.754 & -0.295 & 0.284   \\
KM\_Mod   & $D_\alpha$ & 5 & 7     & 0.75  & 0.25 & 0.057         & 0.15 & 0.096              & -0.381        & 0.591   & 0.149  & 0.501    & 1.073                   & 2.246  & 0.377  & 0.161   \\
KM\_Med & $D_\alpha$ & 5 & 7     & 0.75  & 0.25 & 0.064         & 0.15 & 0.104              & -0.401        & 0.619   & 0.16   & 0.506    & 1.057                   & 2.55   & 0.428  & 0.119   \\
SP\_Mod    & $D_\alpha$ & 5 & 7     & 0.75  & 0.25 & 0.053         & 0.15 & 0.103              & -0.301        & 0.519   & 0.177  & 0.514    & 1.011                   & 2.11   & 0.354  & 0.196   \\
SP\_Med  & $D_\alpha$ & 5 & 7     & 0.75  & 0.25 & 0.069         & 0.15 & 0.103              & -0.282        & 0.67    & 0.245  & 0.505    & 1.069                   & 2.745  & 0.461  & 0.093   \\
KM\_Mod   & $D_\alpha$ & 7 & 1     & 0.75  & 0.25 & -0.071        & 0.15 & 0.117              & -0.733        & -0.604  & -0.097 & 0.487    & 0.963                   & -2.81  & -0.472 & 0.084   \\
KM\_Med & $D_\alpha$ & 7 & 1     & 0.75  & 0.25 & -0.076        & 0.15 & 0.119              & -0.725        & -0.642  & -0.105 & 0.486    & 0.964                   & -3.028 & -0.509 & 0.061   \\
SP\_Mod    & $D_\alpha$ & 7 & 1     & 0.75  & 0.25 & -0.027        & 0.15 & 0.122              & -0.574        & -0.225  & -0.048 & 0.496    & 0.982                   & -1.089 & -0.183 & 0.505   \\
SP\_Med  & $D_\alpha$ & 7 & 1     & 0.75  & 0.25 & -0.04         & 0.15 & 0.121              & -0.636        & -0.332  & -0.063 & 0.496    & 0.965                   & -1.59  & -0.267 & 0.33    \\
KM\_Mod   & $D_\alpha$ & 7 & 3     & 0.75  & 0.25 & -0.022        & 0.15 & 0.122              & -0.516        & -0.184  & -0.044 & 0.507    & 0.946                   & -0.891 & -0.15  & 0.586   \\
KM\_Med & $D_\alpha$ & 7 & 3     & 0.75  & 0.25 & 0.006         & 0.15 & 0.115              & -0.401        & 0.055   & 0.016  & 0.505    & 0.986                   & 0.252  & 0.042  & 0.879   \\
SP\_Mod    & $D_\alpha$ & 7 & 3     & 0.75  & 0.25 & -0.019        & 0.15 & 0.12               & -0.586        & -0.156  & -0.032 & 0.506    & 0.955                   & -0.74  & -0.124 & 0.652   \\
SP\_Med  & $D_\alpha$ & 7 & 3     & 0.75  & 0.25 & -0.054        & 0.15 & 0.125              & -0.738        & -0.436  & -0.074 & 0.509    & 0.904                   & -2.158 & -0.362 & 0.182   \\
KM\_Mod   & $D_\alpha$ & 7 & 5     & 0.75  & 0.25 & -0.008        & 0.15 & 0.12               & -0.566        & -0.069  & -0.015 & 0.508    & 0.958                   & -0.327 & -0.055 & 0.842   \\
KM\_Med & $D_\alpha$ & 7 & 5     & 0.75  & 0.25 & 0.019         & 0.15 & 0.109              & -0.376        & 0.177   & 0.051  & 0.498    & 1.031                   & 0.762  & 0.128  & 0.644   \\
SP\_Mod    & $D_\alpha$ & 7 & 5     & 0.75  & 0.25 & 0.028         & 0.15 & 0.112              & -0.364        & 0.254   & 0.078  & 0.499    & 1.04                    & 1.129  & 0.19   & 0.494   \\
SP\_Med  & $D_\alpha$ & 7 & 5     & 0.75  & 0.25 & 0.022         & 0.15 & 0.108              & -0.396        & 0.205   & 0.056  & 0.495    & 1.048                   & 0.878  & 0.147  & 0.594   \\
KM\_Mod   & $D_\alpha$ & 7 & 7     & 0.75  & 0.25 & 0.065         & 0.15 & 0.097              & -0.267        & 0.676   & 0.245  & 0.502    & 1.077                   & 2.591  & 0.435  & 0.105   \\
KM\_Med & $D_\alpha$ & 7 & 7     & 0.75  & 0.25 & 0.022         & 0.15 & 0.105              & -0.385        & 0.213   & 0.058  & 0.5      & 1.027                   & 0.889  & 0.149  & 0.588   \\
SP\_Mod    & $D_\alpha$ & 7 & 7     & 0.75  & 0.25 & 0.073         & 0.15 & 0.1                & -0.272        & 0.728   & 0.269  & 0.51     & 1.05                    & 2.901  & 0.487  & 0.074   \\
SP\_Med  & $D_\alpha$ & 7 & 7     & 0.75  & 0.25 & 0.081         & 0.15 & 0.105              & -0.382        & 0.771   & 0.211  & 0.504    & 1.087                   & 3.2    & 0.538  & 0.051   \\
CCF              & $D_\alpha$ & 1 & 1     & 0.85  & 0.15 & -0.127        & 0.15 & 0.116              & -0.848        & -1.092  & -0.15  & 0.468    & 0.972                   & -5.042 & -0.847 & 0.002   \\
CCF              & $D_\alpha$ & 1 & 3     & 0.85  & 0.15 & 0.023         & 0.15 & 0.123              & -0.503        & 0.188   & 0.046  & 0.511    & 0.985                   & 0.915  & 0.154  & 0.582   \\
CCF              & $D_\alpha$ & 1 & 5     & 0.85  & 0.15 & -0.075        & 0.15 & 0.119              & -0.752        & -0.629  & -0.099 & 0.49     & 0.948                   & -2.968 & -0.499 & 0.066   \\
CCF              & $D_\alpha$ & 1 & 7     & 0.85  & 0.15 & 0.03          & 0.15 & 0.1                & -0.337        & 0.299   & 0.088  & 0.497    & 1.051                   & 1.182  & 0.199  & 0.47    \\
CCF              & $D_\alpha$ & 3 & 1     & 0.85  & 0.15 & -0.108        & 0.15 & 0.118              & -0.8          & -0.911  & -0.135 & 0.485    & 0.932                   & -4.281 & -0.719 & 0.008   \\
CCF              & $D_\alpha$ & 3 & 3     & 0.85  & 0.15 & -0.002        & 0.15 & 0.119              & -0.478        & -0.016  & -0.004 & 0.505    & 0.976                   & -0.077 & -0.013 & 0.963   \\
CCF              & $D_\alpha$ & 3 & 5     & 0.85  & 0.15 & -0.025        & 0.15 & 0.115              & -0.626        & -0.219  & -0.04  & 0.497    & 0.982                   & -0.996 & -0.167 & 0.543   \\
CCF              & $D_\alpha$ & 3 & 7     & 0.85  & 0.15 & 0.041         & 0.15 & 0.099              & -0.347        & 0.419   & 0.119  & 0.505    & 1.03                    & 1.643  & 0.276  & 0.314   \\
CCF              & $D_\alpha$ & 5 & 1     & 0.85  & 0.15 & -0.103        & 0.15 & 0.118              & -0.797        & -0.876  & -0.13  & 0.487    & 0.928                   & -4.101 & -0.689 & 0.011   \\
CCF              & $D_\alpha$ & 5 & 3     & 0.85  & 0.15 & 0.032         & 0.15 & 0.116              & -0.343        & 0.278   & 0.094  & 0.506    & 1.016                   & 1.28   & 0.215  & 0.441   \\
CCF              & $D_\alpha$ & 5 & 5     & 0.85  & 0.15 & -0.069        & 0.15 & 0.118              & -0.716        & -0.587  & -0.097 & 0.489    & 0.96                    & -2.747 & -0.461 & 0.089   \\
CCF              & $D_\alpha$ & 5 & 7     & 0.85  & 0.15 & 0.084         & 0.15 & 0.093              & -0.297        & 0.911   & 0.284  & 0.5      & 1.107                   & 3.353  & 0.563  & 0.037   \\
CCF              & $D_\alpha$ & 7 & 1     & 0.85  & 0.15 & -0.087        & 0.15 & 0.115              & -0.767        & -0.752  & -0.113 & 0.482    & 0.967                   & -3.438 & -0.578 & 0.034   \\
CCF              & $D_\alpha$ & 7 & 3     & 0.85  & 0.15 & -0.03         & 0.15 & 0.122              & -0.576        & -0.243  & -0.051 & 0.499    & 0.968                   & -1.175 & -0.197 & 0.471   \\
CCF              & $D_\alpha$ & 7 & 5     & 0.85  & 0.15 & -0.009        & 0.15 & 0.113              & -0.434        & -0.076  & -0.02  & 0.5      & 0.988                   & -0.34  & -0.057 & 0.836   \\
CCF              & $D_\alpha$ & 7 & 7     & 0.85  & 0.15 & 0.041         & 0.15 & 0.097              & -0.382        & 0.422   & 0.107  & 0.494    & 1.077                   & 1.617  & 0.272  & 0.321   \\
CCF              & $D_\alpha$ & 1 & 1     & 0.75  & 0.25 & -0.146        & 0.15 & 0.122              & -0.908        & -1.193  & -0.161 & 0.473    & 0.93                    & -5.787 & -0.972 & 0.0     \\
CCF              & $D_\alpha$ & 1 & 3     & 0.75  & 0.25 & 0.032         & 0.15 & 0.12               & -0.337        & 0.27    & 0.096  & 0.509    & 1.005                   & 1.286  & 0.216  & 0.44    \\
CCF              & $D_\alpha$ & 1 & 5     & 0.75  & 0.25 & -0.044        & 0.15 & 0.123              & -0.658        & -0.36   & -0.067 & 0.505    & 0.928                   & -1.759 & -0.296 & 0.278   \\
CCF              & $D_\alpha$ & 1 & 7     & 0.75  & 0.25 & 0.064         & 0.15 & 0.099              & -0.282        & 0.643   & 0.227  & 0.503    & 1.069                   & 2.538  & 0.426  & 0.118   \\
CCF              & $D_\alpha$ & 3 & 1     & 0.75  & 0.25 & -0.093        & 0.15 & 0.121              & -0.78         & -0.767  & -0.119 & 0.491    & 0.923                   & -3.697 & -0.621 & 0.021   \\
CCF              & $D_\alpha$ & 3 & 3     & 0.75  & 0.25 & 0.024         & 0.15 & 0.119              & -0.447        & 0.202   & 0.054  & 0.508    & 0.997                   & 0.955  & 0.16   & 0.565   \\
CCF              & $D_\alpha$ & 3 & 5     & 0.75  & 0.25 & -0.019        & 0.15 & 0.117              & -0.606        & -0.158  & -0.031 & 0.499    & 0.979                   & -0.734 & -0.123 & 0.654   \\
CCF              & $D_\alpha$ & 3 & 7     & 0.75  & 0.25 & 0.039         & 0.15 & 0.1                & -0.32         & 0.386   & 0.121  & 0.507    & 1.021                   & 1.536  & 0.258  & 0.347   \\
CCF              & $D_\alpha$ & 5 & 1     & 0.75  & 0.25 & -0.041        & 0.15 & 0.119              & -0.618        & -0.348  & -0.067 & 0.504    & 0.934                   & -1.643 & -0.276 & 0.313   \\
CCF              & $D_\alpha$ & 5 & 3     & 0.75  & 0.25 & 0.007         & 0.15 & 0.118              & -0.492        & 0.056   & 0.013  & 0.501    & 1.006                   & 0.261  & 0.044  & 0.874   \\
CCF              & $D_\alpha$ & 5 & 5     & 0.75  & 0.25 & -0.051        & 0.15 & 0.118              & -0.641        & -0.431  & -0.08  & 0.494    & 0.962                   & -2.026 & -0.34  & 0.212   \\
CCF              & $D_\alpha$ & 5 & 7     & 0.75  & 0.25 & 0.092         & 0.15 & 0.093              & -0.333        & 0.989   & 0.277  & 0.509    & 1.081                   & 3.655  & 0.614  & 0.023   \\
CCF              & $D_\alpha$ & 7 & 1     & 0.75  & 0.25 & -0.044        & 0.15 & 0.118              & -0.661        & -0.371  & -0.066 & 0.497    & 0.958                   & -1.735 & -0.291 & 0.286   \\
CCF              & $D_\alpha$ & 7 & 3     & 0.75  & 0.25 & -0.02         & 0.15 & 0.122              & -0.538        & -0.168  & -0.038 & 0.509    & 0.941                   & -0.81  & -0.136 & 0.62    \\
CCF              & $D_\alpha$ & 7 & 5     & 0.75  & 0.25 & 0.007         & 0.15 & 0.115              & -0.443        & 0.058   & 0.015  & 0.502    & 0.999                   & 0.266  & 0.045  & 0.872   \\
CCF              & $D_\alpha$ & 7 & 7     & 0.75  & 0.25 & 0.056         & 0.15 & 0.097              & -0.362        & 0.581   & 0.156  & 0.504    & 1.056                   & 2.234  & 0.375  & 0.169  \\
\hline
\end{longtable}
\end{small}



\subsection*{Futures data set: performance metrics for the entire grid -  rescaled to target volatility}
\label{futures_full_results}



\begin{small}
\captionof{table}*{Table S3: Futures data set: performance metrics for the entire grid - rescaled to target volatility. The experiment has
been set with the values $p = \{1,3,5,7\}$, $\delta = \{1,3,5,7\}$, and $\alpha = \{0.7,0.75,0.8,0.85\}$.}
\label{tab: futures_grid}
\begin{longtable}{|p{2.9cm}p{1.2cm}p{0.1cm}p{0.1cm}p{0.5cm}p{0.5cm}p{1.4cm}p{1.2cm}p{1.6cm}p{1.7cm}p{1cm}p{1cm}p{0.5cm}p{1.2cm}p{1.4cm}p{0.9cm}p{1.5cm}|}
\toprule
\textbf{Method}       & \textbf{Strategy}   & \textbf{$p$} & \textbf{$\delta$} & \textbf{$\alpha$} & \textbf{$\beta$} & \textbf{E[Returns]} & \textbf{Volatility}  & \textbf{Downside deviation} & \textbf{Maximum drawdown} & \textbf{Sortino ratio} & \textbf{Calmar ratio} & \textbf{Hit rate} & \textbf{$\frac{\text{Avg. profit}}{\text{Avg. loss}}$} & \textbf{PnL per trade}  & \textbf{Sharpe ratio} & \textbf{P-value} \\
\midrule
KM\_Mod   & $G_\beta$ & 1 & 1     & 0.85  & 0.15 & -0.12         & 0.15 & 0.104              & -0.945        & -1.151  & -0.127 & 0.48     & 0.943                   & -4.768 & -0.801 & 0.0     \\
KM\_Med & $G_\beta$ & 1 & 1     & 0.85  & 0.15 & -0.138        & 0.15 & 0.111              & -0.963        & -1.247  & -0.143 & 0.47     & 0.954                   & -5.475 & -0.92  & 0.0     \\
SP\_Mod    & $G_\beta$ & 1 & 1     & 0.85  & 0.15 & -0.142        & 0.15 & 0.103              & -0.967        & -1.383  & -0.147 & 0.476    & 0.938                   & -5.646 & -0.949 & 0.0     \\
SP\_Med  & $G_\beta$ & 1 & 1     & 0.85  & 0.15 & -0.141        & 0.15 & 0.107              & -0.966        & -1.315  & -0.146 & 0.475    & 0.937                   & -5.581 & -0.938 & 0.0     \\
KM\_Mod   & $G_\beta$ & 1 & 3     & 0.85  & 0.15 & 0.009         & 0.15 & 0.103              & -0.473        & 0.083   & 0.018  & 0.505    & 0.991                   & 0.34   & 0.057  & 0.797   \\
KM\_Med & $G_\beta$ & 1 & 3     & 0.85  & 0.15 & 0.023         & 0.15 & 0.106              & -0.516        & 0.216   & 0.044  & 0.507    & 0.998                   & 0.911  & 0.153  & 0.49    \\
SP\_Mod    & $G_\beta$ & 1 & 3     & 0.85  & 0.15 & 0.003         & 0.15 & 0.099              & -0.531        & 0.032   & 0.006  & 0.501    & 0.998                   & 0.124  & 0.021  & 0.925   \\
SP\_Med  & $G_\beta$ & 1 & 3     & 0.85  & 0.15 & -0.005        & 0.15 & 0.104              & -0.548        & -0.048  & -0.009 & 0.495    & 1.015                   & -0.196 & -0.033 & 0.882   \\
KM\_Mod   & $G_\beta$ & 1 & 5     & 0.85  & 0.15 & -0.049        & 0.15 & 0.107              & -0.778        & -0.457  & -0.063 & 0.505    & 0.928                   & -1.945 & -0.327 & 0.139   \\
KM\_Med & $G_\beta$ & 1 & 5     & 0.85  & 0.15 & 0.001         & 0.15 & 0.106              & -0.513        & 0.005   & 0.001  & 0.502    & 0.992                   & 0.02   & 0.003  & 0.988   \\
SP\_Mod    & $G_\beta$ & 1 & 5     & 0.85  & 0.15 & -0.042        & 0.15 & 0.099              & -0.76         & -0.421  & -0.055 & 0.488    & 1.001                   & -1.649 & -0.277 & 0.211   \\
SP\_Med  & $G_\beta$ & 1 & 5     & 0.85  & 0.15 & 0.015         & 0.15 & 0.101              & -0.577        & 0.151   & 0.027  & 0.497    & 1.028                   & 0.608  & 0.102  & 0.645   \\
KM\_Mod   & $G_\beta$ & 1 & 7     & 0.85  & 0.15 & 0.032         & 0.15 & 0.098              & -0.515        & 0.322   & 0.061  & 0.497    & 1.05                    & 1.256  & 0.211  & 0.34    \\
KM\_Med & $G_\beta$ & 1 & 7     & 0.85  & 0.15 & 0.029         & 0.15 & 0.105              & -0.479        & 0.28    & 0.061  & 0.5      & 1.035                   & 1.169  & 0.196  & 0.375   \\
SP\_Mod    & $G_\beta$ & 1 & 7     & 0.85  & 0.15 & -0.033        & 0.15 & 0.103              & -0.789        & -0.323  & -0.042 & 0.501    & 0.96                    & -1.326 & -0.223 & 0.314   \\
SP\_Med  & $G_\beta$ & 1 & 7     & 0.85  & 0.15 & -0.0          & 0.15 & 0.105              & -0.586        & -0.005  & -0.001 & 0.498    & 1.006                   & -0.019 & -0.003 & 0.988   \\
KM\_Mod   & $G_\beta$ & 3 & 1     & 0.85  & 0.15 & -0.09         & 0.15 & 0.105              & -0.888        & -0.857  & -0.101 & 0.482    & 0.967                   & -3.554 & -0.597 & 0.007   \\
KM\_Med & $G_\beta$ & 3 & 1     & 0.85  & 0.15 & -0.112        & 0.15 & 0.11               & -0.922        & -1.014  & -0.121 & 0.47     & 0.986                   & -4.432 & -0.745 & 0.001   \\
SP\_Mod    & $G_\beta$ & 3 & 1     & 0.85  & 0.15 & -0.091        & 0.15 & 0.101              & -0.89         & -0.901  & -0.103 & 0.482    & 0.97                    & -3.623 & -0.609 & 0.006   \\
SP\_Med  & $G_\beta$ & 3 & 1     & 0.85  & 0.15 & -0.102        & 0.15 & 0.105              & -0.902        & -0.973  & -0.113 & 0.481    & 0.958                   & -4.04  & -0.679 & 0.002   \\
KM\_Mod   & $G_\beta$ & 3 & 3     & 0.85  & 0.15 & 0.001         & 0.15 & 0.104              & -0.42         & 0.01    & 0.002  & 0.507    & 0.973                   & 0.042  & 0.007  & 0.975   \\
KM\_Med & $G_\beta$ & 3 & 3     & 0.85  & 0.15 & 0.019         & 0.15 & 0.109              & -0.386        & 0.173   & 0.049  & 0.514    & 0.966                   & 0.75   & 0.126  & 0.57    \\
SP\_Mod    & $G_\beta$ & 3 & 3     & 0.85  & 0.15 & -0.004        & 0.15 & 0.102              & -0.543        & -0.036  & -0.007 & 0.51     & 0.956                   & -0.145 & -0.024 & 0.912   \\
SP\_Med  & $G_\beta$ & 3 & 3     & 0.85  & 0.15 & -0.001        & 0.15 & 0.103              & -0.454        & -0.014  & -0.003 & 0.5      & 1.0                     & -0.057 & -0.009 & 0.966   \\
KM\_Mod   & $G_\beta$ & 3 & 5     & 0.85  & 0.15 & -0.058        & 0.15 & 0.107              & -0.779        & -0.54   & -0.074 & 0.494    & 0.959                   & -2.288 & -0.384 & 0.082   \\
KM\_Med & $G_\beta$ & 3 & 5     & 0.85  & 0.15 & -0.026        & 0.15 & 0.107              & -0.609        & -0.24   & -0.042 & 0.492    & 1.003                   & -1.022 & -0.172 & 0.438   \\
SP\_Mod    & $G_\beta$ & 3 & 5     & 0.85  & 0.15 & -0.051        & 0.15 & 0.099              & -0.757        & -0.52   & -0.068 & 0.489    & 0.986                   & -2.034 & -0.342 & 0.123   \\
SP\_Med  & $G_\beta$ & 3 & 5     & 0.85  & 0.15 & -0.026        & 0.15 & 0.103              & -0.698        & -0.249  & -0.037 & 0.492    & 1.003                   & -1.013 & -0.17  & 0.443   \\
KM\_Mod   & $G_\beta$ & 3 & 7     & 0.85  & 0.15 & -0.007        & 0.15 & 0.097              & -0.566        & -0.07   & -0.012 & 0.491    & 1.027                   & -0.27  & -0.045 & 0.838   \\
KM\_Med & $G_\beta$ & 3 & 7     & 0.85  & 0.15 & -0.031        & 0.15 & 0.104              & -0.64         & -0.297  & -0.048 & 0.489    & 1.006                   & -1.231 & -0.207 & 0.351   \\
SP\_Mod    & $G_\beta$ & 3 & 7     & 0.85  & 0.15 & -0.05         & 0.15 & 0.1                & -0.755        & -0.5    & -0.066 & 0.49     & 0.983                   & -1.988 & -0.334 & 0.132   \\
SP\_Med  & $G_\beta$ & 3 & 7     & 0.85  & 0.15 & -0.036        & 0.15 & 0.103              & -0.646        & -0.348  & -0.056 & 0.489    & 1.002                   & -1.426 & -0.24  & 0.28    \\
KM\_Mod   & $G_\beta$ & 5 & 1     & 0.85  & 0.15 & -0.086        & 0.15 & 0.105              & -0.892        & -0.817  & -0.096 & 0.486    & 0.957                   & -3.395 & -0.57  & 0.01    \\
KM\_Med & $G_\beta$ & 5 & 1     & 0.85  & 0.15 & -0.103        & 0.15 & 0.109              & -0.918        & -0.943  & -0.112 & 0.475    & 0.977                   & -4.069 & -0.684 & 0.002   \\
SP\_Mod    & $G_\beta$ & 5 & 1     & 0.85  & 0.15 & -0.07         & 0.15 & 0.102              & -0.855        & -0.681  & -0.081 & 0.494    & 0.948                   & -2.759 & -0.464 & 0.036   \\
SP\_Med  & $G_\beta$ & 5 & 1     & 0.85  & 0.15 & -0.087        & 0.15 & 0.106              & -0.881        & -0.817  & -0.098 & 0.488    & 0.949                   & -3.435 & -0.577 & 0.009   \\
KM\_Mod   & $G_\beta$ & 5 & 3     & 0.85  & 0.15 & 0.004         & 0.15 & 0.101              & -0.489        & 0.044   & 0.009  & 0.502    & 0.996                   & 0.178  & 0.03   & 0.892   \\
KM\_Med & $G_\beta$ & 5 & 3     & 0.85  & 0.15 & 0.033         & 0.15 & 0.106              & -0.579        & 0.309   & 0.057  & 0.51     & 0.998                   & 1.302  & 0.219  & 0.323   \\
SP\_Mod    & $G_\beta$ & 5 & 3     & 0.85  & 0.15 & 0.022         & 0.15 & 0.101              & -0.376        & 0.219   & 0.059  & 0.51     & 0.984                   & 0.877  & 0.147  & 0.506   \\
SP\_Med  & $G_\beta$ & 5 & 3     & 0.85  & 0.15 & 0.019         & 0.15 & 0.102              & -0.41         & 0.183   & 0.046  & 0.499    & 1.026                   & 0.745  & 0.125  & 0.572   \\
KM\_Mod   & $G_\beta$ & 5 & 5     & 0.85  & 0.15 & -0.055        & 0.15 & 0.105              & -0.818        & -0.524  & -0.067 & 0.492    & 0.97                    & -2.182 & -0.367 & 0.097   \\
KM\_Med & $G_\beta$ & 5 & 5     & 0.85  & 0.15 & -0.053        & 0.15 & 0.106              & -0.767        & -0.496  & -0.069 & 0.486    & 0.993                   & -2.095 & -0.352 & 0.112   \\
SP\_Mod    & $G_\beta$ & 5 & 5     & 0.85  & 0.15 & -0.086        & 0.15 & 0.099              & -0.887        & -0.863  & -0.097 & 0.483    & 0.974                   & -3.408 & -0.572 & 0.01    \\
SP\_Med  & $G_\beta$ & 5 & 5     & 0.85  & 0.15 & -0.043        & 0.15 & 0.104              & -0.776        & -0.409  & -0.055 & 0.498    & 0.96                    & -1.688 & -0.284 & 0.201   \\
KM\_Mod   & $G_\beta$ & 5 & 7     & 0.85  & 0.15 & 0.012         & 0.15 & 0.1                & -0.528        & 0.123   & 0.023  & 0.499    & 1.018                   & 0.492  & 0.083  & 0.709   \\
KM\_Med & $G_\beta$ & 5 & 7     & 0.85  & 0.15 & 0.02          & 0.15 & 0.106              & -0.464        & 0.187   & 0.043  & 0.503    & 1.011                   & 0.787  & 0.132  & 0.551   \\
SP\_Mod    & $G_\beta$ & 5 & 7     & 0.85  & 0.15 & 0.019         & 0.15 & 0.103              & -0.465        & 0.186   & 0.041  & 0.503    & 1.009                   & 0.757  & 0.127  & 0.566   \\
SP\_Med  & $G_\beta$ & 5 & 7     & 0.85  & 0.15 & 0.01          & 0.15 & 0.105              & -0.488        & 0.095   & 0.02   & 0.495    & 1.031                   & 0.396  & 0.067  & 0.764   \\
KM\_Mod   & $G_\beta$ & 7 & 1     & 0.85  & 0.15 & -0.105        & 0.15 & 0.104              & -0.936        & -1.012  & -0.113 & 0.482    & 0.95                    & -4.182 & -0.702 & 0.002   \\
KM\_Med & $G_\beta$ & 7 & 1     & 0.85  & 0.15 & -0.084        & 0.15 & 0.107              & -0.898        & -0.784  & -0.094 & 0.48     & 0.98                    & -3.344 & -0.562 & 0.011   \\
SP\_Mod    & $G_\beta$ & 7 & 1     & 0.85  & 0.15 & -0.086        & 0.15 & 0.102              & -0.876        & -0.837  & -0.098 & 0.489    & 0.951                   & -3.4   & -0.571 & 0.01    \\
SP\_Med  & $G_\beta$ & 7 & 1     & 0.85  & 0.15 & -0.105        & 0.15 & 0.106              & -0.908        & -0.984  & -0.115 & 0.485    & 0.941                   & -4.157 & -0.698 & 0.002   \\
KM\_Mod   & $G_\beta$ & 7 & 3     & 0.85  & 0.15 & -0.037        & 0.15 & 0.102              & -0.769        & -0.362  & -0.048 & 0.494    & 0.981                   & -1.471 & -0.247 & 0.265   \\
KM\_Med & $G_\beta$ & 7 & 3     & 0.85  & 0.15 & -0.023        & 0.15 & 0.108              & -0.633        & -0.21   & -0.036 & 0.5      & 0.974                   & -0.898 & -0.151 & 0.496   \\
SP\_Mod    & $G_\beta$ & 7 & 3     & 0.85  & 0.15 & -0.004        & 0.15 & 0.1                & -0.53         & -0.036  & -0.007 & 0.502    & 0.988                   & -0.142 & -0.024 & 0.915   \\
SP\_Med  & $G_\beta$ & 7 & 3     & 0.85  & 0.15 & -0.036        & 0.15 & 0.103              & -0.727        & -0.351  & -0.05  & 0.489    & 1.001                   & -1.432 & -0.241 & 0.278   \\
KM\_Mod   & $G_\beta$ & 7 & 5     & 0.85  & 0.15 & -0.024        & 0.15 & 0.105              & -0.786        & -0.225  & -0.03  & 0.496    & 0.987                   & -0.937 & -0.157 & 0.477   \\
KM\_Med & $G_\beta$ & 7 & 5     & 0.85  & 0.15 & -0.013        & 0.15 & 0.106              & -0.669        & -0.121  & -0.019 & 0.495    & 1.007                   & -0.51  & -0.086 & 0.699   \\
SP\_Mod    & $G_\beta$ & 7 & 5     & 0.85  & 0.15 & -0.019        & 0.15 & 0.098              & -0.684        & -0.194  & -0.028 & 0.495    & 1.0                     & -0.759 & -0.128 & 0.565   \\
SP\_Med  & $G_\beta$ & 7 & 5     & 0.85  & 0.15 & 0.021         & 0.15 & 0.103              & -0.475        & 0.203   & 0.044  & 0.503    & 1.013                   & 0.827  & 0.139  & 0.53    \\
KM\_Mod   & $G_\beta$ & 7 & 7     & 0.85  & 0.15 & 0.006         & 0.15 & 0.099              & -0.505        & 0.059   & 0.011  & 0.496    & 1.025                   & 0.23   & 0.039  & 0.862   \\
KM\_Med & $G_\beta$ & 7 & 7     & 0.85  & 0.15 & 0.017         & 0.15 & 0.102              & -0.454        & 0.163   & 0.037  & 0.498    & 1.028                   & 0.661  & 0.111  & 0.616   \\
SP\_Mod    & $G_\beta$ & 7 & 7     & 0.85  & 0.15 & -0.007        & 0.15 & 0.102              & -0.504        & -0.073  & -0.015 & 0.502    & 0.984                   & -0.295 & -0.05  & 0.823   \\
SP\_Med  & $G_\beta$ & 7 & 7     & 0.85  & 0.15 & 0.004         & 0.15 & 0.104              & -0.44         & 0.039   & 0.009  & 0.492    & 1.037                   & 0.162  & 0.027  & 0.902   \\
KM\_Mod   & $G_\beta$ & 1 & 1     & 0.8   & 0.2  & -0.122        & 0.15 & 0.104              & -0.948        & -1.173  & -0.129 & 0.476    & 0.956                   & -4.844 & -0.814 & 0.0     \\
KM\_Med & $G_\beta$ & 1 & 1     & 0.8   & 0.2  & -0.145        & 0.15 & 0.108              & -0.968        & -1.341  & -0.15  & 0.466    & 0.966                   & -5.76  & -0.968 & 0.0     \\
SP\_Mod    & $G_\beta$ & 1 & 1     & 0.8   & 0.2  & -0.137        & 0.15 & 0.104              & -0.961        & -1.319  & -0.142 & 0.475    & 0.947                   & -5.433 & -0.913 & 0.0     \\
SP\_Med  & $G_\beta$ & 1 & 1     & 0.8   & 0.2  & -0.144        & 0.15 & 0.108              & -0.968        & -1.337  & -0.149 & 0.475    & 0.934                   & -5.731 & -0.963 & 0.0     \\
KM\_Mod   & $G_\beta$ & 1 & 3     & 0.8   & 0.2  & -0.01         & 0.15 & 0.104              & -0.631        & -0.098  & -0.016 & 0.494    & 1.013                   & -0.403 & -0.068 & 0.76    \\
KM\_Med & $G_\beta$ & 1 & 3     & 0.8   & 0.2  & 0.027         & 0.15 & 0.105              & -0.549        & 0.253   & 0.048  & 0.513    & 0.98                    & 1.053  & 0.177  & 0.424   \\
SP\_Mod    & $G_\beta$ & 1 & 3     & 0.8   & 0.2  & 0.016         & 0.15 & 0.101              & -0.61         & 0.161   & 0.027  & 0.502    & 1.012                   & 0.643  & 0.108  & 0.626   \\
SP\_Med  & $G_\beta$ & 1 & 3     & 0.8   & 0.2  & -0.01         & 0.15 & 0.105              & -0.494        & -0.094  & -0.02  & 0.493    & 1.017                   & -0.391 & -0.066 & 0.767   \\
KM\_Mod   & $G_\beta$ & 1 & 5     & 0.8   & 0.2  & -0.05         & 0.15 & 0.107              & -0.795        & -0.469  & -0.063 & 0.494    & 0.965                   & -2.0   & -0.336 & 0.128   \\
KM\_Med & $G_\beta$ & 1 & 5     & 0.8   & 0.2  & -0.015        & 0.15 & 0.107              & -0.622        & -0.136  & -0.023 & 0.497    & 0.996                   & -0.576 & -0.097 & 0.662   \\
SP\_Mod    & $G_\beta$ & 1 & 5     & 0.8   & 0.2  & -0.012        & 0.15 & 0.102              & -0.594        & -0.12   & -0.021 & 0.501    & 0.982                   & -0.487 & -0.082 & 0.712   \\
SP\_Med  & $G_\beta$ & 1 & 5     & 0.8   & 0.2  & -0.019        & 0.15 & 0.104              & -0.696        & -0.18   & -0.027 & 0.491    & 1.016                   & -0.742 & -0.125 & 0.574   \\
KM\_Mod   & $G_\beta$ & 1 & 7     & 0.8   & 0.2  & 0.006         & 0.15 & 0.1                & -0.633        & 0.062   & 0.01   & 0.503    & 0.996                   & 0.246  & 0.041  & 0.852   \\
KM\_Med & $G_\beta$ & 1 & 7     & 0.8   & 0.2  & 0.02          & 0.15 & 0.104              & -0.543        & 0.188   & 0.036  & 0.498    & 1.033                   & 0.776  & 0.13   & 0.556   \\
SP\_Mod    & $G_\beta$ & 1 & 7     & 0.8   & 0.2  & -0.023        & 0.15 & 0.105              & -0.691        & -0.219  & -0.033 & 0.495    & 0.993                   & -0.91  & -0.153 & 0.49    \\
SP\_Med  & $G_\beta$ & 1 & 7     & 0.8   & 0.2  & 0.008         & 0.15 & 0.105              & -0.546        & 0.077   & 0.015  & 0.497    & 1.02                    & 0.322  & 0.054  & 0.807   \\
KM\_Mod   & $G_\beta$ & 3 & 1     & 0.8   & 0.2  & -0.103        & 0.15 & 0.104              & -0.905        & -0.991  & -0.114 & 0.478    & 0.971                   & -4.097 & -0.688 & 0.002   \\
KM\_Med & $G_\beta$ & 3 & 1     & 0.8   & 0.2  & -0.12         & 0.15 & 0.108              & -0.933        & -1.115  & -0.129 & 0.469    & 0.981                   & -4.761 & -0.8   & 0.0     \\
SP\_Mod    & $G_\beta$ & 3 & 1     & 0.8   & 0.2  & -0.109        & 0.15 & 0.104              & -0.92         & -1.053  & -0.119 & 0.479    & 0.961                   & -4.332 & -0.728 & 0.001   \\
SP\_Med  & $G_\beta$ & 3 & 1     & 0.8   & 0.2  & -0.104        & 0.15 & 0.106              & -0.908        & -0.973  & -0.114 & 0.48     & 0.958                   & -4.114 & -0.691 & 0.002   \\
KM\_Mod   & $G_\beta$ & 3 & 3     & 0.8   & 0.2  & -0.004        & 0.15 & 0.106              & -0.428        & -0.036  & -0.009 & 0.502    & 0.986                   & -0.153 & -0.026 & 0.908   \\
KM\_Med & $G_\beta$ & 3 & 3     & 0.8   & 0.2  & 0.023         & 0.15 & 0.109              & -0.4          & 0.208   & 0.056  & 0.511    & 0.981                   & 0.895  & 0.15   & 0.498   \\
SP\_Mod    & $G_\beta$ & 3 & 3     & 0.8   & 0.2  & -0.0          & 0.15 & 0.103              & -0.479        & -0.005  & -0.001 & 0.505    & 0.979                   & -0.02  & -0.003 & 0.988   \\
SP\_Med  & $G_\beta$ & 3 & 3     & 0.8   & 0.2  & -0.014        & 0.15 & 0.106              & -0.458        & -0.136  & -0.032 & 0.497    & 0.994                   & -0.575 & -0.097 & 0.663   \\
KM\_Mod   & $G_\beta$ & 3 & 5     & 0.8   & 0.2  & -0.041        & 0.15 & 0.106              & -0.707        & -0.389  & -0.059 & 0.494    & 0.975                   & -1.644 & -0.276 & 0.212   \\
KM\_Med & $G_\beta$ & 3 & 5     & 0.8   & 0.2  & -0.038        & 0.15 & 0.108              & -0.67         & -0.35   & -0.056 & 0.494    & 0.98                    & -1.497 & -0.251 & 0.255   \\
SP\_Mod    & $G_\beta$ & 3 & 5     & 0.8   & 0.2  & -0.032        & 0.15 & 0.101              & -0.641        & -0.317  & -0.05  & 0.494    & 0.988                   & -1.276 & -0.214 & 0.333   \\
SP\_Med  & $G_\beta$ & 3 & 5     & 0.8   & 0.2  & -0.026        & 0.15 & 0.105              & -0.648        & -0.249  & -0.04  & 0.491    & 1.005                   & -1.036 & -0.174 & 0.432   \\
KM\_Mod   & $G_\beta$ & 3 & 7     & 0.8   & 0.2  & -0.019        & 0.15 & 0.098              & -0.662        & -0.19   & -0.028 & 0.494    & 1.001                   & -0.741 & -0.124 & 0.575   \\
KM\_Med & $G_\beta$ & 3 & 7     & 0.8   & 0.2  & -0.041        & 0.15 & 0.103              & -0.708        & -0.396  & -0.058 & 0.486    & 1.008                   & -1.625 & -0.273 & 0.219   \\
SP\_Mod    & $G_\beta$ & 3 & 7     & 0.8   & 0.2  & -0.047        & 0.15 & 0.1                & -0.759        & -0.472  & -0.063 & 0.484    & 1.008                   & -1.884 & -0.316 & 0.154   \\
SP\_Med  & $G_\beta$ & 3 & 7     & 0.8   & 0.2  & -0.038        & 0.15 & 0.104              & -0.656        & -0.365  & -0.058 & 0.493    & 0.983                   & -1.511 & -0.254 & 0.252   \\
KM\_Mod   & $G_\beta$ & 5 & 1     & 0.8   & 0.2  & -0.097        & 0.15 & 0.105              & -0.897        & -0.927  & -0.108 & 0.482    & 0.962                   & -3.856 & -0.648 & 0.003   \\
KM\_Med & $G_\beta$ & 5 & 1     & 0.8   & 0.2  & -0.099        & 0.15 & 0.108              & -0.907        & -0.909  & -0.109 & 0.484    & 0.95                    & -3.912 & -0.657 & 0.003   \\
SP\_Mod    & $G_\beta$ & 5 & 1     & 0.8   & 0.2  & -0.092        & 0.15 & 0.103              & -0.892        & -0.894  & -0.103 & 0.482    & 0.969                   & -3.65  & -0.613 & 0.006   \\
SP\_Med  & $G_\beta$ & 5 & 1     & 0.8   & 0.2  & -0.098        & 0.15 & 0.107              & -0.903        & -0.915  & -0.108 & 0.485    & 0.946                   & -3.879 & -0.652 & 0.003   \\
KM\_Mod   & $G_\beta$ & 5 & 3     & 0.8   & 0.2  & 0.002         & 0.15 & 0.103              & -0.608        & 0.016   & 0.003  & 0.499    & 1.004                   & 0.067  & 0.011  & 0.96    \\
KM\_Med & $G_\beta$ & 5 & 3     & 0.8   & 0.2  & 0.016         & 0.15 & 0.106              & -0.673        & 0.153   & 0.024  & 0.506    & 0.994                   & 0.641  & 0.108  & 0.627   \\
SP\_Mod    & $G_\beta$ & 5 & 3     & 0.8   & 0.2  & 0.04          & 0.15 & 0.103              & -0.385        & 0.388   & 0.104  & 0.51     & 1.007                   & 1.587  & 0.267  & 0.229   \\
SP\_Med  & $G_\beta$ & 5 & 3     & 0.8   & 0.2  & 0.027         & 0.15 & 0.106              & -0.379        & 0.256   & 0.072  & 0.5      & 1.032                   & 1.075  & 0.181  & 0.415   \\
KM\_Mod   & $G_\beta$ & 5 & 5     & 0.8   & 0.2  & -0.057        & 0.15 & 0.105              & -0.83         & -0.546  & -0.069 & 0.488    & 0.981                   & -2.265 & -0.381 & 0.085   \\
KM\_Med & $G_\beta$ & 5 & 5     & 0.8   & 0.2  & -0.06         & 0.15 & 0.106              & -0.791        & -0.561  & -0.075 & 0.49     & 0.969                   & -2.365 & -0.397 & 0.072   \\
SP\_Mod    & $G_\beta$ & 5 & 5     & 0.8   & 0.2  & -0.082        & 0.15 & 0.102              & -0.869        & -0.8    & -0.094 & 0.484    & 0.97                    & -3.238 & -0.544 & 0.014   \\
SP\_Med  & $G_\beta$ & 5 & 5     & 0.8   & 0.2  & -0.043        & 0.15 & 0.105              & -0.738        & -0.405  & -0.058 & 0.492    & 0.983                   & -1.692 & -0.284 & 0.199   \\
KM\_Mod   & $G_\beta$ & 5 & 7     & 0.8   & 0.2  & 0.028         & 0.15 & 0.101              & -0.507        & 0.277   & 0.055  & 0.506    & 1.007                   & 1.108  & 0.186  & 0.4     \\
KM\_Med & $G_\beta$ & 5 & 7     & 0.8   & 0.2  & 0.026         & 0.15 & 0.104              & -0.51         & 0.252   & 0.051  & 0.505    & 1.012                   & 1.041  & 0.175  & 0.43    \\
SP\_Mod    & $G_\beta$ & 5 & 7     & 0.8   & 0.2  & 0.027         & 0.15 & 0.104              & -0.505        & 0.26    & 0.053  & 0.503    & 1.021                   & 1.068  & 0.179  & 0.418   \\
SP\_Med  & $G_\beta$ & 5 & 7     & 0.8   & 0.2  & 0.008         & 0.15 & 0.105              & -0.457        & 0.076   & 0.018  & 0.499    & 1.015                   & 0.318  & 0.053  & 0.809   \\
KM\_Mod   & $G_\beta$ & 7 & 1     & 0.8   & 0.2  & -0.11         & 0.15 & 0.104              & -0.939        & -1.056  & -0.117 & 0.476    & 0.968                   & -4.359 & -0.732 & 0.001   \\
KM\_Med & $G_\beta$ & 7 & 1     & 0.8   & 0.2  & -0.077        & 0.15 & 0.106              & -0.889        & -0.728  & -0.087 & 0.481    & 0.983                   & -3.066 & -0.515 & 0.02    \\
SP\_Mod    & $G_\beta$ & 7 & 1     & 0.8   & 0.2  & -0.099        & 0.15 & 0.104              & -0.897        & -0.953  & -0.111 & 0.487    & 0.941                   & -3.944 & -0.663 & 0.003   \\
SP\_Med  & $G_\beta$ & 7 & 1     & 0.8   & 0.2  & -0.113        & 0.15 & 0.108              & -0.921        & -1.044  & -0.122 & 0.481    & 0.946                   & -4.474 & -0.752 & 0.001   \\
KM\_Mod   & $G_\beta$ & 7 & 3     & 0.8   & 0.2  & -0.026        & 0.15 & 0.104              & -0.713        & -0.252  & -0.037 & 0.496    & 0.987                   & -1.041 & -0.175 & 0.43    \\
KM\_Med & $G_\beta$ & 7 & 3     & 0.8   & 0.2  & -0.028        & 0.15 & 0.107              & -0.684        & -0.267  & -0.042 & 0.497    & 0.977                   & -1.131 & -0.19  & 0.391   \\
SP\_Mod    & $G_\beta$ & 7 & 3     & 0.8   & 0.2  & -0.008        & 0.15 & 0.103              & -0.566        & -0.075  & -0.014 & 0.501    & 0.986                   & -0.305 & -0.051 & 0.817   \\
SP\_Med  & $G_\beta$ & 7 & 3     & 0.8   & 0.2  & -0.024        & 0.15 & 0.105              & -0.65         & -0.227  & -0.037 & 0.492    & 1.004                   & -0.946 & -0.159 & 0.473   \\
KM\_Mod   & $G_\beta$ & 7 & 5     & 0.8   & 0.2  & -0.01         & 0.15 & 0.106              & -0.759        & -0.098  & -0.014 & 0.499    & 0.992                   & -0.412 & -0.069 & 0.755   \\
KM\_Med & $G_\beta$ & 7 & 5     & 0.8   & 0.2  & 0.008         & 0.15 & 0.106              & -0.629        & 0.078   & 0.013  & 0.503    & 0.998                   & 0.327  & 0.055  & 0.804   \\
SP\_Mod    & $G_\beta$ & 7 & 5     & 0.8   & 0.2  & -0.027        & 0.15 & 0.101              & -0.711        & -0.273  & -0.039 & 0.494    & 0.992                   & -1.089 & -0.183 & 0.409   \\
SP\_Med  & $G_\beta$ & 7 & 5     & 0.8   & 0.2  & -0.0          & 0.15 & 0.103              & -0.599        & -0.001  & -0.0   & 0.498    & 1.007                   & -0.003 & -0.001 & 0.998   \\
KM\_Mod   & $G_\beta$ & 7 & 7     & 0.8   & 0.2  & 0.006         & 0.15 & 0.1                & -0.517        & 0.064   & 0.012  & 0.501    & 1.004                   & 0.254  & 0.043  & 0.847   \\
KM\_Med & $G_\beta$ & 7 & 7     & 0.8   & 0.2  & 0.009         & 0.15 & 0.102              & -0.479        & 0.09    & 0.019  & 0.495    & 1.03                    & 0.363  & 0.061  & 0.783   \\
SP\_Mod    & $G_\beta$ & 7 & 7     & 0.8   & 0.2  & 0.0           & 0.15 & 0.102              & -0.43         & 0.002   & 0.0    & 0.495    & 1.021                   & 0.007  & 0.001  & 0.996   \\
SP\_Med  & $G_\beta$ & 7 & 7     & 0.8   & 0.2  & 0.02          & 0.15 & 0.103              & -0.455        & 0.191   & 0.044  & 0.497    & 1.036                   & 0.786  & 0.132  & 0.551   \\
KM\_Mod   & $G_\beta$ & 1 & 1     & 0.75  & 0.25 & -0.129        & 0.15 & 0.106              & -0.956        & -1.219  & -0.135 & 0.471    & 0.968                   & -5.112 & -0.859 & 0.0     \\
KM\_Med & $G_\beta$ & 1 & 1     & 0.75  & 0.25 & -0.13         & 0.15 & 0.108              & -0.956        & -1.2    & -0.135 & 0.475    & 0.949                   & -5.139 & -0.863 & 0.0     \\
SP\_Mod    & $G_\beta$ & 1 & 1     & 0.75  & 0.25 & -0.147        & 0.15 & 0.105              & -0.97         & -1.393  & -0.151 & 0.474    & 0.937                   & -5.83  & -0.979 & 0.0     \\
SP\_Med  & $G_\beta$ & 1 & 1     & 0.75  & 0.25 & -0.135        & 0.15 & 0.109              & -0.962        & -1.235  & -0.14  & 0.477    & 0.936                   & -5.34  & -0.897 & 0.0     \\
KM\_Mod   & $G_\beta$ & 1 & 3     & 0.75  & 0.25 & 0.001         & 0.15 & 0.103              & -0.626        & 0.006   & 0.001  & 0.495    & 1.02                    & 0.024  & 0.004  & 0.985   \\
KM\_Med & $G_\beta$ & 1 & 3     & 0.75  & 0.25 & 0.02          & 0.15 & 0.104              & -0.581        & 0.193   & 0.034  & 0.507    & 0.994                   & 0.792  & 0.133  & 0.548   \\
SP\_Mod    & $G_\beta$ & 1 & 3     & 0.75  & 0.25 & 0.018         & 0.15 & 0.102              & -0.629        & 0.177   & 0.029  & 0.504    & 1.007                   & 0.715  & 0.12   & 0.587   \\
SP\_Med  & $G_\beta$ & 1 & 3     & 0.75  & 0.25 & 0.009         & 0.15 & 0.104              & -0.565        & 0.088   & 0.016  & 0.498    & 1.02                    & 0.363  & 0.061  & 0.783   \\
KM\_Mod   & $G_\beta$ & 1 & 5     & 0.75  & 0.25 & -0.042        & 0.15 & 0.109              & -0.754        & -0.386  & -0.056 & 0.499    & 0.958                   & -1.664 & -0.28  & 0.206   \\
KM\_Med & $G_\beta$ & 1 & 5     & 0.75  & 0.25 & -0.017        & 0.15 & 0.108              & -0.6          & -0.155  & -0.028 & 0.494    & 1.004                   & -0.667 & -0.112 & 0.613   \\
SP\_Mod    & $G_\beta$ & 1 & 5     & 0.75  & 0.25 & -0.013        & 0.15 & 0.105              & -0.622        & -0.123  & -0.021 & 0.503    & 0.972                   & -0.515 & -0.086 & 0.696   \\
SP\_Med  & $G_\beta$ & 1 & 5     & 0.75  & 0.25 & -0.036        & 0.15 & 0.105              & -0.73         & -0.343  & -0.049 & 0.488    & 1.004                   & -1.43  & -0.24  & 0.278   \\
KM\_Mod   & $G_\beta$ & 1 & 7     & 0.75  & 0.25 & 0.02          & 0.15 & 0.102              & -0.58         & 0.192   & 0.034  & 0.502    & 1.017                   & 0.775  & 0.13   & 0.556   \\
KM\_Med & $G_\beta$ & 1 & 7     & 0.75  & 0.25 & 0.003         & 0.15 & 0.105              & -0.588        & 0.032   & 0.006  & 0.497    & 1.017                   & 0.135  & 0.023  & 0.919   \\
SP\_Mod    & $G_\beta$ & 1 & 7     & 0.75  & 0.25 & -0.029        & 0.15 & 0.106              & -0.716        & -0.27   & -0.04  & 0.501    & 0.962                   & -1.132 & -0.19  & 0.39    \\
SP\_Med  & $G_\beta$ & 1 & 7     & 0.75  & 0.25 & 0.002         & 0.15 & 0.106              & -0.626        & 0.015   & 0.003  & 0.505    & 0.981                   & 0.063  & 0.011  & 0.962   \\
KM\_Mod   & $G_\beta$ & 3 & 1     & 0.75  & 0.25 & -0.107        & 0.15 & 0.106              & -0.918        & -1.012  & -0.117 & 0.471    & 0.991                   & -4.256 & -0.715 & 0.001   \\
KM\_Med & $G_\beta$ & 3 & 1     & 0.75  & 0.25 & -0.138        & 0.15 & 0.108              & -0.953        & -1.28   & -0.145 & 0.472    & 0.95                    & -5.495 & -0.923 & 0.0     \\
SP\_Mod    & $G_\beta$ & 3 & 1     & 0.75  & 0.25 & -0.127        & 0.15 & 0.105              & -0.946        & -1.205  & -0.134 & 0.472    & 0.967                   & -5.044 & -0.847 & 0.0     \\
SP\_Med  & $G_\beta$ & 3 & 1     & 0.75  & 0.25 & -0.125        & 0.15 & 0.108              & -0.94         & -1.164  & -0.133 & 0.475    & 0.953                   & -4.967 & -0.834 & 0.0     \\
KM\_Mod   & $G_\beta$ & 3 & 3     & 0.75  & 0.25 & -0.013        & 0.15 & 0.108              & -0.439        & -0.124  & -0.03  & 0.5      & 0.984                   & -0.528 & -0.089 & 0.689   \\
KM\_Med & $G_\beta$ & 3 & 3     & 0.75  & 0.25 & 0.014         & 0.15 & 0.109              & -0.389        & 0.125   & 0.035  & 0.515    & 0.957                   & 0.54   & 0.091  & 0.682   \\
SP\_Mod    & $G_\beta$ & 3 & 3     & 0.75  & 0.25 & 0.011         & 0.15 & 0.104              & -0.443        & 0.109   & 0.026  & 0.507    & 0.985                   & 0.451  & 0.076  & 0.732   \\
SP\_Med  & $G_\beta$ & 3 & 3     & 0.75  & 0.25 & 0.007         & 0.15 & 0.108              & -0.374        & 0.062   & 0.018  & 0.511    & 0.965                   & 0.266  & 0.045  & 0.84    \\
KM\_Mod   & $G_\beta$ & 3 & 5     & 0.75  & 0.25 & -0.042        & 0.15 & 0.107              & -0.704        & -0.397  & -0.06  & 0.493    & 0.978                   & -1.678 & -0.282 & 0.202   \\
KM\_Med & $G_\beta$ & 3 & 5     & 0.75  & 0.25 & -0.032        & 0.15 & 0.109              & -0.635        & -0.289  & -0.05  & 0.495    & 0.983                   & -1.255 & -0.211 & 0.34    \\
SP\_Mod    & $G_\beta$ & 3 & 5     & 0.75  & 0.25 & -0.037        & 0.15 & 0.104              & -0.687        & -0.358  & -0.054 & 0.494    & 0.98                    & -1.483 & -0.249 & 0.26    \\
SP\_Med  & $G_\beta$ & 3 & 5     & 0.75  & 0.25 & -0.033        & 0.15 & 0.107              & -0.673        & -0.306  & -0.049 & 0.489    & 1.004                   & -1.296 & -0.218 & 0.326   \\
KM\_Mod   & $G_\beta$ & 3 & 7     & 0.75  & 0.25 & -0.008        & 0.15 & 0.098              & -0.634        & -0.086  & -0.013 & 0.498    & 0.999                   & -0.337 & -0.057 & 0.798   \\
KM\_Med & $G_\beta$ & 3 & 7     & 0.75  & 0.25 & -0.042        & 0.15 & 0.103              & -0.719        & -0.41   & -0.059 & 0.489    & 0.993                   & -1.678 & -0.282 & 0.204   \\
SP\_Mod    & $G_\beta$ & 3 & 7     & 0.75  & 0.25 & -0.049        & 0.15 & 0.101              & -0.739        & -0.487  & -0.067 & 0.49     & 0.985                   & -1.958 & -0.329 & 0.138   \\
SP\_Med  & $G_\beta$ & 3 & 7     & 0.75  & 0.25 & -0.033        & 0.15 & 0.105              & -0.626        & -0.314  & -0.053 & 0.501    & 0.957                   & -1.312 & -0.22  & 0.32    \\
KM\_Mod   & $G_\beta$ & 5 & 1     & 0.75  & 0.25 & -0.113        & 0.15 & 0.107              & -0.926        & -1.057  & -0.122 & 0.474    & 0.974                   & -4.472 & -0.751 & 0.001   \\
KM\_Med & $G_\beta$ & 5 & 1     & 0.75  & 0.25 & -0.094        & 0.15 & 0.109              & -0.9          & -0.867  & -0.105 & 0.486    & 0.948                   & -3.741 & -0.628 & 0.004   \\
SP\_Mod    & $G_\beta$ & 5 & 1     & 0.75  & 0.25 & -0.109        & 0.15 & 0.105              & -0.92         & -1.041  & -0.119 & 0.474    & 0.977                   & -4.339 & -0.729 & 0.001   \\
SP\_Med  & $G_\beta$ & 5 & 1     & 0.75  & 0.25 & -0.107        & 0.15 & 0.107              & -0.924        & -0.999  & -0.116 & 0.478    & 0.961                   & -4.244 & -0.713 & 0.001   \\
KM\_Mod   & $G_\beta$ & 5 & 3     & 0.75  & 0.25 & 0.007         & 0.15 & 0.103              & -0.563        & 0.069   & 0.013  & 0.495    & 1.029                   & 0.284  & 0.048  & 0.83    \\
KM\_Med & $G_\beta$ & 5 & 3     & 0.75  & 0.25 & 0.015         & 0.15 & 0.105              & -0.631        & 0.146   & 0.024  & 0.51     & 0.98                    & 0.609  & 0.102  & 0.644   \\
SP\_Mod    & $G_\beta$ & 5 & 3     & 0.75  & 0.25 & 0.029         & 0.15 & 0.104              & -0.383        & 0.278   & 0.075  & 0.507    & 1.005                   & 1.146  & 0.193  & 0.385   \\
SP\_Med  & $G_\beta$ & 5 & 3     & 0.75  & 0.25 & 0.033         & 0.15 & 0.107              & -0.426        & 0.31    & 0.078  & 0.505    & 1.02                    & 1.316  & 0.221  & 0.319   \\
KM\_Mod   & $G_\beta$ & 5 & 5     & 0.75  & 0.25 & -0.052        & 0.15 & 0.105              & -0.786        & -0.494  & -0.066 & 0.493    & 0.968                   & -2.061 & -0.346 & 0.118   \\
KM\_Med & $G_\beta$ & 5 & 5     & 0.75  & 0.25 & -0.072        & 0.15 & 0.108              & -0.851        & -0.668  & -0.085 & 0.487    & 0.968                   & -2.859 & -0.48  & 0.03    \\
SP\_Mod    & $G_\beta$ & 5 & 5     & 0.75  & 0.25 & -0.096        & 0.15 & 0.106              & -0.904        & -0.908  & -0.106 & 0.484    & 0.956                   & -3.815 & -0.641 & 0.004   \\
SP\_Med  & $G_\beta$ & 5 & 5     & 0.75  & 0.25 & -0.046        & 0.15 & 0.106              & -0.745        & -0.433  & -0.062 & 0.489    & 0.99                    & -1.827 & -0.307 & 0.166   \\
KM\_Mod   & $G_\beta$ & 5 & 7     & 0.75  & 0.25 & 0.033         & 0.15 & 0.101              & -0.488        & 0.325   & 0.067  & 0.506    & 1.014                   & 1.306  & 0.219  & 0.322   \\
KM\_Med & $G_\beta$ & 5 & 7     & 0.75  & 0.25 & 0.019         & 0.15 & 0.104              & -0.509        & 0.182   & 0.037  & 0.503    & 1.012                   & 0.748  & 0.126  & 0.57    \\
SP\_Mod    & $G_\beta$ & 5 & 7     & 0.75  & 0.25 & 0.023         & 0.15 & 0.101              & -0.455        & 0.225   & 0.05   & 0.503    & 1.015                   & 0.904  & 0.152  & 0.493   \\
SP\_Med  & $G_\beta$ & 5 & 7     & 0.75  & 0.25 & 0.021         & 0.15 & 0.106              & -0.428        & 0.193   & 0.048  & 0.511    & 0.981                   & 0.815  & 0.137  & 0.536   \\
KM\_Mod   & $G_\beta$ & 7 & 1     & 0.75  & 0.25 & -0.114        & 0.15 & 0.106              & -0.942        & -1.08   & -0.121 & 0.474    & 0.971                   & -4.538 & -0.762 & 0.001   \\
KM\_Med & $G_\beta$ & 7 & 1     & 0.75  & 0.25 & -0.092        & 0.15 & 0.107              & -0.913        & -0.86   & -0.101 & 0.484    & 0.956                   & -3.647 & -0.613 & 0.006   \\
SP\_Mod    & $G_\beta$ & 7 & 1     & 0.75  & 0.25 & -0.091        & 0.15 & 0.106              & -0.88         & -0.858  & -0.103 & 0.483    & 0.963                   & -3.593 & -0.604 & 0.006   \\
SP\_Med  & $G_\beta$ & 7 & 1     & 0.75  & 0.25 & -0.118        & 0.15 & 0.109              & -0.936        & -1.085  & -0.126 & 0.481    & 0.94                    & -4.674 & -0.785 & 0.0     \\
KM\_Mod   & $G_\beta$ & 7 & 3     & 0.75  & 0.25 & -0.026        & 0.15 & 0.105              & -0.706        & -0.247  & -0.037 & 0.494    & 0.996                   & -1.027 & -0.173 & 0.436   \\
KM\_Med & $G_\beta$ & 7 & 3     & 0.75  & 0.25 & -0.014        & 0.15 & 0.107              & -0.571        & -0.134  & -0.025 & 0.504    & 0.968                   & -0.567 & -0.095 & 0.667   \\
SP\_Mod    & $G_\beta$ & 7 & 3     & 0.75  & 0.25 & -0.007        & 0.15 & 0.103              & -0.624        & -0.064  & -0.011 & 0.501    & 0.989                   & -0.263 & -0.044 & 0.842   \\
SP\_Med  & $G_\beta$ & 7 & 3     & 0.75  & 0.25 & -0.022        & 0.15 & 0.107              & -0.7          & -0.206  & -0.032 & 0.503    & 0.964                   & -0.879 & -0.148 & 0.505   \\
KM\_Mod   & $G_\beta$ & 7 & 5     & 0.75  & 0.25 & -0.024        & 0.15 & 0.106              & -0.774        & -0.224  & -0.031 & 0.494    & 0.998                   & -0.939 & -0.158 & 0.476   \\
KM\_Med & $G_\beta$ & 7 & 5     & 0.75  & 0.25 & -0.002        & 0.15 & 0.106              & -0.599        & -0.015  & -0.003 & 0.498    & 1.007                   & -0.063 & -0.011 & 0.962   \\
SP\_Mod    & $G_\beta$ & 7 & 5     & 0.75  & 0.25 & -0.02         & 0.15 & 0.103              & -0.687        & -0.198  & -0.03  & 0.496    & 0.991                   & -0.813 & -0.137 & 0.538   \\
SP\_Med  & $G_\beta$ & 7 & 5     & 0.75  & 0.25 & -0.001        & 0.15 & 0.104              & -0.586        & -0.009  & -0.002 & 0.496    & 1.016                   & -0.036 & -0.006 & 0.978   \\
KM\_Mod   & $G_\beta$ & 7 & 7     & 0.75  & 0.25 & -0.001        & 0.15 & 0.102              & -0.587        & -0.007  & -0.001 & 0.498    & 1.009                   & -0.028 & -0.005 & 0.983   \\
KM\_Med & $G_\beta$ & 7 & 7     & 0.75  & 0.25 & 0.005         & 0.15 & 0.103              & -0.534        & 0.045   & 0.009  & 0.495    & 1.028                   & 0.185  & 0.031  & 0.888   \\
SP\_Mod    & $G_\beta$ & 7 & 7     & 0.75  & 0.25 & -0.01         & 0.15 & 0.102              & -0.508        & -0.097  & -0.019 & 0.494    & 1.013                   & -0.392 & -0.066 & 0.766   \\
SP\_Med  & $G_\beta$ & 7 & 7     & 0.75  & 0.25 & 0.022         & 0.15 & 0.105              & -0.457        & 0.209   & 0.048  & 0.508    & 0.994                   & 0.869  & 0.146  & 0.51    \\
KM\_Mod   & $G_\beta$ & 1 & 1     & 0.7   & 0.3  & -0.137        & 0.15 & 0.109              & -0.962        & -1.259  & -0.143 & 0.474    & 0.946                   & -5.441 & -0.914 & 0.0     \\
KM\_Med & $G_\beta$ & 1 & 1     & 0.7   & 0.3  & -0.143        & 0.15 & 0.111              & -0.968        & -1.294  & -0.148 & 0.475    & 0.93                    & -5.694 & -0.957 & 0.0     \\
SP\_Mod    & $G_\beta$ & 1 & 1     & 0.7   & 0.3  & -0.136        & 0.15 & 0.106              & -0.961        & -1.278  & -0.141 & 0.476    & 0.94                    & -5.394 & -0.906 & 0.0     \\
SP\_Med  & $G_\beta$ & 1 & 1     & 0.7   & 0.3  & -0.136        & 0.15 & 0.11               & -0.961        & -1.235  & -0.141 & 0.474    & 0.943                   & -5.383 & -0.904 & 0.0     \\
KM\_Mod   & $G_\beta$ & 1 & 3     & 0.7   & 0.3  & 0.003         & 0.15 & 0.102              & -0.628        & 0.031   & 0.005  & 0.494    & 1.028                   & 0.124  & 0.021  & 0.925   \\
KM\_Med & $G_\beta$ & 1 & 3     & 0.7   & 0.3  & 0.033         & 0.15 & 0.102              & -0.6          & 0.327   & 0.056  & 0.509    & 1.005                   & 1.324  & 0.222  & 0.315   \\
SP\_Mod    & $G_\beta$ & 1 & 3     & 0.7   & 0.3  & 0.01          & 0.15 & 0.102              & -0.601        & 0.093   & 0.016  & 0.498    & 1.021                   & 0.377  & 0.063  & 0.775   \\
SP\_Med  & $G_\beta$ & 1 & 3     & 0.7   & 0.3  & -0.003        & 0.15 & 0.106              & -0.575        & -0.032  & -0.006 & 0.494    & 1.02                    & -0.134 & -0.023 & 0.919   \\
KM\_Mod   & $G_\beta$ & 1 & 5     & 0.7   & 0.3  & -0.042        & 0.15 & 0.109              & -0.756        & -0.39   & -0.056 & 0.494    & 0.977                   & -1.683 & -0.283 & 0.201   \\
KM\_Med & $G_\beta$ & 1 & 5     & 0.7   & 0.3  & -0.019        & 0.15 & 0.109              & -0.592        & -0.172  & -0.032 & 0.5      & 0.976                   & -0.747 & -0.125 & 0.571   \\
SP\_Mod    & $G_\beta$ & 1 & 5     & 0.7   & 0.3  & -0.023        & 0.15 & 0.107              & -0.671        & -0.218  & -0.035 & 0.5      & 0.973                   & -0.925 & -0.155 & 0.483   \\
SP\_Med  & $G_\beta$ & 1 & 5     & 0.7   & 0.3  & -0.048        & 0.15 & 0.106              & -0.779        & -0.45   & -0.061 & 0.486    & 1.002                   & -1.887 & -0.317 & 0.152   \\
KM\_Mod   & $G_\beta$ & 1 & 7     & 0.7   & 0.3  & 0.024         & 0.15 & 0.103              & -0.519        & 0.23    & 0.046  & 0.507    & 1.001                   & 0.942  & 0.158  & 0.475   \\
KM\_Med & $G_\beta$ & 1 & 7     & 0.7   & 0.3  & -0.001        & 0.15 & 0.105              & -0.59         & -0.012  & -0.002 & 0.497    & 1.012                   & -0.052 & -0.009 & 0.969   \\
SP\_Mod    & $G_\beta$ & 1 & 7     & 0.7   & 0.3  & -0.033        & 0.15 & 0.106              & -0.709        & -0.311  & -0.047 & 0.496    & 0.976                   & -1.308 & -0.22  & 0.32    \\
SP\_Med  & $G_\beta$ & 1 & 7     & 0.7   & 0.3  & -0.009        & 0.15 & 0.108              & -0.678        & -0.081  & -0.013 & 0.503    & 0.978                   & -0.345 & -0.058 & 0.793   \\
KM\_Mod   & $G_\beta$ & 3 & 1     & 0.7   & 0.3  & -0.112        & 0.15 & 0.108              & -0.927        & -1.038  & -0.121 & 0.479    & 0.954                   & -4.464 & -0.75  & 0.001   \\
KM\_Med & $G_\beta$ & 3 & 1     & 0.7   & 0.3  & -0.141        & 0.15 & 0.109              & -0.957        & -1.297  & -0.148 & 0.468    & 0.962                   & -5.607 & -0.942 & 0.0     \\
SP\_Mod    & $G_\beta$ & 3 & 1     & 0.7   & 0.3  & -0.133        & 0.15 & 0.106              & -0.952        & -1.255  & -0.14  & 0.471    & 0.965                   & -5.277 & -0.886 & 0.0     \\
SP\_Med  & $G_\beta$ & 3 & 1     & 0.7   & 0.3  & -0.116        & 0.15 & 0.108              & -0.927        & -1.069  & -0.125 & 0.477    & 0.955                   & -4.6   & -0.773 & 0.0     \\
KM\_Mod   & $G_\beta$ & 3 & 3     & 0.7   & 0.3  & 0.004         & 0.15 & 0.107              & -0.398        & 0.042   & 0.011  & 0.502    & 0.998                   & 0.178  & 0.03   & 0.893   \\
KM\_Med & $G_\beta$ & 3 & 3     & 0.7   & 0.3  & 0.011         & 0.15 & 0.108              & -0.427        & 0.099   & 0.025  & 0.514    & 0.956                   & 0.423  & 0.071  & 0.749   \\
SP\_Mod    & $G_\beta$ & 3 & 3     & 0.7   & 0.3  & 0.006         & 0.15 & 0.105              & -0.408        & 0.06    & 0.015  & 0.503    & 0.997                   & 0.25   & 0.042  & 0.85    \\
SP\_Med  & $G_\beta$ & 3 & 3     & 0.7   & 0.3  & 0.004         & 0.15 & 0.108              & -0.402        & 0.039   & 0.01   & 0.505    & 0.984                   & 0.166  & 0.028  & 0.9     \\
KM\_Mod   & $G_\beta$ & 3 & 5     & 0.7   & 0.3  & -0.038        & 0.15 & 0.107              & -0.698        & -0.355  & -0.054 & 0.492    & 0.986                   & -1.509 & -0.254 & 0.252   \\
KM\_Med & $G_\beta$ & 3 & 5     & 0.7   & 0.3  & -0.04         & 0.15 & 0.111              & -0.7          & -0.361  & -0.057 & 0.497    & 0.964                   & -1.591 & -0.267 & 0.226   \\
SP\_Mod    & $G_\beta$ & 3 & 5     & 0.7   & 0.3  & -0.043        & 0.15 & 0.107              & -0.707        & -0.407  & -0.061 & 0.499    & 0.955                   & -1.725 & -0.29  & 0.19    \\
SP\_Med  & $G_\beta$ & 3 & 5     & 0.7   & 0.3  & -0.034        & 0.15 & 0.107              & -0.656        & -0.317  & -0.052 & 0.491    & 0.994                   & -1.351 & -0.227 & 0.305   \\
KM\_Mod   & $G_\beta$ & 3 & 7     & 0.7   & 0.3  & -0.022        & 0.15 & 0.1                & -0.705        & -0.224  & -0.032 & 0.497    & 0.986                   & -0.89  & -0.15  & 0.5     \\
KM\_Med & $G_\beta$ & 3 & 7     & 0.7   & 0.3  & -0.044        & 0.15 & 0.103              & -0.743        & -0.427  & -0.059 & 0.488    & 0.997                   & -1.74  & -0.292 & 0.188   \\
SP\_Mod    & $G_\beta$ & 3 & 7     & 0.7   & 0.3  & -0.054        & 0.15 & 0.102              & -0.776        & -0.525  & -0.069 & 0.49     & 0.976                   & -2.126 & -0.357 & 0.108   \\
SP\_Med  & $G_\beta$ & 3 & 7     & 0.7   & 0.3  & -0.044        & 0.15 & 0.106              & -0.711        & -0.416  & -0.062 & 0.497    & 0.959                   & -1.749 & -0.294 & 0.185   \\
KM\_Mod   & $G_\beta$ & 5 & 1     & 0.7   & 0.3  & -0.12         & 0.15 & 0.108              & -0.937        & -1.111  & -0.128 & 0.474    & 0.963                   & -4.761 & -0.8   & 0.0     \\
KM\_Med & $G_\beta$ & 5 & 1     & 0.7   & 0.3  & -0.108        & 0.15 & 0.11               & -0.923        & -0.982  & -0.117 & 0.484    & 0.938                   & -4.276 & -0.718 & 0.001   \\
SP\_Mod    & $G_\beta$ & 5 & 1     & 0.7   & 0.3  & -0.103        & 0.15 & 0.106              & -0.908        & -0.977  & -0.114 & 0.478    & 0.971                   & -4.09  & -0.687 & 0.002   \\
SP\_Med  & $G_\beta$ & 5 & 1     & 0.7   & 0.3  & -0.108        & 0.15 & 0.108              & -0.923        & -0.995  & -0.117 & 0.484    & 0.938                   & -4.269 & -0.717 & 0.001   \\
KM\_Mod   & $G_\beta$ & 5 & 3     & 0.7   & 0.3  & 0.001         & 0.15 & 0.104              & -0.559        & 0.006   & 0.001  & 0.493    & 1.029                   & 0.026  & 0.004  & 0.984   \\
KM\_Med & $G_\beta$ & 5 & 3     & 0.7   & 0.3  & 0.008         & 0.15 & 0.106              & -0.587        & 0.074   & 0.013  & 0.51     & 0.969                   & 0.314  & 0.053  & 0.812   \\
SP\_Mod    & $G_\beta$ & 5 & 3     & 0.7   & 0.3  & 0.019         & 0.15 & 0.104              & -0.383        & 0.181   & 0.049  & 0.503    & 1.009                   & 0.747  & 0.126  & 0.571   \\
SP\_Med  & $G_\beta$ & 5 & 3     & 0.7   & 0.3  & 0.041         & 0.15 & 0.108              & -0.373        & 0.382   & 0.11   & 0.509    & 1.015                   & 1.634  & 0.275  & 0.217   \\
KM\_Mod   & $G_\beta$ & 5 & 5     & 0.7   & 0.3  & -0.068        & 0.15 & 0.107              & -0.849        & -0.64   & -0.08  & 0.488    & 0.968                   & -2.712 & -0.456 & 0.039   \\
KM\_Med & $G_\beta$ & 5 & 5     & 0.7   & 0.3  & -0.072        & 0.15 & 0.109              & -0.852        & -0.659  & -0.084 & 0.486    & 0.973                   & -2.854 & -0.479 & 0.03    \\
SP\_Mod    & $G_\beta$ & 5 & 5     & 0.7   & 0.3  & -0.096        & 0.15 & 0.107              & -0.9          & -0.901  & -0.107 & 0.489    & 0.933                   & -3.829 & -0.643 & 0.004   \\
SP\_Med  & $G_\beta$ & 5 & 5     & 0.7   & 0.3  & -0.053        & 0.15 & 0.107              & -0.776        & -0.495  & -0.069 & 0.49     & 0.976                   & -2.11  & -0.354 & 0.11    \\
KM\_Mod   & $G_\beta$ & 5 & 7     & 0.7   & 0.3  & 0.036         & 0.15 & 0.1                & -0.421        & 0.363   & 0.086  & 0.509    & 1.006                   & 1.441  & 0.242  & 0.273   \\
KM\_Med & $G_\beta$ & 5 & 7     & 0.7   & 0.3  & 0.025         & 0.15 & 0.101              & -0.528        & 0.244   & 0.046  & 0.503    & 1.019                   & 0.973  & 0.163  & 0.46    \\
SP\_Mod    & $G_\beta$ & 5 & 7     & 0.7   & 0.3  & 0.011         & 0.15 & 0.102              & -0.478        & 0.109   & 0.023  & 0.504    & 0.998                   & 0.441  & 0.074  & 0.738   \\
SP\_Med  & $G_\beta$ & 5 & 7     & 0.7   & 0.3  & 0.006         & 0.15 & 0.107              & -0.535        & 0.053   & 0.011  & 0.507    & 0.979                   & 0.228  & 0.038  & 0.863   \\
KM\_Mod   & $G_\beta$ & 7 & 1     & 0.7   & 0.3  & -0.097        & 0.15 & 0.106              & -0.923        & -0.912  & -0.105 & 0.479    & 0.971                   & -3.848 & -0.646 & 0.003   \\
KM\_Med & $G_\beta$ & 7 & 1     & 0.7   & 0.3  & -0.096        & 0.15 & 0.108              & -0.921        & -0.887  & -0.104 & 0.48     & 0.967                   & -3.812 & -0.64  & 0.004   \\
SP\_Mod    & $G_\beta$ & 7 & 1     & 0.7   & 0.3  & -0.086        & 0.15 & 0.106              & -0.865        & -0.817  & -0.1   & 0.485    & 0.962                   & -3.422 & -0.575 & 0.009   \\
SP\_Med  & $G_\beta$ & 7 & 1     & 0.7   & 0.3  & -0.107        & 0.15 & 0.11               & -0.921        & -0.97   & -0.116 & 0.487    & 0.93                    & -4.235 & -0.712 & 0.001   \\
KM\_Mod   & $G_\beta$ & 7 & 3     & 0.7   & 0.3  & -0.022        & 0.15 & 0.106              & -0.665        & -0.213  & -0.034 & 0.496    & 0.99                    & -0.892 & -0.15  & 0.499   \\
KM\_Med & $G_\beta$ & 7 & 3     & 0.7   & 0.3  & -0.016        & 0.15 & 0.107              & -0.629        & -0.145  & -0.025 & 0.505    & 0.963                   & -0.616 & -0.104 & 0.64    \\
SP\_Mod    & $G_\beta$ & 7 & 3     & 0.7   & 0.3  & -0.001        & 0.15 & 0.103              & -0.598        & -0.005  & -0.001 & 0.498    & 1.009                   & -0.022 & -0.004 & 0.987   \\
SP\_Med  & $G_\beta$ & 7 & 3     & 0.7   & 0.3  & -0.017        & 0.15 & 0.108              & -0.655        & -0.154  & -0.025 & 0.501    & 0.978                   & -0.656 & -0.11  & 0.619   \\
KM\_Mod   & $G_\beta$ & 7 & 5     & 0.7   & 0.3  & -0.002        & 0.15 & 0.104              & -0.639        & -0.021  & -0.003 & 0.499    & 1.003                   & -0.086 & -0.014 & 0.948   \\
KM\_Med & $G_\beta$ & 7 & 5     & 0.7   & 0.3  & 0.003         & 0.15 & 0.107              & -0.579        & 0.031   & 0.006  & 0.499    & 1.009                   & 0.134  & 0.022  & 0.919   \\
SP\_Mod    & $G_\beta$ & 7 & 5     & 0.7   & 0.3  & -0.026        & 0.15 & 0.104              & -0.699        & -0.25   & -0.037 & 0.501    & 0.966                   & -1.036 & -0.174 & 0.432   \\
SP\_Med  & $G_\beta$ & 7 & 5     & 0.7   & 0.3  & 0.003         & 0.15 & 0.104              & -0.513        & 0.028   & 0.006  & 0.495    & 1.026                   & 0.117  & 0.02   & 0.929   \\
KM\_Mod   & $G_\beta$ & 7 & 7     & 0.7   & 0.3  & 0.006         & 0.15 & 0.103              & -0.484        & 0.06    & 0.013  & 0.503    & 0.996                   & 0.246  & 0.041  & 0.852   \\
KM\_Med & $G_\beta$ & 7 & 7     & 0.7   & 0.3  & 0.004         & 0.15 & 0.103              & -0.551        & 0.042   & 0.008  & 0.496    & 1.023                   & 0.172  & 0.029  & 0.896   \\
SP\_Mod    & $G_\beta$ & 7 & 7     & 0.7   & 0.3  & -0.011        & 0.15 & 0.103              & -0.528        & -0.106  & -0.021 & 0.496    & 1.004                   & -0.435 & -0.073 & 0.742   \\
SP\_Med  & $G_\beta$ & 7 & 7     & 0.7   & 0.3  & 0.007         & 0.15 & 0.105              & -0.467        & 0.071   & 0.016  & 0.503    & 0.999                   & 0.295  & 0.05   & 0.823   \\
CCF              & $G_\beta$ & 1 & 1     & 0.85  & 0.15 & -0.164        & 0.15 & 0.111              & -0.977        & -1.482  & -0.168 & 0.469    & 0.935                   & -6.507 & -1.093 & 0.0     \\
CCF              & $G_\beta$ & 1 & 3     & 0.85  & 0.15 & -0.0          & 0.15 & 0.103              & -0.51         & -0.004  & -0.001 & 0.501    & 0.997                   & -0.016 & -0.003 & 0.991   \\
CCF              & $G_\beta$ & 1 & 5     & 0.85  & 0.15 & -0.028        & 0.15 & 0.108              & -0.69         & -0.262  & -0.041 & 0.502    & 0.96                    & -1.128 & -0.189 & 0.391   \\
CCF              & $G_\beta$ & 1 & 7     & 0.85  & 0.15 & -0.005        & 0.15 & 0.106              & -0.559        & -0.051  & -0.01  & 0.504    & 0.978                   & -0.217 & -0.036 & 0.869   \\
CCF              & $G_\beta$ & 3 & 1     & 0.85  & 0.15 & -0.163        & 0.15 & 0.11               & -0.971        & -1.48   & -0.168 & 0.471    & 0.926                   & -6.468 & -1.087 & 0.0     \\
CCF              & $G_\beta$ & 3 & 3     & 0.85  & 0.15 & 0.033         & 0.15 & 0.103              & -0.415        & 0.317   & 0.078  & 0.504    & 1.021                   & 1.291  & 0.217  & 0.327   \\
CCF              & $G_\beta$ & 3 & 5     & 0.85  & 0.15 & -0.02         & 0.15 & 0.108              & -0.595        & -0.184  & -0.033 & 0.502    & 0.971                   & -0.789 & -0.133 & 0.549   \\
CCF              & $G_\beta$ & 3 & 7     & 0.85  & 0.15 & -0.064        & 0.15 & 0.107              & -0.812        & -0.598  & -0.079 & 0.491    & 0.963                   & -2.536 & -0.426 & 0.054   \\
CCF              & $G_\beta$ & 5 & 1     & 0.85  & 0.15 & -0.108        & 0.15 & 0.109              & -0.933        & -0.989  & -0.116 & 0.478    & 0.96                    & -4.281 & -0.719 & 0.001   \\
CCF              & $G_\beta$ & 5 & 3     & 0.85  & 0.15 & 0.048         & 0.15 & 0.103              & -0.292        & 0.471   & 0.166  & 0.508    & 1.024                   & 1.922  & 0.323  & 0.144   \\
CCF              & $G_\beta$ & 5 & 5     & 0.85  & 0.15 & -0.062        & 0.15 & 0.108              & -0.791        & -0.576  & -0.079 & 0.491    & 0.962                   & -2.479 & -0.417 & 0.059   \\
CCF              & $G_\beta$ & 5 & 7     & 0.85  & 0.15 & -0.024        & 0.15 & 0.107              & -0.69         & -0.222  & -0.034 & 0.502    & 0.964                   & -0.942 & -0.158 & 0.475   \\
CCF              & $G_\beta$ & 7 & 1     & 0.85  & 0.15 & -0.135        & 0.15 & 0.109              & -0.963        & -1.241  & -0.14  & 0.477    & 0.936                   & -5.368 & -0.902 & 0.0     \\
CCF              & $G_\beta$ & 7 & 3     & 0.85  & 0.15 & -0.01         & 0.15 & 0.105              & -0.545        & -0.092  & -0.018 & 0.497    & 0.999                   & -0.383 & -0.064 & 0.772   \\
CCF              & $G_\beta$ & 7 & 5     & 0.85  & 0.15 & -0.013        & 0.15 & 0.106              & -0.602        & -0.121  & -0.021 & 0.504    & 0.97                    & -0.508 & -0.085 & 0.7     \\
CCF              & $G_\beta$ & 7 & 7     & 0.85  & 0.15 & -0.025        & 0.15 & 0.107              & -0.667        & -0.236  & -0.038 & 0.5      & 0.971                   & -1.001 & -0.168 & 0.447   \\
CCF              & $G_\beta$ & 1 & 1     & 0.8   & 0.2  & -0.155        & 0.15 & 0.111              & -0.973        & -1.392  & -0.159 & 0.474    & 0.924                   & -6.157 & -1.034 & 0.0     \\
CCF              & $G_\beta$ & 1 & 3     & 0.8   & 0.2  & -0.002        & 0.15 & 0.103              & -0.555        & -0.02   & -0.004 & 0.498    & 1.005                   & -0.082 & -0.014 & 0.95    \\
CCF              & $G_\beta$ & 1 & 5     & 0.8   & 0.2  & -0.034        & 0.15 & 0.11               & -0.695        & -0.312  & -0.049 & 0.508    & 0.932                   & -1.365 & -0.229 & 0.299   \\
CCF              & $G_\beta$ & 1 & 7     & 0.8   & 0.2  & 0.001         & 0.15 & 0.106              & -0.497        & 0.006   & 0.001  & 0.506    & 0.976                   & 0.026  & 0.004  & 0.984   \\
CCF              & $G_\beta$ & 3 & 1     & 0.8   & 0.2  & -0.155        & 0.15 & 0.112              & -0.966        & -1.386  & -0.16  & 0.477    & 0.913                   & -6.149 & -1.033 & 0.0     \\
CCF              & $G_\beta$ & 3 & 3     & 0.8   & 0.2  & 0.025         & 0.15 & 0.104              & -0.423        & 0.238   & 0.059  & 0.503    & 1.017                   & 0.984  & 0.165  & 0.455   \\
CCF              & $G_\beta$ & 3 & 5     & 0.8   & 0.2  & -0.013        & 0.15 & 0.108              & -0.601        & -0.124  & -0.022 & 0.503    & 0.975                   & -0.533 & -0.09  & 0.686   \\
CCF              & $G_\beta$ & 3 & 7     & 0.8   & 0.2  & -0.044        & 0.15 & 0.105              & -0.775        & -0.417  & -0.056 & 0.495    & 0.97                    & -1.734 & -0.291 & 0.188   \\
CCF              & $G_\beta$ & 5 & 1     & 0.8   & 0.2  & -0.115        & 0.15 & 0.11               & -0.938        & -1.043  & -0.123 & 0.481    & 0.943                   & -4.566 & -0.767 & 0.0     \\
CCF              & $G_\beta$ & 5 & 3     & 0.8   & 0.2  & 0.03          & 0.15 & 0.104              & -0.366        & 0.29    & 0.082  & 0.507    & 1.007                   & 1.195  & 0.201  & 0.365   \\
CCF              & $G_\beta$ & 5 & 5     & 0.8   & 0.2  & -0.037        & 0.15 & 0.104              & -0.744        & -0.35   & -0.049 & 0.501    & 0.954                   & -1.452 & -0.244 & 0.271   \\
CCF              & $G_\beta$ & 5 & 7     & 0.8   & 0.2  & 0.017         & 0.15 & 0.103              & -0.536        & 0.166   & 0.032  & 0.507    & 0.991                   & 0.683  & 0.115  & 0.604   \\
CCF              & $G_\beta$ & 7 & 1     & 0.8   & 0.2  & -0.123        & 0.15 & 0.11               & -0.957        & -1.112  & -0.128 & 0.483    & 0.924                   & -4.872 & -0.819 & 0.0     \\
CCF              & $G_\beta$ & 7 & 3     & 0.8   & 0.2  & -0.008        & 0.15 & 0.105              & -0.569        & -0.08   & -0.015 & 0.496    & 1.007                   & -0.333 & -0.056 & 0.801   \\
CCF              & $G_\beta$ & 7 & 5     & 0.8   & 0.2  & -0.006        & 0.15 & 0.108              & -0.611        & -0.054  & -0.01  & 0.51     & 0.955                   & -0.233 & -0.039 & 0.86    \\
CCF              & $G_\beta$ & 7 & 7     & 0.8   & 0.2  & 0.006         & 0.15 & 0.105              & -0.545        & 0.06    & 0.012  & 0.504    & 0.993                   & 0.249  & 0.042  & 0.85    \\
CCF              & $G_\beta$ & 1 & 1     & 0.75  & 0.25 & -0.148        & 0.15 & 0.111              & -0.969        & -1.327  & -0.152 & 0.472    & 0.938                   & -5.854 & -0.983 & 0.0     \\
CCF              & $G_\beta$ & 1 & 3     & 0.75  & 0.25 & 0.013         & 0.15 & 0.104              & -0.446        & 0.13    & 0.03   & 0.502    & 1.01                    & 0.535  & 0.09   & 0.685   \\
CCF              & $G_\beta$ & 1 & 5     & 0.75  & 0.25 & -0.035        & 0.15 & 0.11               & -0.71         & -0.32   & -0.05  & 0.503    & 0.948                   & -1.403 & -0.236 & 0.286   \\
CCF              & $G_\beta$ & 1 & 7     & 0.75  & 0.25 & 0.017         & 0.15 & 0.105              & -0.393        & 0.165   & 0.044  & 0.501    & 1.016                   & 0.685  & 0.115  & 0.603   \\
CCF              & $G_\beta$ & 3 & 1     & 0.75  & 0.25 & -0.144        & 0.15 & 0.112              & -0.958        & -1.293  & -0.151 & 0.475    & 0.933                   & -5.733 & -0.963 & 0.0     \\
CCF              & $G_\beta$ & 3 & 3     & 0.75  & 0.25 & 0.033         & 0.15 & 0.106              & -0.407        & 0.316   & 0.082  & 0.509    & 1.005                   & 1.329  & 0.223  & 0.314   \\
CCF              & $G_\beta$ & 3 & 5     & 0.75  & 0.25 & -0.017        & 0.15 & 0.109              & -0.603        & -0.161  & -0.029 & 0.502    & 0.971                   & -0.692 & -0.116 & 0.599   \\
CCF              & $G_\beta$ & 3 & 7     & 0.75  & 0.25 & -0.032        & 0.15 & 0.104              & -0.727        & -0.311  & -0.045 & 0.492    & 0.995                   & -1.289 & -0.217 & 0.329   \\
CCF              & $G_\beta$ & 5 & 1     & 0.75  & 0.25 & -0.115        & 0.15 & 0.111              & -0.943        & -1.043  & -0.122 & 0.48     & 0.944                   & -4.577 & -0.769 & 0.0     \\
CCF              & $G_\beta$ & 5 & 3     & 0.75  & 0.25 & 0.026         & 0.15 & 0.105              & -0.393        & 0.243   & 0.065  & 0.505    & 1.011                   & 1.013  & 0.17   & 0.442   \\
CCF              & $G_\beta$ & 5 & 5     & 0.75  & 0.25 & -0.05         & 0.15 & 0.104              & -0.814        & -0.476  & -0.061 & 0.497    & 0.954                   & -1.97  & -0.331 & 0.136   \\
CCF              & $G_\beta$ & 5 & 7     & 0.75  & 0.25 & 0.009         & 0.15 & 0.104              & -0.591        & 0.084   & 0.015  & 0.501    & 1.005                   & 0.349  & 0.059  & 0.791   \\
CCF              & $G_\beta$ & 7 & 1     & 0.75  & 0.25 & -0.125        & 0.15 & 0.11               & -0.961        & -1.131  & -0.13  & 0.476    & 0.949                   & -4.948 & -0.831 & 0.0     \\
CCF              & $G_\beta$ & 7 & 3     & 0.75  & 0.25 & -0.005        & 0.15 & 0.106              & -0.471        & -0.046  & -0.01  & 0.499    & 0.997                   & -0.193 & -0.032 & 0.883   \\
CCF              & $G_\beta$ & 7 & 5     & 0.75  & 0.25 & 0.005         & 0.15 & 0.108              & -0.541        & 0.046   & 0.009  & 0.512    & 0.959                   & 0.199  & 0.033  & 0.88    \\
CCF              & $G_\beta$ & 7 & 7     & 0.75  & 0.25 & 0.013         & 0.15 & 0.104              & -0.535        & 0.121   & 0.024  & 0.502    & 1.007                   & 0.499  & 0.084  & 0.705   \\
CCF              & $G_\beta$ & 1 & 1     & 0.7   & 0.3  & -0.149        & 0.15 & 0.111              & -0.968        & -1.341  & -0.154 & 0.471    & 0.94                    & -5.926 & -0.996 & 0.0     \\
CCF              & $G_\beta$ & 1 & 3     & 0.7   & 0.3  & 0.012         & 0.15 & 0.103              & -0.495        & 0.115   & 0.024  & 0.505    & 0.993                   & 0.471  & 0.079  & 0.721   \\
CCF              & $G_\beta$ & 1 & 5     & 0.7   & 0.3  & -0.03         & 0.15 & 0.111              & -0.673        & -0.273  & -0.045 & 0.507    & 0.938                   & -1.203 & -0.202 & 0.36    \\
CCF              & $G_\beta$ & 1 & 7     & 0.7   & 0.3  & 0.025         & 0.15 & 0.105              & -0.435        & 0.242   & 0.058  & 0.503    & 1.019                   & 1.008  & 0.169  & 0.445   \\
CCF              & $G_\beta$ & 3 & 1     & 0.7   & 0.3  & -0.14         & 0.15 & 0.112              & -0.955        & -1.252  & -0.147 & 0.475    & 0.936                   & -5.571 & -0.936 & 0.0     \\
CCF              & $G_\beta$ & 3 & 3     & 0.7   & 0.3  & 0.025         & 0.15 & 0.106              & -0.405        & 0.237   & 0.062  & 0.512    & 0.983                   & 0.999  & 0.168  & 0.449   \\
CCF              & $G_\beta$ & 3 & 5     & 0.7   & 0.3  & -0.014        & 0.15 & 0.11               & -0.615        & -0.131  & -0.023 & 0.506    & 0.96                    & -0.57  & -0.096 & 0.665   \\
CCF              & $G_\beta$ & 3 & 7     & 0.7   & 0.3  & -0.042        & 0.15 & 0.104              & -0.783        & -0.402  & -0.054 & 0.492    & 0.981                   & -1.663 & -0.279 & 0.208   \\
CCF              & $G_\beta$ & 5 & 1     & 0.7   & 0.3  & -0.112        & 0.15 & 0.111              & -0.936        & -1.012  & -0.12  & 0.485    & 0.93                    & -4.463 & -0.75  & 0.001   \\
CCF              & $G_\beta$ & 5 & 3     & 0.7   & 0.3  & 0.014         & 0.15 & 0.106              & -0.511        & 0.135   & 0.028  & 0.508    & 0.983                   & 0.566  & 0.095  & 0.668   \\
CCF              & $G_\beta$ & 5 & 5     & 0.7   & 0.3  & -0.049        & 0.15 & 0.105              & -0.812        & -0.467  & -0.06  & 0.5      & 0.942                   & -1.948 & -0.327 & 0.14    \\
CCF              & $G_\beta$ & 5 & 7     & 0.7   & 0.3  & 0.026         & 0.15 & 0.103              & -0.57         & 0.252   & 0.046  & 0.505    & 1.012                   & 1.032  & 0.173  & 0.433   \\
CCF              & $G_\beta$ & 7 & 1     & 0.7   & 0.3  & -0.131        & 0.15 & 0.111              & -0.966        & -1.181  & -0.136 & 0.479    & 0.929                   & -5.211 & -0.875 & 0.0     \\
CCF              & $G_\beta$ & 7 & 3     & 0.7   & 0.3  & 0.002         & 0.15 & 0.106              & -0.409        & 0.015   & 0.004  & 0.504    & 0.984                   & 0.064  & 0.011  & 0.961   \\
CCF              & $G_\beta$ & 7 & 5     & 0.7   & 0.3  & -0.0          & 0.15 & 0.109              & -0.582        & -0.003  & -0.001 & 0.51     & 0.96                    & -0.014 & -0.002 & 0.992   \\
CCF              & $G_\beta$ & 7 & 7     & 0.7   & 0.3  & 0.011         & 0.15 & 0.104              & -0.594        & 0.102   & 0.018  & 0.501    & 1.008                   & 0.421  & 0.071  & 0.749  \\
\hline
KM\_Mod   & $D_\alpha$ & 1 & 1     & 0.85  & 0.15 & -0.152        & 0.15 & 0.117              & -0.972        & -1.301  & -0.157 & 0.476    & 0.909                   & -6.05  & -1.016 & 0.0     \\
KM\_Med & $D_\alpha$ & 1 & 1     & 0.85  & 0.15 & -0.136        & 0.15 & 0.117              & -0.961        & -1.162  & -0.142 & 0.48     & 0.915                   & -5.399 & -0.907 & 0.0     \\
SP\_Mod    & $D_\alpha$ & 1 & 1     & 0.85  & 0.15 & -0.161        & 0.15 & 0.117              & -0.975        & -1.371  & -0.165 & 0.473    & 0.911                   & -6.375 & -1.071 & 0.0     \\
SP\_Med  & $D_\alpha$ & 1 & 1     & 0.85  & 0.15 & -0.152        & 0.15 & 0.117              & -0.974        & -1.305  & -0.156 & 0.479    & 0.899                   & -6.038 & -1.014 & 0.0     \\
KM\_Mod   & $D_\alpha$ & 1 & 3     & 0.85  & 0.15 & -0.003        & 0.15 & 0.112              & -0.556        & -0.023  & -0.005 & 0.504    & 0.982                   & -0.101 & -0.017 & 0.939   \\
KM\_Med & $D_\alpha$ & 1 & 3     & 0.85  & 0.15 & 0.004         & 0.15 & 0.111              & -0.59         & 0.033   & 0.006  & 0.5      & 1.003                   & 0.145  & 0.024  & 0.913   \\
SP\_Mod    & $D_\alpha$ & 1 & 3     & 0.85  & 0.15 & -0.002        & 0.15 & 0.111              & -0.531        & -0.015  & -0.003 & 0.509    & 0.964                   & -0.068 & -0.011 & 0.959   \\
SP\_Med  & $D_\alpha$ & 1 & 3     & 0.85  & 0.15 & 0.008         & 0.15 & 0.111              & -0.586        & 0.075   & 0.014  & 0.506    & 0.987                   & 0.328  & 0.055  & 0.803   \\
KM\_Mod   & $D_\alpha$ & 1 & 5     & 0.85  & 0.15 & -0.065        & 0.15 & 0.117              & -0.859        & -0.555  & -0.076 & 0.491    & 0.957                   & -2.577 & -0.433 & 0.049   \\
KM\_Med & $D_\alpha$ & 1 & 5     & 0.85  & 0.15 & -0.051        & 0.15 & 0.117              & -0.807        & -0.431  & -0.063 & 0.495    & 0.957                   & -2.008 & -0.337 & 0.126   \\
SP\_Mod    & $D_\alpha$ & 1 & 5     & 0.85  & 0.15 & -0.045        & 0.15 & 0.118              & -0.795        & -0.38   & -0.056 & 0.501    & 0.941                   & -1.782 & -0.299 & 0.174   \\
SP\_Med  & $D_\alpha$ & 1 & 5     & 0.85  & 0.15 & -0.035        & 0.15 & 0.118              & -0.765        & -0.294  & -0.045 & 0.5      & 0.959                   & -1.37  & -0.23  & 0.297   \\
KM\_Mod   & $D_\alpha$ & 1 & 7     & 0.85  & 0.15 & 0.019         & 0.15 & 0.112              & -0.732        & 0.171   & 0.026  & 0.507    & 0.996                   & 0.758  & 0.127  & 0.566   \\
KM\_Med & $D_\alpha$ & 1 & 7     & 0.85  & 0.15 & 0.024         & 0.15 & 0.111              & -0.66         & 0.213   & 0.036  & 0.505    & 1.008                   & 0.937  & 0.157  & 0.477   \\
SP\_Mod    & $D_\alpha$ & 1 & 7     & 0.85  & 0.15 & 0.038         & 0.15 & 0.111              & -0.658        & 0.34    & 0.057  & 0.511    & 1.003                   & 1.495  & 0.251  & 0.257   \\
SP\_Med  & $D_\alpha$ & 1 & 7     & 0.85  & 0.15 & 0.027         & 0.15 & 0.111              & -0.658        & 0.242   & 0.041  & 0.51     & 0.993                   & 1.07   & 0.18   & 0.417   \\
KM\_Mod   & $D_\alpha$ & 3 & 1     & 0.85  & 0.15 & -0.127        & 0.15 & 0.119              & -0.945        & -1.073  & -0.135 & 0.48     & 0.923                   & -5.051 & -0.849 & 0.0     \\
KM\_Med & $D_\alpha$ & 3 & 1     & 0.85  & 0.15 & -0.136        & 0.15 & 0.119              & -0.953        & -1.143  & -0.143 & 0.478    & 0.92                    & -5.391 & -0.906 & 0.0     \\
SP\_Mod    & $D_\alpha$ & 3 & 1     & 0.85  & 0.15 & -0.148        & 0.15 & 0.119              & -0.963        & -1.243  & -0.154 & 0.475    & 0.919                   & -5.882 & -0.988 & 0.0     \\
SP\_Med  & $D_\alpha$ & 3 & 1     & 0.85  & 0.15 & -0.141        & 0.15 & 0.119              & -0.957        & -1.191  & -0.148 & 0.479    & 0.911                   & -5.604 & -0.941 & 0.0     \\
KM\_Mod   & $D_\alpha$ & 3 & 3     & 0.85  & 0.15 & -0.008        & 0.15 & 0.114              & -0.446        & -0.073  & -0.019 & 0.506    & 0.965                   & -0.331 & -0.056 & 0.801   \\
KM\_Med & $D_\alpha$ & 3 & 3     & 0.85  & 0.15 & -0.008        & 0.15 & 0.114              & -0.434        & -0.068  & -0.018 & 0.507    & 0.964                   & -0.307 & -0.052 & 0.816   \\
SP\_Mod    & $D_\alpha$ & 3 & 3     & 0.85  & 0.15 & -0.002        & 0.15 & 0.114              & -0.413        & -0.014  & -0.004 & 0.511    & 0.954                   & -0.065 & -0.011 & 0.961   \\
SP\_Med  & $D_\alpha$ & 3 & 3     & 0.85  & 0.15 & -0.004        & 0.15 & 0.113              & -0.432        & -0.032  & -0.008 & 0.51     & 0.957                   & -0.142 & -0.024 & 0.914   \\
KM\_Mod   & $D_\alpha$ & 3 & 5     & 0.85  & 0.15 & -0.033        & 0.15 & 0.114              & -0.684        & -0.285  & -0.048 & 0.493    & 0.987                   & -1.291 & -0.217 & 0.326   \\
KM\_Med & $D_\alpha$ & 3 & 5     & 0.85  & 0.15 & -0.04         & 0.15 & 0.115              & -0.729        & -0.353  & -0.055 & 0.494    & 0.976                   & -1.603 & -0.269 & 0.223   \\
SP\_Mod    & $D_\alpha$ & 3 & 5     & 0.85  & 0.15 & -0.026        & 0.15 & 0.115              & -0.718        & -0.224  & -0.036 & 0.499    & 0.972                   & -1.02  & -0.171 & 0.439   \\
SP\_Med  & $D_\alpha$ & 3 & 5     & 0.85  & 0.15 & -0.044        & 0.15 & 0.115              & -0.747        & -0.38   & -0.058 & 0.494    & 0.969                   & -1.731 & -0.291 & 0.188   \\
KM\_Mod   & $D_\alpha$ & 3 & 7     & 0.85  & 0.15 & -0.028        & 0.15 & 0.108              & -0.756        & -0.255  & -0.037 & 0.492    & 0.996                   & -1.096 & -0.184 & 0.407   \\
KM\_Med & $D_\alpha$ & 3 & 7     & 0.85  & 0.15 & -0.03         & 0.15 & 0.107              & -0.779        & -0.282  & -0.039 & 0.49     & 1.001                   & -1.202 & -0.202 & 0.363   \\
SP\_Mod    & $D_\alpha$ & 3 & 7     & 0.85  & 0.15 & -0.011        & 0.15 & 0.107              & -0.712        & -0.105  & -0.016 & 0.501    & 0.982                   & -0.445 & -0.075 & 0.736   \\
SP\_Med  & $D_\alpha$ & 3 & 7     & 0.85  & 0.15 & -0.023        & 0.15 & 0.106              & -0.75         & -0.214  & -0.03  & 0.492    & 1.005                   & -0.904 & -0.152 & 0.494   \\
KM\_Mod   & $D_\alpha$ & 5 & 1     & 0.85  & 0.15 & -0.11         & 0.15 & 0.118              & -0.922        & -0.933  & -0.12  & 0.483    & 0.932                   & -4.381 & -0.736 & 0.001   \\
KM\_Med & $D_\alpha$ & 5 & 1     & 0.85  & 0.15 & -0.107        & 0.15 & 0.118              & -0.916        & -0.906  & -0.117 & 0.481    & 0.943                   & -4.242 & -0.713 & 0.001   \\
SP\_Mod    & $D_\alpha$ & 5 & 1     & 0.85  & 0.15 & -0.113        & 0.15 & 0.119              & -0.925        & -0.95   & -0.122 & 0.483    & 0.929                   & -4.483 & -0.753 & 0.001   \\
SP\_Med  & $D_\alpha$ & 5 & 1     & 0.85  & 0.15 & -0.122        & 0.15 & 0.119              & -0.937        & -1.025  & -0.13  & 0.486    & 0.908                   & -4.825 & -0.811 & 0.0     \\
KM\_Mod   & $D_\alpha$ & 5 & 3     & 0.85  & 0.15 & 0.001         & 0.15 & 0.111              & -0.53         & 0.011   & 0.002  & 0.5      & 1.002                   & 0.048  & 0.008  & 0.971   \\
KM\_Med & $D_\alpha$ & 5 & 3     & 0.85  & 0.15 & 0.007         & 0.15 & 0.112              & -0.514        & 0.065   & 0.014  & 0.504    & 0.993                   & 0.291  & 0.049  & 0.826   \\
SP\_Mod    & $D_\alpha$ & 5 & 3     & 0.85  & 0.15 & 0.023         & 0.15 & 0.111              & -0.424        & 0.21    & 0.055  & 0.511    & 0.985                   & 0.923  & 0.155  & 0.484   \\
SP\_Med  & $D_\alpha$ & 5 & 3     & 0.85  & 0.15 & 0.028         & 0.15 & 0.111              & -0.401        & 0.25    & 0.069  & 0.513    & 0.982                   & 1.098  & 0.184  & 0.405   \\
KM\_Mod   & $D_\alpha$ & 5 & 5     & 0.85  & 0.15 & -0.029        & 0.15 & 0.113              & -0.761        & -0.253  & -0.038 & 0.495    & 0.985                   & -1.134 & -0.19  & 0.389   \\
KM\_Med & $D_\alpha$ & 5 & 5     & 0.85  & 0.15 & -0.038        & 0.15 & 0.112              & -0.802        & -0.34   & -0.048 & 0.496    & 0.968                   & -1.516 & -0.255 & 0.25    \\
SP\_Mod    & $D_\alpha$ & 5 & 5     & 0.85  & 0.15 & -0.055        & 0.15 & 0.114              & -0.845        & -0.482  & -0.065 & 0.494    & 0.957                   & -2.178 & -0.366 & 0.098   \\
SP\_Med  & $D_\alpha$ & 5 & 5     & 0.85  & 0.15 & -0.05         & 0.15 & 0.113              & -0.832        & -0.446  & -0.061 & 0.495    & 0.957                   & -2.0   & -0.336 & 0.129   \\
KM\_Mod   & $D_\alpha$ & 5 & 7     & 0.85  & 0.15 & 0.041         & 0.15 & 0.107              & -0.482        & 0.387   & 0.086  & 0.502    & 1.043                   & 1.642  & 0.276  & 0.212   \\
KM\_Med & $D_\alpha$ & 5 & 7     & 0.85  & 0.15 & 0.051         & 0.15 & 0.107              & -0.42         & 0.474   & 0.12   & 0.506    & 1.038                   & 2.007  & 0.337  & 0.127   \\
SP\_Mod    & $D_\alpha$ & 5 & 7     & 0.85  & 0.15 & 0.06          & 0.15 & 0.104              & -0.412        & 0.575   & 0.145  & 0.509    & 1.041                   & 2.371  & 0.398  & 0.07    \\
SP\_Med  & $D_\alpha$ & 5 & 7     & 0.85  & 0.15 & 0.031         & 0.15 & 0.107              & -0.532        & 0.29    & 0.058  & 0.503    & 1.026                   & 1.226  & 0.206  & 0.351   \\
KM\_Mod   & $D_\alpha$ & 7 & 1     & 0.85  & 0.15 & -0.107        & 0.15 & 0.117              & -0.937        & -0.915  & -0.114 & 0.481    & 0.943                   & -4.248 & -0.714 & 0.001   \\
KM\_Med & $D_\alpha$ & 7 & 1     & 0.85  & 0.15 & -0.107        & 0.15 & 0.117              & -0.934        & -0.917  & -0.115 & 0.481    & 0.944                   & -4.251 & -0.714 & 0.001   \\
SP\_Mod    & $D_\alpha$ & 7 & 1     & 0.85  & 0.15 & -0.103        & 0.15 & 0.117              & -0.932        & -0.881  & -0.111 & 0.483    & 0.939                   & -4.101 & -0.689 & 0.002   \\
SP\_Med  & $D_\alpha$ & 7 & 1     & 0.85  & 0.15 & -0.107        & 0.15 & 0.116              & -0.925        & -0.922  & -0.115 & 0.482    & 0.941                   & -4.237 & -0.712 & 0.001   \\
KM\_Mod   & $D_\alpha$ & 7 & 3     & 0.85  & 0.15 & -0.037        & 0.15 & 0.114              & -0.716        & -0.323  & -0.051 & 0.497    & 0.966                   & -1.46  & -0.245 & 0.267   \\
KM\_Med & $D_\alpha$ & 7 & 3     & 0.85  & 0.15 & -0.022        & 0.15 & 0.113              & -0.653        & -0.196  & -0.034 & 0.503    & 0.961                   & -0.882 & -0.148 & 0.503   \\
SP\_Mod    & $D_\alpha$ & 7 & 3     & 0.85  & 0.15 & -0.018        & 0.15 & 0.113              & -0.659        & -0.157  & -0.027 & 0.503    & 0.966                   & -0.702 & -0.118 & 0.594   \\
SP\_Med  & $D_\alpha$ & 7 & 3     & 0.85  & 0.15 & -0.028        & 0.15 & 0.113              & -0.677        & -0.247  & -0.041 & 0.504    & 0.952                   & -1.111 & -0.187 & 0.399   \\
KM\_Mod   & $D_\alpha$ & 7 & 5     & 0.85  & 0.15 & 0.023         & 0.15 & 0.111              & -0.522        & 0.211   & 0.045  & 0.503    & 1.017                   & 0.929  & 0.156  & 0.481   \\
KM\_Med & $D_\alpha$ & 7 & 5     & 0.85  & 0.15 & 0.015         & 0.15 & 0.111              & -0.531        & 0.137   & 0.029  & 0.503    & 1.008                   & 0.605  & 0.102  & 0.646   \\
SP\_Mod    & $D_\alpha$ & 7 & 5     & 0.85  & 0.15 & 0.015         & 0.15 & 0.113              & -0.59         & 0.132   & 0.025  & 0.506    & 0.996                   & 0.589  & 0.099  & 0.655   \\
SP\_Med  & $D_\alpha$ & 7 & 5     & 0.85  & 0.15 & 0.028         & 0.15 & 0.112              & -0.522        & 0.253   & 0.054  & 0.506    & 1.01                    & 1.123  & 0.189  & 0.395   \\
KM\_Mod   & $D_\alpha$ & 7 & 7     & 0.85  & 0.15 & 0.025         & 0.15 & 0.108              & -0.452        & 0.234   & 0.056  & 0.496    & 1.05                    & 1.004  & 0.169  & 0.446   \\
KM\_Med & $D_\alpha$ & 7 & 7     & 0.85  & 0.15 & 0.03          & 0.15 & 0.108              & -0.459        & 0.28    & 0.066  & 0.498    & 1.046                   & 1.202  & 0.202  & 0.362   \\
SP\_Mod    & $D_\alpha$ & 7 & 7     & 0.85  & 0.15 & 0.031         & 0.15 & 0.108              & -0.502        & 0.283   & 0.061  & 0.503    & 1.027                   & 1.213  & 0.204  & 0.357   \\
SP\_Med  & $D_\alpha$ & 7 & 7     & 0.85  & 0.15 & 0.036         & 0.15 & 0.107              & -0.44         & 0.333   & 0.081  & 0.501    & 1.04                    & 1.417  & 0.238  & 0.282   \\
KM\_Mod   & $D_\alpha$ & 1 & 1     & 0.8   & 0.2  & -0.138        & 0.15 & 0.117              & -0.962        & -1.179  & -0.143 & 0.477    & 0.921                   & -5.468 & -0.919 & 0.0     \\
KM\_Med & $D_\alpha$ & 1 & 1     & 0.8   & 0.2  & -0.127        & 0.15 & 0.117              & -0.953        & -1.087  & -0.134 & 0.48     & 0.925                   & -5.059 & -0.85  & 0.0     \\
SP\_Mod    & $D_\alpha$ & 1 & 1     & 0.8   & 0.2  & -0.152        & 0.15 & 0.117              & -0.971        & -1.29   & -0.156 & 0.477    & 0.905                   & -6.016 & -1.011 & 0.0     \\
SP\_Med  & $D_\alpha$ & 1 & 1     & 0.8   & 0.2  & -0.152        & 0.15 & 0.116              & -0.971        & -1.31   & -0.156 & 0.477    & 0.908                   & -6.03  & -1.013 & 0.0     \\
KM\_Mod   & $D_\alpha$ & 1 & 3     & 0.8   & 0.2  & 0.004         & 0.15 & 0.11               & -0.556        & 0.036   & 0.007  & 0.497    & 1.018                   & 0.159  & 0.027  & 0.904   \\
KM\_Med & $D_\alpha$ & 1 & 3     & 0.8   & 0.2  & 0.007         & 0.15 & 0.11               & -0.565        & 0.065   & 0.013  & 0.497    & 1.022                   & 0.281  & 0.047  & 0.831   \\
SP\_Mod    & $D_\alpha$ & 1 & 3     & 0.8   & 0.2  & -0.004        & 0.15 & 0.112              & -0.577        & -0.032  & -0.006 & 0.505    & 0.976                   & -0.141 & -0.024 & 0.915   \\
SP\_Med  & $D_\alpha$ & 1 & 3     & 0.8   & 0.2  & 0.0           & 0.15 & 0.11               & -0.582        & 0.002   & 0.0    & 0.5      & 1.0                     & 0.01   & 0.002  & 0.994   \\
KM\_Mod   & $D_\alpha$ & 1 & 5     & 0.8   & 0.2  & -0.054        & 0.15 & 0.117              & -0.837        & -0.463  & -0.065 & 0.491    & 0.967                   & -2.16  & -0.363 & 0.1     \\
KM\_Med & $D_\alpha$ & 1 & 5     & 0.8   & 0.2  & -0.057        & 0.15 & 0.117              & -0.835        & -0.489  & -0.069 & 0.494    & 0.954                   & -2.274 & -0.382 & 0.083   \\
SP\_Mod    & $D_\alpha$ & 1 & 5     & 0.8   & 0.2  & -0.04         & 0.15 & 0.118              & -0.759        & -0.342  & -0.053 & 0.502    & 0.945                   & -1.605 & -0.27  & 0.222   \\
SP\_Med  & $D_\alpha$ & 1 & 5     & 0.8   & 0.2  & -0.048        & 0.15 & 0.118              & -0.816        & -0.405  & -0.058 & 0.5      & 0.942                   & -1.891 & -0.318 & 0.149   \\
KM\_Mod   & $D_\alpha$ & 1 & 7     & 0.8   & 0.2  & 0.019         & 0.15 & 0.112              & -0.713        & 0.167   & 0.026  & 0.509    & 0.989                   & 0.744  & 0.125  & 0.573   \\
KM\_Med & $D_\alpha$ & 1 & 7     & 0.8   & 0.2  & 0.027         & 0.15 & 0.111              & -0.598        & 0.241   & 0.045  & 0.508    & 1.003                   & 1.065  & 0.179  & 0.419   \\
SP\_Mod    & $D_\alpha$ & 1 & 7     & 0.8   & 0.2  & 0.033         & 0.15 & 0.11               & -0.636        & 0.298   & 0.052  & 0.504    & 1.025                   & 1.301  & 0.219  & 0.324   \\
SP\_Med  & $D_\alpha$ & 1 & 7     & 0.8   & 0.2  & 0.04          & 0.15 & 0.111              & -0.564        & 0.359   & 0.07   & 0.512    & 1.003                   & 1.573  & 0.264  & 0.233   \\
KM\_Mod   & $D_\alpha$ & 3 & 1     & 0.8   & 0.2  & -0.141        & 0.15 & 0.119              & -0.957        & -1.187  & -0.147 & 0.475    & 0.928                   & -5.589 & -0.939 & 0.0     \\
KM\_Med & $D_\alpha$ & 3 & 1     & 0.8   & 0.2  & -0.132        & 0.15 & 0.119              & -0.949        & -1.111  & -0.139 & 0.478    & 0.926                   & -5.228 & -0.878 & 0.0     \\
SP\_Mod    & $D_\alpha$ & 3 & 1     & 0.8   & 0.2  & -0.155        & 0.15 & 0.12               & -0.968        & -1.29   & -0.16  & 0.474    & 0.915                   & -6.132 & -1.03  & 0.0     \\
SP\_Med  & $D_\alpha$ & 3 & 1     & 0.8   & 0.2  & -0.134        & 0.15 & 0.118              & -0.952        & -1.137  & -0.141 & 0.478    & 0.922                   & -5.328 & -0.895 & 0.0     \\
KM\_Mod   & $D_\alpha$ & 3 & 3     & 0.8   & 0.2  & 0.002         & 0.15 & 0.114              & -0.398        & 0.016   & 0.005  & 0.503    & 0.991                   & 0.073  & 0.012  & 0.956   \\
KM\_Med & $D_\alpha$ & 3 & 3     & 0.8   & 0.2  & 0.008         & 0.15 & 0.113              & -0.394        & 0.067   & 0.019  & 0.508    & 0.976                   & 0.301  & 0.051  & 0.819   \\
SP\_Mod    & $D_\alpha$ & 3 & 3     & 0.8   & 0.2  & -0.004        & 0.15 & 0.114              & -0.44         & -0.033  & -0.008 & 0.507    & 0.968                   & -0.147 & -0.025 & 0.911   \\
SP\_Med  & $D_\alpha$ & 3 & 3     & 0.8   & 0.2  & -0.01         & 0.15 & 0.113              & -0.425        & -0.09   & -0.024 & 0.508    & 0.957                   & -0.405 & -0.068 & 0.759   \\
KM\_Mod   & $D_\alpha$ & 3 & 5     & 0.8   & 0.2  & -0.028        & 0.15 & 0.116              & -0.679        & -0.245  & -0.042 & 0.498    & 0.974                   & -1.129 & -0.19  & 0.391   \\
KM\_Med & $D_\alpha$ & 3 & 5     & 0.8   & 0.2  & -0.042        & 0.15 & 0.115              & -0.761        & -0.368  & -0.056 & 0.493    & 0.975                   & -1.684 & -0.283 & 0.2     \\
SP\_Mod    & $D_\alpha$ & 3 & 5     & 0.8   & 0.2  & -0.013        & 0.15 & 0.115              & -0.645        & -0.116  & -0.021 & 0.501    & 0.978                   & -0.529 & -0.089 & 0.688   \\
SP\_Med  & $D_\alpha$ & 3 & 5     & 0.8   & 0.2  & -0.028        & 0.15 & 0.114              & -0.707        & -0.248  & -0.04  & 0.497    & 0.975                   & -1.122 & -0.189 & 0.394   \\
KM\_Mod   & $D_\alpha$ & 3 & 7     & 0.8   & 0.2  & -0.017        & 0.15 & 0.108              & -0.696        & -0.162  & -0.025 & 0.495    & 0.998                   & -0.692 & -0.116 & 0.6     \\
KM\_Med & $D_\alpha$ & 3 & 7     & 0.8   & 0.2  & -0.026        & 0.15 & 0.107              & -0.757        & -0.244  & -0.034 & 0.487    & 1.02                    & -1.035 & -0.174 & 0.433   \\
SP\_Mod    & $D_\alpha$ & 3 & 7     & 0.8   & 0.2  & -0.02         & 0.15 & 0.107              & -0.746        & -0.188  & -0.027 & 0.496    & 0.992                   & -0.797 & -0.134 & 0.546   \\
SP\_Med  & $D_\alpha$ & 3 & 7     & 0.8   & 0.2  & -0.029        & 0.15 & 0.106              & -0.795        & -0.277  & -0.037 & 0.49     & 1.004                   & -1.165 & -0.196 & 0.378   \\
KM\_Mod   & $D_\alpha$ & 5 & 1     & 0.8   & 0.2  & -0.106        & 0.15 & 0.118              & -0.916        & -0.893  & -0.115 & 0.482    & 0.942                   & -4.196 & -0.705 & 0.001   \\
KM\_Med & $D_\alpha$ & 5 & 1     & 0.8   & 0.2  & -0.095        & 0.15 & 0.118              & -0.897        & -0.805  & -0.106 & 0.488    & 0.931                   & -3.771 & -0.633 & 0.004   \\
SP\_Mod    & $D_\alpha$ & 5 & 1     & 0.8   & 0.2  & -0.11         & 0.15 & 0.119              & -0.92         & -0.921  & -0.119 & 0.483    & 0.93                    & -4.355 & -0.732 & 0.001   \\
SP\_Med  & $D_\alpha$ & 5 & 1     & 0.8   & 0.2  & -0.115        & 0.15 & 0.118              & -0.927        & -0.975  & -0.124 & 0.483    & 0.928                   & -4.548 & -0.764 & 0.0     \\
KM\_Mod   & $D_\alpha$ & 5 & 3     & 0.8   & 0.2  & 0.008         & 0.15 & 0.111              & -0.46         & 0.076   & 0.018  & 0.504    & 0.995                   & 0.336  & 0.056  & 0.799   \\
KM\_Med & $D_\alpha$ & 5 & 3     & 0.8   & 0.2  & 0.012         & 0.15 & 0.111              & -0.506        & 0.11    & 0.024  & 0.502    & 1.008                   & 0.482  & 0.081  & 0.715   \\
SP\_Mod    & $D_\alpha$ & 5 & 3     & 0.8   & 0.2  & 0.023         & 0.15 & 0.111              & -0.366        & 0.207   & 0.063  & 0.511    & 0.986                   & 0.914  & 0.154  & 0.488   \\
SP\_Med  & $D_\alpha$ & 5 & 3     & 0.8   & 0.2  & 0.038         & 0.15 & 0.11               & -0.334        & 0.346   & 0.114  & 0.511    & 1.005                   & 1.512  & 0.254  & 0.252   \\
KM\_Mod   & $D_\alpha$ & 5 & 5     & 0.8   & 0.2  & -0.038        & 0.15 & 0.114              & -0.809        & -0.337  & -0.047 & 0.494    & 0.976                   & -1.518 & -0.255 & 0.249   \\
KM\_Med & $D_\alpha$ & 5 & 5     & 0.8   & 0.2  & -0.038        & 0.15 & 0.114              & -0.781        & -0.334  & -0.049 & 0.498    & 0.962                   & -1.515 & -0.255 & 0.25    \\
SP\_Mod    & $D_\alpha$ & 5 & 5     & 0.8   & 0.2  & -0.053        & 0.15 & 0.116              & -0.811        & -0.454  & -0.065 & 0.498    & 0.945                   & -2.086 & -0.35  & 0.112   \\
SP\_Med  & $D_\alpha$ & 5 & 5     & 0.8   & 0.2  & -0.047        & 0.15 & 0.115              & -0.797        & -0.406  & -0.059 & 0.502    & 0.935                   & -1.86  & -0.312 & 0.157   \\
KM\_Mod   & $D_\alpha$ & 5 & 7     & 0.8   & 0.2  & 0.049         & 0.15 & 0.107              & -0.457        & 0.453   & 0.106  & 0.505    & 1.041                   & 1.931  & 0.324  & 0.142   \\
KM\_Med & $D_\alpha$ & 5 & 7     & 0.8   & 0.2  & 0.041         & 0.15 & 0.107              & -0.518        & 0.389   & 0.08   & 0.503    & 1.043                   & 1.643  & 0.276  & 0.211   \\
SP\_Mod    & $D_\alpha$ & 5 & 7     & 0.8   & 0.2  & 0.05          & 0.15 & 0.108              & -0.524        & 0.462   & 0.095  & 0.509    & 1.026                   & 1.975  & 0.332  & 0.133   \\
SP\_Med  & $D_\alpha$ & 5 & 7     & 0.8   & 0.2  & 0.026         & 0.15 & 0.107              & -0.518        & 0.241   & 0.05   & 0.503    & 1.021                   & 1.023  & 0.172  & 0.437   \\
KM\_Mod   & $D_\alpha$ & 7 & 1     & 0.8   & 0.2  & -0.118        & 0.15 & 0.118              & -0.95         & -1.003  & -0.125 & 0.48     & 0.935                   & -4.699 & -0.789 & 0.0     \\
KM\_Med & $D_\alpha$ & 7 & 1     & 0.8   & 0.2  & -0.099        & 0.15 & 0.117              & -0.923        & -0.839  & -0.107 & 0.487    & 0.93                    & -3.911 & -0.657 & 0.003   \\
SP\_Mod    & $D_\alpha$ & 7 & 1     & 0.8   & 0.2  & -0.102        & 0.15 & 0.117              & -0.926        & -0.87   & -0.11  & 0.481    & 0.949                   & -4.055 & -0.681 & 0.002   \\
SP\_Med  & $D_\alpha$ & 7 & 1     & 0.8   & 0.2  & -0.107        & 0.15 & 0.116              & -0.926        & -0.921  & -0.115 & 0.482    & 0.939                   & -4.234 & -0.711 & 0.001   \\
KM\_Mod   & $D_\alpha$ & 7 & 3     & 0.8   & 0.2  & -0.032        & 0.15 & 0.114              & -0.704        & -0.277  & -0.045 & 0.496    & 0.976                   & -1.252 & -0.21  & 0.342   \\
KM\_Med & $D_\alpha$ & 7 & 3     & 0.8   & 0.2  & -0.03         & 0.15 & 0.113              & -0.718        & -0.271  & -0.042 & 0.501    & 0.957                   & -1.209 & -0.203 & 0.359   \\
SP\_Mod    & $D_\alpha$ & 7 & 3     & 0.8   & 0.2  & -0.024        & 0.15 & 0.113              & -0.704        & -0.209  & -0.034 & 0.503    & 0.96                    & -0.939 & -0.158 & 0.476   \\
SP\_Med  & $D_\alpha$ & 7 & 3     & 0.8   & 0.2  & -0.015        & 0.15 & 0.112              & -0.601        & -0.132  & -0.025 & 0.502    & 0.973                   & -0.59  & -0.099 & 0.655   \\
KM\_Mod   & $D_\alpha$ & 7 & 5     & 0.8   & 0.2  & 0.024         & 0.15 & 0.113              & -0.56         & 0.214   & 0.043  & 0.504    & 1.013                   & 0.955  & 0.16   & 0.469   \\
KM\_Med & $D_\alpha$ & 7 & 5     & 0.8   & 0.2  & 0.03          & 0.15 & 0.112              & -0.455        & 0.273   & 0.067  & 0.51     & 0.998                   & 1.21   & 0.203  & 0.359   \\
SP\_Mod    & $D_\alpha$ & 7 & 5     & 0.8   & 0.2  & 0.006         & 0.15 & 0.113              & -0.668        & 0.05    & 0.008  & 0.505    & 0.988                   & 0.222  & 0.037  & 0.866   \\
SP\_Med  & $D_\alpha$ & 7 & 5     & 0.8   & 0.2  & 0.024         & 0.15 & 0.112              & -0.537        & 0.216   & 0.045  & 0.511    & 0.988                   & 0.96   & 0.161  & 0.467   \\
KM\_Mod   & $D_\alpha$ & 7 & 7     & 0.8   & 0.2  & 0.038         & 0.15 & 0.108              & -0.35         & 0.352   & 0.109  & 0.502    & 1.039                   & 1.514  & 0.254  & 0.25    \\
KM\_Med & $D_\alpha$ & 7 & 7     & 0.8   & 0.2  & 0.037         & 0.15 & 0.108              & -0.434        & 0.343   & 0.085  & 0.5      & 1.047                   & 1.472  & 0.247  & 0.264   \\
SP\_Mod    & $D_\alpha$ & 7 & 7     & 0.8   & 0.2  & 0.029         & 0.15 & 0.108              & -0.467        & 0.271   & 0.062  & 0.5      & 1.037                   & 1.158  & 0.195  & 0.379   \\
SP\_Med  & $D_\alpha$ & 7 & 7     & 0.8   & 0.2  & 0.035         & 0.15 & 0.107              & -0.504        & 0.323   & 0.069  & 0.501    & 1.04                    & 1.371  & 0.23   & 0.298   \\
KM\_Mod   & $D_\alpha$ & 1 & 1     & 0.75  & 0.25 & -0.14         & 0.15 & 0.117              & -0.965        & -1.2    & -0.146 & 0.478    & 0.916                   & -5.574 & -0.936 & 0.0     \\
KM\_Med & $D_\alpha$ & 1 & 1     & 0.75  & 0.25 & -0.128        & 0.15 & 0.117              & -0.955        & -1.088  & -0.134 & 0.479    & 0.925                   & -5.068 & -0.851 & 0.0     \\
SP\_Mod    & $D_\alpha$ & 1 & 1     & 0.75  & 0.25 & -0.151        & 0.15 & 0.118              & -0.971        & -1.287  & -0.156 & 0.476    & 0.91                    & -6.005 & -1.009 & 0.0     \\
SP\_Med  & $D_\alpha$ & 1 & 1     & 0.75  & 0.25 & -0.142        & 0.15 & 0.115              & -0.964        & -1.23   & -0.147 & 0.478    & 0.916                   & -5.632 & -0.946 & 0.0     \\
KM\_Mod   & $D_\alpha$ & 1 & 3     & 0.75  & 0.25 & 0.009         & 0.15 & 0.11               & -0.525        & 0.082   & 0.017  & 0.497    & 1.024                   & 0.36   & 0.06   & 0.785   \\
KM\_Med & $D_\alpha$ & 1 & 3     & 0.75  & 0.25 & 0.009         & 0.15 & 0.111              & -0.568        & 0.078   & 0.015  & 0.498    & 1.02                    & 0.342  & 0.057  & 0.795   \\
SP\_Mod    & $D_\alpha$ & 1 & 3     & 0.75  & 0.25 & -0.005        & 0.15 & 0.113              & -0.602        & -0.042  & -0.008 & 0.508    & 0.964                   & -0.187 & -0.031 & 0.887   \\
SP\_Med  & $D_\alpha$ & 1 & 3     & 0.75  & 0.25 & 0.005         & 0.15 & 0.11               & -0.64         & 0.046   & 0.008  & 0.503    & 0.995                   & 0.203  & 0.034  & 0.878   \\
KM\_Mod   & $D_\alpha$ & 1 & 5     & 0.75  & 0.25 & -0.05         & 0.15 & 0.118              & -0.807        & -0.426  & -0.062 & 0.494    & 0.962                   & -1.992 & -0.335 & 0.129   \\
KM\_Med & $D_\alpha$ & 1 & 5     & 0.75  & 0.25 & -0.043        & 0.15 & 0.117              & -0.79         & -0.371  & -0.055 & 0.495    & 0.966                   & -1.719 & -0.289 & 0.191   \\
SP\_Mod    & $D_\alpha$ & 1 & 5     & 0.75  & 0.25 & -0.029        & 0.15 & 0.118              & -0.732        & -0.249  & -0.04  & 0.502    & 0.958                   & -1.165 & -0.196 & 0.376   \\
SP\_Med  & $D_\alpha$ & 1 & 5     & 0.75  & 0.25 & -0.053        & 0.15 & 0.117              & -0.815        & -0.453  & -0.065 & 0.5      & 0.937                   & -2.105 & -0.354 & 0.109   \\
KM\_Mod   & $D_\alpha$ & 1 & 7     & 0.75  & 0.25 & 0.025         & 0.15 & 0.113              & -0.606        & 0.224   & 0.042  & 0.512    & 0.982                   & 1.002  & 0.168  & 0.448   \\
KM\_Med & $D_\alpha$ & 1 & 7     & 0.75  & 0.25 & 0.025         & 0.15 & 0.112              & -0.571        & 0.222   & 0.043  & 0.511    & 0.987                   & 0.983  & 0.165  & 0.456   \\
SP\_Mod    & $D_\alpha$ & 1 & 7     & 0.75  & 0.25 & 0.024         & 0.15 & 0.111              & -0.692        & 0.212   & 0.034  & 0.503    & 1.019                   & 0.933  & 0.157  & 0.479   \\
SP\_Med  & $D_\alpha$ & 1 & 7     & 0.75  & 0.25 & 0.034         & 0.15 & 0.11               & -0.659        & 0.307   & 0.051  & 0.511    & 0.996                   & 1.334  & 0.224  & 0.311   \\
KM\_Mod   & $D_\alpha$ & 3 & 1     & 0.75  & 0.25 & -0.14         & 0.15 & 0.119              & -0.958        & -1.18   & -0.147 & 0.474    & 0.931                   & -5.571 & -0.936 & 0.0     \\
KM\_Med & $D_\alpha$ & 3 & 1     & 0.75  & 0.25 & -0.139        & 0.15 & 0.119              & -0.957        & -1.171  & -0.145 & 0.478    & 0.917                   & -5.517 & -0.927 & 0.0     \\
SP\_Mod    & $D_\alpha$ & 3 & 1     & 0.75  & 0.25 & -0.151        & 0.15 & 0.12               & -0.966        & -1.256  & -0.156 & 0.475    & 0.912                   & -5.988 & -1.006 & 0.0     \\
SP\_Med  & $D_\alpha$ & 3 & 1     & 0.75  & 0.25 & -0.136        & 0.15 & 0.118              & -0.953        & -1.149  & -0.143 & 0.48     & 0.915                   & -5.394 & -0.906 & 0.0     \\
KM\_Mod   & $D_\alpha$ & 3 & 3     & 0.75  & 0.25 & -0.018        & 0.15 & 0.115              & -0.474        & -0.157  & -0.038 & 0.505    & 0.957                   & -0.715 & -0.12  & 0.587   \\
KM\_Med & $D_\alpha$ & 3 & 3     & 0.75  & 0.25 & -0.002        & 0.15 & 0.114              & -0.388        & -0.017  & -0.005 & 0.507    & 0.971                   & -0.075 & -0.013 & 0.955   \\
SP\_Mod    & $D_\alpha$ & 3 & 3     & 0.75  & 0.25 & 0.007         & 0.15 & 0.114              & -0.413        & 0.063   & 0.017  & 0.508    & 0.979                   & 0.286  & 0.048  & 0.828   \\
SP\_Med  & $D_\alpha$ & 3 & 3     & 0.75  & 0.25 & -0.01         & 0.15 & 0.112              & -0.409        & -0.089  & -0.025 & 0.507    & 0.961                   & -0.398 & -0.067 & 0.763   \\
KM\_Mod   & $D_\alpha$ & 3 & 5     & 0.75  & 0.25 & -0.03         & 0.15 & 0.115              & -0.689        & -0.26   & -0.043 & 0.494    & 0.987                   & -1.185 & -0.199 & 0.368   \\
KM\_Med & $D_\alpha$ & 3 & 5     & 0.75  & 0.25 & -0.036        & 0.15 & 0.115              & -0.746        & -0.312  & -0.048 & 0.494    & 0.98                    & -1.425 & -0.239 & 0.278   \\
SP\_Mod    & $D_\alpha$ & 3 & 5     & 0.75  & 0.25 & -0.023        & 0.15 & 0.115              & -0.693        & -0.2    & -0.033 & 0.498    & 0.979                   & -0.915 & -0.154 & 0.487   \\
SP\_Med  & $D_\alpha$ & 3 & 5     & 0.75  & 0.25 & -0.028        & 0.15 & 0.115              & -0.703        & -0.248  & -0.04  & 0.501    & 0.963                   & -1.128 & -0.189 & 0.391   \\
KM\_Mod   & $D_\alpha$ & 3 & 7     & 0.75  & 0.25 & -0.007        & 0.15 & 0.108              & -0.64         & -0.061  & -0.01  & 0.497    & 1.003                   & -0.261 & -0.044 & 0.843   \\
KM\_Med & $D_\alpha$ & 3 & 7     & 0.75  & 0.25 & -0.024        & 0.15 & 0.107              & -0.775        & -0.224  & -0.031 & 0.489    & 1.016                   & -0.952 & -0.16  & 0.471   \\
SP\_Mod    & $D_\alpha$ & 3 & 7     & 0.75  & 0.25 & -0.009        & 0.15 & 0.107              & -0.662        & -0.083  & -0.014 & 0.494    & 1.012                   & -0.355 & -0.06  & 0.788   \\
SP\_Med  & $D_\alpha$ & 3 & 7     & 0.75  & 0.25 & -0.029        & 0.15 & 0.106              & -0.805        & -0.271  & -0.036 & 0.492    & 0.998                   & -1.14  & -0.191 & 0.389   \\
KM\_Mod   & $D_\alpha$ & 5 & 1     & 0.75  & 0.25 & -0.11         & 0.15 & 0.118              & -0.923        & -0.934  & -0.119 & 0.48     & 0.944                   & -4.375 & -0.735 & 0.001   \\
KM\_Med & $D_\alpha$ & 5 & 1     & 0.75  & 0.25 & -0.093        & 0.15 & 0.116              & -0.896        & -0.795  & -0.103 & 0.486    & 0.942                   & -3.673 & -0.617 & 0.005   \\
SP\_Mod    & $D_\alpha$ & 5 & 1     & 0.75  & 0.25 & -0.122        & 0.15 & 0.119              & -0.937        & -1.022  & -0.13  & 0.479    & 0.931                   & -4.827 & -0.811 & 0.0     \\
SP\_Med  & $D_\alpha$ & 5 & 1     & 0.75  & 0.25 & -0.109        & 0.15 & 0.118              & -0.921        & -0.925  & -0.118 & 0.484    & 0.929                   & -4.323 & -0.726 & 0.001   \\
KM\_Mod   & $D_\alpha$ & 5 & 3     & 0.75  & 0.25 & 0.005         & 0.15 & 0.112              & -0.481        & 0.048   & 0.011  & 0.504    & 0.99                    & 0.213  & 0.036  & 0.872   \\
KM\_Med & $D_\alpha$ & 5 & 3     & 0.75  & 0.25 & 0.016         & 0.15 & 0.11               & -0.486        & 0.143   & 0.032  & 0.503    & 1.008                   & 0.626  & 0.105  & 0.635   \\
SP\_Mod    & $D_\alpha$ & 5 & 3     & 0.75  & 0.25 & 0.02          & 0.15 & 0.112              & -0.39         & 0.182   & 0.052  & 0.508    & 0.993                   & 0.808  & 0.136  & 0.54    \\
SP\_Med  & $D_\alpha$ & 5 & 3     & 0.75  & 0.25 & 0.021         & 0.15 & 0.109              & -0.351        & 0.19    & 0.059  & 0.504    & 1.01                    & 0.823  & 0.138  & 0.532   \\
KM\_Mod   & $D_\alpha$ & 5 & 5     & 0.75  & 0.25 & -0.039        & 0.15 & 0.117              & -0.777        & -0.336  & -0.05  & 0.495    & 0.97                    & -1.556 & -0.261 & 0.236   \\
KM\_Med & $D_\alpha$ & 5 & 5     & 0.75  & 0.25 & -0.042        & 0.15 & 0.114              & -0.817        & -0.366  & -0.051 & 0.494    & 0.971                   & -1.661 & -0.279 & 0.207   \\
SP\_Mod    & $D_\alpha$ & 5 & 5     & 0.75  & 0.25 & -0.063        & 0.15 & 0.118              & -0.849        & -0.534  & -0.074 & 0.497    & 0.933                   & -2.503 & -0.421 & 0.056   \\
SP\_Med  & $D_\alpha$ & 5 & 5     & 0.75  & 0.25 & -0.037        & 0.15 & 0.116              & -0.78         & -0.319  & -0.047 & 0.499    & 0.958                   & -1.465 & -0.246 & 0.265   \\
KM\_Mod   & $D_\alpha$ & 5 & 7     & 0.75  & 0.25 & 0.056         & 0.15 & 0.107              & -0.389        & 0.521   & 0.144  & 0.506    & 1.045                   & 2.216  & 0.372  & 0.092   \\
KM\_Med & $D_\alpha$ & 5 & 7     & 0.75  & 0.25 & 0.041         & 0.15 & 0.108              & -0.413        & 0.383   & 0.1    & 0.501    & 1.047                   & 1.639  & 0.275  & 0.213   \\
SP\_Mod    & $D_\alpha$ & 5 & 7     & 0.75  & 0.25 & 0.051         & 0.15 & 0.104              & -0.42         & 0.494   & 0.122  & 0.505    & 1.045                   & 2.04   & 0.343  & 0.119   \\
SP\_Med  & $D_\alpha$ & 5 & 7     & 0.75  & 0.25 & 0.04          & 0.15 & 0.107              & -0.529        & 0.371   & 0.075  & 0.505    & 1.028                   & 1.572  & 0.264  & 0.232   \\
KM\_Mod   & $D_\alpha$ & 7 & 1     & 0.75  & 0.25 & -0.112        & 0.15 & 0.118              & -0.94         & -0.952  & -0.119 & 0.479    & 0.945                   & -4.444 & -0.747 & 0.001   \\
KM\_Med & $D_\alpha$ & 7 & 1     & 0.75  & 0.25 & -0.093        & 0.15 & 0.117              & -0.916        & -0.794  & -0.102 & 0.484    & 0.947                   & -3.692 & -0.62  & 0.005   \\
SP\_Mod    & $D_\alpha$ & 7 & 1     & 0.75  & 0.25 & -0.09         & 0.15 & 0.118              & -0.911        & -0.764  & -0.099 & 0.483    & 0.957                   & -3.566 & -0.599 & 0.006   \\
SP\_Med  & $D_\alpha$ & 7 & 1     & 0.75  & 0.25 & -0.104        & 0.15 & 0.117              & -0.922        & -0.891  & -0.113 & 0.484    & 0.936                   & -4.124 & -0.693 & 0.002   \\
KM\_Mod   & $D_\alpha$ & 7 & 3     & 0.75  & 0.25 & -0.036        & 0.15 & 0.115              & -0.721        & -0.312  & -0.05  & 0.498    & 0.964                   & -1.419 & -0.238 & 0.281   \\
KM\_Med & $D_\alpha$ & 7 & 3     & 0.75  & 0.25 & -0.022        & 0.15 & 0.113              & -0.642        & -0.191  & -0.034 & 0.502    & 0.964                   & -0.858 & -0.144 & 0.515   \\
SP\_Mod    & $D_\alpha$ & 7 & 3     & 0.75  & 0.25 & -0.019        & 0.15 & 0.113              & -0.721        & -0.165  & -0.026 & 0.499    & 0.979                   & -0.743 & -0.125 & 0.573   \\
SP\_Med  & $D_\alpha$ & 7 & 3     & 0.75  & 0.25 & -0.03         & 0.15 & 0.113              & -0.706        & -0.27   & -0.043 & 0.499    & 0.968                   & -1.208 & -0.203 & 0.359   \\
KM\_Mod   & $D_\alpha$ & 7 & 5     & 0.75  & 0.25 & 0.005         & 0.15 & 0.112              & -0.645        & 0.048   & 0.008  & 0.503    & 0.995                   & 0.213  & 0.036  & 0.872   \\
KM\_Med & $D_\alpha$ & 7 & 5     & 0.75  & 0.25 & 0.035         & 0.15 & 0.111              & -0.39         & 0.316   & 0.09   & 0.511    & 1.001                   & 1.393  & 0.234  & 0.291   \\
SP\_Mod    & $D_\alpha$ & 7 & 5     & 0.75  & 0.25 & 0.004         & 0.15 & 0.113              & -0.703        & 0.038   & 0.006  & 0.508    & 0.975                   & 0.171  & 0.029  & 0.897   \\
SP\_Med  & $D_\alpha$ & 7 & 5     & 0.75  & 0.25 & 0.022         & 0.15 & 0.112              & -0.588        & 0.199   & 0.038  & 0.508    & 0.996                   & 0.885  & 0.149  & 0.502   \\
KM\_Mod   & $D_\alpha$ & 7 & 7     & 0.75  & 0.25 & 0.036         & 0.15 & 0.108              & -0.411        & 0.336   & 0.088  & 0.502    & 1.038                   & 1.441  & 0.242  & 0.274   \\
KM\_Med & $D_\alpha$ & 7 & 7     & 0.75  & 0.25 & 0.036         & 0.15 & 0.108              & -0.399        & 0.335   & 0.091  & 0.499    & 1.05                    & 1.443  & 0.242  & 0.273   \\
SP\_Mod    & $D_\alpha$ & 7 & 7     & 0.75  & 0.25 & 0.027         & 0.15 & 0.108              & -0.474        & 0.253   & 0.057  & 0.498    & 1.043                   & 1.079  & 0.181  & 0.412   \\
SP\_Med  & $D_\alpha$ & 7 & 7     & 0.75  & 0.25 & 0.031         & 0.15 & 0.107              & -0.462        & 0.29    & 0.067  & 0.501    & 1.037                   & 1.23   & 0.207  & 0.35    \\
KM\_Mod   & $D_\alpha$ & 1 & 1     & 0.7   & 0.3  & -0.153        & 0.15 & 0.12               & -0.973        & -1.274  & -0.157 & 0.475    & 0.91                    & -6.056 & -1.017 & 0.0     \\
KM\_Med & $D_\alpha$ & 1 & 1     & 0.7   & 0.3  & -0.14         & 0.15 & 0.12               & -0.965        & -1.17   & -0.145 & 0.477    & 0.918                   & -5.568 & -0.935 & 0.0     \\
SP\_Mod    & $D_\alpha$ & 1 & 1     & 0.7   & 0.3  & -0.148        & 0.15 & 0.118              & -0.969        & -1.259  & -0.153 & 0.475    & 0.916                   & -5.876 & -0.987 & 0.0     \\
SP\_Med  & $D_\alpha$ & 1 & 1     & 0.7   & 0.3  & -0.141        & 0.15 & 0.116              & -0.963        & -1.22   & -0.147 & 0.479    & 0.911                   & -5.599 & -0.941 & 0.0     \\
KM\_Mod   & $D_\alpha$ & 1 & 3     & 0.7   & 0.3  & 0.009         & 0.15 & 0.109              & -0.53         & 0.082   & 0.017  & 0.496    & 1.027                   & 0.354  & 0.06   & 0.788   \\
KM\_Med & $D_\alpha$ & 1 & 3     & 0.7   & 0.3  & 0.016         & 0.15 & 0.11               & -0.57         & 0.142   & 0.027  & 0.502    & 1.011                   & 0.618  & 0.104  & 0.639   \\
SP\_Mod    & $D_\alpha$ & 1 & 3     & 0.7   & 0.3  & -0.012        & 0.15 & 0.113              & -0.602        & -0.105  & -0.02  & 0.505    & 0.967                   & -0.468 & -0.079 & 0.723   \\
SP\_Med  & $D_\alpha$ & 1 & 3     & 0.7   & 0.3  & -0.004        & 0.15 & 0.11               & -0.631        & -0.036  & -0.006 & 0.503    & 0.984                   & -0.156 & -0.026 & 0.906   \\
KM\_Mod   & $D_\alpha$ & 1 & 5     & 0.7   & 0.3  & -0.05         & 0.15 & 0.118              & -0.804        & -0.422  & -0.062 & 0.496    & 0.952                   & -1.972 & -0.331 & 0.133   \\
KM\_Med & $D_\alpha$ & 1 & 5     & 0.7   & 0.3  & -0.042        & 0.15 & 0.117              & -0.785        & -0.362  & -0.054 & 0.496    & 0.962                   & -1.684 & -0.283 & 0.2     \\
SP\_Mod    & $D_\alpha$ & 1 & 5     & 0.7   & 0.3  & -0.043        & 0.15 & 0.118              & -0.793        & -0.362  & -0.054 & 0.497    & 0.959                   & -1.697 & -0.285 & 0.196   \\
SP\_Med  & $D_\alpha$ & 1 & 5     & 0.7   & 0.3  & -0.069        & 0.15 & 0.117              & -0.854        & -0.584  & -0.08  & 0.498    & 0.924                   & -2.719 & -0.457 & 0.038   \\
KM\_Mod   & $D_\alpha$ & 1 & 7     & 0.7   & 0.3  & 0.034         & 0.15 & 0.112              & -0.54         & 0.3     & 0.062  & 0.509    & 1.008                   & 1.334  & 0.224  & 0.312   \\
KM\_Med & $D_\alpha$ & 1 & 7     & 0.7   & 0.3  & 0.027         & 0.15 & 0.111              & -0.552        & 0.246   & 0.05   & 0.511    & 0.988                   & 1.086  & 0.182  & 0.41    \\
SP\_Mod    & $D_\alpha$ & 1 & 7     & 0.7   & 0.3  & 0.017         & 0.15 & 0.111              & -0.71         & 0.154   & 0.024  & 0.501    & 1.016                   & 0.68   & 0.114  & 0.606   \\
SP\_Med  & $D_\alpha$ & 1 & 7     & 0.7   & 0.3  & 0.023         & 0.15 & 0.11               & -0.667        & 0.208   & 0.034  & 0.514    & 0.972                   & 0.911  & 0.153  & 0.49    \\
KM\_Mod   & $D_\alpha$ & 3 & 1     & 0.7   & 0.3  & -0.139        & 0.15 & 0.119              & -0.958        & -1.163  & -0.145 & 0.475    & 0.927                   & -5.505 & -0.925 & 0.0     \\
KM\_Med & $D_\alpha$ & 3 & 1     & 0.7   & 0.3  & -0.148        & 0.15 & 0.119              & -0.963        & -1.239  & -0.153 & 0.478    & 0.908                   & -5.855 & -0.984 & 0.0     \\
SP\_Mod    & $D_\alpha$ & 3 & 1     & 0.7   & 0.3  & -0.151        & 0.15 & 0.12               & -0.967        & -1.264  & -0.156 & 0.472    & 0.924                   & -6.001 & -1.008 & 0.0     \\
SP\_Med  & $D_\alpha$ & 3 & 1     & 0.7   & 0.3  & -0.12         & 0.15 & 0.118              & -0.935        & -1.018  & -0.129 & 0.484    & 0.917                   & -4.774 & -0.802 & 0.0     \\
KM\_Mod   & $D_\alpha$ & 3 & 3     & 0.7   & 0.3  & -0.013        & 0.15 & 0.115              & -0.458        & -0.114  & -0.029 & 0.506    & 0.961                   & -0.519 & -0.087 & 0.694   \\
KM\_Med & $D_\alpha$ & 3 & 3     & 0.7   & 0.3  & -0.0          & 0.15 & 0.113              & -0.388        & -0.004  & -0.001 & 0.504    & 0.982                   & -0.017 & -0.003 & 0.99    \\
SP\_Mod    & $D_\alpha$ & 3 & 3     & 0.7   & 0.3  & 0.002         & 0.15 & 0.113              & -0.406        & 0.013   & 0.004  & 0.506    & 0.976                   & 0.06   & 0.01   & 0.964   \\
SP\_Med  & $D_\alpha$ & 3 & 3     & 0.7   & 0.3  & -0.015        & 0.15 & 0.112              & -0.446        & -0.133  & -0.033 & 0.502    & 0.973                   & -0.59  & -0.099 & 0.654   \\
KM\_Mod   & $D_\alpha$ & 3 & 5     & 0.7   & 0.3  & -0.035        & 0.15 & 0.115              & -0.703        & -0.303  & -0.05  & 0.495    & 0.977                   & -1.384 & -0.233 & 0.293   \\
KM\_Med & $D_\alpha$ & 3 & 5     & 0.7   & 0.3  & -0.041        & 0.15 & 0.116              & -0.786        & -0.352  & -0.052 & 0.494    & 0.974                   & -1.62  & -0.272 & 0.218   \\
SP\_Mod    & $D_\alpha$ & 3 & 5     & 0.7   & 0.3  & -0.036        & 0.15 & 0.117              & -0.734        & -0.312  & -0.049 & 0.499    & 0.96                    & -1.441 & -0.242 & 0.273   \\
SP\_Med  & $D_\alpha$ & 3 & 5     & 0.7   & 0.3  & -0.026        & 0.15 & 0.115              & -0.655        & -0.23   & -0.04  & 0.502    & 0.961                   & -1.051 & -0.177 & 0.424   \\
KM\_Mod   & $D_\alpha$ & 3 & 7     & 0.7   & 0.3  & -0.017        & 0.15 & 0.108              & -0.715        & -0.155  & -0.023 & 0.49     & 1.018                   & -0.664 & -0.112 & 0.615   \\
KM\_Med & $D_\alpha$ & 3 & 7     & 0.7   & 0.3  & -0.022        & 0.15 & 0.108              & -0.739        & -0.201  & -0.029 & 0.489    & 1.018                   & -0.858 & -0.144 & 0.516   \\
SP\_Mod    & $D_\alpha$ & 3 & 7     & 0.7   & 0.3  & -0.005        & 0.15 & 0.108              & -0.685        & -0.047  & -0.007 & 0.495    & 1.016                   & -0.202 & -0.034 & 0.878   \\
SP\_Med  & $D_\alpha$ & 3 & 7     & 0.7   & 0.3  & -0.022        & 0.15 & 0.106              & -0.769        & -0.208  & -0.029 & 0.498    & 0.981                   & -0.877 & -0.147 & 0.507   \\
KM\_Mod   & $D_\alpha$ & 5 & 1     & 0.7   & 0.3  & -0.112        & 0.15 & 0.118              & -0.924        & -0.945  & -0.121 & 0.478    & 0.949                   & -4.43  & -0.744 & 0.001   \\
KM\_Med & $D_\alpha$ & 5 & 1     & 0.7   & 0.3  & -0.097        & 0.15 & 0.117              & -0.904        & -0.832  & -0.107 & 0.485    & 0.94                    & -3.845 & -0.646 & 0.003   \\
SP\_Mod    & $D_\alpha$ & 5 & 1     & 0.7   & 0.3  & -0.12         & 0.15 & 0.12               & -0.935        & -1.002  & -0.128 & 0.48     & 0.932                   & -4.756 & -0.799 & 0.0     \\
SP\_Med  & $D_\alpha$ & 5 & 1     & 0.7   & 0.3  & -0.099        & 0.15 & 0.116              & -0.922        & -0.853  & -0.107 & 0.487    & 0.93                    & -3.917 & -0.658 & 0.003   \\
KM\_Mod   & $D_\alpha$ & 5 & 3     & 0.7   & 0.3  & -0.01         & 0.15 & 0.112              & -0.531        & -0.092  & -0.019 & 0.499    & 0.991                   & -0.408 & -0.069 & 0.757   \\
KM\_Med & $D_\alpha$ & 5 & 3     & 0.7   & 0.3  & 0.012         & 0.15 & 0.111              & -0.491        & 0.104   & 0.024  & 0.504    & 1.0                     & 0.458  & 0.077  & 0.728   \\
SP\_Mod    & $D_\alpha$ & 5 & 3     & 0.7   & 0.3  & 0.013         & 0.15 & 0.111              & -0.381        & 0.12    & 0.035  & 0.506    & 0.991                   & 0.529  & 0.089  & 0.688   \\
SP\_Med  & $D_\alpha$ & 5 & 3     & 0.7   & 0.3  & 0.023         & 0.15 & 0.109              & -0.347        & 0.209   & 0.066  & 0.504    & 1.011                   & 0.906  & 0.152  & 0.492   \\
KM\_Mod   & $D_\alpha$ & 5 & 5     & 0.7   & 0.3  & -0.042        & 0.15 & 0.118              & -0.794        & -0.356  & -0.053 & 0.497    & 0.961                   & -1.663 & -0.279 & 0.206   \\
KM\_Med & $D_\alpha$ & 5 & 5     & 0.7   & 0.3  & -0.04         & 0.15 & 0.115              & -0.817        & -0.351  & -0.049 & 0.496    & 0.966                   & -1.601 & -0.269 & 0.224   \\
SP\_Mod    & $D_\alpha$ & 5 & 5     & 0.7   & 0.3  & -0.067        & 0.15 & 0.119              & -0.853        & -0.562  & -0.078 & 0.498    & 0.926                   & -2.649 & -0.445 & 0.043   \\
SP\_Med  & $D_\alpha$ & 5 & 5     & 0.7   & 0.3  & -0.038        & 0.15 & 0.116              & -0.798        & -0.326  & -0.047 & 0.502    & 0.947                   & -1.498 & -0.252 & 0.255   \\
KM\_Mod   & $D_\alpha$ & 5 & 7     & 0.7   & 0.3  & 0.063         & 0.15 & 0.104              & -0.319        & 0.612   & 0.199  & 0.502    & 1.074                   & 2.518  & 0.423  & 0.054   \\
KM\_Med & $D_\alpha$ & 5 & 7     & 0.7   & 0.3  & 0.05          & 0.15 & 0.105              & -0.396        & 0.479   & 0.127  & 0.501    & 1.062                   & 1.995  & 0.335  & 0.128   \\
SP\_Mod    & $D_\alpha$ & 5 & 7     & 0.7   & 0.3  & 0.055         & 0.15 & 0.104              & -0.416        & 0.528   & 0.133  & 0.507    & 1.041                   & 2.19   & 0.368  & 0.094   \\
SP\_Med  & $D_\alpha$ & 5 & 7     & 0.7   & 0.3  & 0.046         & 0.15 & 0.109              & -0.477        & 0.42    & 0.096  & 0.511    & 1.015                   & 1.816  & 0.305  & 0.167   \\
KM\_Mod   & $D_\alpha$ & 7 & 1     & 0.7   & 0.3  & -0.11         & 0.15 & 0.117              & -0.935        & -0.939  & -0.118 & 0.477    & 0.955                   & -4.364 & -0.733 & 0.001   \\
KM\_Med & $D_\alpha$ & 7 & 1     & 0.7   & 0.3  & -0.109        & 0.15 & 0.118              & -0.935        & -0.927  & -0.117 & 0.483    & 0.933                   & -4.341 & -0.729 & 0.001   \\
SP\_Mod    & $D_\alpha$ & 7 & 1     & 0.7   & 0.3  & -0.088        & 0.15 & 0.117              & -0.903        & -0.753  & -0.097 & 0.48     & 0.969                   & -3.483 & -0.585 & 0.008   \\
SP\_Med  & $D_\alpha$ & 7 & 1     & 0.7   & 0.3  & -0.096        & 0.15 & 0.116              & -0.913        & -0.829  & -0.106 & 0.487    & 0.935                   & -3.828 & -0.643 & 0.003   \\
KM\_Mod   & $D_\alpha$ & 7 & 3     & 0.7   & 0.3  & -0.046        & 0.15 & 0.115              & -0.747        & -0.403  & -0.062 & 0.496    & 0.96                    & -1.832 & -0.308 & 0.164   \\
KM\_Med & $D_\alpha$ & 7 & 3     & 0.7   & 0.3  & -0.027        & 0.15 & 0.115              & -0.693        & -0.235  & -0.039 & 0.503    & 0.956                   & -1.068 & -0.18  & 0.417   \\
SP\_Mod    & $D_\alpha$ & 7 & 3     & 0.7   & 0.3  & -0.002        & 0.15 & 0.113              & -0.618        & -0.014  & -0.002 & 0.507    & 0.97                    & -0.061 & -0.01  & 0.963   \\
SP\_Med  & $D_\alpha$ & 7 & 3     & 0.7   & 0.3  & -0.021        & 0.15 & 0.112              & -0.695        & -0.192  & -0.031 & 0.499    & 0.978                   & -0.853 & -0.143 & 0.518   \\
KM\_Mod   & $D_\alpha$ & 7 & 5     & 0.7   & 0.3  & 0.016         & 0.15 & 0.112              & -0.544        & 0.145   & 0.03   & 0.504    & 1.005                   & 0.645  & 0.108  & 0.625   \\
KM\_Med & $D_\alpha$ & 7 & 5     & 0.7   & 0.3  & 0.027         & 0.15 & 0.111              & -0.481        & 0.24    & 0.056  & 0.509    & 0.998                   & 1.06   & 0.178  & 0.421   \\
SP\_Mod    & $D_\alpha$ & 7 & 5     & 0.7   & 0.3  & 0.001         & 0.15 & 0.113              & -0.703        & 0.013   & 0.002  & 0.511    & 0.961                   & 0.059  & 0.01   & 0.964   \\
SP\_Med  & $D_\alpha$ & 7 & 5     & 0.7   & 0.3  & 0.025         & 0.15 & 0.112              & -0.559        & 0.221   & 0.044  & 0.51     & 0.99                    & 0.986  & 0.166  & 0.455   \\
KM\_Mod   & $D_\alpha$ & 7 & 7     & 0.7   & 0.3  & 0.048         & 0.15 & 0.108              & -0.326        & 0.446   & 0.147  & 0.501    & 1.059                   & 1.901  & 0.319  & 0.148   \\
KM\_Med & $D_\alpha$ & 7 & 7     & 0.7   & 0.3  & 0.031         & 0.15 & 0.108              & -0.414        & 0.284   & 0.074  & 0.501    & 1.036                   & 1.217  & 0.204  & 0.356   \\
SP\_Mod    & $D_\alpha$ & 7 & 7     & 0.7   & 0.3  & 0.033         & 0.15 & 0.108              & -0.465        & 0.309   & 0.072  & 0.5      & 1.044                   & 1.322  & 0.222  & 0.315   \\
SP\_Med  & $D_\alpha$ & 7 & 7     & 0.7   & 0.3  & 0.03          & 0.15 & 0.107              & -0.433        & 0.282   & 0.069  & 0.503    & 1.024                   & 1.192  & 0.2    & 0.365   \\
CCF              & $D_\alpha$ & 1 & 1     & 0.85  & 0.15 & -0.119        & 0.15 & 0.114              & -0.947        & -1.047  & -0.126 & 0.476    & 0.949                   & -4.72  & -0.793 & 0.0     \\
CCF              & $D_\alpha$ & 1 & 3     & 0.85  & 0.15 & -0.001        & 0.15 & 0.111              & -0.583        & -0.012  & -0.002 & 0.501    & 0.994                   & -0.054 & -0.009 & 0.967   \\
CCF              & $D_\alpha$ & 1 & 5     & 0.85  & 0.15 & -0.055        & 0.15 & 0.116              & -0.822        & -0.477  & -0.067 & 0.492    & 0.966                   & -2.186 & -0.367 & 0.096   \\
CCF              & $D_\alpha$ & 1 & 7     & 0.85  & 0.15 & 0.039         & 0.15 & 0.11               & -0.564        & 0.355   & 0.069  & 0.511    & 1.002                   & 1.543  & 0.259  & 0.242   \\
CCF              & $D_\alpha$ & 3 & 1     & 0.85  & 0.15 & -0.113        & 0.15 & 0.116              & -0.924        & -0.979  & -0.123 & 0.476    & 0.957                   & -4.493 & -0.755 & 0.001   \\
CCF              & $D_\alpha$ & 3 & 3     & 0.85  & 0.15 & 0.001         & 0.15 & 0.113              & -0.46         & 0.006   & 0.001  & 0.505    & 0.98                    & 0.026  & 0.004  & 0.985   \\
CCF              & $D_\alpha$ & 3 & 5     & 0.85  & 0.15 & -0.036        & 0.15 & 0.114              & -0.673        & -0.313  & -0.053 & 0.493    & 0.983                   & -1.413 & -0.237 & 0.283   \\
CCF              & $D_\alpha$ & 3 & 7     & 0.85  & 0.15 & -0.007        & 0.15 & 0.105              & -0.678        & -0.067  & -0.01  & 0.495    & 1.012                   & -0.28  & -0.047 & 0.832   \\
CCF              & $D_\alpha$ & 5 & 1     & 0.85  & 0.15 & -0.093        & 0.15 & 0.116              & -0.894        & -0.805  & -0.104 & 0.483    & 0.955                   & -3.698 & -0.621 & 0.005   \\
CCF              & $D_\alpha$ & 5 & 3     & 0.85  & 0.15 & 0.029         & 0.15 & 0.11               & -0.459        & 0.265   & 0.064  & 0.508    & 1.003                   & 1.162  & 0.195  & 0.379   \\
CCF              & $D_\alpha$ & 5 & 5     & 0.85  & 0.15 & -0.072        & 0.15 & 0.116              & -0.864        & -0.625  & -0.084 & 0.49     & 0.95                    & -2.876 & -0.483 & 0.028   \\
CCF              & $D_\alpha$ & 5 & 7     & 0.85  & 0.15 & 0.066         & 0.15 & 0.104              & -0.391        & 0.64    & 0.17   & 0.509    & 1.048                   & 2.635  & 0.443  & 0.044   \\
CCF              & $D_\alpha$ & 7 & 1     & 0.85  & 0.15 & -0.104        & 0.15 & 0.115              & -0.93         & -0.906  & -0.112 & 0.479    & 0.957                   & -4.124 & -0.693 & 0.002   \\
CCF              & $D_\alpha$ & 7 & 3     & 0.85  & 0.15 & -0.024        & 0.15 & 0.112              & -0.64         & -0.215  & -0.038 & 0.499    & 0.973                   & -0.955 & -0.16  & 0.469   \\
CCF              & $D_\alpha$ & 7 & 5     & 0.85  & 0.15 & 0.019         & 0.15 & 0.111              & -0.568        & 0.168   & 0.033  & 0.506    & 0.997                   & 0.741  & 0.124  & 0.574   \\
CCF              & $D_\alpha$ & 7 & 7     & 0.85  & 0.15 & 0.045         & 0.15 & 0.107              & -0.426        & 0.422   & 0.106  & 0.504    & 1.042                   & 1.793  & 0.301  & 0.173   \\
CCF              & $D_\alpha$ & 1 & 1     & 0.8   & 0.2  & -0.107        & 0.15 & 0.113              & -0.937        & -0.946  & -0.114 & 0.478    & 0.956                   & -4.246 & -0.713 & 0.001   \\
CCF              & $D_\alpha$ & 1 & 3     & 0.8   & 0.2  & 0.001         & 0.15 & 0.112              & -0.584        & 0.005   & 0.001  & 0.5      & 1.0                     & 0.023  & 0.004  & 0.986   \\
CCF              & $D_\alpha$ & 1 & 5     & 0.8   & 0.2  & -0.057        & 0.15 & 0.116              & -0.82         & -0.492  & -0.07  & 0.492    & 0.961                   & -2.263 & -0.38  & 0.085   \\
CCF              & $D_\alpha$ & 1 & 7     & 0.8   & 0.2  & 0.043         & 0.15 & 0.11               & -0.547        & 0.39    & 0.078  & 0.508    & 1.021                   & 1.703  & 0.286  & 0.197   \\
CCF              & $D_\alpha$ & 3 & 1     & 0.8   & 0.2  & -0.103        & 0.15 & 0.116              & -0.911        & -0.888  & -0.113 & 0.481    & 0.95                    & -4.099 & -0.689 & 0.002   \\
CCF              & $D_\alpha$ & 3 & 3     & 0.8   & 0.2  & -0.003        & 0.15 & 0.114              & -0.449        & -0.027  & -0.007 & 0.504    & 0.98                    & -0.124 & -0.021 & 0.925   \\
CCF              & $D_\alpha$ & 3 & 5     & 0.8   & 0.2  & -0.028        & 0.15 & 0.113              & -0.655        & -0.251  & -0.043 & 0.491    & 0.999                   & -1.13  & -0.19  & 0.391   \\
CCF              & $D_\alpha$ & 3 & 7     & 0.8   & 0.2  & 0.007         & 0.15 & 0.104              & -0.627        & 0.064   & 0.011  & 0.492    & 1.04                    & 0.263  & 0.044  & 0.842   \\
CCF              & $D_\alpha$ & 5 & 1     & 0.8   & 0.2  & -0.084        & 0.15 & 0.115              & -0.875        & -0.729  & -0.096 & 0.484    & 0.961                   & -3.332 & -0.56  & 0.011   \\
CCF              & $D_\alpha$ & 5 & 3     & 0.8   & 0.2  & 0.011         & 0.15 & 0.112              & -0.529        & 0.094   & 0.02   & 0.504    & 0.998                   & 0.419  & 0.07   & 0.751   \\
CCF              & $D_\alpha$ & 5 & 5     & 0.8   & 0.2  & -0.044        & 0.15 & 0.114              & -0.821        & -0.39   & -0.054 & 0.493    & 0.973                   & -1.757 & -0.295 & 0.182   \\
CCF              & $D_\alpha$ & 5 & 7     & 0.8   & 0.2  & 0.081         & 0.15 & 0.103              & -0.398        & 0.779   & 0.202  & 0.507    & 1.074                   & 3.195  & 0.537  & 0.014   \\
CCF              & $D_\alpha$ & 7 & 1     & 0.8   & 0.2  & -0.096        & 0.15 & 0.115              & -0.912        & -0.838  & -0.106 & 0.479    & 0.967                   & -3.819 & -0.642 & 0.004   \\
CCF              & $D_\alpha$ & 7 & 3     & 0.8   & 0.2  & -0.014        & 0.15 & 0.113              & -0.607        & -0.122  & -0.023 & 0.5      & 0.983                   & -0.546 & -0.092 & 0.679   \\
CCF              & $D_\alpha$ & 7 & 5     & 0.8   & 0.2  & 0.016         & 0.15 & 0.111              & -0.562        & 0.143   & 0.028  & 0.502    & 1.011                   & 0.629  & 0.106  & 0.633   \\
CCF              & $D_\alpha$ & 7 & 7     & 0.8   & 0.2  & 0.064         & 0.15 & 0.106              & -0.38         & 0.603   & 0.169  & 0.503    & 1.072                   & 2.548  & 0.428  & 0.053   \\
CCF              & $D_\alpha$ & 1 & 1     & 0.75  & 0.25 & -0.108        & 0.15 & 0.113              & -0.938        & -0.952  & -0.115 & 0.479    & 0.953                   & -4.269 & -0.717 & 0.001   \\
CCF              & $D_\alpha$ & 1 & 3     & 0.75  & 0.25 & 0.013         & 0.15 & 0.112              & -0.527        & 0.113   & 0.024  & 0.505    & 0.995                   & 0.502  & 0.084  & 0.704   \\
CCF              & $D_\alpha$ & 1 & 5     & 0.75  & 0.25 & -0.057        & 0.15 & 0.117              & -0.834        & -0.49   & -0.068 & 0.493    & 0.958                   & -2.266 & -0.381 & 0.084   \\
CCF              & $D_\alpha$ & 1 & 7     & 0.75  & 0.25 & 0.047         & 0.15 & 0.111              & -0.503        & 0.428   & 0.094  & 0.511    & 1.014                   & 1.879  & 0.316  & 0.155   \\
CCF              & $D_\alpha$ & 3 & 1     & 0.75  & 0.25 & -0.094        & 0.15 & 0.116              & -0.89         & -0.807  & -0.106 & 0.482    & 0.954                   & -3.732 & -0.627 & 0.004   \\
CCF              & $D_\alpha$ & 3 & 3     & 0.75  & 0.25 & -0.002        & 0.15 & 0.114              & -0.414        & -0.018  & -0.005 & 0.506    & 0.972                   & -0.08  & -0.014 & 0.951   \\
CCF              & $D_\alpha$ & 3 & 5     & 0.75  & 0.25 & -0.038        & 0.15 & 0.113              & -0.72         & -0.331  & -0.052 & 0.493    & 0.983                   & -1.49  & -0.25  & 0.257   \\
CCF              & $D_\alpha$ & 3 & 7     & 0.75  & 0.25 & 0.01          & 0.15 & 0.105              & -0.65         & 0.092   & 0.015  & 0.498    & 1.021                   & 0.383  & 0.064  & 0.771   \\
CCF              & $D_\alpha$ & 5 & 1     & 0.75  & 0.25 & -0.078        & 0.15 & 0.114              & -0.869        & -0.678  & -0.089 & 0.483    & 0.972                   & -3.077 & -0.517 & 0.019   \\
CCF              & $D_\alpha$ & 5 & 3     & 0.75  & 0.25 & 0.01          & 0.15 & 0.111              & -0.573        & 0.091   & 0.018  & 0.505    & 0.992                   & 0.403  & 0.068  & 0.76    \\
CCF              & $D_\alpha$ & 5 & 5     & 0.75  & 0.25 & -0.049        & 0.15 & 0.113              & -0.836        & -0.438  & -0.059 & 0.492    & 0.973                   & -1.954 & -0.328 & 0.138   \\
CCF              & $D_\alpha$ & 5 & 7     & 0.75  & 0.25 & 0.057         & 0.15 & 0.108              & -0.476        & 0.525   & 0.119  & 0.51     & 1.032                   & 2.245  & 0.377  & 0.088   \\
CCF              & $D_\alpha$ & 7 & 1     & 0.75  & 0.25 & -0.083        & 0.15 & 0.115              & -0.895        & -0.725  & -0.093 & 0.481    & 0.975                   & -3.303 & -0.555 & 0.012   \\
CCF              & $D_\alpha$ & 7 & 3     & 0.75  & 0.25 & -0.012        & 0.15 & 0.113              & -0.606        & -0.104  & -0.019 & 0.503    & 0.973                   & -0.463 & -0.078 & 0.725   \\
CCF              & $D_\alpha$ & 7 & 5     & 0.75  & 0.25 & 0.023         & 0.15 & 0.112              & -0.549        & 0.207   & 0.042  & 0.507    & 1.002                   & 0.916  & 0.154  & 0.488   \\
CCF              & $D_\alpha$ & 7 & 7     & 0.75  & 0.25 & 0.061         & 0.15 & 0.107              & -0.393        & 0.574   & 0.156  & 0.511    & 1.032                   & 2.439  & 0.41   & 0.064   \\
CCF              & $D_\alpha$ & 1 & 1     & 0.7   & 0.3  & -0.115        & 0.15 & 0.113              & -0.943        & -1.015  & -0.122 & 0.475    & 0.959                   & -4.561 & -0.766 & 0.001   \\
CCF              & $D_\alpha$ & 1 & 3     & 0.7   & 0.3  & 0.008         & 0.15 & 0.113              & -0.539        & 0.075   & 0.016  & 0.504    & 0.994                   & 0.334  & 0.056  & 0.8     \\
CCF              & $D_\alpha$ & 1 & 5     & 0.7   & 0.3  & -0.05         & 0.15 & 0.116              & -0.796        & -0.435  & -0.063 & 0.493    & 0.965                   & -2.001 & -0.336 & 0.128   \\
CCF              & $D_\alpha$ & 1 & 7     & 0.7   & 0.3  & 0.051         & 0.15 & 0.111              & -0.527        & 0.461   & 0.097  & 0.512    & 1.017                   & 2.026  & 0.34   & 0.125   \\
CCF              & $D_\alpha$ & 3 & 1     & 0.7   & 0.3  & -0.096        & 0.15 & 0.117              & -0.897        & -0.823  & -0.107 & 0.481    & 0.958                   & -3.817 & -0.641 & 0.003   \\
CCF              & $D_\alpha$ & 3 & 3     & 0.7   & 0.3  & -0.007        & 0.15 & 0.114              & -0.436        & -0.059  & -0.016 & 0.506    & 0.969                   & -0.268 & -0.045 & 0.839   \\
CCF              & $D_\alpha$ & 3 & 5     & 0.7   & 0.3  & -0.027        & 0.15 & 0.114              & -0.635        & -0.235  & -0.042 & 0.496    & 0.982                   & -1.062 & -0.178 & 0.42    \\
CCF              & $D_\alpha$ & 3 & 7     & 0.7   & 0.3  & 0.0           & 0.15 & 0.105              & -0.654        & 0.004   & 0.001  & 0.497    & 1.011                   & 0.018  & 0.003  & 0.989   \\
CCF              & $D_\alpha$ & 5 & 1     & 0.7   & 0.3  & -0.08         & 0.15 & 0.114              & -0.872        & -0.698  & -0.092 & 0.482    & 0.972                   & -3.168 & -0.532 & 0.016   \\
CCF              & $D_\alpha$ & 5 & 3     & 0.7   & 0.3  & 0.002         & 0.15 & 0.112              & -0.614        & 0.016   & 0.003  & 0.505    & 0.981                   & 0.07   & 0.012  & 0.957   \\
CCF              & $D_\alpha$ & 5 & 5     & 0.7   & 0.3  & -0.046        & 0.15 & 0.113              & -0.812        & -0.407  & -0.057 & 0.495    & 0.963                   & -1.823 & -0.306 & 0.166   \\
CCF              & $D_\alpha$ & 5 & 7     & 0.7   & 0.3  & 0.068         & 0.15 & 0.107              & -0.442        & 0.629   & 0.153  & 0.509    & 1.048                   & 2.683  & 0.451  & 0.041   \\
CCF              & $D_\alpha$ & 7 & 1     & 0.7   & 0.3  & -0.095        & 0.15 & 0.115              & -0.914        & -0.82   & -0.104 & 0.479    & 0.966                   & -3.756 & -0.631 & 0.004   \\
CCF              & $D_\alpha$ & 7 & 3     & 0.7   & 0.3  & -0.008        & 0.15 & 0.113              & -0.63         & -0.075  & -0.013 & 0.505    & 0.969                   & -0.336 & -0.056 & 0.799   \\
CCF              & $D_\alpha$ & 7 & 5     & 0.7   & 0.3  & 0.023         & 0.15 & 0.112              & -0.56         & 0.209   & 0.042  & 0.509    & 0.994                   & 0.925  & 0.155  & 0.483   \\
CCF              & $D_\alpha$ & 7 & 7     & 0.7   & 0.3  & 0.053         & 0.15 & 0.107              & -0.432        & 0.496   & 0.123  & 0.509    & 1.031                   & 2.116  & 0.355  & 0.108  \\


\hline
\end{longtable}
\end{small}




\end{landscape}
%\end{document}
